# Supplementary material for: The G-index of a closed, spin, hyperbolic manifold of dimension 2 or 4
Source: arXiv:2106.04642 ancillary file (2022-05-14)
Supplement: Supplementary file 1 [file davishsi042621indexed.pdf]

# Davis manifold harmonic spinors

Steven Tschantz

4/26/21

---

## Routines

Some legacy routines.

*ldot*

```
ln[ ]:= ldot[x_, y_] := Drop[x, -1].Drop[y, -1] - x[[-1]] * y[[-1]];
```

*jmat*

```
ln[ ]:= jmat[n_] := DiagonalMatrix[Append[Table[1, {n}], -1]];
```

*rmat*

```
ln[ ]:= rmat[v_] := IdentityMatrix[Length[v]] - 2 * Transpose[Table[v, {Length[v]}]] *  
  (Table[v, {Length[v]}].jmat[Length[v] - 1]) / ldot[v, v];
```

*rmat*

```
ln[ ]:= rmat[v_] := IdentityMatrix[Length[v]] -  
  2 * Outer[Times, v, Append[Drop[v, -1], -v[[-1]]], 1] / ldot[v, v];
```

*diagram*

```
ln[ ]:= diagram[m_, opts___] := Graph[Apply[Join, Flatten[Table[  
  Which[m[[i, j]] == 2, {}, m[[i, j]] == 3, {UndirectedEdge[i, j]}, IntegerQ[m[[i, j]]],  
    {Labeled[UndirectedEdge[i, j], ToString[m[[i, j]]]}], m[[i, j]] == Infinity,  
    {Labeled[UndirectedEdge[i, j], "\infty"}], True, {Labeled[UndirectedEdge[i, j], "*"}]],  
  {i, 1, Length[m] - 1}, {j, i + 1, Length[m]}, 1]], opts];
```

*sggen*

```
ln[ ]:= sggen[gen_, nmax_ : Infinity] :=  
  FixedPoint[Function[p, {Union[p[[1]], Apply[Union, Map[Function[m, Map[m.# &, gen]],  
    Complement[p[[1]], p[[2]]]}], p[[1]]}],  
    {{IdentityMatrix[Length[gen[[1]]]}], {}, nmax}][[1]];
```

---

## Complex, Quaternions

Write  $\text{complex}[a_1, a_2]$  for  $a_1 + i a_2$  with  $a_1$  and  $a_2$  real, explicitly the real and complex parts. Represent complex numbers as  $2 \times 2$  matrices of reals,  $n \times n$  complex matrices as  $2n \times 2n$  real matrices. Choose the matrix for  $\exp(i\theta)$  to be a positive rotation by angle  $\theta$ . Write  $\text{quaternion}[a_1, a_2, a_3, a_4]$  for  $a_1 + i a_2 + j a_3 + k a_4$  with  $a_i$  assumed real. Represent quaternions as  $2 \times 2$  complex matrices and so  $4 \times 4$  real matrices,  $n \times n$  quaternion matrices as  $2n \times 2n$  complex or  $4n \times 4n$  real matrices. Choose the matrix for quaternions so unit quaternions are in  $\text{SU}(2)$ .

*complex, quaternion*

```
In[ ]:= complex[ ] = complex[0, 0];
quaternion[ ] = quaternion[0, 0, 0, 0];
```

*fromcomplex, tocomplex*

```
In[ ]:= tocomplex[z_] := complex[Re[z], Im[z]];
fromcomplex[x_] := x /. {complex[a1_, a2_] => a1 + I * a2};
```

*compleximat, complexonemat*

```
In[ ]:= complexonemat = {{1, 0}, {0, 1}};
compleximat = {{0, -1}, {1, 0}};
```

*complextomatrix, matrixiscomplex, matrixtocomplex*

```
In[ ]:= complextomatrix[complex[a1_, a2_]] := a1 * complexonemat + a2 * compleximat;
matrixtocomplex[{{a11_, a12_}, {a21_, a22_}}] := complex[a11, a21];
matrixiscomplex[m_] := m == complextomatrix[matrixtocomplex[m]];
```

*complexconjugate, complexnorm*

```
In[ ]:= complexconjugate[complex[a1_, a2_]] := complex[a1, -a2];
complexnorm[complex[a1_, a2_]] := Sqrt[a1^2 + a2^2];
```

*cmattormat, rmatiscmat, rmattocmat*

```
In[ ]:= cmattormat[m_?MatrixQ] := ArrayFlatten[Map[complextomatrix, m, {2}]];
rmatiscmat[m_?MatrixQ] :=
  Map[matrixtocomplex, Transpose[Partition[Map[Partition[#, 2] &, m], 2], {1, 3, 2}], {2}];
rmatiscmat[m_] := m == cmattormat[rmatiscmat[m]];
```

*quaternionicmat, quaternionjcmat, quaternionkcmat, quaterniononecmat*

```
In[ ]:= quaterniononecmat = Map[tocomplex, {{1, 0}, {0, 1}}, {2}];
quaternionicmat = Map[tocomplex, {{I, 0}, {0, -I}}, {2}];
quaternionjcmat = Map[tocomplex, {{0, 1}, {-1, 0}}, {2}];
quaternionkcmat = Map[tocomplex, {{0, I}, {I, 0}}, {2}];
```

*cmatrixisquaternion, cmatrixtoquaternion, quaterniontocmatrix*

```
In[ ]:= quaterniontocmatrix[quaternion[a1_, a2_, a3_, a4_]] :=
  rmatiscmat[a1 * cmattormat[quaterniononecmat] + a2 * cmattormat[quaternionicmat] +
    a3 * cmattormat[quaternionjcmat] + a4 * cmattormat[quaternionkcmat]];
cmatrixtoquaternion[m_] := quaternion[m[[1, 1, 1]], m[[1, 1, 2]],
  m[[1, 2, 1]], m[[1, 2, 2]]];
cmatrixisquaternion[m_] := m == quaterniontocmatrix[cmatrixtoquaternion[m]];
```

*quaternionconjugate, quaternionnorm*

```
In[ ]:= quaternionconjugate[quaternion[a1_, a2_, a3_, a4_]] := quaternion[a1, -a2, -a3, -a4];
quaternionnorm[quaternion[a1_, a2_, a3_, a4_]] := Sqrt[a1^2 + a2^2 + a3^2 + a4^2];
```

*matrixisquaternion, matrixtoquaternion, quaterniontomatrix*

```
In[ ]:= quaterniontomatrix[q_] := cmattormat[quaterniontocmatrix[q]];
matrixtoquaternion[m_] := cmatrixtoquaternion[rmatiscmat[m]];
matrixisquaternion[m_] := m == quaterniontomatrix[matrixtoquaternion[m]];
```

*cmatisqmat, cmattoqmat, qmattocmat*

```
In[ ]:= qmattocmat[m_?MatrixQ] := ArrayFlatten[Map[quaterniontocmatrix, m, {2}]];
cmattoqmat[m_?MatrixQ] := Map[cmatrixtoquaternion,
  Transpose[Partition[Map[Partition[#, 2] &, m], 2], {1, 3, 2}], {2}];
cmatisqmat[m_] := m == qmattocmat[cmattoqmat[m]];
```

*qmattormat, rmatiscqmat, rmattoqmat*

```
In[ ]:= qmattormat[m_?MatrixQ] := cmattormat[qmattocmat[m]];
rmattoqmat[m_?MatrixQ] := cmattoqmat[rmatiscqmat[m]];
rmatiscqmat[m_] := m == qmattormat[rmattoqmat[m]];
```

Format

```
In[ ]:= Format[quaternion[a1_, a2_, a3_, a4_]] := a1 + a2 * i + a3 * j + a4 * k;
```

## Representation of Spin(4,1)

```
In[ ]:= matrixtoquaternion[quaterniontomatrix[quaternion[a0, a1, 0, 0]] +
  quaterniontomatrix[quaternion[b0, b1, 0, 0]].quaterniontomatrix[quaternion[0, 0, 1, 0]]]
```

```
Out[ ]:= a0 + a1 i + b0 j + b1 k
```

```
In[ ]:= fromcomplex[quaterniontomatrix[%]] // MatrixForm
```

```
Out[ ]//MatrixForm=
```

$$\begin{pmatrix} a0 + i a1 & b0 + i b1 \\ -b0 + i b1 & a0 - i a1 \end{pmatrix}$$

```
qm1, qm2, qm3, qm4, qm5
```

```
In[ ]:= qm1 = {{quaternion[0, 0, 0, 0], quaternion[1, 0, 0, 0]},
  {quaternion[-1, 0, 0, 0], quaternion[0, 0, 0, 0]}};
qm2 = {{quaternion[0, 0, 0, 0], quaternion[0, 1, 0, 0]},
  {quaternion[0, 1, 0, 0], quaternion[0, 0, 0, 0]}};
qm3 = {{quaternion[0, 0, 0, 0], quaternion[0, 0, 1, 0]},
  {quaternion[0, 0, 1, 0], quaternion[0, 0, 0, 0]}};
qm4 = {{quaternion[0, 0, 0, 0], quaternion[0, 0, 0, 1]},
  {quaternion[0, 0, 0, 1], quaternion[0, 0, 0, 0]}};
qm5 = {{quaternion[1, 0, 0, 0], quaternion[0, 0, 0, 0]},
  {quaternion[0, 0, 0, 0], quaternion[-1, 0, 0, 0]}};
```

```
In[ ]:= Map[MatrixForm, {qm1, qm2, qm3, qm4, qm5}]
```

$$\text{Out[ ]} = \left\{ \begin{pmatrix} 0 & 1 \\ -1 & 0 \end{pmatrix}, \begin{pmatrix} 0 & i \\ i & 0 \end{pmatrix}, \begin{pmatrix} 0 & j \\ j & 0 \end{pmatrix}, \begin{pmatrix} 0 & k \\ k & 0 \end{pmatrix}, \begin{pmatrix} 1 & 0 \\ 0 & -1 \end{pmatrix} \right\}$$

```
cm1, cm2, cm3, cm4, cm5
```

```
In[ ]:= Map[MatrixForm,
  {cm1, cm2, cm3, cm4, cm5} = Map[fromcomplex[qmattocmat[#]] &, {qm1, qm2, qm3, qm4, qm5}]]
```

$$\text{Out[ ]} = \left\{ \begin{pmatrix} 0 & 0 & 1 & 0 \\ 0 & 0 & 0 & 1 \\ -1 & 0 & 0 & 0 \\ 0 & -1 & 0 & 0 \end{pmatrix}, \begin{pmatrix} 0 & 0 & i & 0 \\ 0 & 0 & 0 & -i \\ i & 0 & 0 & 0 \\ 0 & -i & 0 & 0 \end{pmatrix}, \begin{pmatrix} 0 & 0 & 0 & 1 \\ 0 & 0 & -1 & 0 \\ 0 & 1 & 0 & 0 \\ -1 & 0 & 0 & 0 \end{pmatrix}, \begin{pmatrix} 0 & 0 & 0 & i \\ 0 & 0 & i & 0 \\ 0 & i & 0 & 0 \\ i & 0 & 0 & 0 \end{pmatrix}, \begin{pmatrix} 1 & 0 & 0 & 0 \\ 0 & 1 & 0 & 0 \\ 0 & 0 & -1 & 0 \\ 0 & 0 & 0 & -1 \end{pmatrix} \right\}$$

*rm1, rm2, rm3, rm4, rm5*

```
In[ ]:= Map[MatrixForm, {rm1, rm2, rm3, rm4, rm5} = Map[qmattormat[#, &], {qm1, qm2, qm3, qm4, qm5}]]
```

$$\text{Out[ ]} = \left\{ \begin{pmatrix} 0 & 0 & 0 & 0 & 1 & 0 & 0 & 0 \\ 0 & 0 & 0 & 0 & 0 & 1 & 0 & 0 \\ 0 & 0 & 0 & 0 & 0 & 0 & 1 & 0 \\ 0 & 0 & 0 & 0 & 0 & 0 & 0 & 1 \\ -1 & 0 & 0 & 0 & 0 & 0 & 0 & 0 \\ 0 & -1 & 0 & 0 & 0 & 0 & 0 & 0 \\ 0 & 0 & -1 & 0 & 0 & 0 & 0 & 0 \\ 0 & 0 & 0 & -1 & 0 & 0 & 0 & 0 \end{pmatrix}, \begin{pmatrix} 0 & 0 & 0 & 0 & 0 & -1 & 0 & 0 \\ 0 & 0 & 0 & 0 & 1 & 0 & 0 & 0 \\ 0 & 0 & 0 & 0 & 0 & 0 & 0 & 1 \\ 0 & 0 & 0 & 0 & 0 & 0 & -1 & 0 \\ 0 & -1 & 0 & 0 & 0 & 0 & 0 & 0 \\ 1 & 0 & 0 & 0 & 0 & 0 & 0 & 0 \\ 0 & 0 & 0 & 1 & 0 & 0 & 0 & 0 \\ 0 & 0 & -1 & 0 & 0 & 0 & 0 & 0 \end{pmatrix}, \right.$$

$$\left. \begin{pmatrix} 0 & 0 & 0 & 0 & 0 & 0 & 1 & 0 \\ 0 & 0 & 0 & 0 & 0 & 0 & 0 & 1 \\ 0 & 0 & 0 & 0 & -1 & 0 & 0 & 0 \\ 0 & 0 & 0 & 0 & 0 & -1 & 0 & 0 \\ 0 & 0 & 1 & 0 & 0 & 0 & 0 & 0 \\ 0 & 0 & 0 & 1 & 0 & 0 & 0 & 0 \\ -1 & 0 & 0 & 0 & 0 & 0 & 0 & 0 \\ 0 & -1 & 0 & 0 & 0 & 0 & 0 & 0 \end{pmatrix}, \begin{pmatrix} 0 & 0 & 0 & 0 & 0 & 0 & 0 & -1 \\ 0 & 0 & 0 & 0 & 0 & 0 & 1 & 0 \\ 0 & 0 & 0 & 0 & 0 & -1 & 0 & 0 \\ 0 & 0 & 0 & 0 & 1 & 0 & 0 & 0 \\ 0 & 0 & 0 & -1 & 0 & 0 & 0 & 0 \\ 0 & 0 & 1 & 0 & 0 & 0 & 0 & 0 \\ 0 & -1 & 0 & 0 & 0 & 0 & 0 & 0 \\ 1 & 0 & 0 & 0 & 0 & 0 & 0 & 0 \end{pmatrix}, \begin{pmatrix} 1 & 0 & 0 & 0 & 0 & 0 & 0 & 0 \\ 0 & 1 & 0 & 0 & 0 & 0 & 0 & 0 \\ 0 & 0 & 1 & 0 & 0 & 0 & 0 & 0 \\ 0 & 0 & 0 & 1 & 0 & 0 & 0 & 0 \\ 0 & 0 & 0 & 0 & -1 & 0 & 0 & 0 \\ 0 & 0 & 0 & 0 & 0 & -1 & 0 & 0 \\ 0 & 0 & 0 & 0 & 0 & 0 & -1 & 0 \\ 0 & 0 & 0 & 0 & 0 & 0 & 0 & -1 \end{pmatrix} \right\}$$

```
In[ ]:= Map[rmattoqmat,
  Map[Apply[Dot, #] &, Join[{{IdentityMatrix[8]}}, Subsets[#, {2}], Subsets[#, {4}]]] &[
    {rm1, rm2, rm3, rm4, rm5}]]
```

```
Out[ ]:= {{ {1, 0}, {0, 1}}, {{i, 0}, {0, -i}}, {{j, 0}, {0, -j}}, {{k, 0}, {0, -k}},
  {{0, -1}, {-1, 0}}, {{k, 0}, {0, k}}, {{-j, 0}, {0, -j}}, {{0, -i}, {i, 0}},
  {{i, 0}, {0, i}}, {{0, -j}, {j, 0}}, {{0, -k}, {k, 0}}, {{-1, 0}, {0, 1}},
  {{0, -k}, {-k, 0}}, {{0, j}, {j, 0}}, {{0, -i}, {-i, 0}}, {{0, 1}, {-1, 0}} }
```

```
In[ ]:= rmattoqmat[
  Total[MapThread[Times, {Map[qmattormat, %], {a0 + d0, a1 - d1, a2 - d2, a3 - d3, -b0 - c0,
    a3 + d3, -a2 - d2, -b1 + c1, a1 + d1, -b2 + c2, -b3 + c3, -a0 + d0,
    -b3 - c3, b2 + c2, -b1 - c1, b0 - c0} / 2}]]] // Simplify // MatrixForm
```

*Out[ ]//MatrixForm=*

$$\begin{pmatrix} a0 + a1 i + a2 j + a3 k & b0 + b1 i + b2 j + b3 k \\ c0 + c1 i + c2 j + c3 k & d0 + d1 i + d2 j + d3 k \end{pmatrix}$$

*isSU11Hq*

```
In[ ]:= isSU11Hq[qm_] := qmattormat[Transpose[Map[quaternionconjugate, qm, {2}]]] .
  qmattormat[qm5].qmattormat[qm] == qmattormat[qm5];
```

*isSU11H*

```
In[ ]:= isSU11H[rm_] := qmattormat[Transpose[Map[quaternionconjugate, rmattoqmat[rm], {2}]]] .
  qmattormat[qm5].rm == qmattormat[qm5];
```

*inverseSU11Hq*

```
In[ ]:= inverseSU11Hq[qm_] := rmattoqmat[qmattormat[qm5] .
  qmattormat[Transpose[Map[quaternionconjugate, qm, {2}]]] . qmattormat[qm5]];
```

*inverseSU11H*

```
In[ ]:= inverseSU11H[rm_] := qmattormat[qm5] .
  qmattormat[Transpose[Map[quaternionconjugate, rmattoqmat[rm], {2}]]] . qmattormat[qm5];
```

```
In[ ]:= FullSimplify[
  qmattormat[inverseSU11Hq[{{quaternion[a0, a1, a2, a3], quaternion[b0, b1, b2, b3]},
    {quaternion[c0, c1, c2, c3], quaternion[d0, d1, d2, d3]}}]].
  qmattormat[{{quaternion[a0, a1, a2, a3], quaternion[b0, b1, b2, b3]},
    {quaternion[c0, c1, c2, c3], quaternion[d0, d1, d2, d3]}}] ==
  IdentityMatrix[8], Assumptions →
  {Element[a0 | a1 | a2 | a3 | b0 | b1 | b2 | b3 | c0 | c1 | c2 | c3 | d0 | d1 | d2 | d3, Reals] &&
    LogicalExpand[isSU11Hq[{{quaternion[a0, a1, a2, a3], quaternion[b0, b1, b2, b3]},
      {quaternion[c0, c1, c2, c3], quaternion[d0, d1, d2, d3]}}]]]}
```

```
Out[ ]:= True
```

```
In[ ]:= FullSimplify[
  inverseSU11H[qmattormat[{{quaternion[a0, a1, a2, a3], quaternion[b0, b1, b2, b3]},
    {quaternion[c0, c1, c2, c3], quaternion[d0, d1, d2, d3]}}]].
  qmattormat[{{quaternion[a0, a1, a2, a3], quaternion[b0, b1, b2, b3]},
    {quaternion[c0, c1, c2, c3], quaternion[d0, d1, d2, d3]}}] == IdentityMatrix[8],
  Assumptions → {Element[a0 | a1 | a2 | a3 | b0 | b1 | b2 | b3 | c0 | c1 | c2 | c3 | d0 | d1 | d2 | d3,
    Reals] && LogicalExpand[isSU11H[qmattormat[{{quaternion[a0, a1, a2, a3], quaternion[b0, b1, b2, b3]},
      {quaternion[c0, c1, c2, c3], quaternion[d0, d1, d2, d3]}}]]]}]}
```

```
Out[ ]:= True
```

h4tow, wtoh4

```
In[ ]:= h4tow[{v1_, v2_, v3_, v4_, v5_}] := v1 * rm1 + v2 * rm2 + v3 * rm3 + v4 * rm4 + v5 * rm5;
wtoh4[w_] := {w[[1, 5]], -w[[1, 6]], w[[1, 7]], -w[[1, 8]], w[[1, 1]]};
```

```
In[ ]:= h4tow[{v1, v2, v3, v4, v5}] // MatrixForm
```

Out[ ]//MatrixForm=

$$\begin{pmatrix} v5 & 0 & 0 & 0 & v1 & -v2 & v3 & -v4 \\ 0 & v5 & 0 & 0 & v2 & v1 & v4 & v3 \\ 0 & 0 & v5 & 0 & -v3 & -v4 & v1 & v2 \\ 0 & 0 & 0 & v5 & v4 & -v3 & -v2 & v1 \\ -v1 & -v2 & v3 & -v4 & -v5 & 0 & 0 & 0 \\ v2 & -v1 & v4 & v3 & 0 & -v5 & 0 & 0 \\ -v3 & -v4 & -v1 & v2 & 0 & 0 & -v5 & 0 \\ v4 & -v3 & -v2 & -v1 & 0 & 0 & 0 & -v5 \end{pmatrix}$$

```
In[ ]:= wtoh4[%]
```

```
Out[ ]:= {v1, v2, v3, v4, v5}
```

spinprojectionq

```
In[ ]:= spinprojectionq[qm_] := Module[{v1, v2, v3, v4, v5},
  wtoh4[qmattormat[qm].h4tow[{v1, v2, v3, v4, v5}].qmattormat[inverseSU11Hq[qm]]] /.
  Thread[{v1, v2, v3, v4, v5} → IdentityMatrix[5]]];
```

spinprojection

```
In[ ]:= spinprojection[rm_] :=
  Module[{v1, v2, v3, v4, v5}, wtoh4[rm.h4tow[{v1, v2, v3, v4, v5}].inverseSU11H[rm]] /.
  Thread[{v1, v2, v3, v4, v5} → IdentityMatrix[5]]];
```

reflectionlift

```
In[ ]:= reflectionlift[{v1_, v2_, v3_, v4_, v5_}] :=
  Total[MapThread[Times, {{v1, v2, v3, v4, v5}, {rm1, rm2, rm3, rm4, rm5}}]]];
```

```
In[ ]:= FullSimplify[
  Transpose[#].DiagonalMatrix[{1, 1, 1, 1, -1}].# == DiagonalMatrix[{1, 1, 1, 1, -1}] &[
    spinprojection[qmattormat[{{quaternion[a0, a1, a2, a3], quaternion[b0, b1, b2, b3]},
      {quaternion[c0, c1, c2, c3], quaternion[d0, d1, d2, d3]}}]], Assumptions →
    {Element[a0 | a1 | a2 | a3 | b0 | b1 | b2 | b3 | c0 | c1 | c2 | c3 | d0 | d1 | d2 | d3, Reals] &&
      LogicalExpand[isSU11H[qmattormat[{{quaternion[a0, a1, a2, a3], quaternion[b0, b1,
        b2, b3]}, {quaternion[c0, c1, c2, c3], quaternion[d0, d1, d2, d3]}}]]]]]
```

```
Out[ ]:= True
```

```
In[ ]:= FullSimplify[
  isSU11H[reflectionlift[{v1, v2, v3, v4, v5}].reflectionlift[{w1, w2, w3, w4, w5}]],
  Assumptions → {Element[v1 | v2 | v3 | v4 | v5 | w1 | w2 | w3 | w4 | w5, Reals],
    ldot[{v1, v2, v3, v4, v5}, {v1, v2, v3, v4, v5}] == 1 &&
    ldot[{w1, w2, w3, w4, w5}, {w1, w2, w3, w4, w5}] == 1}]
```

```
Out[ ]:= True
```

```
In[ ]:= FullSimplify[
  spinprojection[reflectionlift[{v1, v2, v3, v4, v5}]] == rmat[{v1, v2, v3, v4, v5}],
  Assumptions → {ldot[{v1, v2, v3, v4, v5}, {v1, v2, v3, v4, v5}] == 1}]
```

```
Out[ ]:= True
```

```
In[ ]:= FullSimplify[
  spinprojection[reflectionlift[{v1, v2, v3, v4, v5}].reflectionlift[{w1, w2, w3, w4, w5}]] ==
  rmat[{v1, v2, v3, v4, v5}].rmat[{w1, w2, w3, w4, w5}],
  Assumptions → {ldot[{v1, v2, v3, v4, v5}, {v1, v2, v3, v4, v5}] == 1 &&
    ldot[{w1, w2, w3, w4, w5}, {w1, w2, w3, w4, w5}] == 1}]
```

```
Out[ ]:= True
```

Factor a Lorentzian matrix as a product of reflections in planes normal to vectors.

*reflectionfactor, reflectionfactor1, reflectionfactor2, reflectionfactor3, reflectionfactor4*

```
In[ ]:= reflectionfactor[m_] :=
  If[m.{0, 0, 0, 0, 1} == {0, 0, 0, 0, 1}, reflectionfactor1[m], Prepend[reflectionfactor1[
    rmat[m.{0, 0, 0, 0, 1} - {0, 0, 0, 0, 1}].m], m.{0, 0, 0, 0, 1} - {0, 0, 0, 0, 1}]];
  reflectionfactor1[m_] := If[m.{1, 0, 0, 0, 0} == {1, 0, 0, 0, 0}, reflectionfactor2[m],
    Prepend[reflectionfactor2[rmat[m.{1, 0, 0, 0, 0} - {1, 0, 0, 0, 0}].m],
      m.{1, 0, 0, 0, 0} - {1, 0, 0, 0, 0}]];
  reflectionfactor2[m_] := If[m.{0, 1, 0, 0, 0} == {0, 1, 0, 0, 0}, reflectionfactor3[m],
    Prepend[reflectionfactor3[rmat[m.{0, 1, 0, 0, 0} - {0, 1, 0, 0, 0}].m],
      m.{0, 1, 0, 0, 0} - {0, 1, 0, 0, 0}]];
  reflectionfactor3[m_] := If[m.{0, 0, 1, 0, 0} == {0, 0, 1, 0, 0}, reflectionfactor4[m],
    Prepend[reflectionfactor4[rmat[m.{0, 0, 1, 0, 0} - {0, 0, 1, 0, 0}].m],
      m.{0, 0, 1, 0, 0} - {0, 0, 1, 0, 0}]];
  reflectionfactor4[m_] := If[m.{0, 0, 0, 1, 0} == {0, 0, 0, 1, 0},
    {}, {m.{0, 0, 0, 1, 0} - {0, 0, 0, 1, 0}}];
```

*reflectvectorseq*

```
In[ ]:= reflectvectorseq[s_] := Apply[Dot, Append[Map[rmat, s], IdentityMatrix[5]]];
```

*spinvectorseq*

```
In[ ]:= spinvectorseq[s_] := Apply[Dot, Append[Map[reflectionlift, s], IdentityMatrix[8]]];
```

spinlift

```
In[ ]:= spinlift[m_] := # / Det[#]^(1/8) &[spinvectorseq[reflectionfactor[m]]];
```

## Q[tau] etc.

tau

```
In[ ]:= tau = (1 + Sqrt[5]) / 2;
```

toQtau

```
In[ ]:= toQtau[x_] := ToNumberField[x, tau];
```

toQroot5

```
In[ ]:= toQroot5[x_] := ToNumberField[x, Sqrt[5]];
```

kappa

```
In[ ]:= kappa = FullSimplify[Sqrt[1 + 3 tau]]
```

$$\text{Out[ ]} = \sqrt{\frac{1}{2} (5 + 3 \sqrt{5})}$$

```
In[ ]:= MinimalPolynomial[kappa, t]
```

$$\text{Out[ ]} = -5 - 5 t^2 + t^4$$

toQkappa

```
In[ ]:= toQkappa[x_] := ToNumberField[x, kappa];
```

```
In[ ]:= toQkappa[kappa]
```

$$\text{Out[ ]} = \sqrt{2.42\dots}$$

```
In[ ]:= Clear[formatkappa]
```

formatkappa

```
In[ ]:= formatkappa[x_] :=  
  toQkappa[x] /. {AlgebraicNumber[Root[-5 - 5 #1^2 + #1^4 &, 2], {a1_, a2_, a3_, a4_}] :>  
    Collect[a1 + a2 * κ + a3 * (1 + 3 τ) + a4 * (1 + 3 τ) * κ, {κ, τ}]}
```

fromformatkapparule

```
In[ ]:= fromformatkapparule = {κ → Sqrt[1 + 3 tau], τ → tau};
```

## 5335 simplex

gm5335

```
In[ ]:= MatrixForm[formatkappa[gm5335 = toQkappa[{{1, -tau/2, 0, 0, 0}, {-tau/2, 1, -1/2, 0, 0},  
  {0, -1/2, 1, -1/2, 0}, {0, 0, -1/2, 1, -tau/2}, {0, 0, 0, -tau/2, 1}}]]]
```

Out[ ]//MatrixForm=

$$\begin{pmatrix} 1 & -\frac{\tau}{2} & 0 & 0 & 0 \\ -\frac{\tau}{2} & 1 & -\frac{1}{2} & 0 & 0 \\ 0 & -\frac{1}{2} & 1 & -\frac{1}{2} & 0 \\ 0 & 0 & -\frac{1}{2} & 1 & -\frac{\tau}{2} \\ 0 & 0 & 0 & -\frac{\tau}{2} & 1 \end{pmatrix}$$

```
In[ ]:= diagram[FullSimplify[Pi / ArcCos[-gm5335]]]
```

```
Out[ ]:= 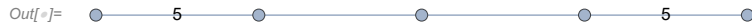
```

*nv5335*

```
In[ ]:= TableForm[formatkappa[nv5335 = toQkappa[{
  {0, 0, 0, -1, 0},
  {0, -(tau - 1) / 2, 1 / 2, tau / 2, 0},
  {0, 0, -1, 0, 0},
  {-(tau - 1) / 2, tau / 2, 1 / 2, 0, 0},
  {(tau + 1), 0, 0, 0, Sqrt[1 + 3 tau]} }]]]
```

*Out[ ]//TableForm=*

|                                |                                |               |                  |          |
|--------------------------------|--------------------------------|---------------|------------------|----------|
| 0                              | 0                              | 0             | -1               | 0        |
| 0                              | $\frac{1}{2} - \frac{\tau}{2}$ | $\frac{1}{2}$ | $\frac{\tau}{2}$ | 0        |
| 0                              | 0                              | -1            | 0                | 0        |
| $\frac{1}{2} - \frac{\tau}{2}$ | $\frac{\tau}{2}$               | $\frac{1}{2}$ | 0                | 0        |
| $1 + \tau$                     | 0                              | 0             | 0                | $\kappa$ |

```
In[ ]:= FullSimplify[Outer[ldot, nv5335, nv5335, 1] == gm5335]
```

```
Out[ ]:= True
```

*verts5335*

```
In[ ]:= TableForm[
  formatkappa[verts5335 = toQkappa[Map[Function[i, FullSimplify[{x1, x2, x3, x4, x5} /.
    Solve[Apply[And, Map[ldot[{x1, x2, x3, x4, x5}, #] == 0 &,
      nv5335[[Complement[Range[5], {i}]]]]]] && ldot[{x1, x2, x3, x4, x5},
      {x1, x2, x3, x4, x5}] == -1 && x5 > 0, {x1, x2, x3, x4, x5}][[1]]]], Range[5]]]]]
```

*Out[ ]//TableForm=*

|                       |                                                      |                                                    |          |              |
|-----------------------|------------------------------------------------------|----------------------------------------------------|----------|--------------|
| $\kappa (2 + 3 \tau)$ | $\kappa (1 + \tau)$                                  | 0                                                  | $\kappa$ | $5 + 8 \tau$ |
| $\kappa (1 + \tau)$   | $\kappa$                                             | 0                                                  | 0        | $2 + 3 \tau$ |
| $\kappa \tau$         | $\kappa \left(-\frac{1}{5} + \frac{2\tau}{5}\right)$ | $\kappa \left(\frac{3}{5} - \frac{\tau}{5}\right)$ | 0        | $1 + 2 \tau$ |
| $\kappa$              | 0                                                    | 0                                                  | 0        | $1 + \tau$   |
| 0                     | 0                                                    | 0                                                  | 0        | 1            |

*gen5335*

```
In[ ]:= gen5335 = Map[rmat, nv5335];
```



```
In[ ]:= Map[MatrixForm[formatkappa[#]] &, gen5335]
```

$$\text{Out[ ]} = \left\{ \begin{pmatrix} 1 & 0 & 0 & 0 & 0 \\ 0 & 1 & 0 & 0 & 0 \\ 0 & 0 & 1 & 0 & 0 \\ 0 & 0 & 0 & -1 & 0 \\ 0 & 0 & 0 & 0 & 1 \end{pmatrix}, \begin{pmatrix} 1 & 0 & 0 & 0 & 0 \\ 0 & \frac{\tau}{2} & -\frac{1}{2} + \frac{\tau}{2} & \frac{1}{2} & 0 \\ 0 & -\frac{1}{2} + \frac{\tau}{2} & \frac{1}{2} & -\frac{\tau}{2} & 0 \\ 0 & \frac{1}{2} & -\frac{\tau}{2} & \frac{1}{2} - \frac{\tau}{2} & 0 \\ 0 & 0 & 0 & 0 & 1 \end{pmatrix}, \begin{pmatrix} 1 & 0 & 0 & 0 & 0 \\ 0 & 1 & 0 & 0 & 0 \\ 0 & 0 & -1 & 0 & 0 \\ 0 & 0 & 0 & 1 & 0 \\ 0 & 0 & 0 & 0 & 1 \end{pmatrix}, \right.$$

$$\left. \begin{pmatrix} \frac{\tau}{2} & \frac{1}{2} & -\frac{1}{2} + \frac{\tau}{2} & 0 & 0 \\ \frac{1}{2} & \frac{1}{2} - \frac{\tau}{2} & -\frac{\tau}{2} & 0 & 0 \\ -\frac{1}{2} + \frac{\tau}{2} & -\frac{\tau}{2} & \frac{1}{2} & 0 & 0 \\ 0 & 0 & 0 & 1 & 0 \\ 0 & 0 & 0 & 0 & 1 \end{pmatrix}, \begin{pmatrix} -3 - 6\tau & 0 & 0 & 0 & \kappa(2 + 2\tau) \\ 0 & 1 & 0 & 0 & 0 \\ 0 & 0 & 1 & 0 & 0 \\ 0 & 0 & 0 & 1 & 0 \\ \kappa(-2 - 2\tau) & 0 & 0 & 0 & 3 + 6\tau \end{pmatrix} \right\}$$

```
insideoutmat
```

```
In[ ]:= MatrixForm[
  formatkappa[insideoutmat = Transpose[Reverse[verts5335]].Inverse[Transpose[verts5335]]]]
```

```
Out[ ]//MatrixForm=
```

$$\begin{pmatrix} -4 - 7\tau & -1 - 3\tau & 0 & -1 - \tau & \kappa(2 + 3\tau) \\ -1 - 3\tau & -1 - \tau & 0 & 0 & \kappa(1 + \tau) \\ 0 & 0 & 1 & 0 & 0 \\ -1 - \tau & 0 & 0 & 0 & \kappa \\ \kappa(-2 - 3\tau) & \kappa(-1 - \tau) & 0 & -\kappa & 5 + 8\tau \end{pmatrix}$$

```
In[ ]:= Det[insideoutmat]
```

```
Out[ ]:= 1
```

```
relators5335
```

```
In[ ]:= relators5335 = {gen[1].gen[1], gen[2].gen[2], gen[3].gen[3], gen[4].gen[4], gen[5].gen[5],
  gen[1].gen[2].gen[1].gen[2].gen[1].gen[2].gen[1].gen[2].gen[1].gen[2],
  gen[1].gen[3].gen[1].gen[3], gen[1].gen[4].gen[1].gen[4],
  gen[1].gen[5].gen[1].gen[5], gen[2].gen[3].gen[2].gen[3].gen[2].gen[3],
  gen[2].gen[4].gen[2].gen[4], gen[2].gen[5].gen[2].gen[5],
  gen[3].gen[4].gen[3].gen[4].gen[3].gen[4], gen[3].gen[5].gen[3].gen[5],
  gen[4].gen[5].gen[4].gen[5].gen[4].gen[5].gen[4].gen[5].gen[4].gen[5]};
```

```
In[ ]:= Union[relators5335 /. {gen[i_] => gen5335[[i]]}] == {IdentityMatrix[5]}
```

```
Out[ ]:= True
```

```
gen5335i
```

```
In[ ]:= gen5335i = Append[gen5335, insideoutmat];
```

```
relators5335i
```

```
In[ ]:= relators5335i = Join[relators5335, {gen[6].gen[6], gen[6].gen[1].gen[6].gen[5],
  gen[6].gen[2].gen[6].gen[4], gen[6].gen[3].gen[6].gen[3],
  gen[6].gen[4].gen[6].gen[2], gen[6].gen[5].gen[6].gen[1]}];
```

```
In[ ]:= Union[relators5335i /. {gen[i_] => gen5335i[[i]]}] == {IdentityMatrix[5]}
```

```
Out[ ]:= True
```

gen533

```
In[ ]:= gen533 = Take[gen5335, 4];
```

relators533

```
In[ ]:= relators533 = Select[relators5335, FreeQ[#, gen[5]] &]
```

```
Out[ ]:= {gen[1].gen[1], gen[2].gen[2], gen[3].gen[3], gen[4].gen[4],
  gen[1].gen[2].gen[1].gen[2].gen[1].gen[2].gen[1].gen[2].gen[1].gen[2],
  gen[1].gen[3].gen[1].gen[3], gen[1].gen[4].gen[1].gen[4],
  gen[2].gen[3].gen[2].gen[3].gen[2].gen[3],
  gen[2].gen[4].gen[2].gen[4], gen[3].gen[4].gen[3].gen[4].gen[3].gen[4]}
```

```
In[ ]:= Union[relators533 /. {gen[i_] -> gen533[[i]]}] == {IdentityMatrix[5]}
```

```
Out[ ]:= True
```

genop5335

```
In[ ]:= Map[MatrixForm[formatkappa[#]] &, genop5335 = Map[gen5335[[1]].# &, gen5335[[2 ;; -1]]]]
```

$$\text{Out[ ]} = \left\{ \begin{pmatrix} 1 & 0 & 0 & 0 & 0 \\ 0 & \frac{\tau}{2} & -\frac{1}{2} + \frac{\tau}{2} & \frac{1}{2} & 0 \\ 0 & -\frac{1}{2} + \frac{\tau}{2} & \frac{1}{2} & -\frac{\tau}{2} & 0 \\ 0 & -\frac{1}{2} & \frac{\tau}{2} & -\frac{1}{2} + \frac{\tau}{2} & 0 \\ 0 & 0 & 0 & 0 & 1 \end{pmatrix}, \begin{pmatrix} 1 & 0 & 0 & 0 & 0 \\ 0 & 1 & 0 & 0 & 0 \\ 0 & 0 & -1 & 0 & 0 \\ 0 & 0 & 0 & -1 & 0 \\ 0 & 0 & 0 & 0 & 1 \end{pmatrix}, \right.$$

$$\left. \begin{pmatrix} \frac{\tau}{2} & \frac{1}{2} & -\frac{1}{2} + \frac{\tau}{2} & 0 & 0 \\ \frac{1}{2} & \frac{1}{2} - \frac{\tau}{2} & -\frac{\tau}{2} & 0 & 0 \\ -\frac{1}{2} + \frac{\tau}{2} & -\frac{\tau}{2} & \frac{1}{2} & 0 & 0 \\ 0 & 0 & 0 & -1 & 0 \\ 0 & 0 & 0 & 0 & 1 \end{pmatrix}, \begin{pmatrix} -3 - 6\tau & 0 & 0 & 0 & \kappa(2 + 2\tau) \\ 0 & 1 & 0 & 0 & 0 \\ 0 & 0 & 1 & 0 & 0 \\ 0 & 0 & 0 & -1 & 0 \\ \kappa(-2 - 2\tau) & 0 & 0 & 0 & 3 + 6\tau \end{pmatrix} \right\}$$

```
In[ ]:= Map[Det, genop5335]
```

```
Out[ ]:= {1, 1, 1, 1}
```

relatorsop5335

```
In[ ]:= relatorsop5335 = {gen[1].gen[1].gen[1].gen[1].gen[1], gen[2].gen[2], gen[3].gen[3],
  gen[4].gen[4], Inverse[gen[1]].gen[2].Inverse[gen[1]].gen[2].Inverse[gen[1]].gen[2],
  Inverse[gen[1]].gen[3].Inverse[gen[1]].gen[3],
  Inverse[gen[1]].gen[4].Inverse[gen[1]].gen[4],
  Inverse[gen[2]].gen[3].Inverse[gen[2]].gen[3].Inverse[gen[2]].gen[3],
  Inverse[gen[2]].gen[4].Inverse[gen[2]].gen[4],
  Inverse[gen[3]].gen[4].Inverse[gen[3]].gen[4].Inverse[gen[3]].
  gen[4].Inverse[gen[3]].gen[4].Inverse[gen[3]].gen[4]};
```

```
In[ ]:= Union[relatorsop5335 /. {gen[i_] -> genop5335[[i]]}] == {IdentityMatrix[5]}
```

```
Out[ ]:= True
```

genop533

```
In[ ]:= genop533 = Take[genop5335, 3];
```

relatorsop533

```
In[ ]:= relatorsop533 = Select[relatorsop5335, FreeQ[#, gen[4]] &];
```

```
In[ ]:= Union[relatorsop533 /. {gen[i_] => genop533[[i]]}] == {IdentityMatrix[5]}
```

```
Out[ ]:= True
```

Lift the generators of the orientation preserving symmetries of the 120-cell to  $8 \times 8$  real matrix representation of spin. View as quaternion matrices. They don't satisfy the relators so the o.p. symmetries group does not lift to spin.

```
genop5335lift
```

```
In[ ]:= Map[MatrixForm[rmattoqmat[formatkappa[#]]] &,
  genop5335lift = toQkappa[Map[spinlift, genop5335]]]
```

```
Out[ ]:= {  $\begin{pmatrix} -\frac{i}{2} + j \left( \frac{1}{2} - \frac{\tau}{2} \right) - \frac{\tau}{2} & 0 \\ 0 & -\frac{i}{2} + j \left( \frac{1}{2} - \frac{\tau}{2} \right) - \frac{\tau}{2} \end{pmatrix}, \begin{pmatrix} i & 0 \\ 0 & i \end{pmatrix},$ 
 $\begin{pmatrix} -\frac{i}{2} + k \left( -\frac{1}{2} + \frac{\tau}{2} \right) + \frac{j\tau}{2} & 0 \\ 0 & -\frac{i}{2} + k \left( \frac{1}{2} - \frac{\tau}{2} \right) + \frac{j\tau}{2} \end{pmatrix}, \begin{pmatrix} k(-1-\tau) & -k\kappa \\ k\kappa & k(1+\tau) \end{pmatrix} \}$ 
```

```
genop533lift
```

```
In[ ]:= genop533lift = Take[genop5335lift, 3];
```

```
In[ ]:= Map[Det, genop5335lift]
```

```
Out[ ]:= {1, 1, 1, 1}
```

```
In[ ]:= Map[spinprojection, genop5335lift] == genop5335
```

```
Out[ ]:= True
```

```
In[ ]:= Union[relatorsop533 /. {gen[i_] => genop533lift[[i]]}] == {IdentityMatrix[8]}
```

```
Out[ ]:= False
```

```
In[ ]:= Union[relatorsop533 /. {gen[i_] => genop533lift[[i]]}] ==
  {-IdentityMatrix[8], IdentityMatrix[8]}
```

```
Out[ ]:= True
```

```
In[ ]:= Union[relatorsop5335 /. {gen[i_] => genop5335lift[[i]]}] == {IdentityMatrix[8]}
```

```
Out[ ]:= False
```

```
In[ ]:= Union[relatorsop5335 /. {gen[i_] => genop5335lift[[i]]}] ==
  {-IdentityMatrix[8], IdentityMatrix[8]}
```

```
Out[ ]:= True
```

```
In[ ]:= Map[Mod[Total[#], 2] &,
  relatorsop533 /. {Inverse[x_] => x, Dot -> List} /. {gen[i_] => IdentityMatrix[4][[i]]}]
```

```
Out[ ]:= {{1, 0, 0, 0}, {0, 0, 0, 0}, {0, 0, 0, 0}, {1, 1, 0, 0}, {0, 0, 0, 0}, {0, 1, 1, 0}}
```

```
In[ ]:= relatorsop533 /. {gen[i_] => genop533lift[[i]]} /.
  {-IdentityMatrix[8] -> 1, IdentityMatrix[8] -> 0}
```

```
Out[ ]:= {0, 1, 1, 0, 1, 0}
```

```
In[ ]:= LinearSolve[%%, %, Modulus -> 2]
```

... LinearSolve: Linear equation encountered that has no solution.

```
Out[ ]:= LinearSolve[{ {1, 0, 0, 0}, {0, 0, 0, 0}, {0, 0, 0, 0}, {1, 1, 0, 0}, {0, 0, 0, 0}, {0, 1, 1, 0}},
  {0, 1, 1, 0, 1, 0}, Modulus -> 2]
```

```
In[ ]:= Map[Mod[Total[#, 2] &,
  relatorsop5335 /. {Inverse[x_] -> x, Dot -> List} /. {gen[i_] -> IdentityMatrix[4][[i]]}]
```

```
Out[ ]:= {{1, 0, 0, 0}, {0, 0, 0, 0}, {0, 0, 0, 0}, {0, 0, 0, 0}, {1, 1, 0, 0},
  {0, 0, 0, 0}, {0, 0, 0, 0}, {0, 1, 1, 0}, {0, 0, 0, 0}, {0, 0, 1, 1}}
```

```
In[ ]:= relatorsop5335 /. {gen[i_] -> genop5335lift[[i]]} /.
  {-IdentityMatrix[8] -> 1, IdentityMatrix[8] -> 0}
```

```
Out[ ]:= {0, 1, 1, 1, 0, 1, 1, 0, 1, 0}
```

```
In[ ]:= LinearSolve[%%, %, Modulus -> 2]
```

... LinearSolve: Linear equation encountered that has no solution.

```
Out[ ]:= LinearSolve[{ {1, 0, 0, 0}, {0, 0, 0, 0}, {0, 0, 0, 0}, {0, 0, 0, 0},
  {1, 1, 0, 0}, {0, 0, 0, 0}, {0, 0, 0, 0}, {0, 1, 1, 0}, {0, 0, 0, 0}, {0, 0, 1, 1}},
  {0, 1, 1, 1, 0, 1, 1, 0, 1, 0}, Modulus -> 2]
```

insideoutmatlift

```
In[ ]:= insideoutmatlift =
  ToNumberField[#2, #1[{-1, 1}]] & [ToNumberField[Union[Flatten[#]]], #] & [
  spinlift[insideoutmat]];
```

```
In[ ]:= insideoutmatlift
```

```
Out[ ]:= {{0, -2.49..., 0.951..., 1.54..., -0.636..., -2.30..., 0, 1.67...},
  {2.49..., 0, -1.54..., 0.951..., 2.30..., -0.636..., -1.67..., 0},
  {-0.951..., 1.54..., 0, 2.49..., 0, 1.67..., -0.636..., 2.30...},
  {-1.54..., -0.951..., -2.49..., 0, -1.67..., 0, -2.30..., -0.636...},
  {-0.636..., 2.30..., 0, -1.67..., 0, 2.49..., 0.951..., -1.54...},
  {-2.30..., -0.636..., 1.67..., 0, -2.49..., 0, 1.54..., 0.951...},
  {0, -1.67..., -0.636..., -2.30..., -0.951..., -1.54..., 0, -2.49...},
  {1.67..., 0, 2.30..., -0.636..., 1.54..., -0.951..., 2.49..., 0}}
```

```
In[ ]:= Sqrt[formatkappa[tau - 1]] / 2 *
  MatrixForm[rmattoqmat[formatkappa[insideoutmatlift / (Sqrt[tau - 1] / 2)]]]
```

```
Out[ ]:= 
$$\frac{1}{2} \sqrt{-1 + \tau} \begin{pmatrix} j \kappa - k \kappa \tau + i \kappa (1 + \tau) & k (-1 - 2 \tau) - \tau + i (1 + 3 \tau) \\ i (-1 - 3 \tau) - \tau + k (1 + 2 \tau) & j \kappa + i \kappa (-1 - \tau) + k \kappa \tau \end{pmatrix}$$

```

```
In[ ]:= insideoutmatlift.insideoutmatlift
```

```
Out[ ]:= {{-1, 0, 0, 0, 0, 0, 0, 0}, {0, -1, 0, 0, 0, 0, 0, 0},
          {0, 0, -1, 0, 0, 0, 0, 0}, {0, 0, 0, -1, 0, 0, 0, 0}, {0, 0, 0, 0, -1, 0, 0, 0},
          {0, 0, 0, 0, 0, -1, 0, 0}, {0, 0, 0, 0, 0, 0, -1, 0}, {0, 0, 0, 0, 0, 0, 0, -1}}
```

```
In[ ]:= insideoutmatlift.insideoutmatlift.insideoutmatlift.insideoutmatlift
```

```
Out[ ]:= {{1, 0, 0, 0, 0, 0, 0, 0}, {0, 1, 0, 0, 0, 0, 0, 0},
          {0, 0, 1, 0, 0, 0, 0, 0}, {0, 0, 0, 1, 0, 0, 0, 0}, {0, 0, 0, 0, 1, 0, 0, 0},
          {0, 0, 0, 0, 0, 1, 0, 0}, {0, 0, 0, 0, 0, 0, 1, 0}, {0, 0, 0, 0, 0, 0, 0, 1}}
```

```
In[ ]:= Det[insideoutmatlift]
```

```
Out[ ]:= 1
```

```
In[ ]:= toQkappa[spinprojection[insideoutmatlift]] == insideoutmat
```

```
Out[ ]:= True
```

```
In[ ]:= rmattoqmat[insideoutmatlift] // MatrixForm
```

```
Out[ ]//MatrixForm=
```

$$\begin{pmatrix} i \sqrt{2.49...} + j \sqrt{0.951...} + k \sqrt{-1.54...} & k \sqrt{-1.67...} + \sqrt{-0.636...} + i \sqrt{2.30...} \\ i \sqrt{-2.30...} + \sqrt{-0.636...} + k \sqrt{1.67...} & k \sqrt{1.54...} + j \sqrt{0.951...} + i \sqrt{-2.49...} \end{pmatrix}$$

```
grp533
```

```
In[ ]:= AbsoluteTiming[Dimensions[grp533 = sggen[gen533]]]
```

```
Out[ ]:= {19.0896, {14400, 5, 5}}
```

```
grp533
```

```
In[ ]:= AbsoluteTiming[Dimensions[grp533 = sggen[gen533]]]
```

```
Out[ ]:= {8.42038, {7200, 5, 5}}
```

```
grp533lift
```

```
In[ ]:= AbsoluteTiming[Dimensions[grp533lift = sggen[gen533lift]]]
```

```
Out[ ]:= {45.4641, {14400, 8, 8}}
```

## Symmetry group of 120-cell

```
In[ ]:= Dimensions[gen533]
```

```
Out[ ]:= {4, 5, 5}
```

```
symgrp
```

```
In[ ]:= AbsoluteTiming[symgrp = sggen[gen533];]
```

```
Out[ ]:= {18.7718, Null}
```

```
In[ ]:= Dimensions[symgrp]
```

```
Out[ ]:= {14400, 5, 5}
```

```
In[ ]:= Union[Flatten[symgrp]]
```

```
Out[ ]:= { -1, -1/2, 0, 1/2, 1, 0.309..., 0.809..., -0.809..., -0.309... }
```

We identify a useful subgroup of the symmetry group.

*signmats*

```
In[ ]:= signmats = Map[DiagonalMatrix[Append[#, 1]] &, Distribute[Table[{-1, 1}, {4}], List, List]];
```

```
In[ ]:= Dimensions[signmats]
```

```
Out[ ]:= {16, 5, 5}
```

*evenperms*

```
In[ ]:= evenperms = Map[Append[#, 5] &, Select[Permutations[Range[4]], Signature[#] == 1 &]];
```

*permsignmats*

```
In[ ]:= permsignmats = Apply[Union, Map[Function[m, Map[m[#]] &, evenperms]], signmats]];
```

```
In[ ]:= Dimensions[permsignmats]
```

```
Out[ ]:= {192, 5, 5}
```

## 120-cell

```
In[ ]:= verts5335[[4]]
```

```
Out[ ]:= {2.42..., 0, 0, 0, 2.62...}
```

*v4orbitpre*

```
In[ ]:= AbsoluteTiming[
  v4orbitpre = SortBy[Union[Map[#.verts5335[[4]] &, symgrp]], Round[N[# * 10^6]] &];]
```

```
Out[ ]:= {1.09312, Null}
```

```
In[ ]:= Dimensions[v4orbitpre]
```

```
Out[ ]:= {120, 5}
```

*v3orbit*

```
In[ ]:= AbsoluteTiming[
  v3orbit = SortBy[Union[Map[#.verts5335[[3]] &, symgrp]], Round[N[# * 10^6]] &];]
```

```
Out[ ]:= {2.97167, Null}
```

```
In[ ]:= Dimensions[v3orbit]
```

```
Out[ ]:= {720, 5}
```

*v2orbit*

```
In[ ]:= AbsoluteTiming[
  v2orbit = SortBy[Union[Map[#.verts5335[[2]] &, symgrp]], Round[N[# * 10^6]] &];]
```

```
Out[ ]:= {1.78965, Null}
```

```
In[ ]:= Dimensions[v2orbit]
```

```
Out[ ]:= {1200, 5}
```

v1orbit

```
In[ ]:= AbsoluteTiming[
  v1orbit = SortBy[Union[Map[#.verts5335[[1]] &, symgrp]], Round[N[# * 10^6]] &];]
```

```
Out[ ]:= {2.63199, Null}
```

```
In[ ]:= Dimensions[v1orbit]
```

```
Out[ ]:= {600, 5}
```

v4entrylist

```
In[ ]:= v4entrylist = Union[Flatten[v4orbitpre]]
```

```
Out[ ]:= {0, -2.42..., 0.748..., -1.21..., 1.96...,
  -1.96..., 1.21..., -0.748..., 2.42..., 2.62...}
```

v4entrylistt

```
In[ ]:= v4entrylistt = {0, 1 +  $\tau$ , -Sqrt[1 + 3  $\tau$ ], -1 / 2 * Sqrt[1 + 3  $\tau$ ],
  1 / 2 * Sqrt[1 + 3  $\tau$ ], Sqrt[1 + 3  $\tau$ ], -1 / 2 * (-1 +  $\tau$ ) * Sqrt[1 + 3  $\tau$ ],
  1 / 2 * (-1 +  $\tau$ ) * Sqrt[1 + 3  $\tau$ ], -1 / 2 *  $\tau$  * Sqrt[1 + 3  $\tau$ ], 1 / 2 *  $\tau$  * Sqrt[1 + 3  $\tau$ ]}
```

```
Out[ ]:= {0, 1 +  $\tau$ , - $\sqrt{1 + 3 \tau}$ , - $\frac{1}{2} \sqrt{1 + 3 \tau}$ ,  $\frac{1}{2} \sqrt{1 + 3 \tau}$ ,  $\sqrt{1 + 3 \tau}$ ,
  - $\frac{1}{2} (-1 + \tau) \sqrt{1 + 3 \tau}$ ,  $\frac{1}{2} (-1 + \tau) \sqrt{1 + 3 \tau}$ , - $\frac{1}{2} \tau \sqrt{1 + 3 \tau}$ ,  $\frac{1}{2} \tau \sqrt{1 + 3 \tau}$ }
```

```
In[ ]:= v4entrylist == Union[Map[toQkappa, v4entrylistt /. { $\tau \rightarrow \text{tau}$ }]]
```

```
Out[ ]:= True
```

```
In[ ]:= Sort[v4entrylistt]
```

```
Out[ ]:= {0, 1 +  $\tau$ , - $\sqrt{1 + 3 \tau}$ , - $\frac{1}{2} \sqrt{1 + 3 \tau}$ ,  $\frac{1}{2} \sqrt{1 + 3 \tau}$ ,  $\sqrt{1 + 3 \tau}$ ,
  - $\frac{1}{2} (-1 + \tau) \sqrt{1 + 3 \tau}$ ,  $\frac{1}{2} (-1 + \tau) \sqrt{1 + 3 \tau}$ , - $\frac{1}{2} \tau \sqrt{1 + 3 \tau}$ ,  $\frac{1}{2} \tau \sqrt{1 + 3 \tau}$ }
```

v4orbit

```
In[ ]:= v4orbit = Apply[Join, {#[[1]], Reverse[#[[2]]]} &[
  Transpose[SortBy[Union[Map[SortBy[{#, DiagonalMatrix[{-1, -1, -1, -1, 1}].#],
    Round[N[# * 10^6]] &] &, v4orbitpre]], Round[N[# * 10^6]] &]]];]
```

```
In[ ]:= Dimensions[v4orbit]
```

```
Out[ ]:= {120, 5}
```

v4indrules

```
In[ ]:= v4indrules = Thread[v4orbit → Range[Length[v4orbit]]];
```

v3indrules

```
In[ ]:= v3indrules = Thread[v3orbit → Range[Length[v3orbit]]];
```

v2indrules

```
In[ ]:= v2indrules = Thread[v2orbit → Range[Length[v2orbit]]];
```

*v1indrul*

```
In[ ]:= v1indrul = Thread[v1orbit → Range[Length[v1orbit]]];
```

*ind3by4*

```
In[ ]:= Dimensions[ind3by4 =
  Union[Map[{#.verts5335[[3]] /. v3indrul, #.verts5335[[4]] /. v4indrul} &, symgrp]]]
```

```
Out[ ]:= {1440, 2}
```

*ind3to4*

```
In[ ]:= Dimensions[ind3to4 = Partition[ind3by4, 2][[All, All, 2]]]
```

```
Out[ ]:= {720, 2}
```

*ind4to3*

```
In[ ]:= Dimensions[ind4to3 = Partition[Sort[Map[Reverse, ind3by4]], 12][[All, All, 2]]]
```

```
Out[ ]:= {120, 12}
```

*ind2by4*

```
In[ ]:= Dimensions[ind2by4 =
  Union[Map[{#.verts5335[[2]] /. v2indrul, #.verts5335[[4]] /. v4indrul} &, symgrp]]]
```

```
Out[ ]:= {3600, 2}
```

*ind2to4*

```
In[ ]:= Dimensions[ind2to4 = Partition[ind2by4, 3][[All, All, 2]]]
```

```
Out[ ]:= {1200, 3}
```

*ind4to2*

```
In[ ]:= Dimensions[ind4to2 = Partition[Sort[Map[Reverse, ind2by4]], 30][[All, All, 2]]]
```

```
Out[ ]:= {120, 30}
```

*ind2by3*

```
In[ ]:= Dimensions[ind2by3 =
  Union[Map[{#.verts5335[[2]] /. v2indrul, #.verts5335[[3]] /. v3indrul} &, symgrp]]]
```

```
Out[ ]:= {3600, 2}
```

*ind2to3*

```
In[ ]:= Dimensions[ind2to3 = Partition[ind2by3, 3][[All, All, 2]]]
```

```
Out[ ]:= {1200, 3}
```

*ind3to2*

```
In[ ]:= Dimensions[ind3to2 = Partition[Sort[Map[Reverse, ind2by3]], 5][[All, All, 2]]]
```

```
Out[ ]:= {720, 5}
```

*ind1by4*

```
In[ ]:= Dimensions[ind1by4 =
  Union[Map[{#.verts5335[[1]] /. v1indrul, #.verts5335[[4]] /. v4indrul} &, symgrp]]]
```

```
Out[ ]:= {2400, 2}
```

*ind1to4*

```
In[ ]:= Dimensions[ind1to4 = Partition[ind1by4, 4][[All, All, 2]]]
```

```
Out[ ]:= {600, 4}
```



ind4to1

```
In[ ]:= Dimensions[ind4to1 = Partition[Sort[Map[Reverse, ind1by4]], 20] [[All, All, 2]]]
```

```
Out[ ]:= {120, 20}
```

ind1by3

```
In[ ]:= Dimensions[ind1by3 =  
  Union[Map[{#.verts5335[[1]] /. v1indrules, #.verts5335[[3]] /. v3indrules} &, symgrp]]]
```

```
Out[ ]:= {3600, 2}
```

```
In[ ]:= Sort[Map[Reverse, ind1by3]] [[Range[20]]]
```

```
Out[ ]:= {{1, 1}, {1, 2}, {1, 3}, {1, 4}, {1, 7}, {2, 1}, {2, 2}, {2, 5}, {2, 6}, {2, 8},  
  {3, 1}, {3, 3}, {3, 5}, {3, 9}, {3, 11}, {4, 2}, {4, 4}, {4, 6}, {4, 10}, {4, 12}}
```

ind1to3

```
In[ ]:= Dimensions[ind1to3 = Partition[ind1by3, 6] [[All, All, 2]]]
```

```
Out[ ]:= {600, 6}
```

ind3to1

```
In[ ]:= Dimensions[ind3to1 = Partition[Sort[Map[Reverse, ind1by3]], 5] [[All, All, 2]]]
```

```
Out[ ]:= {720, 5}
```

ind1by2

```
In[ ]:= Dimensions[ind1by2 =  
  Union[Map[{#.verts5335[[1]] /. v1indrules, #.verts5335[[2]] /. v2indrules} &, symgrp]]]
```

```
Out[ ]:= {2400, 2}
```

ind1to2

```
In[ ]:= Dimensions[ind1to2 = Partition[ind1by2, 4] [[All, All, 2]]]
```

```
Out[ ]:= {600, 4}
```

ind2to1

```
In[ ]:= Dimensions[ind2to1 = Partition[Sort[Map[Reverse, ind1by2]], 2] [[All, All, 2]]]
```

```
Out[ ]:= {1200, 2}
```

```
In[ ]:= nv5335[[5]]
```

```
Out[ ]:= {2.62..., 0, 0, 0, 2.42...}
```

```
In[ ]:= gen5335[[5]].verts5335[[5]] - verts5335[[5]]
```

```
Out[ ]:= {12.7..., 0, 0, 0, 11.7...}
```

```
In[ ]:= %[[{1, -1}]] / %[[{1, -1}]]
```

```
Out[ ]:= {0.207..., 0.207...}
```

```
In[ ]:= nv5335[[5]]
```

```
Out[ ]:= {2.62..., 0, 0, 0, 2.42...}
```

```
In[ ]:= verts5335[ [4] ]
```

```
Out[ ]:= { 2.42..., 0, 0, 0, 2.62... }
```

```
In[ ]:= %%[ [ {1, -1} ] ] / %%[ [ {1, -1} ] ]
```

```
Out[ ]:= { 1.08..., 0.924... }
```

*s5points*

```
In[ ]:= s5points = Map[ Function[ c, Append[ nv5335[ [5, 1] ] / verts5335[ [4, 1] ] * c[ [1 ;; 4] ],  
  nv5335[ [5, 5] ] / verts5335[ [4, 5] ] * c[ [5] ] ] ], v4orbit];
```

```
In[ ]:= Apply[ And, Map[ rmat[ s5points[ [#] ] ].v4orbit[ [#] ] == v4orbit[ [#] ] &, Range[120] ] ]
```

```
Out[ ]:= True
```

```
In[ ]:= Apply[ And, Map[ ldot[ s5points[ [#] ], v4orbit[ [#] ] ] == 0 &, Range[120] ] ]
```

```
Out[ ]:= True
```

*antipodalindex*

```
In[ ]:= antipodalindex =  
  Map[ Position[ s5points, DiagonalMatrix[ {-1, -1, -1, -1, 1} ].# ] [ [1, 1] ] &, s5points];
```

```
In[ ]:= antipodalindex == 121 - Range[120]
```

```
Out[ ]:= True
```

## Davis manifold

*davisspmat*

```
In[ ]:= AbsoluteTiming[ davisspmat =  
  Map[ rmat[ s5points[ [#] ] - s5points[ [ antipodalindex[ [#] ] ] ] ].rmat[ s5points[ [#] ] ] &,  
  Range[120] ] ];
```

```
Out[ ]:= { 0.238731, Null }
```

```
In[ ]:= Dimensions[ davisspmat ]
```

```
Out[ ]:= { 120, 5, 5 }
```

```
In[ ]:= Apply[ And, Map[  
  davisspmat[ [ antipodalindex[ [#] ] ] ].davisspmat[ [#] ] == IdentityMatrix[5] &, Range[120] ] ]
```

```
Out[ ]:= True
```

*ind3by4sp*

```
In[ ]:= Timing[ ind3by4sp =  
  Map[ Function[ rfp, { rfp[ [1] ], Complement[ ind3to4[ [ rfp[ [1] ] ] ], { rfp[ [2] ] } ] [ [1] ] ] ],  
  Map[ Function[ rfp, { davisspmat[ [ rfp[ [2] ] ] ].v3orbit[ [ rfp[ [1] ] ] ] /. v3indrules,  
    davisspmat[ [ rfp[ [2] ] ] ].v4orbit[ [ rfp[ [2] ] ] ] /. v4indrules } ], ind3by4 ] ];
```

```
Out[ ]:= { 1.57813, Null }
```

```
In[ ]:= Dimensions[ ind3by4sp ]
```

```
Out[ ]:= { 1440, 2 }
```

*ind3by4spperm*

```
In[ ]:= ind3by4spperm = ind3by4sp /. MapThread[Rule, {ind3by4, Range[Length[ind3by4]]}, 1];

In[ ]:= Dimensions[ind3by4spperm]

Out[ ]:= {1440}

In[ ]:= Union[ind3by4spperm] === Range[Length[ind3by4]]

Out[ ]:= True

In[ ]:= ind3by4spperm[[ind3by4spperm[[ind3by4spperm[[ind3by4spperm[[ind3by4spperm]]]]]]]] ===
  Range[Length[ind3by4]]

Out[ ]:= True

In[ ]:= ind3by4spperm[[ind3by4spperm]][[ind3by4spperm]][[ind3by4spperm]][[ind3by4spperm]] ==
  Range[Length[ind3by4]]

Out[ ]:= True

In[ ]:= ind3by4spperm[[10]]

Out[ ]:= 1227
```

*allridgecycles*

```
In[ ]:= allridgecycles =
  Union[Map[Sort, Map[ind3by4[[#, 1]] &, Transpose[{Range[Length[ind3by4]], ind3by4spperm,
    ind3by4spperm[[ind3by4spperm]], ind3by4spperm[[ind3by4spperm[[ind3by4spperm]]]],
    ind3by4spperm[[ind3by4spperm[[ind3by4spperm[[ind3by4spperm]]]]]]}], {2}]]];

In[ ]:= Dimensions[allridgecycles]

Out[ ]:= {144, 5}

In[ ]:= Apply[Union, allridgecycles] == Range[720]

Out[ ]:= True
```

*allcycles*

```
In[ ]:= allcycles =
  Map[Reverse, Map[ind3by4[[#, 2]] &, Transpose[{Range[Length[ind3by4]], ind3by4spperm,
    ind3by4spperm[[ind3by4spperm]], ind3by4spperm[[ind3by4spperm[[ind3by4spperm]]]],
    ind3by4spperm[[ind3by4spperm[[ind3by4spperm[[ind3by4spperm]]]]]]}], {2}]]];

In[ ]:= Dimensions[allcycles]

Out[ ]:= {1440, 5}
```

*allcyclesandperms*

```
In[ ]:= allcyclesandperms = Union[
  Map[Sort[{#, RotateLeft[#, 1], RotateLeft[#, 2], RotateLeft[#, 3], RotateLeft[#, 4],
    Reverse[121 - #], Reverse[121 - RotateLeft[#, 1]], Reverse[121 - RotateLeft[#, 2]],
    Reverse[121 - RotateLeft[#, 3]], Reverse[121 - RotateLeft[#, 4]]}] &, allcycles]];

In[ ]:= Dimensions[allcyclesandperms]

Out[ ]:= {144, 10, 5}
```

*repcycles*

```
In[ ]:= repcycles = Map[#[[1]] &, allcyclesandperms];
```

```
In[ ]:= Dimensions[repcycles]
```

```
Out[ ]:= {144, 5}
```

*davisrelators*

```
In[ ]:= davisrelators =
```

```
Join[Table[gen[i].gen[121-i], {i, 1, 60}], Map[Apply[Dot, Map[gen, #]] &, repcycles]];
```

```
In[ ]:= Union[davisrelators /. {gen[i_] => davissspmat[[i]]}] == {IdentityMatrix[5]}
```

```
Out[ ]:= True
```

```
In[ ]:= TableForm[davissspmat[[Range[60], 1 ;; 4, 5]] /. {toQkappa[-tau * Sqrt[1 + 3 tau]] -> -c1,
toQkappa[tau * Sqrt[1 + 3 tau]] -> c1, toQkappa[-2 (1 + tau) * Sqrt[1 + 3 tau]] -> -c4,
toQkappa[2 (1 + tau) * Sqrt[1 + 3 tau]] -> c4, toQkappa[-(1 + tau) * Sqrt[1 + 3 tau]] -> -c2,
toQkappa[(1 + tau) * Sqrt[1 + 3 tau]] -> c2, toQkappa[-(1 + 2 tau) * Sqrt[1 + 3 tau]] -> -c3,
toQkappa[(1 + 2 tau) * Sqrt[1 + 3 tau]] -> c3}, TableHeadings -> {Range[60], {}}]
```

*Out[ ]//TableForm=*

|    |    |     |     |     |
|----|----|-----|-----|-----|
| 1  | c4 | 0   | 0   | 0   |
| 2  | c3 | c2  | c1  | 0   |
| 3  | c3 | c2  | -c1 | 0   |
| 4  | c3 | c1  | 0   | c2  |
| 5  | c3 | c1  | 0   | -c2 |
| 6  | c3 | 0   | c2  | c1  |
| 7  | c3 | 0   | c2  | -c1 |
| 8  | c3 | 0   | -c2 | c1  |
| 9  | c3 | 0   | -c2 | -c1 |
| 10 | c3 | -c1 | 0   | c2  |
| 11 | c3 | -c1 | 0   | -c2 |
| 12 | c3 | -c2 | c1  | 0   |
| 13 | c3 | -c2 | -c1 | 0   |
| 14 | c2 | c3  | 0   | c1  |
| 15 | c2 | c3  | 0   | -c1 |
| 16 | c2 | c2  | c2  | c2  |
| 17 | c2 | c2  | c2  | -c2 |
| 18 | c2 | c2  | -c2 | c2  |
| 19 | c2 | c2  | -c2 | -c2 |
| 20 | c2 | c1  | c3  | 0   |
| 21 | c2 | c1  | -c3 | 0   |
| 22 | c2 | 0   | c1  | c3  |
| 23 | c2 | 0   | c1  | -c3 |
| 24 | c2 | 0   | -c1 | c3  |
| 25 | c2 | 0   | -c1 | -c3 |
| 26 | c2 | -c1 | c3  | 0   |
| 27 | c2 | -c1 | -c3 | 0   |
| 28 | c2 | -c2 | c2  | c2  |
| 29 | c2 | -c2 | c2  | -c2 |
| 30 | c2 | -c2 | -c2 | c2  |
| 31 | c2 | -c2 | -c2 | -c2 |
| 32 | c2 | -c3 | 0   | c1  |
| 33 | c2 | -c3 | 0   | -c1 |
| 34 | c1 | c3  | c2  | 0   |

|    |    |     |     |     |
|----|----|-----|-----|-----|
| 35 | c1 | c3  | -c2 | 0   |
| 36 | c1 | c2  | 0   | c3  |
| 37 | c1 | c2  | 0   | -c3 |
| 38 | c1 | 0   | c3  | c2  |
| 39 | c1 | 0   | c3  | -c2 |
| 40 | c1 | 0   | -c3 | c2  |
| 41 | c1 | 0   | -c3 | -c2 |
| 42 | c1 | -c2 | 0   | c3  |
| 43 | c1 | -c2 | 0   | -c3 |
| 44 | c1 | -c3 | c2  | 0   |
| 45 | c1 | -c3 | -c2 | 0   |
| 46 | 0  | c4  | 0   | 0   |
| 47 | 0  | c3  | c1  | c2  |
| 48 | 0  | c3  | c1  | -c2 |
| 49 | 0  | c3  | -c1 | c2  |
| 50 | 0  | c3  | -c1 | -c2 |
| 51 | 0  | c2  | c3  | c1  |
| 52 | 0  | c2  | c3  | -c1 |
| 53 | 0  | c2  | -c3 | c1  |
| 54 | 0  | c2  | -c3 | -c1 |
| 55 | 0  | c1  | c2  | c3  |
| 56 | 0  | c1  | c2  | -c3 |
| 57 | 0  | c1  | -c2 | c3  |
| 58 | 0  | c1  | -c2 | -c3 |
| 59 | 0  | 0   | c4  | 0   |
| 60 | 0  | 0   | 0   | c4  |

```
In[ ]:= davisrelators // ColumnForm
```

```
Out[ ]:= gen[1].gen[120]
gen[2].gen[119]
gen[3].gen[118]
gen[4].gen[117]
gen[5].gen[116]
gen[6].gen[115]
gen[7].gen[114]
gen[8].gen[113]
gen[9].gen[112]
gen[10].gen[111]
gen[11].gen[110]
gen[12].gen[109]
gen[13].gen[108]
gen[14].gen[107]
gen[15].gen[106]
gen[16].gen[105]
gen[17].gen[104]
gen[18].gen[103]
gen[19].gen[102]
gen[20].gen[101]
gen[21].gen[100]
gen[22].gen[99]
```

```

gen[23].gen[98]
gen[24].gen[97]
gen[25].gen[96]
gen[26].gen[95]
gen[27].gen[94]
gen[28].gen[93]
gen[29].gen[92]
gen[30].gen[91]
gen[31].gen[90]
gen[32].gen[89]
gen[33].gen[88]
gen[34].gen[87]
gen[35].gen[86]
gen[36].gen[85]
gen[37].gen[84]
gen[38].gen[83]
gen[39].gen[82]
gen[40].gen[81]
gen[41].gen[80]
gen[42].gen[79]
gen[43].gen[78]
gen[44].gen[77]
gen[45].gen[76]
gen[46].gen[75]
gen[47].gen[74]
gen[48].gen[73]
gen[49].gen[72]
gen[50].gen[71]
gen[51].gen[70]
gen[52].gen[69]
gen[53].gen[68]
gen[54].gen[67]
gen[55].gen[66]
gen[56].gen[65]
gen[57].gen[64]
gen[58].gen[63]
gen[59].gen[62]
gen[60].gen[61]
gen[1].gen[108].gen[45].gen[34].gen[119]
gen[1].gen[109].gen[44].gen[35].gen[118]
gen[1].gen[110].gen[43].gen[36].gen[117]
gen[1].gen[111].gen[42].gen[37].gen[116]
gen[1].gen[112].gen[41].gen[38].gen[115]
gen[1].gen[113].gen[40].gen[39].gen[114]
gen[1].gen[114].gen[39].gen[40].gen[113]
gen[1].gen[115].gen[38].gen[41].gen[112]
gen[1].gen[116].gen[37].gen[42].gen[111]
gen[1].gen[117].gen[36].gen[43].gen[110]
gen[1].gen[118].gen[35].gen[44].gen[109]
gen[1].gen[119].gen[34].gen[45].gen[108]

```

```

gen[2].gen[101].gen[59].gen[21].gen[118]
gen[2].gen[104].gen[56].gen[24].gen[117]
gen[2].gen[105].gen[55].gen[25].gen[116]
gen[2].gen[106].gen[50].gen[28].gen[115]
gen[2].gen[107].gen[49].gen[29].gen[114]
gen[2].gen[114].gen[29].gen[49].gen[107]
gen[2].gen[115].gen[28].gen[50].gen[106]
gen[2].gen[116].gen[25].gen[55].gen[105]
gen[2].gen[117].gen[24].gen[56].gen[104]
gen[2].gen[118].gen[21].gen[59].gen[101]
gen[3].gen[102].gen[58].gen[22].gen[117]
gen[3].gen[103].gen[57].gen[23].gen[116]
gen[3].gen[106].gen[48].gen[30].gen[113]
gen[3].gen[107].gen[47].gen[31].gen[112]
gen[3].gen[112].gen[31].gen[47].gen[107]
gen[3].gen[113].gen[30].gen[48].gen[106]
gen[3].gen[116].gen[23].gen[57].gen[103]
gen[3].gen[117].gen[22].gen[58].gen[102]
gen[4].gen[103].gen[53].gen[26].gen[115]
gen[4].gen[105].gen[51].gen[27].gen[113]
gen[4].gen[107].gen[46].gen[32].gen[111]
gen[4].gen[111].gen[32].gen[46].gen[107]
gen[4].gen[113].gen[27].gen[51].gen[105]
gen[4].gen[115].gen[26].gen[53].gen[103]
gen[5].gen[102].gen[54].gen[26].gen[114]
gen[5].gen[104].gen[52].gen[27].gen[112]
gen[5].gen[106].gen[46].gen[33].gen[110]
gen[5].gen[110].gen[33].gen[46].gen[106]
gen[5].gen[112].gen[27].gen[52].gen[104]
gen[5].gen[114].gen[26].gen[54].gen[102]
gen[6].gen[99].gen[60].gen[23].gen[114]
gen[6].gen[101].gen[52].gen[30].gen[111]
gen[6].gen[105].gen[47].gen[33].gen[109]
gen[6].gen[109].gen[33].gen[47].gen[105]
gen[6].gen[111].gen[30].gen[52].gen[101]
gen[6].gen[114].gen[23].gen[60].gen[99]
gen[7].gen[101].gen[51].gen[31].gen[110]
gen[7].gen[104].gen[48].gen[32].gen[109]
gen[7].gen[109].gen[32].gen[48].gen[104]
gen[7].gen[110].gen[31].gen[51].gen[101]
gen[8].gen[97].gen[60].gen[25].gen[112]
gen[8].gen[100].gen[54].gen[28].gen[111]
gen[8].gen[103].gen[49].gen[33].gen[108]
gen[8].gen[108].gen[33].gen[49].gen[103]
gen[8].gen[111].gen[28].gen[54].gen[100]
gen[8].gen[112].gen[25].gen[60].gen[97]
gen[9].gen[100].gen[53].gen[29].gen[110]
gen[9].gen[102].gen[50].gen[32].gen[108]
gen[9].gen[108].gen[32].gen[50].gen[102]
gen[9].gen[110].gen[29].gen[53].gen[100]

```

gen[10].gen[97].gen[57].gen[29].gen[109]  
 gen[10].gen[99].gen[55].gen[31].gen[108]  
 gen[10].gen[108].gen[31].gen[55].gen[99]  
 gen[10].gen[109].gen[29].gen[57].gen[97]  
 gen[11].gen[96].gen[58].gen[28].gen[109]  
 gen[11].gen[98].gen[56].gen[30].gen[108]  
 gen[11].gen[108].gen[30].gen[56].gen[98]  
 gen[11].gen[109].gen[28].gen[58].gen[96]  
 gen[12].gen[95].gen[59].gen[27].gen[108]  
 gen[12].gen[108].gen[27].gen[59].gen[95]  
 gen[14].gen[85].gen[60].gen[37].gen[106]  
 gen[14].gen[86].gen[54].gen[38].gen[105]  
 gen[14].gen[87].gen[52].gen[40].gen[103]  
 gen[14].gen[103].gen[40].gen[52].gen[87]  
 gen[14].gen[105].gen[38].gen[54].gen[86]  
 gen[14].gen[106].gen[37].gen[60].gen[85]  
 gen[15].gen[86].gen[53].gen[39].gen[104]  
 gen[15].gen[87].gen[51].gen[41].gen[102]  
 gen[15].gen[102].gen[41].gen[51].gen[87]  
 gen[15].gen[104].gen[39].gen[53].gen[86]  
 gen[16].gen[85].gen[57].gen[39].gen[101]  
 gen[16].gen[87].gen[48].gen[42].gen[99]  
 gen[16].gen[99].gen[42].gen[48].gen[87]  
 gen[16].gen[101].gen[39].gen[57].gen[85]  
 gen[17].gen[84].gen[58].gen[38].gen[101]  
 gen[17].gen[87].gen[47].gen[43].gen[98]  
 gen[17].gen[98].gen[43].gen[47].gen[87]  
 gen[17].gen[101].gen[38].gen[58].gen[84]  
 gen[18].gen[85].gen[55].gen[41].gen[100]  
 gen[18].gen[86].gen[50].gen[42].gen[97]  
 gen[18].gen[97].gen[42].gen[50].gen[86]  
 gen[18].gen[100].gen[41].gen[55].gen[85]  
 gen[19].gen[84].gen[56].gen[40].gen[100]  
 gen[19].gen[86].gen[49].gen[43].gen[96]  
 gen[19].gen[96].gen[43].gen[49].gen[86]  
 gen[19].gen[100].gen[40].gen[56].gen[84]  
 gen[20].gen[87].gen[46].gen[44].gen[95]  
 gen[20].gen[95].gen[44].gen[46].gen[87]  
 gen[21].gen[86].gen[46].gen[45].gen[94]  
 gen[21].gen[94].gen[45].gen[46].gen[86]  
 gen[22].gen[83].gen[59].gen[40].gen[97]  
 gen[22].gen[85].gen[49].gen[44].gen[93]  
 gen[22].gen[93].gen[44].gen[49].gen[85]  
 gen[22].gen[97].gen[40].gen[59].gen[83]  
 gen[23].gen[82].gen[59].gen[41].gen[96]  
 gen[23].gen[84].gen[50].gen[44].gen[92]  
 gen[23].gen[92].gen[44].gen[50].gen[84]  
 gen[23].gen[96].gen[41].gen[59].gen[82]  
 gen[24].gen[85].gen[47].gen[45].gen[91]  
 gen[24].gen[91].gen[45].gen[47].gen[85]



```

gen[25].gen[84].gen[48].gen[45].gen[90]
gen[25].gen[90].gen[45].gen[48].gen[84]
gen[26].gen[82].gen[56].gen[42].gen[93]
gen[26].gen[83].gen[55].gen[43].gen[92]
gen[26].gen[92].gen[43].gen[55].gen[83]
gen[26].gen[93].gen[42].gen[56].gen[82]
gen[27].gen[80].gen[58].gen[42].gen[91]
gen[27].gen[81].gen[57].gen[43].gen[90]
gen[27].gen[90].gen[43].gen[57].gen[81]
gen[27].gen[91].gen[42].gen[58].gen[80]
gen[28].gen[83].gen[51].gen[45].gen[89]
gen[28].gen[89].gen[45].gen[51].gen[83]
gen[29].gen[82].gen[52].gen[45].gen[88]
gen[29].gen[88].gen[45].gen[52].gen[82]
gen[30].gen[81].gen[53].gen[44].gen[89]
gen[30].gen[89].gen[44].gen[53].gen[81]
gen[31].gen[80].gen[54].gen[44].gen[88]
gen[31].gen[88].gen[44].gen[54].gen[80]
gen[32].gen[79].gen[60].gen[43].gen[88]
gen[32].gen[88].gen[43].gen[60].gen[79]
gen[46].gen[71].gen[58].gen[55].gen[74]
gen[46].gen[72].gen[57].gen[56].gen[73]
gen[46].gen[73].gen[56].gen[57].gen[72]
gen[46].gen[74].gen[55].gen[58].gen[71]
gen[47].gen[70].gen[59].gen[53].gen[72]
gen[47].gen[72].gen[53].gen[59].gen[70]
gen[48].gen[69].gen[59].gen[54].gen[71]
gen[48].gen[71].gen[54].gen[59].gen[69]
gen[51].gen[66].gen[60].gen[56].gen[69]
gen[51].gen[69].gen[56].gen[60].gen[66]
gen[53].gen[64].gen[60].gen[58].gen[67]
gen[53].gen[67].gen[58].gen[60].gen[64]

```

```
In[ ]:= TableForm[Map[Apply[List, #] /. {gen[i_] -> i} &, davisrelators]]
```

```
Out[ ]//TableForm=
```

```

1      120
2      119
3      118
4      117
5      116
6      115
7      114
8      113
9      112
10     111
11     110
12     109
13     108
14     107
15     106
16     105

```

|    |     |    |    |     |
|----|-----|----|----|-----|
| 17 | 104 |    |    |     |
| 18 | 103 |    |    |     |
| 19 | 102 |    |    |     |
| 20 | 101 |    |    |     |
| 21 | 100 |    |    |     |
| 22 | 99  |    |    |     |
| 23 | 98  |    |    |     |
| 24 | 97  |    |    |     |
| 25 | 96  |    |    |     |
| 26 | 95  |    |    |     |
| 27 | 94  |    |    |     |
| 28 | 93  |    |    |     |
| 29 | 92  |    |    |     |
| 30 | 91  |    |    |     |
| 31 | 90  |    |    |     |
| 32 | 89  |    |    |     |
| 33 | 88  |    |    |     |
| 34 | 87  |    |    |     |
| 35 | 86  |    |    |     |
| 36 | 85  |    |    |     |
| 37 | 84  |    |    |     |
| 38 | 83  |    |    |     |
| 39 | 82  |    |    |     |
| 40 | 81  |    |    |     |
| 41 | 80  |    |    |     |
| 42 | 79  |    |    |     |
| 43 | 78  |    |    |     |
| 44 | 77  |    |    |     |
| 45 | 76  |    |    |     |
| 46 | 75  |    |    |     |
| 47 | 74  |    |    |     |
| 48 | 73  |    |    |     |
| 49 | 72  |    |    |     |
| 50 | 71  |    |    |     |
| 51 | 70  |    |    |     |
| 52 | 69  |    |    |     |
| 53 | 68  |    |    |     |
| 54 | 67  |    |    |     |
| 55 | 66  |    |    |     |
| 56 | 65  |    |    |     |
| 57 | 64  |    |    |     |
| 58 | 63  |    |    |     |
| 59 | 62  |    |    |     |
| 60 | 61  |    |    |     |
| 1  | 108 | 45 | 34 | 119 |
| 1  | 109 | 44 | 35 | 118 |
| 1  | 110 | 43 | 36 | 117 |
| 1  | 111 | 42 | 37 | 116 |
| 1  | 112 | 41 | 38 | 115 |
| 1  | 113 | 40 | 39 | 114 |

|   |     |    |    |     |
|---|-----|----|----|-----|
| 1 | 114 | 39 | 40 | 113 |
| 1 | 115 | 38 | 41 | 112 |
| 1 | 116 | 37 | 42 | 111 |
| 1 | 117 | 36 | 43 | 110 |
| 1 | 118 | 35 | 44 | 109 |
| 1 | 119 | 34 | 45 | 108 |
| 2 | 101 | 59 | 21 | 118 |
| 2 | 104 | 56 | 24 | 117 |
| 2 | 105 | 55 | 25 | 116 |
| 2 | 106 | 50 | 28 | 115 |
| 2 | 107 | 49 | 29 | 114 |
| 2 | 114 | 29 | 49 | 107 |
| 2 | 115 | 28 | 50 | 106 |
| 2 | 116 | 25 | 55 | 105 |
| 2 | 117 | 24 | 56 | 104 |
| 2 | 118 | 21 | 59 | 101 |
| 3 | 102 | 58 | 22 | 117 |
| 3 | 103 | 57 | 23 | 116 |
| 3 | 106 | 48 | 30 | 113 |
| 3 | 107 | 47 | 31 | 112 |
| 3 | 112 | 31 | 47 | 107 |
| 3 | 113 | 30 | 48 | 106 |
| 3 | 116 | 23 | 57 | 103 |
| 3 | 117 | 22 | 58 | 102 |
| 4 | 103 | 53 | 26 | 115 |
| 4 | 105 | 51 | 27 | 113 |
| 4 | 107 | 46 | 32 | 111 |
| 4 | 111 | 32 | 46 | 107 |
| 4 | 113 | 27 | 51 | 105 |
| 4 | 115 | 26 | 53 | 103 |
| 5 | 102 | 54 | 26 | 114 |
| 5 | 104 | 52 | 27 | 112 |
| 5 | 106 | 46 | 33 | 110 |
| 5 | 110 | 33 | 46 | 106 |
| 5 | 112 | 27 | 52 | 104 |
| 5 | 114 | 26 | 54 | 102 |
| 6 | 99  | 60 | 23 | 114 |
| 6 | 101 | 52 | 30 | 111 |
| 6 | 105 | 47 | 33 | 109 |
| 6 | 109 | 33 | 47 | 105 |
| 6 | 111 | 30 | 52 | 101 |
| 6 | 114 | 23 | 60 | 99  |
| 7 | 101 | 51 | 31 | 110 |
| 7 | 104 | 48 | 32 | 109 |
| 7 | 109 | 32 | 48 | 104 |
| 7 | 110 | 31 | 51 | 101 |
| 8 | 97  | 60 | 25 | 112 |
| 8 | 100 | 54 | 28 | 111 |
| 8 | 103 | 49 | 33 | 108 |
| 8 | 108 | 33 | 49 | 103 |

|    |     |    |    |     |
|----|-----|----|----|-----|
| 8  | 111 | 28 | 54 | 100 |
| 8  | 112 | 25 | 60 | 97  |
| 9  | 100 | 53 | 29 | 110 |
| 9  | 102 | 50 | 32 | 108 |
| 9  | 108 | 32 | 50 | 102 |
| 9  | 110 | 29 | 53 | 100 |
| 10 | 97  | 57 | 29 | 109 |
| 10 | 99  | 55 | 31 | 108 |
| 10 | 108 | 31 | 55 | 99  |
| 10 | 109 | 29 | 57 | 97  |
| 11 | 96  | 58 | 28 | 109 |
| 11 | 98  | 56 | 30 | 108 |
| 11 | 108 | 30 | 56 | 98  |
| 11 | 109 | 28 | 58 | 96  |
| 12 | 95  | 59 | 27 | 108 |
| 12 | 108 | 27 | 59 | 95  |
| 14 | 85  | 60 | 37 | 106 |
| 14 | 86  | 54 | 38 | 105 |
| 14 | 87  | 52 | 40 | 103 |
| 14 | 103 | 40 | 52 | 87  |
| 14 | 105 | 38 | 54 | 86  |
| 14 | 106 | 37 | 60 | 85  |
| 15 | 86  | 53 | 39 | 104 |
| 15 | 87  | 51 | 41 | 102 |
| 15 | 102 | 41 | 51 | 87  |
| 15 | 104 | 39 | 53 | 86  |
| 16 | 85  | 57 | 39 | 101 |
| 16 | 87  | 48 | 42 | 99  |
| 16 | 99  | 42 | 48 | 87  |
| 16 | 101 | 39 | 57 | 85  |
| 17 | 84  | 58 | 38 | 101 |
| 17 | 87  | 47 | 43 | 98  |
| 17 | 98  | 43 | 47 | 87  |
| 17 | 101 | 38 | 58 | 84  |
| 18 | 85  | 55 | 41 | 100 |
| 18 | 86  | 50 | 42 | 97  |
| 18 | 97  | 42 | 50 | 86  |
| 18 | 100 | 41 | 55 | 85  |
| 19 | 84  | 56 | 40 | 100 |
| 19 | 86  | 49 | 43 | 96  |
| 19 | 96  | 43 | 49 | 86  |
| 19 | 100 | 40 | 56 | 84  |
| 20 | 87  | 46 | 44 | 95  |
| 20 | 95  | 44 | 46 | 87  |
| 21 | 86  | 46 | 45 | 94  |
| 21 | 94  | 45 | 46 | 86  |
| 22 | 83  | 59 | 40 | 97  |
| 22 | 85  | 49 | 44 | 93  |
| 22 | 93  | 44 | 49 | 85  |
| 22 | 97  | 40 | 59 | 83  |

|    |    |    |    |    |
|----|----|----|----|----|
| 23 | 82 | 59 | 41 | 96 |
| 23 | 84 | 50 | 44 | 92 |
| 23 | 92 | 44 | 50 | 84 |
| 23 | 96 | 41 | 59 | 82 |
| 24 | 85 | 47 | 45 | 91 |
| 24 | 91 | 45 | 47 | 85 |
| 25 | 84 | 48 | 45 | 90 |
| 25 | 90 | 45 | 48 | 84 |
| 26 | 82 | 56 | 42 | 93 |
| 26 | 83 | 55 | 43 | 92 |
| 26 | 92 | 43 | 55 | 83 |
| 26 | 93 | 42 | 56 | 82 |
| 27 | 80 | 58 | 42 | 91 |
| 27 | 81 | 57 | 43 | 90 |
| 27 | 90 | 43 | 57 | 81 |
| 27 | 91 | 42 | 58 | 80 |
| 28 | 83 | 51 | 45 | 89 |
| 28 | 89 | 45 | 51 | 83 |
| 29 | 82 | 52 | 45 | 88 |
| 29 | 88 | 45 | 52 | 82 |
| 30 | 81 | 53 | 44 | 89 |
| 30 | 89 | 44 | 53 | 81 |
| 31 | 80 | 54 | 44 | 88 |
| 31 | 88 | 44 | 54 | 80 |
| 32 | 79 | 60 | 43 | 88 |
| 32 | 88 | 43 | 60 | 79 |
| 46 | 71 | 58 | 55 | 74 |
| 46 | 72 | 57 | 56 | 73 |
| 46 | 73 | 56 | 57 | 72 |
| 46 | 74 | 55 | 58 | 71 |
| 47 | 70 | 59 | 53 | 72 |
| 47 | 72 | 53 | 59 | 70 |
| 48 | 69 | 59 | 54 | 71 |
| 48 | 71 | 54 | 59 | 69 |
| 51 | 66 | 60 | 56 | 69 |
| 51 | 69 | 56 | 60 | 66 |
| 53 | 64 | 60 | 58 | 67 |
| 53 | 67 | 58 | 60 | 64 |

```
In[ ]:= s5points[[1]] - s5points[[120]]
```

```
Out[ ]:= { -5.24..., 0, 0, 0, 0 }
```

```
In[ ]:= s5points[[1]]
```

```
Out[ ]:= { -2.62..., 0, 0, 0, 2.42... }
```

```
In[ ]:= davisspmat[[1]] == rmat[{1, 0, 0, 0, 0}].rmat[s5points[[1]]]
```

```
Out[ ]:= True
```

```
In[ ]:= ind1by4 // Dimensions
```

```
Out[ ]:= {2400, 2}
```

```
ind1by4sp
```

```
In[ ]:= Timing[ind1by4sp = Map[Function[rfp, Map[{rfp[[1]], #} &, ind1to4[{rfp[[1]]}]]],  
    Map[Function[rfp, {davisspmat[{rfp[[2]]}].v1orbit[{rfp[[1]]}] /. v1indrules,  
        davisspmat[{rfp[[2]]}].v4orbit[{rfp[[2]]}] /. v4indrules}], ind1by4]];
```

```
Out[ ]:= {2.26563, Null}
```

```
In[ ]:= Dimensions[ind1by4sp]
```

```
Out[ ]:= {2400, 4, 2}
```

```
ind1by4spperm
```

```
In[ ]:= ind1by4spperm = ind1by4sp /. MapThread[Rule, {ind1by4, Range[Length[ind1by4]]}, 1];
```

```
In[ ]:= Dimensions[ind1by4spperm]
```

```
Out[ ]:= {2400, 4}
```

```
In[ ]:= ind2by4 // Dimensions
```

```
Out[ ]:= {3600, 2}
```

```
ind2by4sp
```

```
In[ ]:= Timing[ind2by4sp = Map[Function[rfp, Map[{rfp[[1]], #} &, ind2to4[{rfp[[1]]}]]],  
    Map[Function[rfp, {davisspmat[{rfp[[2]]}].v2orbit[{rfp[[1]]}] /. v2indrules,  
        davisspmat[{rfp[[2]]}].v4orbit[{rfp[[2]]}] /. v4indrules}], ind2by4]];
```

```
Out[ ]:= {3.51563, Null}
```

```
In[ ]:= Dimensions[ind2by4sp]
```

```
Out[ ]:= {3600, 3, 2}
```

```
ind2by4spperm
```

```
In[ ]:= ind2by4spperm = ind2by4sp /. MapThread[Rule, {ind2by4, Range[Length[ind2by4]]}, 1];
```

```
In[ ]:= Dimensions[ind2by4spperm]
```

```
Out[ ]:= {3600, 3}
```

```
all1by4cycles
```

```
In[ ]:= AbsoluteTiming[Dimensions[all1by4cycles =  
    Union[Map[FixedPoint[Union[#, Apply[Union, ind1by4spperm[[#]]]] &, {#}] &,  
        Partition[Range[Length[ind1by4]], 4] [[All, 1]]]]]]
```

```
Out[ ]:= {9.99109, {1, 2400}}
```

```
all2by4cycles
```

```
In[ ]:= AbsoluteTiming[Dimensions[all2by4cycles =  
    Union[Map[FixedPoint[Union[#, Apply[Union, ind2by4spperm[[#]]]] &, {#}] &,  
        Partition[Range[Length[ind2by4]], 3] [[All, 1]]]]]]
```

```
Out[ ]:= {0.177387, {60, 60}}
```

```
alledgecycles
```

```
In[ ]:= Dimensions[alledgecycles = Map[Union[ind2by4[[#]] [[All, 1]]] &, all2by4cycles]]
```

```
Out[ ]:= {60, 20}
```

```
In[ ]:= 1 - 60 + 144 - 60 + 1
```

```
Out[ ]:= 26
```

For each vertex, find a sequence of side pairing maps that takes that vertex to the standard vertex.

```
In[ ]:= Position[v1orbit, verts5335[[1]]]
```

```
Out[ ]:= {{600}}
```

```
In[ ]:= {600, {}}
```

```
Out[ ]:= {600, {}}
```

```
In[ ]:= antipodalindex[ind1to4[{600}]]
```

```
Out[ ]:= {4, 3, 2, 1}
```

*moveback, moveback1*

```
In[ ]:= moveback1[{vn_, snl_}] :=  
  Map[{davisspmat[[#]].v1orbit[vn] /. v1indrules, Append[snl, antipodalindex[[#]]] &,   
    ind1to4[vn]]];  
moveback[x_] := GatherBy[Union[x, Apply[Union, Map[moveback1, x]]], #[[1]] &][[All, 1]];
```

*vertextraces*

```
In[ ]:= AbsoluteTiming[Dimensions[vertextraces = FixedPoint[moveback, {{600, {}}][[All, 2]]]]
```

```
Out[ ]:= {9.5205, {600}}
```

```
In[ ]:= Union[MapThread[Apply[Dot, davisspmat[[#1]]].#2 &, {vertextraces, v1orbit}]] ==  
  {verts5335[[1]]}
```

```
Out[ ]:= True
```

## Davis spin structure

Pick off one specific lift of the first side pairing map as product of reflections in  $Cl(4, 1)$ .

*davisspmatlift1*

```
In[ ]:= davisspmatlift1 = -reflectionlift[{1, 0, 0, 0, 0}].reflectionlift[s5points[[1]]];
```

is a quaternion matrix

```
In[ ]:= rmatismat[davisspmatlift1]
```

```
Out[ ]:= True
```

```
In[ ]:= Det[davisspmatlift1]
```

```
Out[ ]:= 1
```

This is the first Davis side pairing map lift, a real  $2 \times 2$  matrix!

```
In[ ]:= rmattoqmat[formatkappa[davisspmatlift1]] // MatrixForm
```

*Out[ ]//MatrixForm=*

$$\begin{pmatrix} -1 - \tau & \kappa \\ \kappa & -1 - \tau \end{pmatrix}$$

and acts as the first Davis side pairing map.

```
In[ ]:= spinprojection[davisspmatlift1] == davisspmat[[1]]
```

```
Out[ ]:= True
```

Have lift of the o.p. subgroup of the 533 reflections to  $Cl(4, 1)$  and take the image in  $8 \times 8$  real ( $2 \times 2$  quaternion) matrices. Conjugating the first lift by symmetries gives only 120 generators

*davisspmatliftpre*

```
In[ ]:= AbsoluteTiming[
  Dimensions[davisspmatliftpre = Union[Map[#, davisspmatlift1.Inverse[#] &, grpop533lift]]]]
```

```
Out[ ]:= {93.7759, {120, 8, 8}}
```

Corresponding to the Davis side pairing maps.

*davisspmatlift*

```
In[ ]:= AbsoluteTiming[davisspmatlift = davisspmatliftpre[[Ordering[
  Map[Position[davisspmat, spinprojection[#]]][[1, 1]] &, davisspmatliftpre]]];]
```

```
Out[ ]:= {1.22509, Null}
```

Check the action of the lifts agree with the side pairing maps downstairs.

```
In[ ]:= Map[spinprojection, davisspmatlift] == davisspmat
```

```
Out[ ]:= True
```

The side pairing maps satisfy the defining (inverse pair and ridge cycle) relators.

```
In[ ]:= Union[davisrelators /. {gen[i_] => davisspmat[[i]]}] == {IdentityMatrix[5]}
```

```
Out[ ]:= True
```

But so do the 120 lifts we selected, i.e., the Davis manifold group lifts to an isomorphic copy in  $Spin(4, 1)$ .

```
In[ ]:= Union[davisrelators /. {gen[i_] => davisspmatlift[[i]]}] == {IdentityMatrix[8]}
```

```
Out[ ]:= True
```

```
In[ ]:= rmattoqmat[formatkappa[davisspmatlift[[2]]]] // MatrixForm
```

*Out[ ]//MatrixForm=*

$$\begin{pmatrix} -1 - \tau & \frac{i\kappa}{2} + j\kappa \left( -\frac{1}{2} + \frac{\tau}{2} \right) + \frac{\kappa\tau}{2} \\ -\frac{i\kappa}{2} + j\kappa \left( \frac{1}{2} - \frac{\tau}{2} \right) + \frac{\kappa\tau}{2} & -1 - \tau \end{pmatrix}$$

```
In[ ]:= rmattoqmat[formatkappa[davisspmatlift[[3]]]] // MatrixForm
```

*Out[ ]//MatrixForm=*

$$\begin{pmatrix} -1 - \tau & \frac{i\kappa}{2} + j\kappa \left( \frac{1}{2} - \frac{\tau}{2} \right) + \frac{\kappa\tau}{2} \\ -\frac{i\kappa}{2} + j\kappa \left( -\frac{1}{2} + \frac{\tau}{2} \right) + \frac{\kappa\tau}{2} & -1 - \tau \end{pmatrix}$$



```
In[ ]:= rmattoqmat[formatkappa[davisspmatlift[[4]]]] // MatrixForm
```

Out[ ]:=MatrixForm=

$$\begin{pmatrix} -1 - \tau & \frac{\mathbb{k} \kappa}{2} + \mathbb{i} \kappa \left( -\frac{1}{2} + \frac{\tau}{2} \right) + \frac{\kappa \tau}{2} \\ -\frac{\mathbb{k} \kappa}{2} + \mathbb{i} \kappa \left( \frac{1}{2} - \frac{\tau}{2} \right) + \frac{\kappa \tau}{2} & -1 - \tau \end{pmatrix}$$

```
In[ ]:= rmattoqmat[formatkappa[davisspmatlift[[16]]]] // MatrixForm
```

Out[ ]:=MatrixForm=

$$\begin{pmatrix} -1 - \tau & \frac{\kappa}{2} + \frac{\mathbb{i} \kappa}{2} + \frac{\mathbb{j} \kappa}{2} + \frac{\mathbb{k} \kappa}{2} \\ \frac{\kappa}{2} - \frac{\mathbb{i} \kappa}{2} - \frac{\mathbb{j} \kappa}{2} - \frac{\mathbb{k} \kappa}{2} & -1 - \tau \end{pmatrix}$$

## Additions

First some routines for computing subgroups of products, compute conjugacy classes, and orders of elements.

sgpairsgen

```
In[ ]:= sgpairsgen[gen_, nmax_ : Infinity] :=
  FixedPoint[Function[p, {Union[p[[1]], Apply[Union, Map[Function[m, Map[{m[[1]].#[[1]],
    m[[2]].#[[2]]] &, gen]], Complement[p[[1]], p[[2]]]]], p[[1]]}],
    {{IdentityMatrix[Length[gen[[1, 1]]], IdentityMatrix[Length[gen[[1, 2]]]]}, {}},
    nmax][[1]];
```

conjclasses

```
In[ ]:= conjclasses[sg_] := Sort[FixedPoint[Function[p,
  If[p[[1]] == {}, p, Function[c, {Complement[p[[1]], c], Append[p[[2]], c]}][
    Union[Map[Inverse[#].p[[1, 1]].# &, sg]]]], {sg, {}}][[2]]];
```

elementorder

```
In[ ]:= elementorder[m_, lim_ : 100] :=
  Function[p, If[p[[1]] == IdentityMatrix[Length[p[[1]]]], FixedPoint[
    Function[q, If[q[[1]] > p[[2]], q, If[Not[IntegerQ[q[[2]] / q[[1]]]] || MatrixPower[
      m, q[[2]] / q[[1]] != IdentityMatrix[Length[m]], {NextPrime[q[[1]]],
      q[[2]]}, {q[[1]], q[[2]] / q[[1]]}]], {2, p[[2]] !}][[2]], $Failed]][
    FixedPoint[Function[p, If[p[[1]] == IdentityMatrix[Length[m]], p,
      {MatrixPower[m, p[[2]] + 1], p[[2]] + 1}]], {m, 1}, lim]];
```

We find the indices of a word in the generators of the Davis manifold group carrying  $v_5$  to a given point.

reduce1, reducestep

```
In[ ]:= reduce1[m_] :=
  SortBy[Map[{#, davisspmat[[121 - #]].m} &, Range[120]], N[#[[2, -1]]] &][[1]];
reducestep[{g_, m_}] :=
  If[N[m[[-1]]] < N[#[[2, -1]]], {g, m}, {Append[g, #[[1]], #[[2]]] &[reduce1[m]]];
```

represent, representcondition

```
In[ ]:= represent[m_] := FixedPoint[reducestep, {{}, m}][[1]];
representcondition[g_, m_] := Apply[Dot, davisspmat[[g]].verts5335[[5]] == m;
```

representmat, representmatcondition

```
In[ ]:= representmat[m_] := represent[m.verts5335[[5]]];
representmatcondition[g_, m_] := Apply[Dot, davisspmat[[g]] == m;
```

We construct the corresponding lifts of orientation preserving symmetries of the 120-cell.

```
grp533grp533lifts
```

```
In[ ]:= AbsoluteTiming[Dimensions[grp533grp533lifts = SortBy[Map[{#[[1, 1]], #[[All, 2]]] &,
  GatherBy[sgpairs[Transpose[{gen533, gen533lift}]], #[[1]] &], #[[1]] &]]]
```

```
Out[ ]:= {58.7174, {7200, 2}}
```

```
In[ ]:= Map[Dimensions, grp533grp533lifts[[1]]]
```

```
Out[ ]:= {{5, 5}, {2, 8, 8}}
```

```
In[ ]:= grp533 == grp533grp533lifts[[All, 1]]
```

```
Out[ ]:= True
```

```
grp533lift1
```

```
In[ ]:= Dimensions[grp533lift1 = grp533grp533lifts[[All, 2, 1]]]
```

```
Out[ ]:= {7200, 8, 8}
```

## Review

Take  $\kappa = \sqrt{1+3\tau}$  for  $\tau = (1 + \sqrt{5})/2$  the golden ratio, i.e.,  $\kappa$  is the root of  $x^4 - 5x^2 - 5 = 0$  near 2.42. It is convenient to work in the extension field  $\mathbb{Q}[\kappa]$ . Consider the 5335 Coxeter simplex  $\Delta$ , realized in the hyperboloid model of  $H^4$  with side normal vectors and corresponding opposite vertices respectively of

```
In[ ]:= TableForm[formatkappa[nv5335],
  TableHeadings -> {{u1, u2, u3, u4, u5}, {x1, x2, x3, x4, x5}}]
```

```
Out[ ]//TableForm=
```

|       | $x_1$                          | $x_2$                          | $x_3$         | $x_4$            | $x_5$    |
|-------|--------------------------------|--------------------------------|---------------|------------------|----------|
| $u_1$ | 0                              | 0                              | 0             | -1               | 0        |
| $u_2$ | 0                              | $\frac{1}{2} - \frac{\tau}{2}$ | $\frac{1}{2}$ | $\frac{\tau}{2}$ | 0        |
| $u_3$ | 0                              | 0                              | -1            | 0                | 0        |
| $u_4$ | $\frac{1}{2} - \frac{\tau}{2}$ | $\frac{\tau}{2}$               | $\frac{1}{2}$ | 0                | 0        |
| $u_5$ | $1 + \tau$                     | 0                              | 0             | 0                | $\kappa$ |

```
In[ ]:= TableForm[formatkappa[verts5335],
  TableHeadings -> {{v1, v2, v3, v4, v5}, {x1, x2, x3, x4, x5}}]
```

```
Out[ ]//TableForm=
```

|       | $x_1$               | $x_2$                                               | $x_3$                                             | $x_4$    | $x_5$       |
|-------|---------------------|-----------------------------------------------------|---------------------------------------------------|----------|-------------|
| $v_1$ | $\kappa(2 + 3\tau)$ | $\kappa(1 + \tau)$                                  | 0                                                 | $\kappa$ | $5 + 8\tau$ |
| $v_2$ | $\kappa(1 + \tau)$  | $\kappa$                                            | 0                                                 | 0        | $2 + 3\tau$ |
| $v_3$ | $\kappa\tau$        | $\kappa\left(-\frac{1}{5} + \frac{2\tau}{5}\right)$ | $\kappa\left(\frac{3}{5} - \frac{\tau}{5}\right)$ | 0        | $1 + 2\tau$ |
| $v_4$ | $\kappa$            | 0                                                   | 0                                                 | 0        | $1 + \tau$  |
| $v_5$ | 0                   | 0                                                   | 0                                                 | 0        | 1           |

```
In[ ]:= TableForm[formatkappa[Outer[l dot, nv5335, verts5335, 1]],
  TableHeadings -> {{ "u1", "u2", "u3", "u4", "u5"}, {"v1", "v2", "v3", "v4", "v5"}}]
```

Out[ ]//TableForm=

|                | v <sub>1</sub> | v <sub>2</sub>                                       | v <sub>3</sub>                                        | v <sub>4</sub>                                       | v <sub>5</sub> |
|----------------|----------------|------------------------------------------------------|-------------------------------------------------------|------------------------------------------------------|----------------|
| u <sub>1</sub> | $-\kappa$      | 0                                                    | 0                                                     | 0                                                    | 0              |
| u <sub>2</sub> | 0              | $\kappa \left( \frac{1}{2} - \frac{\tau}{2} \right)$ | 0                                                     | 0                                                    | 0              |
| u <sub>3</sub> | 0              | 0                                                    | $\kappa \left( -\frac{3}{5} + \frac{\tau}{5} \right)$ | 0                                                    | 0              |
| u <sub>4</sub> | 0              | 0                                                    | 0                                                     | $\kappa \left( \frac{1}{2} - \frac{\tau}{2} \right)$ | 0              |
| u <sub>5</sub> | 0              | 0                                                    | 0                                                     | 0                                                    | $-\kappa$      |

and Gram matrix

```
In[ ]:= TableForm[formatkappa[Outer[l dot, nv5335, nv5335, 1]],
  TableHeadings -> {{ "u1", "u2", "u3", "u4", "u5"}, {"u1", "u2", "u3", "u4", "u5"}}]
```

Out[ ]//TableForm=

|                | u <sub>1</sub>    | u <sub>2</sub>    | u <sub>3</sub> | u <sub>4</sub>    | u <sub>5</sub>    |
|----------------|-------------------|-------------------|----------------|-------------------|-------------------|
| u <sub>1</sub> | 1                 | $-\frac{\tau}{2}$ | 0              | 0                 | 0                 |
| u <sub>2</sub> | $-\frac{\tau}{2}$ | 1                 | $-\frac{1}{2}$ | 0                 | 0                 |
| u <sub>3</sub> | 0                 | $-\frac{1}{2}$    | 1              | $-\frac{1}{2}$    | 0                 |
| u <sub>4</sub> | 0                 | 0                 | $-\frac{1}{2}$ | 1                 | $-\frac{\tau}{2}$ |
| u <sub>5</sub> | 0                 | 0                 | 0              | $-\frac{\tau}{2}$ | 1                 |

```
In[ ]:= FullSimplify[Outer[l dot, nv5335, nv5335, 1] ==
  -Cos[Pi / {{1, 5, 2, 2, 2}, {5, 1, 3, 2, 2}, {2, 3, 1, 3, 2}, {2, 2, 3, 1, 5}, {2, 2, 2, 5, 1}}]]
```

Out[ ]:= True

Reflections in these sides are given by Lorentzian matrices

```
In[ ]:= TableForm[Map[MatrixForm[formatkappa[#]] &, gen5335],
  TableHeadings -> {"h1", "h2", "h3", "h4", "h5"}, {}]
```

Out[ ]//TableForm=

$$\begin{array}{l}
h_1 \begin{pmatrix} 1 & 0 & 0 & 0 & 0 \\ 0 & 1 & 0 & 0 & 0 \\ 0 & 0 & 1 & 0 & 0 \\ 0 & 0 & 0 & -1 & 0 \\ 0 & 0 & 0 & 0 & 1 \end{pmatrix} \\
h_2 \begin{pmatrix} 1 & 0 & 0 & 0 & 0 \\ 0 & \frac{\tau}{2} & -\frac{1}{2} + \frac{\tau}{2} & \frac{1}{2} & 0 \\ 0 & -\frac{1}{2} + \frac{\tau}{2} & \frac{1}{2} & -\frac{\tau}{2} & 0 \\ 0 & \frac{1}{2} & -\frac{\tau}{2} & \frac{1}{2} - \frac{\tau}{2} & 0 \\ 0 & 0 & 0 & 0 & 1 \end{pmatrix} \\
h_3 \begin{pmatrix} 1 & 0 & 0 & 0 & 0 \\ 0 & 1 & 0 & 0 & 0 \\ 0 & 0 & -1 & 0 & 0 \\ 0 & 0 & 0 & 1 & 0 \\ 0 & 0 & 0 & 0 & 1 \end{pmatrix} \\
h_4 \begin{pmatrix} \frac{\tau}{2} & \frac{1}{2} & -\frac{1}{2} + \frac{\tau}{2} & 0 & 0 \\ \frac{1}{2} & \frac{1}{2} - \frac{\tau}{2} & -\frac{\tau}{2} & 0 & 0 \\ -\frac{1}{2} + \frac{\tau}{2} & -\frac{\tau}{2} & \frac{1}{2} & 0 & 0 \\ 0 & 0 & 0 & 1 & 0 \\ 0 & 0 & 0 & 0 & 1 \end{pmatrix} \\
h_5 \begin{pmatrix} -3 - 6\tau & 0 & 0 & 0 & \kappa(2 + 2\tau) \\ 0 & 1 & 0 & 0 & 0 \\ 0 & 0 & 1 & 0 & 0 \\ 0 & 0 & 0 & 1 & 0 \\ \kappa(-2 - 2\tau) & 0 & 0 & 0 & 3 + 6\tau \end{pmatrix}
\end{array}$$

```
In[ ]:= Apply[And, MapThread[Function[{g, u, i}, Transpose[g].jmat[4].g == jmat[4] && Det[g] == -1 &&
  g.u == -u && (g.Transpose[#] == Transpose[#] & [Drop[verts5335, {i}]])],
  {gen5335, nv5335, Range[5]}]]
```

Out[ ]:= True

Additionally, the symmetry of the 5335 simplex swapping  $v_1$  with  $v_5$ ,  $v_2$  with  $v_4$ , and fixing  $v_3$  is given by the matrix,  $h_0$

```
In[ ]:= MatrixForm[formatkappa[insideoutmat]]
```

Out[ ]//MatrixForm=

$$\begin{pmatrix} -4 - 7\tau & -1 - 3\tau & 0 & -1 - \tau & \kappa(2 + 3\tau) \\ -1 - 3\tau & -1 - \tau & 0 & 0 & \kappa(1 + \tau) \\ 0 & 0 & 1 & 0 & 0 \\ -1 - \tau & 0 & 0 & 0 & \kappa \\ \kappa(-2 - 3\tau) & \kappa(-1 - \tau) & 0 & -\kappa & 5 + 8\tau \end{pmatrix}$$

```
In[ ]:= Transpose[insideoutmat].jmat[4].insideoutmat == jmat[4] && Det[insideoutmat] == 1 &&
  insideoutmat.Transpose[verts5335] == Transpose[Reverse[verts5335]] &&
  insideoutmat.Transpose[nv5335] == Transpose[Reverse[nv5335]]
```

```
Out[ ]:= True
```

The 5335 Coxeter reflection group is generated by the reflections  $h_i, i = 1, \dots, 5$ , in the sides of the 5335 simplex. The generators  $h_i, i = 0, \dots, 5$ , generate a discrete group  $N$  having as fundamental domain the simplex with vertices  $v_0$ , the midpoint of the line segment between  $v_1$  and  $v_5$ , and vertices  $v_i, i = 2, \dots, 5$ , where  $g_0$  acts to swap this domain to the other half of the 5335 Coxeter simplex having vertices  $v_i, i = 0, \dots, 4$ , though  $g_0$  is not a reflection. Take the barycentric subdivision of the 5335 Coxeter simplex with vertices  $v_S$  where  $S \subseteq \{1, 2, 3, 4, 5\}$  is the barycenter of the simplex with vertices  $v_i$  for  $i \in S$ ,  $v_{\{i\}} = v_i$  for  $i = 1, \dots, 5$ , and  $v_0 = v_{\{1,5\}}$ . This subdivision restricts to a subdivision of the fundamental domain for  $N$ . There will be no particular reason to compute coordinates of the points  $v_S$  as it is just as easy to work with the subset  $S$  and the  $v_i$ , for  $i \in S$ . A Lorentzian matrix  $m$  acts so  $mv_S$  is the barycenter of the points  $mv_i$  for  $i \in S$ .

The generators  $h_i, i = 1, \dots, 4$  fix  $v_5$  and generate the 533 Coxeter reflection group of order 14400. The union of the  $h\Delta$  for  $h$  in this group form a regular hyperbolic 120-cell  $P$  with ridge angles  $2\pi/5$ . The centers of the 120 dodecahedral faces of  $P$  are all images  $hv_4$ , the 600 vertices of  $P$  are all images  $hv_1$ , midpoints of 1200 edges of  $P$  are all images  $hv_2$ , and centers of 720 pentagonal ridges are all images  $hv_3$ .

```
In[ ]:= grp533 == sggen[gen5335[[1 ;; 4]]]
```

```
Out[ ]:= True
```

```
In[ ]:= grpop533 == Select[grp533, Det[#] == 1 &]
```

```
Out[ ]:= True
```

```
In[ ]:= Dimensions[grp533]
```

```
Out[ ]:= {14400, 5, 5}
```

```
In[ ]:= Dimensions[grpop533]
```

```
Out[ ]:= {7200, 5, 5}
```

```
In[ ]:= Sort[v1orbit] == Union[Map[#.verts5335[[1]] &, grp533]] &&
  Sort[v2orbit] == Union[Map[#.verts5335[[2]] &, grp533]] &&
  Sort[v3orbit] == Union[Map[#.verts5335[[3]] &, grp533]] &&
  Sort[v4orbit] == Union[Map[#.verts5335[[4]] &, grp533]]
```

```
Out[ ]:= True
```

```
In[ ]:= Dimensions[v1orbit]
```

```
Out[ ]:= {600, 5}
```

```
In[ ]:= Dimensions[v2orbit]
```

```
Out[ ]:= {1200, 5}
```

```
In[ ]:= Dimensions[v3orbit]
```

```
Out[ ]:= {720, 5}
```

```
In[ ]:= Dimensions[v4orbit]
```

```
Out[ ]:= {120, 5}
```

```
In[ ]:= (v1orbit /. v1indrules) == Range[Length[v1orbit]] &&
        (v2orbit /. v2indrules) == Range[Length[v2orbit]] &&
        (v3orbit /. v3indrules) == Range[Length[v3orbit]] &&
        (v4orbit /. v4indrules) == Range[Length[v4orbit]]
```

```
Out[ ]:= True
```

We have tabulated these centers of sides and normal vectors,  $s_i$ , to sides, and taken corresponding indexing conveniently so as to have sides  $i$  and  $121 - i$  always antipodal. The Davis manifold is defined by a side-pairing of  $P$ , each side  $i$  paired to antipodal side  $121 - i$  by a map  $g_i$  taking  $g_i P$  and  $P$  on opposite across side  $121 - i$ . Now side 1 is taken with center

```
In[ ]:= formatkappa[v4orbit[[1]]]
```

```
Out[ ]:= {-κ, 0, 0, 0, 1 + τ}
```

```
In[ ]:= v4orbit[[120]] == verts5335[[4]]
```

```
Out[ ]:= True
```

and normal vector  $s$

```
In[ ]:= formatkappa[s5points[[1]]]
```

```
Out[ ]:= {-1 - τ, 0, 0, 0, κ}
```

```
In[ ]:= s5points[[120]] == nv5335[[5]]
```

```
Out[ ]:= True
```

with side pairing map  $g_1$

```
In[ ]:= MatrixForm[formatkappa[davisspmat[[1]]]]
```

```
Out[ ]:= MatrixForm=
```

$$\begin{pmatrix} 3 + 6\tau & 0 & 0 & 0 & \kappa(2 + 2\tau) \\ 0 & 1 & 0 & 0 & 0 \\ 0 & 0 & 1 & 0 & 0 \\ 0 & 0 & 0 & 1 & 0 \\ \kappa(2 + 2\tau) & 0 & 0 & 0 & 3 + 6\tau \end{pmatrix}$$

```
In[ ]:= Transpose[davisspmat[[1]]].jmat[4].davisspmat[[1]] == jmat[4] &&
        Det[davisspmat[[1]]] == 1 && davisspmat[[1]].v4orbit[[1]] == v4orbit[[120]] &&
        davisspmat[[1]].s5points[[1]] == -s5points[[120]]
```

```
Out[ ]:= True
```

The remaining side pairings map side-pair  $s_i = hs_1$  to  $s_{121-i} = hs_{120}$  by the map  $g_i = hg_1 h^{-1}$  for each  $h$  in the 533 Coxeter group. Let  $K$  be the group generated by the  $g_i, i = 1, \dots, 120$ . Then  $K$  is an orientation preserving torsion free subgroup of isometries of  $H^4$  with fundamental domain  $P$ . The normalizer of  $K$  is

$N$ , an order 28800 extension of  $K$ .

```
In[ ]:= Apply[And,
  MapThread[Function[{g, s, a}, g.s == -a], {davisspmat, s5points, Reverse[s5points]}]]
```

```
Out[ ]:= True
```

Here is a brute force check that the symmetries of the 120-cell conjugate  $g_1$  to all the other side pairing maps.

```
In[ ]:= Union[davisspmat] == Union[Map[#, davisspmat[[1]].Inverse[#] &, grp533]]
```

```
Out[ ]:= True
```

```
In[ ]:= insideoutmat.davisspmat[[1]].Inverse[insideoutmat].v1orbit[[600]] == v1orbit[[599]]
```

```
Out[ ]:= True
```

*ioconjspmat1word*

```
In[ ]:= ioconjspmat1word = Join[121 - Reverse[vertextraces[[599]]], vertextraces[[600]]]
```

```
Out[ ]:= {5, 84, 48, 69, 39, 114, 6, 83, 51, 74, 36, 117}
```

```
In[ ]:= insideoutmat.davisspmat[[1]].Inverse[insideoutmat] ==
  Apply[Dot, davisspmat[[ioconjspmat1word]]]
```

```
Out[ ]:= True
```

So  $h_0$  the symmetry of the 5335 simplex corresponding to the inside out symmetry conjugating  $g_1$  gives  $h_0 g_1 h_0^{-1} = g_5 g_{84} g_{48} g_{69} g_{39} g_{114} g_6 g_{83} g_{51} g_{74} g_{36} g_{117} = w$ .

We can avoid a brute force check that the inside out matrix conjugates all of the side pairing map generators into the Davis manifold group. First, each  $g_i = h g_1 h^{-1}$  for some orientation preserving 120-cell symmetry  $h$ . We claim for any  $h$  an orientation preserving symmetry of the 120 that  $h_0 h = g h' h_0$  for some  $g$  in the Davis manifold group and some  $h'$  an orientation preserving symmetry of the 120 cell, namely  $g h' = h_0 h h_0^{-1}$ . Since the symmetry group of the 120-cell clearly normalizes the Davis manifold group, its enough for this claim to check each  $h_0 h_i h_0^{-1}$  is of the form  $g h'$  for each of the generators  $h_i$ ,  $i = 1, \dots, 4$ , of the symmetry group of the 120-cell. Then

$h_0 g_i h_0^{-1} = h_0 h g_1 h^{-1} h_0^{-1} = g h' h_0 g_1 h_0^{-1} h'^{-1} g^{-1} = g h' w h'^{-1} g^{-1}$  is clearly in the Davis manifold group again.

```
In[ ]:= Position[grp533, Inverse[davisspmat[[1]]].gen5335[[5]]]
```

```
Out[ ]:= {{56}}
```

```
In[ ]:= insideoutmat.gen5335[[1]].Inverse[insideoutmat] ==
  gen5335[[5]] == davisspmat[[1]].grp533[[56]]
```

```
Out[ ]:= True
```

```
In[ ]:= insideoutmat.gen5335[[2]].Inverse[insideoutmat] == gen5335[[4]] &&
  insideoutmat.gen5335[[3]].Inverse[insideoutmat] == gen5335[[3]] &&
  insideoutmat.gen5335[[4]].Inverse[insideoutmat] == gen5335[[2]]
```

```
Out[ ]:= True
```

So now how about a brute force check?

```
In[ ]:= represent[insideoutmat.davisspmat[[1]].Inverse[insideoutmat].verts5335[[5]]]
Out[ ]:= {5, 84, 48, 69, 39, 114, 6, 83, 51, 74, 36, 117}
```

```
In[ ]:= Apply[Dot, davisspmat[[%]]] == insideoutmat.davisspmat[[1]].Inverse[insideoutmat]
Out[ ]:= True
```

So there's a different way of discovering  $h_0 g_1 h_0^{-1}$  as a word in Davis side pairing map generators. Checking similarly for the conjugate of each other generator  $g_i$  takes some time.

```
In[ ]:= AbsoluteTiming[
  Apply[And, Map[insideoutmat.#.Inverse[insideoutmat] == Apply[Dot, davisspmat[[represent[
    insideoutmat.#.Inverse[insideoutmat].verts5335[[5]]]]]] &, davisspmat]]]
Out[ ]:= {82.4454, True}
```

We have the presentation of  $K$  from inverse pairs and ridge cycles.

```
In[ ]:= Union[davisrelators /. Thread[gen[i_] :=> davisspmat[[i]]]] == {IdentityMatrix[5]}
Out[ ]:= True
```

We have a lift of  $K$  to  $\text{Spin}(4, 1)$ .

```
In[ ]:= Apply[And, MapThread[spinprojection[#1] == #2 &, {davisspmatlift, davisspmat}]]
Out[ ]:= True
```

```
In[ ]:= Union[davisrelators /. Thread[gen[i_] :=> davisspmatlift[[i]]]] == {IdentityMatrix[8]}
Out[ ]:= True
```

```
In[ ]:= MatrixForm[rmattoqmat[formatkappa[davisspmatlift[[1]]]]]
Out[ ]:= MatrixForm=
```

$$\begin{pmatrix} -1 - \tau & \kappa \\ \kappa & -1 - \tau \end{pmatrix}$$

```
In[ ]:= formatkappa[
  toQkappa[qmattormat[{{quaternion[-1 - tau, 0, 0, 0], quaternion[kappa, 0, 0, 0]},
    {quaternion[kappa, 0, 0, 0], quaternion[-1 - tau, 0, 0, 0]}]]]
Out[ ]:= {{-1 - \tau, 0, 0, 0, \kappa, 0, 0, 0}, {0, -1 - \tau, 0, 0, 0, \kappa, 0, 0},
  {0, 0, -1 - \tau, 0, 0, 0, \kappa, 0}, {0, 0, 0, -1 - \tau, 0, 0, 0, \kappa}, {\kappa, 0, 0, 0, -1 - \tau, 0, 0, 0},
  {0, \kappa, 0, 0, 0, -1 - \tau, 0, 0}, {0, 0, \kappa, 0, 0, 0, -1 - \tau, 0}, {0, 0, 0, \kappa, 0, 0, 0, -1 - \tau}}
```

But the group of orientation preserving symmetries of the 120-cell is double covered by a group in spin.

```
In[ ]:= Dimensions[grp533]
Out[ ]:= {7200, 5, 5}
```

```
In[ ]:= Dimensions[grp533lift]
Out[ ]:= {14400, 8, 8}
```

We can choose representative lifts for each o.p. sym. of the 120-cell but these don't form a group, instead we need +/- of these.



```
In[ ]:= grpop533lift == Union[grpop533lift1, -grpop533lift1]
```

```
Out[ ]:= True
```

```
In[ ]:= AbsoluteTiming[Map[spinprojection, grpop533lift1] == grpop533]
```

```
Out[ ]:= {47.5348, True}
```

Brute force conjugating  $g_1$  lift by all of these lifts gives all of the Davis group lift generators.

```
In[ ]:= AbsoluteTiming[
  Sort[davisspmatlift] == Union[Map[#.davisspmatlift[[1]].Inverse[#] &, grpop533lift]]]
```

```
Out[ ]:= {88.407, True}
```

Now what about lifting the inside out symmetry?

```
In[ ]:= spinprojection[insideoutmatlift] == insideoutmat // FullSimplify
```

```
Out[ ]:= True
```

```
In[ ]:= rmattoqmat[insideoutmatlift]
```

```
Out[ ]:= { {i (2.49... + j (0.951... + k (-1.54...), k (-1.67... + (-0.636... + i (2.30...)),
  {i (-2.30... + (-0.636... + k (1.67...), k (1.54... + j (0.951... + i (-2.49...)) }
```

```
In[ ]:= Apply[Union, insideoutmatlift]
```

```
Out[ ]:= {0, (2.49..., (1.54..., (0.951..., (-2.30..., (-1.67...,
  (-0.636..., (1.67..., (2.30..., (-0.951..., (-1.54..., (-2.49... ) }
```

iofieldth

```
In[ ]:= iofieldth = Apply[Union, insideoutmatlift][[-1, 1]]
```

```
Out[ ]:= (4.96...
```

```
In[ ]:= ToNumberField[kappa, iofieldth]
```

```
Out[ ]:= (2.42...
```

```
In[ ]:= ToNumberField[iofieldth, kappa]
```

... ToNumberField: Root[1 - 62 #1<sup>2</sup> - 161 #1<sup>4</sup> - 18 #1<sup>6</sup> + #1<sup>8</sup> &, 4, 0] does not belong to the algebraic number field generated by

$$\sqrt{\frac{1}{2}(5 + 3\sqrt{5})}.$$

```
Out[ ]:= ToNumberField[(4.96...,  $\sqrt{\frac{1}{2}(5 + 3\sqrt{5})}$  )]
```

Unfortunately not in the same  $\mathbb{Q}[\kappa]$  field.

```
In[ ]:= insideoutmatlift.davisspmatlift[[1]].Inverse[insideoutmatlift] ==
  Apply[Dot, davisspmatlift[[ioconjspmat1word]]] // FullSimplify
```

```
Out[ ]:= True
```

By the similar reasoning to the previous analysis this is enough to check that the lift of  $h_0$  normalizes the lift of the Davis manifold group, since

```
In[ ]:= Map[Position[grpop533, #] &,
  {gen5335[[3]].gen5335[[1]], gen5335[[3]].gen5335[[2]], gen5335[[3]].gen5335[[4]]}]
```

```
Out[ ]:= {{4287}}, {{4300}}, {{5440}}}
```

```
In[ ]:= sggen[{gen5335[[3]].gen5335[[1]],
  gen5335[[3]].gen5335[[2]], gen5335[[3]].gen5335[[4]]}] == grpop533
```

```
Out[ ]:= True
```

```
In[ ]:= sggen[grpop533lift1[{{4287, 4300, 5440}}]] == grpop533lift
```

```
Out[ ]:= True
```

```
In[ ]:= Position[grpop533, Inverse[davisspmat[[1]]].gen5335[[3]].gen5335[[5]]]
```

```
Out[ ]:= {{27}}
```

```
In[ ]:= insideoutmatlift.grpop533lift1[[4287]].Inverse[insideoutmatlift] ==
  davisspmatlift[[1]].grpop533lift1[[27]] // FullSimplify
```

```
Out[ ]:= True
```

```
In[ ]:= insideoutmatlift.grpop533lift1[[4300]].Inverse[insideoutmatlift] ==
  grpop533lift1[[5440]] && insideoutmatlift.grpop533lift1[[5440]].
  Inverse[insideoutmatlift] == grpop533lift1[[4300]] // FullSimplify
```

```
Out[ ]:= True
```

So the inside out symmetry lift conjugates generators of the orientation preserving 120-cell symmetry lifts into the Davis manifold group lift times the o.p. 120-cell sym. lifts. So the spin structure on the Davis manifold is symmetric with respect to the lift of the orientation preserving elements in the normalizer of the Davis manifold group (and more generally all elements of the normalizer if we lift to  $\text{Pin}(4, 1)$ ).

Or by brute force

```
In[ ]:= AbsoluteTiming[Apply[And,
  Map[FullSimplify[insideoutmatlift.ToNumberField[davisspmatlift[[#]], iofieldth].
    Inverse[insideoutmatlift] == ToNumberField[Apply[Dot, davisspmatlift[[represent[
      insideoutmat.davisspmat[[#]].Inverse[insideoutmat].verts5335[[5]]]]],
      iofieldth]] &, Range[Length[davisspmat]]]]]
```

```
Out[ ]:= {243.383, True}
```

Some more detail on the inside out matrix lift.

In[ ]:= **spinlift**[insideoutmat]

$$\begin{aligned}
 \text{Out[ ]} = & \left\{ \left\{ 0, \frac{\sqrt{-6.33\dots}}{\sqrt{1.75\dots \times 10^3}^{1/8}}, \frac{\sqrt{2.42\dots}}{\sqrt{1.75\dots \times 10^3}^{1/8}}, \frac{\sqrt{3.91\dots}}{\sqrt{1.75\dots \times 10^3}^{1/8}}, \frac{\sqrt{-1.62\dots}}{\sqrt{1.75\dots \times 10^3}^{1/8}}, \right. \right. \\
 & \frac{\sqrt{-5.85\dots}}{\sqrt{1.75\dots \times 10^3}^{1/8}}, 0, \frac{\sqrt{4.24\dots}}{\sqrt{1.75\dots \times 10^3}^{1/8}}, \left. \left\{ \frac{\sqrt{6.33\dots}}{\sqrt{1.75\dots \times 10^3}^{1/8}}, 0, \frac{\sqrt{-3.91\dots}}{\sqrt{1.75\dots \times 10^3}^{1/8}}, \right. \right. \\
 & \frac{\sqrt{2.42\dots}}{\sqrt{1.75\dots \times 10^3}^{1/8}}, \frac{\sqrt{5.85\dots}}{\sqrt{1.75\dots \times 10^3}^{1/8}}, \frac{\sqrt{-1.62\dots}}{\sqrt{1.75\dots \times 10^3}^{1/8}}, \frac{\sqrt{-4.24\dots}}{\sqrt{1.75\dots \times 10^3}^{1/8}}, 0 \left. \right\}, \\
 & \left\{ \frac{\sqrt{-2.42\dots}}{\sqrt{1.75\dots \times 10^3}^{1/8}}, \frac{\sqrt{3.91\dots}}{\sqrt{1.75\dots \times 10^3}^{1/8}}, 0, \frac{\sqrt{6.33\dots}}{\sqrt{1.75\dots \times 10^3}^{1/8}}, 0, \frac{\sqrt{4.24\dots}}{\sqrt{1.75\dots \times 10^3}^{1/8}}, \right. \\
 & \frac{\sqrt{-1.62\dots}}{\sqrt{1.75\dots \times 10^3}^{1/8}}, \frac{\sqrt{5.85\dots}}{\sqrt{1.75\dots \times 10^3}^{1/8}}, \left. \left\{ \frac{\sqrt{-3.91\dots}}{\sqrt{1.75\dots \times 10^3}^{1/8}}, \frac{\sqrt{-2.42\dots}}{\sqrt{1.75\dots \times 10^3}^{1/8}}, \right. \right. \\
 & \frac{\sqrt{-6.33\dots}}{\sqrt{1.75\dots \times 10^3}^{1/8}}, 0, \frac{\sqrt{-4.24\dots}}{\sqrt{1.75\dots \times 10^3}^{1/8}}, 0, \frac{\sqrt{-5.85\dots}}{\sqrt{1.75\dots \times 10^3}^{1/8}}, \frac{\sqrt{-1.62\dots}}{\sqrt{1.75\dots \times 10^3}^{1/8}} \left. \right\}, \\
 & \left\{ \frac{\sqrt{-1.62\dots}}{\sqrt{1.75\dots \times 10^3}^{1/8}}, \frac{\sqrt{5.85\dots}}{\sqrt{1.75\dots \times 10^3}^{1/8}}, 0, \frac{\sqrt{-4.24\dots}}{\sqrt{1.75\dots \times 10^3}^{1/8}}, 0, \frac{\sqrt{6.33\dots}}{\sqrt{1.75\dots \times 10^3}^{1/8}}, \right. \\
 & \frac{\sqrt{2.42\dots}}{\sqrt{1.75\dots \times 10^3}^{1/8}}, \frac{\sqrt{-3.91\dots}}{\sqrt{1.75\dots \times 10^3}^{1/8}}, \left. \left\{ \frac{\sqrt{-5.85\dots}}{\sqrt{1.75\dots \times 10^3}^{1/8}}, \frac{\sqrt{-1.62\dots}}{\sqrt{1.75\dots \times 10^3}^{1/8}}, \right. \right. \\
 & \frac{\sqrt{4.24\dots}}{\sqrt{1.75\dots \times 10^3}^{1/8}}, 0, \frac{\sqrt{-6.33\dots}}{\sqrt{1.75\dots \times 10^3}^{1/8}}, 0, \frac{\sqrt{3.91\dots}}{\sqrt{1.75\dots \times 10^3}^{1/8}}, \frac{\sqrt{2.42\dots}}{\sqrt{1.75\dots \times 10^3}^{1/8}} \left. \right\}, \\
 & \left\{ 0, \frac{\sqrt{-4.24\dots}}{\sqrt{1.75\dots \times 10^3}^{1/8}}, \frac{\sqrt{-1.62\dots}}{\sqrt{1.75\dots \times 10^3}^{1/8}}, \frac{\sqrt{-5.85\dots}}{\sqrt{1.75\dots \times 10^3}^{1/8}}, \frac{\sqrt{-2.42\dots}}{\sqrt{1.75\dots \times 10^3}^{1/8}}, \right. \\
 & \frac{\sqrt{-3.91\dots}}{\sqrt{1.75\dots \times 10^3}^{1/8}}, 0, \frac{\sqrt{-6.33\dots}}{\sqrt{1.75\dots \times 10^3}^{1/8}}, \left. \left\{ \frac{\sqrt{4.24\dots}}{\sqrt{1.75\dots \times 10^3}^{1/8}}, 0, \frac{\sqrt{5.85\dots}}{\sqrt{1.75\dots \times 10^3}^{1/8}}, \right. \right. \\
 & \frac{\sqrt{-1.62\dots}}{\sqrt{1.75\dots \times 10^3}^{1/8}}, \frac{\sqrt{3.91\dots}}{\sqrt{1.75\dots \times 10^3}^{1/8}}, \frac{\sqrt{-2.42\dots}}{\sqrt{1.75\dots \times 10^3}^{1/8}}, \frac{\sqrt{6.33\dots}}{\sqrt{1.75\dots \times 10^3}^{1/8}}, 0 \left. \right\} \left. \right\}
 \end{aligned}$$

The common denominator is the eighth root of  $512 + 768 \tau$  but this simplifies somewhat.

$\text{In}[*]:= \text{formatkappa}[\text{Simplify}[\text{toQkappa}[(512 + 768 * \tau)^{(-1/4)}]]]$

$$\text{Out}[*]= -\frac{1}{4} + \frac{\tau}{4}$$

*insideoutmatlift2*

$\text{In}[*]:= (\text{insideoutmatlift2} = \text{spinlift}[\text{insideoutmat}] /. \{(\text{toQkappa}[512 + 768 * \tau])^{(-1/8)} \Rightarrow \text{Simplify}[\text{Sqrt}[\text{toQkappa}[4 * (512 + 768 * \tau)^{(-1/4)}]] / 2]\} /. \{x\_AlgebraicNumber \Rightarrow \text{formatkappa}[x]\})$

$$\begin{aligned} \text{Out}[*]= & \left\{ \left\{ \theta, \kappa \left( -\frac{1}{2} - \frac{\tau}{2} \right) \sqrt{-1+\tau}, \frac{1}{2} \kappa \sqrt{-1+\tau}, \frac{1}{2} \kappa \sqrt{-1+\tau} \tau, -\frac{1}{2} \sqrt{-1+\tau} \tau, \right. \right. \\ & \left( -\frac{1}{2} - \frac{3\tau}{2} \right) \sqrt{-1+\tau}, \theta, \sqrt{-1+\tau} \left( \frac{1}{2} + \tau \right) \right\}, \left\{ \kappa \left( \frac{1}{2} + \frac{\tau}{2} \right) \sqrt{-1+\tau}, \theta, -\frac{1}{2} \kappa \sqrt{-1+\tau} \tau, \right. \\ & \frac{1}{2} \kappa \sqrt{-1+\tau}, \sqrt{-1+\tau} \left( \frac{1}{2} + \frac{3\tau}{2} \right), -\frac{1}{2} \sqrt{-1+\tau} \tau, \left( -\frac{1}{2} - \tau \right) \sqrt{-1+\tau}, \theta \right\}, \\ & \left\{ -\frac{1}{2} \kappa \sqrt{-1+\tau}, \frac{1}{2} \kappa \sqrt{-1+\tau} \tau, \theta, \kappa \left( \frac{1}{2} + \frac{\tau}{2} \right) \sqrt{-1+\tau}, \theta, \sqrt{-1+\tau} \left( \frac{1}{2} + \tau \right), \right. \\ & \left. -\frac{1}{2} \sqrt{-1+\tau} \tau, \sqrt{-1+\tau} \left( \frac{1}{2} + \frac{3\tau}{2} \right) \right\}, \left\{ -\frac{1}{2} \kappa \sqrt{-1+\tau} \tau, -\frac{1}{2} \kappa \sqrt{-1+\tau}, \right. \\ & \kappa \left( -\frac{1}{2} - \frac{\tau}{2} \right) \sqrt{-1+\tau}, \theta, \left( -\frac{1}{2} - \tau \right) \sqrt{-1+\tau}, \theta, \left( -\frac{1}{2} - \frac{3\tau}{2} \right) \sqrt{-1+\tau}, -\frac{1}{2} \sqrt{-1+\tau} \tau \right\}, \\ & \left\{ -\frac{1}{2} \sqrt{-1+\tau} \tau, \sqrt{-1+\tau} \left( \frac{1}{2} + \frac{3\tau}{2} \right), \theta, \left( -\frac{1}{2} - \tau \right) \sqrt{-1+\tau}, \theta, \kappa \left( \frac{1}{2} + \frac{\tau}{2} \right) \sqrt{-1+\tau}, \right. \\ & \frac{1}{2} \kappa \sqrt{-1+\tau}, -\frac{1}{2} \kappa \sqrt{-1+\tau} \tau \right\}, \left\{ \left( -\frac{1}{2} - \frac{3\tau}{2} \right) \sqrt{-1+\tau}, -\frac{1}{2} \sqrt{-1+\tau} \tau, \right. \\ & \sqrt{-1+\tau} \left( \frac{1}{2} + \tau \right), \theta, \kappa \left( -\frac{1}{2} - \frac{\tau}{2} \right) \sqrt{-1+\tau}, \theta, \frac{1}{2} \kappa \sqrt{-1+\tau} \tau, \frac{1}{2} \kappa \sqrt{-1+\tau} \right\}, \\ & \left\{ \theta, \left( -\frac{1}{2} - \tau \right) \sqrt{-1+\tau}, -\frac{1}{2} \sqrt{-1+\tau} \tau, \left( -\frac{1}{2} - \frac{3\tau}{2} \right) \sqrt{-1+\tau}, -\frac{1}{2} \kappa \sqrt{-1+\tau}, \right. \\ & \left. -\frac{1}{2} \kappa \sqrt{-1+\tau} \tau, \theta, \kappa \left( -\frac{1}{2} - \frac{\tau}{2} \right) \sqrt{-1+\tau} \right\}, \left\{ \sqrt{-1+\tau} \left( \frac{1}{2} + \tau \right), \theta, \sqrt{-1+\tau} \left( \frac{1}{2} + \frac{3\tau}{2} \right), \right. \\ & \left. -\frac{1}{2} \sqrt{-1+\tau} \tau, \frac{1}{2} \kappa \sqrt{-1+\tau} \tau, -\frac{1}{2} \kappa \sqrt{-1+\tau}, \kappa \left( \frac{1}{2} + \frac{\tau}{2} \right) \sqrt{-1+\tau}, \theta \right\} \end{aligned}$$

$\text{In}[*]:= \text{MatrixForm}[\text{rmattoqmat}[\text{formatkappa}[\text{toQkappa}[\text{insideoutmatlift2} / \text{Sqrt}[\tau - 1]]]]] * \text{Sqrt}[\text{formatkappa}[\text{toQkappa}[(\tau - 1)]]]$

$$\text{Out}[*]= \sqrt{-1+\tau} \begin{pmatrix} \frac{j\kappa}{2} + i\kappa \left( \frac{1}{2} + \frac{\tau}{2} \right) - \frac{\kappa\kappa\tau}{2} & \kappa \left( -\frac{1}{2} - \tau \right) - \frac{\tau}{2} + i \left( \frac{1}{2} + \frac{3\tau}{2} \right) \\ i \left( -\frac{1}{2} - \frac{3\tau}{2} \right) - \frac{\tau}{2} + \kappa \left( \frac{1}{2} + \tau \right) & \frac{j\kappa}{2} + i\kappa \left( -\frac{1}{2} - \frac{\tau}{2} \right) + \frac{\kappa\kappa\tau}{2} \end{pmatrix}$$

```
In[ ]:= MatrixForm[rmattoqmat[formatkappa[toQkappa[insideoutmatlift2 / Sqrt[tau - 1]]]] *
  1 / Sqrt[formatkappa[toQkappa[1 / (tau - 1)]]]
```

$$\text{Out[ ]} = \frac{\begin{pmatrix} \frac{j\kappa}{2} + i\kappa \left( \frac{1}{2} + \frac{\tau}{2} \right) - \frac{k\kappa\tau}{2} & k \left( -\frac{1}{2} - \tau \right) - \frac{\tau}{2} + i \left( \frac{1}{2} + \frac{3\tau}{2} \right) \\ i \left( -\frac{1}{2} - \frac{3\tau}{2} \right) - \frac{\tau}{2} + k \left( \frac{1}{2} + \tau \right) & \frac{j\kappa}{2} + i\kappa \left( -\frac{1}{2} - \frac{\tau}{2} \right) + \frac{k\kappa\tau}{2} \end{pmatrix}}{\sqrt{\tau}}$$

```
In[ ]:= insideoutmatlift2 == insideoutmatlift // FullSimplify
```

```
Out[ ]:= True
```

```
In[ ]:= insideoutmatlift2.insideoutmatlift2 == -IdentityMatrix[8]
```

```
Out[ ]:= True
```

So the inside out matrix lift is order 4.

## Binary icosahedral group

We are especially interested in the binary icosahedral group in the symmetry group of the 120-cell (two mirror image versions conjugate by an orientation reversing symmetry of the 120-cell).

pgen1

```
In[ ]:= pgen1 = Select[grp533,
  #.Transpose[v4orbit[{{1, 8, 9, 10}}]] == Transpose[v4orbit[{{2, 3, 5, 4}}]] &][[1]];
```

pgen2

```
In[ ]:= pgen2 = Select[grp533,
  #.Transpose[v4orbit[{{1, 6, 7, 10}}]] == Transpose[v4orbit[{{3, 4, 2, 8}}]] &][[1]];
```

pgen1lift, pgen2lift

```
In[ ]:= {pgen1lift, pgen2lift} = toQkappa[Map[spinlift, {pgen1, pgen2}]];
```

Generate this subgroup in order corresponding to the ordering of sides, since this group acts transitively on sides.

pgrp

```
In[ ]:= Dimensions[pgrp =
  SortBy[Map[#, #.verts5335[[4]] /. v4indrules] &, sggen[{pgen1, pgen2}]], #[[2]] &][[
  All, 1]]]
```

```
Out[ ]:= {120, 5, 5}
```

```
In[ ]:= Map[#.verts5335[[4]] &, pgrp] == v4orbit
```

```
Out[ ]:= True
```

The elements of the 533 group are thus all represented by a product of a binary icosahedral group and the stabilizer of  $v_4$  and  $v_5$ .

stab45

```
In[ ]:= Dimensions[stab45 = sggen[gen5335[[1 ;; 3]]]]
```

```
Out[ ]:= {120, 5, 5}
```

```
In[ ]:= grp533 == Apply[Union, Outer[Dot, pgrp, stab45, 1]]
```

```
Out[ ]:= True
```

*pgrpppgrplift*

```
In[ ]:= Dimensions[pgrpppgrplift = sgpairsgen[{{pgen1, pgen1lift}, {pgen2, pgen2lift}}]]
```

```
Out[ ]:= {120, 2}
```

*pgrplift*

```
In[ ]:= Dimensions[pgrplift = pgrp /. Thread[Apply[Rule, Transpose[pgrpppgrplift]]]]
```

```
Out[ ]:= {120, 8, 8}
```

The lift consists of 2x2 quaternion matrices  $\text{diag}(q, 1)$ , for the binary icosahedral group represented by unit quaternions.

```
In[ ]:= {Tally[Map[rmattoqmat, pgrplift][[All, 2, 2]]],
  Tally[Map[rmattoqmat, pgrplift][[All, 1, 2]]],
  Tally[Map[rmattoqmat, pgrplift][[All, 2, 1]]]}
```

```
Out[ ]:= {{1, 120}}, {{0, 120}}, {{0, 120}}
```

*pquats*

```
In[ ]:= pquats = Map[rmattoqmat, pgrplift][[All, 1, 1]];
```

These quaternions are in turn represented by 2x2 complex matrices.

*gamma*

```
In[ ]:= gamma = ToNumberField[{I, tau}][[1, 1]]
```

```
Out[ ]:= 2.24... + 1.00... i
```

*pcomplex*

```
In[ ]:= pcomplex = Map[ToNumberField[fromcomplex[quaterniontomatrix[#]], gamma] &, pquats];
```

```
In[ ]:= sggen[
  Map[ToNumberField[fromcomplex[quaterniontomatrix[rmattoqmat[#][[1, 1]]]], gamma] &,
  {pgen1, pgen2}]] == Sort[pcomplex]
```

```
Out[ ]:= True
```

*pquatmats*

```
In[ ]:= pquatmats = Map[quaterniontomatrix, pquats];
```

*pquatmatsconjclasses*

```
In[ ]:= Map[Dimensions, pquatmatsconjclasses =
  SortBy[conjclasses[pquatmats], {elementorder[#[[1]]], Length[#]} &]]
```

```
Out[ ]:= {{1, 4, 4}, {1, 4, 4}, {20, 4, 4}, {30, 4, 4},
  {12, 4, 4}, {12, 4, 4}, {20, 4, 4}, {12, 4, 4}, {12, 4, 4}}
```

```
In[ ]:= Map[Union, Map[elementorder, pquatmatsconjclasses, {2}]]
```

```
Out[ ]:= {{1}, {2}, {3}, {4}, {5}, {5}, {6}, {10}, {10}}
```

*pcomplexconjclasses*

```
In[ ]:= Map[Dimensions, pcomplexconjclasses = conjclasses[pcomplex]]
```

```
Out[ ]:= {{1, 2, 2}, {1, 2, 2}, {12, 2, 2}, {12, 2, 2},
  {12, 2, 2}, {12, 2, 2}, {20, 2, 2}, {20, 2, 2}, {30, 2, 2}}
```

```
In[ ]:= Map[Union, Map[elementorder, pcomplexconjclasses, {2}]]
```

```
Out[ ]:= {{2}, {1}, {5}, {5}, {10}, {10}, {3}, {6}, {4}}
```

```
In[ ]:= RootReduce[Map[Union, Map[Tr, pcomplexconjclasses, {2}]]]
```

```
Out[ ]:= {{-2}, {2}, {1/2 (-1 - sqrt(5))}, {1/2 (-1 + sqrt(5))}, {1/2 (1 - sqrt(5))}, {1/2 (1 + sqrt(5))}, {-1}, {1}, {0}}
```

pbargen1, pbargen2

```
In[ ]:= {pbargen1, pbargen2} = Map[Inverse[gen533[[1]]].#.gen533[[1]] &, {pgen1, pgen2}];
```

pbargrp

```
In[ ]:= Dimensions[pbargrp = pgrp /.  
Thread[Apply[Rule, Transpose[sgpairsngen[{{pgen1, pbargen1}, {pgen2, pbargen2}}]]]]]
```

```
Out[ ]:= {120, 5, 5}
```

pbargen1lift, pbargen2lift

```
In[ ]:= {pbargen1lift, pbargen2lift} = toQkappa[-Map[spinlift, {pbargen1, pbargen2}]]];
```

pbargrppbargrplift

```
In[ ]:= Dimensions[  
pbargrppbargrplift = sgpairsngen[{{pbargen1, pbargen1lift}, {pbargen2, pbargen2lift}}, 10]]
```

```
Out[ ]:= {120, 2}
```

pbargrplift

```
In[ ]:= Dimensions[pbargrplift = pbargrp /. Thread[Apply[Rule, Transpose[pbargrppbargrplift]]]]]
```

```
Out[ ]:= {120, 8, 8}
```

```
In[ ]:= {Tally[Map[rmattoqmat, pbargrplift][[All, 1, 1]]],  
Tally[Map[rmattoqmat, pbargrplift][[All, 1, 2]]],  
Tally[Map[rmattoqmat, pbargrplift][[All, 2, 1]]]}
```

```
Out[ ]:= {{{1, 120}}, {{0, 120}}, {{0, 120}}}
```

pbarquats

```
In[ ]:= pbarquats = Map[rmattoqmat, pbargrplift][[All, 2, 2]];
```

```
In[ ]:= Map[Apply[List, #] * {1, -1, -1, 1} &, pbarquats] == Map[Apply[List, #] &, pquats]
```

```
Out[ ]:= True
```

```
In[ ]:= Apply[List, matrixtoquaternion[quaterniontomatrix[quaternion[a, -b, -c, d]].  
quaterniontomatrix[quaternion[w, -x, -y, z]]] * {1, -1, -1, 1} -  
Apply[List, matrixtoquaternion[quaterniontomatrix[quaternion[a, b, c, d]].  
quaterniontomatrix[quaternion[w, x, y, z]]]]]
```

```
Out[ ]:= {0, 0, 0, 0}
```

pbarcomplex

```
In[ ]:= pbarcomplex = Map[ToNumberField[fromcomplex[quaterniontocmatrix[#]], gamma] &, pbarquats];
```

```
In[ ]:= RootReduce[Map[Union, Map[Tr, pcomplexconjclasses, {2}]]]
```

```
Out[ ]:= {{-2}, {2}, {1/2 (-1 - sqrt(5))}, {1/2 (-1 + sqrt(5))}, {1/2 (1 - sqrt(5))}, {1/2 (1 + sqrt(5))}, {-1}, {1}, {0}}
```

```
In[ ]:= RootReduce[Map[Union, Map[Tr, pcomplexconjclasses /. Thread[pcomplex → pbarcomplex], {2}]]]
```

```
Out[ ]:= {{-2}, {2}, {1/2 (-1 - Sqrt[5])}, {1/2 (-1 + Sqrt[5])}, {1/2 (1 - Sqrt[5])}, {1/2 (1 + Sqrt[5])}, {-1}, {1}, {0}}
```

```
In[ ]:= % == %%
```

```
Out[ ]:= True
```

The correspondence between the lifts of the left and right hand binary icosahedral group is thus  $\text{diag}(a + bi + cj + dk, 1) \rightarrow \text{diag}(1, a - bi - cj + dk)$ , which doesn't change the character.

```
In[ ]:= Union[pquats] == Union[Map[Apply[quaternion, #] &, Apply[Union,
  Map[Permutations, Tuples[{{-1, 1}, {0}, {0}, {0}}]]], Map[Apply[quaternion, #] &,
  Apply[Union, Map[Permutations, Tuples[{{-1, 1}, {-1, 1}, {-1, 1}, {-1, 1}} / 2]]],
  Map[Apply[quaternion, #] &, Apply[Union,
    Outer[#1[[#2]] &, Tuples[toQkappa[{{0}, {-1, 1}, {-tau, tau}, {-1/tau, 1/tau}} / 2]],
    Select[Permutations[Range[4]], Signature[#] == 1 &, 1]]]]]
```

```
Out[ ]:= True
```

```
In[ ]:= formatkappa[2 * pgen1] // MatrixForm
```

```
Out[ ]//MatrixForm=
```

$$\begin{pmatrix} \tau & -1 & 1-\tau & 0 & 0 \\ 1 & \tau & 0 & -1+\tau & 0 \\ -1+\tau & 0 & \tau & -1 & 0 \\ 0 & 1-\tau & 1 & \tau & 0 \\ 0 & 0 & 0 & 0 & 2 \end{pmatrix}$$

```
In[ ]:= formatkappa[2 * pgen2] // MatrixForm
```

```
Out[ ]//MatrixForm=
```

$$\begin{pmatrix} \tau & -1 & -1+\tau & 0 & 0 \\ 1 & \tau & 0 & 1-\tau & 0 \\ 1-\tau & 0 & \tau & -1 & 0 \\ 0 & -1+\tau & 1 & \tau & 0 \\ 0 & 0 & 0 & 0 & 2 \end{pmatrix}$$

```
alpha1hat, alpha2hat
```

```
In[ ]:= alpha1hat = pgen1lift;
alpha2hat = pgen2lift;
```

```
In[ ]:= rmattoqmat[formatkappa[pgen1lift]] // MatrixForm
```

```
Out[ ]//MatrixForm=
```

$$\begin{pmatrix} \frac{i}{2} + j \left( -\frac{1}{2} + \frac{\tau}{2} \right) + \frac{\tau}{2} & 0 \\ 0 & 1 \end{pmatrix}$$

```
In[ ]:= rmattoqmat[formatkappa[pgen2lift]] // MatrixForm
```

```
Out[ ]//MatrixForm=
```

$$\begin{pmatrix} \frac{i}{2} + j \left( \frac{1}{2} - \frac{\tau}{2} \right) + \frac{\tau}{2} & 0 \\ 0 & 1 \end{pmatrix}$$



In[ ]:= **FullSimplify[Eigensystem[RootReduce[pgen1]]]**

Out[ ]:=  $\left\{ \{1, (-1)^{1/5}, (-1)^{1/5}, -(-1)^{4/5}, -(-1)^{4/5}\}, \right.$   
 $\left\{ \{0, 0, 0, 0, 1\}, \left\{ \frac{1}{2}(1 + \sqrt{5}), \sqrt{-1.90... i}, 0, 1, 0 \right\}, \left\{ \sqrt{1.90... i}, \frac{1}{2}(1 + \sqrt{5}), 1, 0, 0 \right\}, \right.$   
 $\left. \left\{ \frac{1}{2}(1 + \sqrt{5}), \sqrt{1.90... i}, 0, 1, 0 \right\}, \left\{ \sqrt{-1.90... i}, \frac{1}{2}(1 + \sqrt{5}), 1, 0, 0 \right\} \right\}$

trymat1a

In[ ]:= **trymat1a = Transpose[FullSimplify[**  
**Append[{%[[2, 2]] + %[2, 4]], %[2, 3]] + %[2, 5]], (%[[2, 2]] - %[2, 4]) / I,**  
**(%[[2, 3]] - %[2, 5]) / I} / Sqrt[2 (5 + Sqrt[5])], %[2, 1]]]**

Out[ ]:=  $\left\{ \left\{ \sqrt{\frac{1}{10}(5 + \sqrt{5})}, 0, 0, 1, 0 \right\}, \left\{ 0, \sqrt{\frac{1}{10}(5 + \sqrt{5})}, -1, 0, 0 \right\}, \right.$   
 $\left. \left\{ 0, \sqrt{\frac{2}{5 + \sqrt{5}}}, 0, 0, 0 \right\}, \left\{ \sqrt{\frac{2}{5 + \sqrt{5}}}, 0, 0, 0, 0 \right\}, \{0, 0, 0, 0, 1\} \right\}$

trymat1b

In[ ]:= **trymat1b = Transpose[**  
**FullSimplify[Append[Map[# / Sqrt[1dot[#, #]] &, {trymat1a[[All, 1]] + trymat1a[[All, 4]],**  
**trymat1a[[All, 2]] + trymat1a[[All, 3]], trymat1a[[All, 2]] - trymat1a[[All, 3]],**  
**trymat1a[[All, 1]] - trymat1a[[All, 4]]}], trymat1a[[All, 5]]]**

Out[ ]:=  $\left\{ \left\{ \frac{1}{2} \sqrt{2 + \sqrt{2 + \frac{2}{\sqrt{5}}}}, 0, 0, -\frac{1}{2} \sqrt{2 - \sqrt{2 + \frac{2}{\sqrt{5}}}}, 0 \right\}, \right.$   
 $\left\{ 0, -\frac{1}{2} \sqrt{2 - \sqrt{2 + \frac{2}{\sqrt{5}}}}, \frac{1}{2} \sqrt{2 + \sqrt{2 + \frac{2}{\sqrt{5}}}}, 0, 0 \right\},$   
 $\left\{ 0, \frac{1}{2} \sqrt{2 + \sqrt{2 + \frac{2}{\sqrt{5}}}}, \frac{1}{2} \sqrt{2 - \sqrt{2 + \frac{2}{\sqrt{5}}}}, 0, 0 \right\},$   
 $\left. \left\{ \frac{1}{2} \sqrt{2 - \sqrt{2 + \frac{2}{\sqrt{5}}}}, 0, 0, \frac{1}{2} \sqrt{2 + \sqrt{2 + \frac{2}{\sqrt{5}}}}, 0 \right\}, \{0, 0, 0, 0, 1\} \right\}$

trymat1c

In[ ]:= **trymat1c = trymat1b[[All, {1, 3, 2, 4, 5}]];**

In[ ]:= **Transpose[trymat1c].jmat[4].trymat1c == jmat[4] // FullSimplify**

Out[ ]:= **True**

In[ ]:= **Det[trymat1c] // FullSimplify**

Out[ ]:= **1**

```
In[ ]:= Inverse[trymat1c].pgen1.trymat1c // FullSimplify // MatrixForm
```

```
Out[ ]:= MatrixForm=
```

$$\begin{pmatrix} \frac{1}{4}(1+\sqrt{5}) & -0.588... & 0 & 0 & 0 \\ \frac{1}{4}\sqrt{10-2\sqrt{5}} & \frac{1}{4}(1+\sqrt{5}) & 0 & 0 & 0 \\ 0 & 0 & \frac{1}{4}(1+\sqrt{5}) & -0.588... & 0 \\ 0 & 0 & \frac{1}{4}\sqrt{10-2\sqrt{5}} & \frac{1}{4}(1+\sqrt{5}) & 0 \\ 0 & 0 & 0 & 0 & 1 \end{pmatrix}$$

```
rhtwist
```

```
In[ ]:= MatrixForm[rhtwist =
```

```
FullSimplify[{Cos[Pi/5], -Sin[Pi/5], 0, 0, 0}, {Sin[Pi/5], Cos[Pi/5], 0, 0, 0},  
{0, 0, Cos[Pi/5], -Sin[Pi/5], 0}, {0, 0, Sin[Pi/5], Cos[Pi/5], 0}, {0, 0, 0, 0, 1}]]
```

```
Out[ ]:= MatrixForm=
```

$$\begin{pmatrix} \frac{1}{4}(1+\sqrt{5}) & -0.588... & 0 & 0 & 0 \\ \sqrt{\frac{5}{8}-\frac{\sqrt{5}}{8}} & \frac{1}{4}(1+\sqrt{5}) & 0 & 0 & 0 \\ 0 & 0 & \frac{1}{4}(1+\sqrt{5}) & -0.588... & 0 \\ 0 & 0 & \sqrt{\frac{5}{8}-\frac{\sqrt{5}}{8}} & \frac{1}{4}(1+\sqrt{5}) & 0 \\ 0 & 0 & 0 & 0 & 1 \end{pmatrix}$$

```
In[ ]:= Transpose[rhtwist].jmat[4].rhtwist == jmat[4] // FullSimplify
```

```
Out[ ]:= True
```

```
In[ ]:= Inverse[trymat1c].pgen1.trymat1c == rhtwist // FullSimplify
```

```
Out[ ]:= True
```

```
In[ ]:= pgen2 = DiagonalMatrix[{1, 1, -1, -1, 1}].pgen1.DiagonalMatrix[{1, 1, -1, -1, 1}]
```

```
Out[ ]:= True
```

```
trymat2c
```

```
In[ ]:= trymat2c = DiagonalMatrix[{1, 1, -1, -1, 1}].trymat1c;
```

```
In[ ]:= Transpose[trymat2c].jmat[4].trymat2c == jmat[4] // FullSimplify
```

```
Out[ ]:= True
```

```
In[ ]:= Det[trymat2c] // FullSimplify
```

```
Out[ ]:= 1
```

```
In[ ]:= Inverse[trymat2c].pgen2.trymat2c == rhtwist // FullSimplify
```

```
Out[ ]:= True
```

```
In[ ]:= pbargen1 = DiagonalMatrix[{1, 1, 1, -1, 1}].pgen1.DiagonalMatrix[{1, 1, 1, -1, 1}]
```

```
Out[ ]:= True
```

```
In[ ]:= pbargen2 == DiagonalMatrix[{1, 1, 1, -1, 1}].pgen2.DiagonalMatrix[{1, 1, 1, -1, 1}]
```

```
Out[ ]:= True
```

```
In[ ]:= formatkappa[2 *  
  (DiagonalMatrix[{-1, 1, 1, 1, 1}].pgen1.DiagonalMatrix[{-1, 1, 1, 1, 1}])] // MatrixForm
```

```
Out[ ]//MatrixForm=
```

$$\begin{pmatrix} \tau & 1 & -1 + \tau & 0 & 0 \\ -1 & \tau & 0 & -1 + \tau & 0 \\ 1 - \tau & 0 & \tau & -1 & 0 \\ 0 & 1 - \tau & 1 & \tau & 0 \\ 0 & 0 & 0 & 0 & 2 \end{pmatrix}$$

```
In[ ]:= formatkappa[2 *  
  (DiagonalMatrix[{-1, 1, 1, 1, 1}].pgen2.DiagonalMatrix[{-1, 1, 1, 1, 1}])] // MatrixForm
```

```
Out[ ]//MatrixForm=
```

$$\begin{pmatrix} \tau & 1 & 1 - \tau & 0 & 0 \\ -1 & \tau & 0 & 1 - \tau & 0 \\ -1 + \tau & 0 & \tau & -1 & 0 \\ 0 & -1 + \tau & 1 & \tau & 0 \\ 0 & 0 & 0 & 0 & 2 \end{pmatrix}$$

```
In[ ]:= rmattoqmat[formatkappa[-reflectionlift[{1, 0, 0, 0, 0}].  
  pgen1lift.reflectionlift[{1, 0, 0, 0, 0}]]] // MatrixForm
```

```
Out[ ]//MatrixForm=
```

$$\begin{pmatrix} 1 & 0 \\ 0 & \frac{i}{2} + j \left( -\frac{1}{2} + \frac{\tau}{2} \right) + \frac{\tau}{2} \end{pmatrix}$$

```
In[ ]:= rmattoqmat[formatkappa[-reflectionlift[{1, 0, 0, 0, 0}].  
  pgen2lift.reflectionlift[{1, 0, 0, 0, 0}]]] // MatrixForm
```

```
Out[ ]//MatrixForm=
```

$$\begin{pmatrix} 1 & 0 \\ 0 & \frac{i}{2} + j \left( \frac{1}{2} - \frac{\tau}{2} \right) + \frac{\tau}{2} \end{pmatrix}$$

```
beta1hat, beta2hat
```

```
In[ ]:= beta1hat = -reflectionlift[{1, 0, 0, 0, 0}].pgen1lift.reflectionlift[{1, 0, 0, 0, 0}];  
  beta2hat = -reflectionlift[{1, 0, 0, 0, 0}].pgen2lift.reflectionlift[{1, 0, 0, 0, 0}];
```

```
In[ ]:= rmattoqmat[formatkappa[beta1hat]] // MatrixForm
```

```
Out[ ]//MatrixForm=
```

$$\begin{pmatrix} 1 & 0 \\ 0 & \frac{i}{2} + j \left( -\frac{1}{2} + \frac{\tau}{2} \right) + \frac{\tau}{2} \end{pmatrix}$$

```
In[ ]:= rmattoqmat[formatkappa[beta2hat]] // MatrixForm
```

```
Out[ ]//MatrixForm=
```

$$\begin{pmatrix} 1 & 0 \\ 0 & \frac{i}{2} + j \left( \frac{1}{2} - \frac{\tau}{2} \right) + \frac{\tau}{2} \end{pmatrix}$$

---

## The lift of the orientation preserving symmetry group of

## the Davis manifold

We have generators of the normalizer  $N$  of the Davis manifold group  $K$  and we understand symmetries of the Davis manifold in terms of elements of the group  $N/K$  of order 28800. Take representatives for  $N/K$  of the form  $h$  or  $hh_0$  for  $h$  in the symmetry group of the 120-cell, so  $v_5$  is either fixed or carried to  $v_1$ . We will restrict now to symmetries that are orientation preserving, a group  $N_0/K$  of order 14400, and consider the lift to  $\text{Spin}(4, 1)$  which is a group  $\hat{N}_0/\hat{K}$  of order 28800 double covering the orientation preserving symmetries  $N_0/K$  of the Davis manifold. Represent each element of this group as  $\hat{h}$  or  $\hat{h}\hat{h}_0$  for a fixed choice of lift  $\hat{h}_0$  and  $\hat{h}$  one of the two lifts of an orientation preserving symmetry  $h$  of the 120-cell. To multiply symmetry group elements we need to precompute the indices in the double cover of the orientation preserving subgroup of the 533 group representing elements  $\hat{h}_0\hat{h}\hat{h}_0^{-1}$  modulo  $\hat{K}$ .

```
In[ ]:= Dimensions[grp533lift]
```

```
Out[ ]:= {14400, 8, 8}
```

```
In[ ]:= {Tally[Map[rmattoqmat, grp533lift][[All, 1, 2]]],
  Tally[Map[rmattoqmat, grp533lift][[All, 2, 1]]]}
```

```
Out[ ]:= {{0, 14400}}, {{0, 14400}}
```

```
In[ ]:= Union[Map[rmattoqmat, grp533lift][[All, 1, 1]] == Union[pquats]
```

```
Out[ ]:= True
```

```
In[ ]:= Union[Map[rmattoqmat, grp533lift][[All, 2, 2]] == Union[pquats]
```

```
Out[ ]:= True
```

```
In[ ]:= Union[Map[rmattoqmat, grp533lift]] == Apply[Union,
  Outer[{{#1, quaternion[0, 0, 0, 0]}, {quaternion[0, 0, 0, 0], #2}} &, pquats, 1]]
```

```
Out[ ]:= True
```

So in fact we can do better by taking the lift of the orientation preserving symmetries of the 120-cell as a direct product of subgroups of elements of the form  $\text{diag}(q,1)$  and the form  $\text{diag}(1,q)$  and so we can build a table of how  $\hat{h}_0$  conjugates each of these subgroups. Unfortunately, we have to determine the element of the lift of the Davis manifold group that carries us back to an element in this group. We figure the word in generators of the Davis group downstairs and take the corresponding lifts.

*pquatsrules*

```
In[ ]:= pquatsrules = Thread[pquats → Range[Length[pquats]]];
```

*pquatsio, pquatsiorules*

```
In[ ]:= pquatsio = Map[ToNumberField[#, iofieldth] &, pquats, {2}];
pquatsiorules = Thread[pquatsio → Range[Length[pquatsio]]];
```

*pquatmatsrules*

```
In[ ]:= pquatmatsrules = Thread[pquatmats → Range[Length[pquatmats]]];
```

*pquatmatsio, pquatmatsiorules*

```
In[ ]:= pquatmatsio = Map[ToNumberField[#, iofieldth] &, pquatmats, {2}];
pquatmatsiorules = Thread[pquatmatsio → Range[Length[pquatmatsio]]];
```

In[ ]:= **Position**[pgrp, pgen1]

Out[ ]:= { {119} }

In[ ]:= **Position**[pgrp, pgen2]

Out[ ]:= { {118} }

In[ ]:= **sggen**[pquatmatsio[ [ {119, 118} ] ] ] == **Union**[pquatmatsio]

Out[ ]:= **True**

In[ ]:= **Union**[**Map**[**matrixtoquaternion**, **sggen**[**Map**[**quaterniontomatrix**, **pquatsio**[ [ {119, 118} ] ] ] ] ] ] == **Union**[**pquatsio**]

Out[ ]:= **True**

In[ ]:= **121 - Reverse**[**representmat**[**toQkappa**[**RootReduce**[**insideoutmat**.**pgen1**.**insideoutmat**] ] ] ]

Out[ ]:= { 74, 36, 117 }

In[ ]:= **Apply**[**Dot**, **davisspmat**[ [ {74, 36, 117} ] ] ] .  
**toQkappa**[**RootReduce**[**insideoutmat**.**pgen1**.**insideoutmat**] ]

Out[ ]:=  $\left\{ \left\{ \sqrt{-0.309...}, \sqrt{0.809...}, \frac{1}{2}, 0, 0 \right\}, \left\{ \sqrt{-0.809...}, \sqrt{-0.309...}, 0, \frac{1}{2}, 0 \right\}, \right.$   
 $\left. \left\{ -\frac{1}{2}, 0, \sqrt{-0.309...}, \sqrt{-0.809...}, 0 \right\}, \left\{ 0, -\frac{1}{2}, \sqrt{0.809...}, \sqrt{-0.309...}, 0 \right\}, \{0, 0, 0, 0, 1\} \right\}$

In[ ]:= **121 - Reverse**[**representmat**[**toQkappa**[**RootReduce**[**insideoutmat**.**pgen2**.**insideoutmat**] ] ] ]

Out[ ]:= { 93, 22, 117 }

In[ ]:= **Apply**[**Dot**, **davisspmat**[ [ {93, 22, 117} ] ] ] .  
**toQkappa**[**RootReduce**[**insideoutmat**.**pgen2**.**insideoutmat**] ]

Out[ ]:=  $\left\{ \left\{ \sqrt{-0.309...}, \sqrt{-0.809...}, \frac{1}{2}, 0, 0 \right\}, \left\{ \sqrt{0.809...}, \sqrt{-0.309...}, 0, \frac{1}{2}, 0 \right\}, \right.$   
 $\left. \left\{ -\frac{1}{2}, 0, \sqrt{-0.309...}, \sqrt{0.809...}, 0 \right\}, \left\{ 0, -\frac{1}{2}, \sqrt{-0.809...}, \sqrt{-0.309...}, 0 \right\}, \{0, 0, 0, 0, 1\} \right\}$

In[ ]:= **rmattoqmat**[**pgen1lift**]

Out[ ]:=  $\left\{ \left\{ \frac{i}{2} + j \sqrt{0.309...} + \sqrt{0.809...}, 0 \right\}, \{0, 1\} \right\}$

*pgen1liftconj*

In[ ]:= **rmattoqmat**[**pgen1liftconj** = **Apply**[**Dot**, **davisspmatlift**[ [ {74, 36, 117} ] ] ] ] .  
**toQkappa**[**RootReduce**[**insideoutmatlift**.**pgen1lift**.**Inverse**[**insideoutmatlift**] ] ] ]

Out[ ]:=  $\left\{ \{1, 0\}, \left\{ 0, \frac{j}{2} + i \sqrt{0.809...} + \sqrt{-0.309...} \right\} \right\}$

In[ ]:= **rmattoqmat**[**pgen2lift**]

Out[ ]:=  $\left\{ \left\{ \frac{i}{2} + \sqrt{0.809...} + j \sqrt{-0.309...}, 0 \right\}, \{0, 1\} \right\}$

pgen2liftconj

```
In[ ]:= rmattoqmat[pgen2liftconj = Apply[Dot, davisspmatlift[{{93, 22, 117}}]]].
      toQkappa[RootReduce[insideoutmatlift.pgen2lift.Inverse[insideoutmatlift]]]]
```

Out[ ]:=  $\left\{ \{1, 0\}, \left\{0, \frac{j}{2} + i \left( \sqrt{-0.809...} + \sqrt{-0.309...} \right) \right\} \right\}$

```
In[ ]:= pgen1liftconj == MatrixPower[beta1hat, 3]
```

Out[ ]:= True

```
In[ ]:= pgen2liftconj == MatrixPower[beta2hat, 7]
```

Out[ ]:= True

```
In[ ]:= spinprojection[pgen1liftconj]
```

Out[ ]:=  $\left\{ \left\{ \sqrt{-0.309...}, \sqrt{0.809...}, \frac{1}{2}, 0, 0 \right\}, \left\{ \sqrt{-0.809...}, \sqrt{-0.309...}, 0, \frac{1}{2}, 0 \right\}, \right.$   
 $\left. \left\{ -\frac{1}{2}, 0, \sqrt{-0.309...}, \sqrt{-0.809...}, 0 \right\}, \left\{ 0, -\frac{1}{2}, \sqrt{0.809...}, \sqrt{-0.309...}, 0 \right\}, \{0, 0, 0, 0, 1\} \right\}$

```
In[ ]:= MatrixPower[pbargen1, 7]
```

Out[ ]:=  $\left\{ \left\{ \sqrt{-0.309...}, \sqrt{0.809...}, \frac{1}{2}, 0, 0 \right\}, \left\{ \sqrt{-0.809...}, \sqrt{-0.309...}, 0, \frac{1}{2}, 0 \right\}, \right.$   
 $\left. \left\{ -\frac{1}{2}, 0, \sqrt{-0.309...}, \sqrt{-0.809...}, 0 \right\}, \left\{ 0, -\frac{1}{2}, \sqrt{0.809...}, \sqrt{-0.309...}, 0 \right\}, \{0, 0, 0, 0, 1\} \right\}$

```
In[ ]:= % == %%
```

Out[ ]:= True

```
In[ ]:= spinprojection[pgen2liftconj]
```

Out[ ]:=  $\left\{ \left\{ \sqrt{-0.309...}, \sqrt{-0.809...}, \frac{1}{2}, 0, 0 \right\}, \left\{ \sqrt{0.809...}, \sqrt{-0.309...}, 0, \frac{1}{2}, 0 \right\}, \right.$   
 $\left. \left\{ -\frac{1}{2}, 0, \sqrt{-0.309...}, \sqrt{0.809...}, 0 \right\}, \left\{ 0, -\frac{1}{2}, \sqrt{-0.809...}, \sqrt{-0.309...}, 0 \right\}, \{0, 0, 0, 0, 1\} \right\}$

```
In[ ]:= MatrixPower[pbargen2, 3]
```

Out[ ]:=  $\left\{ \left\{ \sqrt{-0.309...}, \sqrt{-0.809...}, \frac{1}{2}, 0, 0 \right\}, \left\{ \sqrt{0.809...}, \sqrt{-0.309...}, 0, \frac{1}{2}, 0 \right\}, \right.$   
 $\left. \left\{ -\frac{1}{2}, 0, \sqrt{-0.309...}, \sqrt{0.809...}, 0 \right\}, \left\{ 0, -\frac{1}{2}, \sqrt{-0.809...}, \sqrt{-0.309...}, 0 \right\}, \{0, 0, 0, 0, 1\} \right\}$

```
In[ ]:= % == %%
```

Out[ ]:= True

So  $\hat{h}_0 \text{diag}(q, 1) \hat{h}_0^{-1} = \text{diag}(1, \alpha(q))$  modulo  $\hat{K}$  for an automorphism  $\alpha$  of the binary icosahedral group which is not an inner automorphism.

pquatsalphaauto

```
In[ ]:= Dimensions[pquatsalphaauto =  
  Map[matrixtoquaternion, sgpairsgen[{{quaterniontomatrix[rmattoqmat[pgen1lift][[1, 1]]],  
    quaterniontomatrix[rmattoqmat[pgen1liftconj][[2, 2]]]},  
    {quaterniontomatrix[rmattoqmat[pgen2lift][[1, 1]]],  
    quaterniontomatrix[rmattoqmat[pgen2liftconj][[2, 2]]]}}, {2}]]
```

Out[ ]:= {120, 2}

pquatsalphaautoperm

```
In[ ]:= pquatsalphaautoperm = Sort[pquatsalphaauto /. pquatsrules][[All, 2]];
```

```
In[ ]:= pquatsalphaautoperm[[pquatsalphaautoperm]][[pquatsalphaautoperm]][[  
  pquatsalphaautoperm]] == Range[120]
```

Out[ ]:= True

```
In[ ]:= Select[pquatmats, #.pquatmats[[2]].Inverse[#] == pquatmats[[pquatsalphaautoperm[[2]]]] &]
```

Out[ ]:= {}

```
In[ ]:= Select[pquats,  
  quaterniontomatrix[#].quaterniontomatrix[pquats[[2]]].Inverse[quaterniontomatrix[#]] ==  
  quaterniontomatrix[pquats[[pquatsalphaautoperm[[2]]]]] &]
```

Out[ ]:= {}

```
In[ ]:= 121 - Reverse[representmat[toQkappa[RootReduce[insideoutmat.pbargen1.insideoutmat]]]]
```

Out[ ]:= {91, 24, 117}

```
In[ ]:= Apply[Dot, davisspmat[{{91, 24, 117}}]].  
  toQkappa[RootReduce[insideoutmat.pbargen1.insideoutmat]]
```

Out[ ]:=  $\left\{ \left\{ \sqrt{-0.309...}, \sqrt{-0.809...}, -\frac{1}{2}, 0, 0 \right\}, \left\{ \sqrt{0.809...}, \sqrt{-0.309...}, 0, \frac{1}{2}, 0 \right\}, \right.$   
 $\left. \left\{ \frac{1}{2}, 0, \sqrt{-0.309...}, \sqrt{-0.809...}, 0 \right\}, \left\{ 0, -\frac{1}{2}, \sqrt{0.809...}, \sqrt{-0.309...}, 0 \right\}, \{0, 0, 0, 0, 1\} \right\}$

```
In[ ]:= 121 - Reverse[representmat[toQkappa[RootReduce[insideoutmat.pbargen2.insideoutmat]]]]
```

Out[ ]:= {72, 36, 117}

```
In[ ]:= Apply[Dot, davisspmat[{{72, 36, 117}}]].  
  toQkappa[RootReduce[insideoutmat.pbargen2.insideoutmat]]
```

Out[ ]:=  $\left\{ \left\{ \sqrt{-0.309...}, \sqrt{0.809...}, -\frac{1}{2}, 0, 0 \right\}, \left\{ \sqrt{-0.809...}, \sqrt{-0.309...}, 0, \frac{1}{2}, 0 \right\}, \right.$   
 $\left. \left\{ \frac{1}{2}, 0, \sqrt{-0.309...}, \sqrt{0.809...}, 0 \right\}, \left\{ 0, -\frac{1}{2}, \sqrt{-0.809...}, \sqrt{-0.309...}, 0 \right\}, \{0, 0, 0, 0, 1\} \right\}$

```
In[ ]:= rmattoqmat[pbargen1lift]
```

Out[ ]:=  $\left\{ \{1, 0\}, \left\{ 0, -\frac{i}{2} + \sqrt{0.809...} + j\sqrt{-0.309...} \right\} \right\}$

*pbargen1liftconj*

```
In[ ]:= rmattoqmat[pbargen1liftconj = Apply[Dot, davisspmatlift[{{91, 24, 117}}]].
toQkappa[RootReduce[insideoutmatlift.pbargen1lift.Inverse[insideoutmatlift]]]]
```

$$\text{Out[ ]} = \left\{ \left\{ \frac{j}{2} + i \left( \sqrt{-0.809\dots} + \sqrt{-0.309\dots} \right), 0 \right\}, \{0, 1\} \right\}$$

```
In[ ]:= rmattoqmat[pbargen2lift]
```

$$\text{Out[ ]} = \left\{ \{1, 0\}, \left\{ 0, -\frac{i}{2} + j \left( \sqrt{0.309\dots} + \sqrt{0.809\dots} \right) \right\} \right\}$$

*pbargen2liftconj*

```
In[ ]:= rmattoqmat[pbargen2liftconj = Apply[Dot, davisspmatlift[{{72, 36, 117}}]].
toQkappa[RootReduce[insideoutmatlift.pbargen2lift.Inverse[insideoutmatlift]]]]
```

$$\text{Out[ ]} = \left\{ \left\{ \frac{j}{2} + i \left( \sqrt{-0.809\dots} + \sqrt{-0.309\dots} \right), 0 \right\}, \{0, 1\} \right\}$$

*pbarquatsalphaauto*

```
In[ ]:= Dimensions[pbarquatsalphaauto = Map[matrixtoquaternion,
sgpairsgen[{{quaterniontomatrix[rmattoqmat[pbargen1lift][[2, 2]]],
quaterniontomatrix[rmattoqmat[pbargen1liftconj][[1, 1]]],
{quaterniontomatrix[rmattoqmat[pbargen2lift][[2, 2]]],
quaterniontomatrix[rmattoqmat[pbargen2liftconj][[1, 1]]]}}], {2}]]
```

```
Out[ ]:= {120, 2}
```

*pbarquatsalphaautoperm*

```
In[ ]:= pbarquatsalphaautoperm = Sort[pbarquatsalphaauto /. pquatsrules][[All, 2]];
```

*pquatsalphaautoinvperm*

```
In[ ]:= pquatsalphaautoinvperm = Ordering[pquatsalphaautoperm];
```

```
In[ ]:= pbarquatsalphaautoperm == pquatsalphaautoinvperm
```

```
Out[ ]:= True
```

$$\text{So } \hat{h}_0 \text{diag}(1, q) \hat{h}_0^{-1} = \text{diag}(\alpha^{-1}(q), 1) \text{ modulo } \hat{K}.$$

*pquatsinverseperm*

```
In[ ]:= pquatsinverseperm =
Map[matrixtoquaternion[Inverse[quaterniontomatrix[#]]] /. pquatsrules &, pquats];
```

```
In[ ]:= pquatsinverseperm[[pquatsinverseperm]] == Range[120]
```

```
Out[ ]:= True
```

*pquatsminusperm*

```
In[ ]:= pquatsminusperm = Map[-# &, pquats, {2}] /. pquatsrules;
```

```
In[ ]:= pquatsminusperm[[pquatsminusperm]] == Range[120]
```

```
Out[ ]:= True
```

*pquatsmultiplyperm*

```
In[ ]:= pquatsmultiplyperm = Outer[
matrixtoquaternion[quaterniontomatrix[#1].quaterniontomatrix[#2]] /. pquatsrules &,
pquats, pquats, 1];
```



davisopsymliftident

```
In[*]:= davisopsymliftident = davisopsymlift[
  quaternion[1, 0, 0, 0] /. pquatsrules, quaternion[1, 0, 0, 0] /. pquatsrules, 0]

Out[*]:= davisopsymlift[120, 120, 0]
```

davisopsymliftmat, davisopsymliftqmat

```
In[*]:= Clear[davisopsymliftqmat];
davisopsymliftqmat[davisopsymlift[i1_, i2_, j_]] :=
  (davisopsymliftqmat[davisopsymlift[i1, i2, j]] =
    rmattoqmat[If[j == 0, ToNumberField[qmattormat[{pquats[i1], quaternion[0, 0, 0, 0]},
      {quaternion[0, 0, 0, 0], pquats[i2]}]], iofieldth],
    ToNumberField[qmattormat[{pquats[i1], quaternion[0, 0, 0, 0]},
      {quaternion[0, 0, 0, 0], pquats[i2]}]], iofieldth].insideoutmatlift]]);
davisopsymliftmat[davisopsymlift[i1_, i2_, j_]] := qmattormat[
  davisopsymliftqmat[davisopsymlift[i1, i2, j]]];
```

davisopsymliftinverse

```
In[*]:= davisopsymliftinverse[davisopsymlift[i1_, i2_, j_]] :=
  If[j == 0, davisopsymlift[pquatsinverseperm[i1], pquatsinverseperm[i2], 0],
    davisopsymlift[pquatsalphaautoinvperm[pquatsinverseperm[pquatsminusperm[i2]]]],
    pquatsalphaautoperm[pquatsinverseperm[pquatsminusperm[i1]]]], 1];
```

davisopsymliftmultiply

```
In[*]:= davisopsymliftmultiply[davisopsymlift[i1_, i2_, j_], davisopsymlift[k1_, k2_, m_]] :=
  If[j == 0, davisopsymlift[pquatsmultiplyperm[i1, k1], pquatsmultiplyperm[i2, k2], m],
    If[m == 0, davisopsymlift[pquatsmultiplyperm[i1, pquatsalphaautoinvperm[k2]]],
      pquatsmultiplyperm[i2, pquatsalphaautoperm[k1]], 1], davisopsymlift[
      pquatsmultiplyperm[i1, pquatsalphaautoinvperm[pquatsminusperm[k2]]],
      pquatsmultiplyperm[i2, pquatsalphaautoperm[pquatsminusperm[k1]]], 0]]];
```

davisopsymliftgrp

```
In[*]:= Dimensions[davisopsymliftgrp =
  Flatten[Table[davisopsymlift[i1, i2, j], {i1, 1, 120}, {i2, 1, 120}, {j, 0, 1}]]]

Out[*]:= {28800}
```

davisopsymliftcyclicsg

```
In[*]:= davisopsymliftcyclicsg[x_davisopsymlift] :=
  NestWhileList[davisopsymliftmultiply[x, #] &, x, # != davisopsymliftident &];
```

davisopsymliftorder

```
In[*]:= davisopsymliftorder[x_davisopsymlift] := Length[davisopsymliftcyclicsg[x]];

In[*]:= Sort[Tally[Map[davisopsymliftorder, davisopsymliftgrp]]]

Out[*]:= {{1, 1}, {2, 123}, {3, 440}, {4, 1140}, {5, 624}, {6, 3720},
  {8, 3600}, {10, 4752}, {12, 4800}, {15, 960}, {20, 5760}, {30, 2880}}
```

*davisopsymliftconjclassesstart*

```
In[ ]:= AbsoluteTiming[
  Map[Length, davisopsymliftconjclassesstart = SortBy[FixedPoint[Function[xp, If[
    xp[[2]] == {}, xp, Function[cx, {Append[xp[[1]], cx], Complement[xp[[2]], cx}]] [
    Union[Map[davisopsymliftmultiply[davisopsymliftmultiply[#, xp[[2, 1]]],
      davisopsymliftinverse[#]] &, davisopsymliftgrp]]]],
    {{}, davisopsymliftgrp]] [[1]], {davisopsymliftorder[#[[1]]], Length[#]} &]]]
Out[ ]:= {21.3926, {1, 1, 2, 120, 40, 400, 60, 60, 120, 900, 24, 24, 144, 144, 288, 40, 40, 40, 400, 800,
  2400, 3600, 24, 24, 24, 24, 24, 24, 144, 144, 288, 288, 288, 288, 1440, 1440, 1200,
  1200, 2400, 480, 480, 720, 720, 720, 720, 1440, 1440, 480, 480, 480, 480, 480, 480}}
```

```
In[ ]:= Total[%[[2]]]
```

```
Out[ ]:= 28800
```

```
In[ ]:= Sort[Tally[%[[2]]]]
```

```
Out[ ]:= {{1, 2}, {2, 1}, {24, 8}, {40, 4}, {60, 2}, {120, 2}, {144, 4}, {288, 6}, {400, 2},
  {480, 8}, {720, 4}, {800, 1}, {900, 1}, {1200, 2}, {1440, 4}, {2400, 2}, {3600, 1}}
```

```
In[ ]:= Length[davisopsymliftconjclassesstart]
```

```
Out[ ]:= 54
```

```
In[ ]:= Map[Union, Map[davisopsymliftorder, davisopsymliftconjclassesstart, {2}]]
```

```
Out[ ]:= {{1}, {2}, {2}, {2}, {3}, {3}, {4}, {4}, {4}, {4}, {5}, {5}, {5}, {5},
  {5}, {6}, {6}, {6}, {6}, {6}, {6}, {6}, {8}, {10}, {10}, {10}, {10}, {10}, {10},
  {10}, {10}, {10}, {10}, {10}, {10}, {10}, {10}, {10}, {10}, {12}, {12}, {12}, {15},
  {15}, {20}, {20}, {20}, {20}, {20}, {20}, {20}, {30}, {30}, {30}, {30}, {30}, {30}}
```

```
In[ ]:= Sort[Tally[%]]
```

```
Out[ ]:= {{{1}, 1}, {{2}, 3}, {{3}, 2}, {{4}, 4}, {{5}, 5}, {{6}, 6},
  {{8}, 1}, {{10}, 15}, {{12}, 3}, {{15}, 2}, {{20}, 6}, {{30}, 6}}
```

*davisopsymliftminus*

```
In[ ]:= davisopsymliftminus[davisopsymlift[i1_, i2_, j_]] :=
  davisopsymlift[pquatsminusperm[[i1]], pquatsminusperm[[i2]], j];
```

*davisopsymnorm*

```
In[ ]:= davisopsymnorm[x_] := SortBy[x, davisopsymliftorder];
```

*davisopsymliftprojection*

```
In[ ]:= davisopsymliftprojection[x_] := davisopsymnorm[{x, davisopsymliftminus[x]}];
```

*davisopsymmat1*

```
In[ ]:= davisopsymmat1[x_] := toQkappa[RootReduce[spinprojection[davisopsymliftmat[x[[1]]]]]]
```

```
In[ ]:= TrueQ[
```

```
  Apply[And, Table[pgrp[[i]] == davisopsymmat[davisopsymnorm[{davisopsymlift[i, 120, 0],
    davisopsymlift[pquatsminusperm[[i]], 1, 0]}]], {i, 1, 120}]]]
```

```
Out[ ]:= False
```

pquatsbetamapperm

```
In[ ]:= pquatsbetamapperm =
  Sort[sgpairs[{{quaternionmatrix[rmattoqmat[pbargen1lift][[2, 2]]], pbargen1},
    {quaternionmatrix[rmattoqmat[pbargen2lift][[2, 2]]], pbargen2}}] /.
  Thread[pquatmats → Range[120]] /. Thread[pbargrp → Range[120]]][[All, 2]];
```

```
In[ ]:= TrueQ[Apply[And, Table[pbargrp[[pquatsbetamapperm[[i]]]] ==
  davisopsymmat[davisopsymnorm[{davisopsymlift[120, i, 0],
  davisopsymlift[1, pquatsminusperm[[i]], 0]}]], {i, 1, 120}]]]
```

```
Out[ ]:= False
```

```
In[ ]:= insideoutmat ==
  davisopsymmat[davisopsymnorm[{davisopsymlift[120, 120, 1], davisopsymlift[1, 1, 120]}]]
```

```
Out[ ]:= {{-15.3..., -5.85..., 0, -2.62..., 16.6...},
  {-5.85..., -2.62..., 0, 0, 6.33...}, {0, 0, 1, 0, 0},
  {-2.62..., 0, 0, 0, 2.42...}, {-16.6..., -6.33..., 0, -2.42..., 17.9...}} ==
  davisopsymmat[{davisopsymlift[1, 1, 120], davisopsymlift[120, 120, 1]}
```

davisopsymmat

```
In[ ]:= Clear[davisopsymmat];
  davisopsymmat[x_] := (davisopsymmat[x] =
    If[x[[1, 3]] == 0, pgrp[x[[1, 1]]].pbargrp[pquatsbetamapperm[x[[1, 2]]]],
    pgrp[x[[1, 1]]].pbargrp[pquatsbetamapperm[x[[1, 2]]]].insideoutmat);
```

davisopsymident, davisopsyminverse, davisopsymmultiply

```
In[ ]:= davisopsymident = davisopsymliftprojection[davisopsymliftident];
  davisopsyminverse[x_] := davisopsymliftprojection[davisopsymliftinverse[x[[1]]]];
  davisopsymmultiply[x_, y_] :=
    davisopsymliftprojection[davisopsymliftmultiply[x[[1]], y[[1]]];
```

davisopsymcyclicsg

```
In[ ]:= davisopsymcyclicsg[x_] :=
  NestWhileList[davisopsymmultiply[x, #] &, x, # != davisopsymident &];
```

davisopsymorder

```
In[ ]:= davisopsymorder[x_] :=
  Length[Union[Map[davisopsymliftprojection, davisopsymliftcyclicsg[x[[1]]]]];
```

davisopsymgrp

```
In[ ]:= Dimensions[davisopsymgrp = Union[Map[davisopsymliftprojection, davisopsymliftgrp]]]
```

```
Out[ ]:= {14400, 2}
```

```
In[ ]:= Sort[Tally[Map[davisopsymliftorder, davisopsymgrp, {2}]]]
```

```
Out[ ]:= {{1, 2}, 1}, {{2, 2}, 61}, {{3, 6}, 440}, {{4, 4}, 570},
  {{5, 10}, 624}, {{6, 6}, 1640}, {{8, 8}, 1800}, {{10, 10}, 2064},
  {{12, 12}, 2400}, {{15, 30}, 960}, {{20, 20}, 2880}, {{30, 30}, 960}}
```

*davisopsymconjclassesstart*

```
In[ ]:= AbsoluteTiming[Map[Length, davisopsymconjclassesstart = SortBy[
  Union[Map[Union, Map[davisopsymliftprojection, davisopsymliftconjclassesstart, {2}]]],
  {davisopsymorder[#[[1]]], Length[#]} &]]]
```

```
Out[ ]:= {3.86923, {1, 1, 60, 60, 450, 40, 400, 60, 1800, 24, 24, 144, 144, 288, 40, 400, 1200,
  1200, 24, 24, 144, 144, 288, 720, 720, 720, 720, 1200, 480, 480, 720, 720, 480, 480}}
```

*davisopsymconjclasses*

```
In[ ]:= AbsoluteTiming[Map[Length,
  davisopsymconjclasses = Function[cc, Join[SortBy[Select[cc, Length[#] == 2 &][[All, 1]],
    {davisopsymorder[#[[1]]], Length[#]} &],
    Select[cc, Length[#] == 1 &][[All, 1]]][Gather[
    Map[Union, Map[davisopsymliftprojection, davisopsymliftconjclassesstart, {2}]]]]]]]
```

```
Out[ ]:= {4.04263, {1, 40, 400, 60, 24, 24, 144, 144, 288, 40, 24, 24, 288, 1200, 480, 480, 720,
  720, 480, 480, 1, 60, 60, 450, 400, 1200, 1800, 144, 144, 720, 720, 1200, 720, 720}}
```

```
In[ ]:= Total[%[[2]]]
```

```
Out[ ]:= 14400
```

```
In[ ]:= Sort[Tally[%[[2]]]]
```

```
Out[ ]:= {{1, 2}, {24, 4}, {40, 2}, {60, 3}, {144, 4}, {288, 2},
  {400, 2}, {450, 1}, {480, 4}, {720, 6}, {1200, 3}, {1800, 1}}
```

```
In[ ]:= Length[davisopsymconjclasses]
```

```
Out[ ]:= 34
```

```
In[ ]:= Map[Union, Map[davisopsymorder, davisopsymconjclasses, {2}]]
```

```
Out[ ]:= {{1}, {3}, {3}, {4}, {5}, {5}, {5}, {5}, {5}, {6}, {10},
  {10}, {10}, {12}, {15}, {15}, {20}, {20}, {30}, {30}, {2}, {2},
  {2}, {2}, {6}, {6}, {4}, {10}, {10}, {10}, {10}, {6}, {10}, {10}}
```

```
In[ ]:= Sort[Tally[%]]
```

```
Out[ ]:= {{{1}, 1}, {{2}, 4}, {{3}, 2}, {{4}, 2}, {{5}, 5},
  {{6}, 4}, {{10}, 9}, {{12}, 1}, {{15}, 2}, {{20}, 2}, {{30}, 2}}
```

*davisopsymliftconjclasses*

```
In[ ]:= Map[Length, davisopsymliftconjclasses = Function[cc,
  Join[Apply[Join, Select[cc, Length[#] == 2 &], Select[cc, Length[#] == 1 &][[All, 1]]][
    Map[Function[c, Select[davisopsymliftconjclassesstart, Complement[#, c] == {} &]],
    Map[Apply[Union, #] &, davisopsymconjclasses]]]]]
```

```
Out[ ]:= {1, 1, 40, 40, 400, 400, 60, 60, 24, 24, 24, 24, 144, 144, 144, 144, 288, 288, 40, 40, 24,
  24, 24, 24, 288, 288, 1200, 1200, 480, 480, 480, 480, 720, 720, 720, 720, 480, 480,
  480, 480, 2, 120, 120, 900, 800, 2400, 3600, 288, 288, 1440, 1440, 2400, 1440, 1440}
```

```
In[ ]:= Sort[Tally[Map[Length, davisopsymliftconjclasses]]]
```

```
Out[ ]:= {{1, 2}, {2, 1}, {24, 8}, {40, 4}, {60, 2}, {120, 2}, {144, 4}, {288, 6}, {400, 2},
  {480, 8}, {720, 4}, {800, 1}, {900, 1}, {1200, 2}, {1440, 4}, {2400, 2}, {3600, 1}}
```

```

In[ ]:= Sort[Tally[Map[Length, davisopsymliftconjclassesstart]]]
Out[ ]:= {{1, 2}, {2, 1}, {24, 8}, {40, 4}, {60, 2}, {120, 2}, {144, 4}, {288, 6}, {400, 2},
{480, 8}, {720, 4}, {800, 1}, {900, 1}, {1200, 2}, {1440, 4}, {2400, 2}, {3600, 1}}

In[ ]:= Map[davisopsymliftorder, davisopsymliftconjclasses[[All, 1]]]
Out[ ]:= {1, 2, 3, 6, 3, 6, 4, 4, 5, 10, 5, 10, 5, 10, 5, 10, 5, 10, 6, 6, 10, 10, 10, 10, 10, 10, 12, 12, 15,
30, 15, 30, 20, 20, 20, 20, 30, 30, 30, 30, 2, 2, 4, 4, 6, 6, 8, 10, 10, 10, 10, 12, 20, 20}

In[ ]:= Sort[Tally[Map[davisopsymliftorder, davisopsymliftconjclasses[[All, 1]]]]]
Out[ ]:= {{1, 1}, {2, 3}, {3, 2}, {4, 4}, {5, 5}, {6, 6},
{8, 1}, {10, 15}, {12, 3}, {15, 2}, {20, 6}, {30, 6}}

```

## Representations

pquatmatsconjclassnames

```
In[ ]:= pquatmatsconjclassnames = {"1", "2", "3", "4", "5A", "5B", "6", "10A", "10B"}
```

```
Out[ ]:= {1, 2, 3, 4, 5A, 5B, 6, 10A, 10B}
```

```

In[ ]:= TableForm[Map[{elementorder[#[[1]]], Length[#],
Map[formatkappa, #[[1]] /. Thread[pquatmats → pquats]]} &, pquatmatsconjclasses],
TableHeadings → {pquatmatsconjclassnames, {"order", "size", "rep"}}, TableDepth → 2]

```

Out[ ]//TableForm=

|     | order | size | rep                                                                             |
|-----|-------|------|---------------------------------------------------------------------------------|
| 1   | 1     | 1    | 1                                                                               |
| 2   | 2     | 1    | -1                                                                              |
| 3   | 3     | 20   | $-\frac{1}{2} + \frac{i}{2} - \frac{j}{2} + \frac{k}{2}$                        |
| 4   | 4     | 30   | i                                                                               |
| 5A  | 5     | 12   | $-\frac{1}{2} + \frac{i}{2} + \frac{\tau}{2} - \frac{k\tau}{2}$                 |
| 5B  | 5     | 12   | $\frac{i}{2} + j \left( -\frac{1}{2} + \frac{\tau}{2} \right) - \frac{\tau}{2}$ |
| 6   | 6     | 20   | $\frac{1}{2} + \frac{i}{2} - \frac{j}{2} + \frac{k}{2}$                         |
| 10A | 10    | 12   | $\frac{i}{2} + j \left( -\frac{1}{2} + \frac{\tau}{2} \right) + \frac{\tau}{2}$ |
| 10B | 10    | 12   | $\frac{1}{2} + \frac{i}{2} - \frac{\tau}{2} - \frac{k\tau}{2}$                  |

rho1rep

```
In[ ]:= rho1rep = Map[Apply[Rule, #] &, sgpairsgen[toQkappa[{{pquatmats[[14]], {{1}}},
{pquatmats[[48]], {{1}}}, {pquatmats[[58]], {{1}}}], 10]];
```

rho2fieldtheta

```
In[ ]:= rho2fieldtheta = ToNumberField[{kappa, I}][[1, 1]]
```

```
Out[ ]:=  $2.42... + 1.00... i$ 
```

rho2rep

```
In[ ]:= rho2rep = Map[Apply[Rule, #] &, sgpairsgen[
  {{pquatmats[[14]], -ToNumberField[(1 + I) / 2 * {{1, I}, {1, -I}}, rho2fieldtheta]},
  {pquatmats[[48]], ToNumberField[{{0, -I}, {-I, 0}}, rho2fieldtheta]},
  {pquatmats[[58]], -ToNumberField[
    1 / 2 {{-I * (1 - tau), tau + I}, {-tau + I, I * (1 - tau)}}, rho2fieldtheta]}], 10]];
```

rho2primereporig

```
In[ ]:= rho2primereporig = Map[Apply[Rule, #] &, sgpairsgen[
  {{pquatmats[[14]], -ToNumberField[(1 + I) / 2 * {{1, I}, {1, -I}}, rho2fieldtheta]},
  {pquatmats[[48]], ToNumberField[{{0, -I}, {-I, 0}}, rho2fieldtheta]},
  {pquatmats[[58]], -ToNumberField[
    1 / 2 {{-I * tau, 1 + I - tau}, {-1 + I + tau, I * tau}}, rho2fieldtheta]}], 10]];
```

rho2primerep

```
In[ ]:= rho2primerep = Map[Apply[Rule, #] &, sgpairsgen[{{pquatmats[[pquatsalphaautoperm[[14]]]],
  -ToNumberField[(1 + I) / 2 * {{1, I}, {1, -I}}, rho2fieldtheta]},
  {pquatmats[[pquatsalphaautoperm[[48]]]], ToNumberField[{{0, -I}, {-I, 0}},
  rho2fieldtheta]}, {pquatmats[[pquatsalphaautoperm[[58]]]], -ToNumberField[
    1 / 2 {{-I * (1 - tau), tau + I}, {-tau + I, I * (1 - tau)}}, rho2fieldtheta]}], 10]];
```

rho2primeinvrep

```
In[ ]:= rho2primeinvrep =
  Map[Apply[Rule, #] &, sgpairsgen[{{pquatmats[[pquatsalphaautoinvperm[[14]]]],
  -ToNumberField[(1 + I) / 2 * {{1, I}, {1, -I}}, rho2fieldtheta]},
  {pquatmats[[pquatsalphaautoinvperm[[48]]]], ToNumberField[{{0, -I}, {-I, 0}},
  rho2fieldtheta]}, {pquatmats[[pquatsalphaautoinvperm[[58]]]], -ToNumberField[
    1 / 2 {{-I * (1 - tau), tau + I}, {-tau + I, I * (1 - tau)}}, rho2fieldtheta]}], 10]];
```

rho3rep

```
In[ ]:= rho3rep = Map[Apply[Rule, #] &,
  sgpairsgen[toQkappa[{{pquatmats[[14]], {{0, 0, 1}, {1, 0, 0}, {0, 1, 0}}},
  {pquatmats[[48]], {{1, 0, 0}, {0, -1, 0}, {0, 0, -1}}}, {pquatmats[[58]],
  -1 / 2 {{1, tau, 1 - tau}, {tau, 1 - tau, 1}, {1 - tau, 1, tau}}}], 10]];
```

rho3primereporig

```
In[ ]:= rho3primereporig = Map[Apply[Rule, #] &, sgpairsgen[
  toQkappa[{{pquatmats[[pquatsalphaautoperm[[14]]]], {{0, 0, 1}, {1, 0, 0}, {0, 1, 0}}},
  {pquatmats[[pquatsalphaautoperm[[48]]]], {{1, 0, 0}, {0, -1, 0}, {0, 0, -1}}},
  {pquatmats[[pquatsalphaautoperm[[58]]]],
  -1 / 2 {{1, tau, 1 - tau}, {tau, 1 - tau, 1}, {1 - tau, 1, tau}}}], 10]];
```

rho3primerep

```
In[ ]:= rho3primerep = Map[Apply[Rule, #] &, sgpairsgen[
  toQkappa[{{pquatmats[[pquatsalphaautoperm[[14]]]], {{0, 0, 1}, {1, 0, 0}, {0, 1, 0}}},
  {pquatmats[[pquatsalphaautoperm[[48]]]], {{1, 0, 0}, {0, -1, 0}, {0, 0, -1}}},
  {pquatmats[[pquatsalphaautoperm[[58]]]],
  -1 / 2 {{1, tau, 1 - tau}, {tau, 1 - tau, 1}, {1 - tau, 1, tau}}}], 10]];
```

rho3primeinvrep

```
In[ ]:= rho3primeinvrep =
  Map[Apply[Rule, #] &, sgpairsgen[toQkappa[{{pquatmats[[pquatsalphaautoinvperm[[14]]]],
  {{0, 0, 1}, {1, 0, 0}, {0, 1, 0}}}, {pquatmats[[pquatsalphaautoinvperm[[48]]]],
  {{1, 0, 0}, {0, -1, 0}, {0, 0, -1}}}, {pquatmats[[pquatsalphaautoinvperm[[58]]]],
  -1 / 2 {{1, tau, 1 - tau}, {tau, 1 - tau, 1}, {1 - tau, 1, tau}}}], 10]];
```

rho4rep

```
In[ ]:= rho4rep = Map[Apply[Rule, #] &, sgpairsgen[
  toQkappa[{{pquatmats[[14]], {{1, 0, 0, 0}, {0, 0, 0, 1}, {0, 1, 0, 0}, {0, 0, 1, 0}}},
    {pquatmats[[48]], {{1, 0, 0, 0}, {0, 1, 0, 0}, {0, 0, -1, 0}, {0, 0, 0, -1}}},
    {pquatmats[[58]], toQkappa[-1/4 {{1, Sqrt[5], Sqrt[5], Sqrt[5]},
      {Sqrt[5], -3, 1, 1}, {Sqrt[5], 1, 1, -3}, {Sqrt[5], 1, -3, 1}}]}], 10]];
```

rho4alpharep

```
In[ ]:= rho4alpharep =
  Map[Apply[Rule, #] &, sgpairsgen[toQkappa[{{pquatmats[[pquatsalphaautoperm[[14]]]],
    {{1, 0, 0, 0}, {0, 0, 0, 1}, {0, 1, 0, 0}, {0, 0, 1, 0}}},
    {pquatmats[[pquatsalphaautoperm[[48]]]], {{1, 0, 0, 0}, {0, 1, 0, 0},
      {0, 0, -1, 0}, {0, 0, 0, -1}}}, {pquatmats[[pquatsalphaautoperm[[58]]]],
    toQkappa[-1/4 {{1, Sqrt[5], Sqrt[5], Sqrt[5]}, {Sqrt[5], -3, 1, 1},
      {Sqrt[5], 1, 1, -3}, {Sqrt[5], 1, -3, 1}}]}], 10]];
```

rho4alphainvrep

```
In[ ]:= rho4alphainvrep =
  Map[Apply[Rule, #] &, sgpairsgen[toQkappa[{{pquatmats[[pquatsalphaautoinvperm[[14]]]],
    {{1, 0, 0, 0}, {0, 0, 0, 1}, {0, 1, 0, 0}, {0, 0, 1, 0}}},
    {pquatmats[[pquatsalphaautoinvperm[[48]]]], {{1, 0, 0, 0}, {0, 1, 0, 0},
      {0, 0, -1, 0}, {0, 0, 0, -1}}}, {pquatmats[[pquatsalphaautoinvperm[[58]]]],
    toQkappa[-1/4 {{1, Sqrt[5], Sqrt[5], Sqrt[5]}, {Sqrt[5], -3, 1, 1},
      {Sqrt[5], 1, 1, -3}, {Sqrt[5], 1, -3, 1}}]}], 10]];
```

rho4primefieldth

```
In[ ]:= rho4primefieldth = ToNumberField[{kappa, Exp[2 Pi * I / 3], I}][[1, 1]]
```

```
Out[ ]:= 2.92... + 1.87... i
```

rho4primerep

```
In[ ]:= rho4primerep =
  Map[Apply[Rule, #] &, sgpairsgen[{{pquatmats[[14]], -ToNumberField[(1 + I) / 2 *
    {Exp[2 Pi * I / 3], Exp[2 Pi * I / 3] * I, 0, 0}, {Exp[2 Pi * I / 3],
      -Exp[2 Pi * I / 3] * I, 0, 0}, {0, 0, Exp[2 Pi * I / 3]^2, Exp[2 Pi * I / 3]^2 * I},
      {0, 0, Exp[2 Pi * I / 3]^2, -Exp[2 Pi * I / 3]^2 * I}}, rho4primefieldth}},
    {pquatmats[[48]], ToNumberField[{{0, -I, 0, 0}, {-I, 0, 0, 0}, {0, 0, 0, -I},
      {0, 0, -I, 0}}, rho4primefieldth}}, {pquatmats[[58]],
    -ToNumberField[RootReduce[1/4 {{Exp[2 Pi * I / 3]^2 - Exp[2 Pi * I / 3] - I,
      1 - I, -I * Exp[2 Pi * I / 3] * (tau + Exp[2 Pi * I / 3]),
      (I * Exp[2 Pi * I / 3]^2 - I - 1) (Exp[2 Pi * I / 3]^2 * tau + 1)},
      {-I - 1, Exp[2 Pi * I / 3]^2 - Exp[2 Pi * I / 3] + I, (I * Exp[2 Pi * I / 3]^2 - I + 1)
        (Exp[2 Pi * I / 3]^2 * tau + 1), I * Exp[2 Pi * I / 3] * (tau + Exp[2 Pi * I / 3])},
      {-I * Exp[2 Pi * I / 3] * (Exp[2 Pi * I / 3] * tau + 1), (I * Exp[2 Pi * I / 3] - I - 1)
        (Exp[2 Pi * I / 3] * tau + 1), -Exp[2 Pi * I / 3]^2 + Exp[2 Pi * I / 3] - I, 1 - I},
      {(I * Exp[2 Pi * I / 3] - I + 1) (Exp[2 Pi * I / 3] * tau + 1),
      I * Exp[2 Pi * I / 3] * (Exp[2 Pi * I / 3] * tau + 1), -I - 1,
      -Exp[2 Pi * I / 3]^2 + Exp[2 Pi * I / 3] + I}}], rho4primefieldth}}], 10]];
```

rho4primealpharep

```

In[ ]:= rho4primealpharep =
  Map[Apply[Rule, #] &, sgpairsgen[{{pquatmats[[pquatsalphaautoperm[[14]]]],
    -ToNumberField[(1 + I) / 2 * {{Exp[2 Pi * I / 3], Exp[2 Pi * I / 3] * I, 0, 0},
      {Exp[2 Pi * I / 3], -Exp[2 Pi * I / 3] * I, 0, 0}, {0, 0, Exp[2 Pi * I / 3]^2,
        Exp[2 Pi * I / 3]^2 * I}, {0, 0, Exp[2 Pi * I / 3]^2, -Exp[2 Pi * I / 3]^2 * I}},
      rho4primefieldth}}, {pquatmats[[pquatsalphaautoperm[[48]]]],
    ToNumberField[{{0, -I, 0, 0}, {-I, 0, 0, 0}, {0, 0, 0, -I}, {0, 0, -I, 0}},
      rho4primefieldth}}, {pquatmats[[pquatsalphaautoperm[[58]]]],
    -ToNumberField[RootReduce[1 / 4 {{Exp[2 Pi * I / 3]^2 - Exp[2 Pi * I / 3] - I, 1 - I,
      -I * Exp[2 Pi * I / 3] * (tau + Exp[2 Pi * I / 3]), (I * Exp[2 Pi * I / 3]^2 - I - 1)
        (Exp[2 Pi * I / 3]^2 * tau + 1)}, {-I - 1, Exp[2 Pi * I / 3]^2 - Exp[2 Pi * I / 3] + I,
        (I * Exp[2 Pi * I / 3]^2 - I + 1) (Exp[2 Pi * I / 3]^2 * tau + 1), I * Exp[2 Pi * I / 3] *
        (tau + Exp[2 Pi * I / 3])}, {-I * Exp[2 Pi * I / 3] * (Exp[2 Pi * I / 3] * tau + 1),
        (I * Exp[2 Pi * I / 3] - I - 1) (Exp[2 Pi * I / 3] * tau + 1),
        -Exp[2 Pi * I / 3]^2 + Exp[2 Pi * I / 3] - I, 1 - I}, {(I * Exp[2 Pi * I / 3] - I + 1)
        (Exp[2 Pi * I / 3] * tau + 1), I * Exp[2 Pi * I / 3] * (Exp[2 Pi * I / 3] * tau + 1),
        -I - 1, -Exp[2 Pi * I / 3]^2 + Exp[2 Pi * I / 3] + I}}], rho4primefieldth}}], 10]];

```

rho4primealphainvrep

```

In[ ]:= rho4primealphainvrep =
  Map[Apply[Rule, #] &, sgpairsgen[{{pquatmats[[pquatsalphaautoinvperm[[14]]]],
    -ToNumberField[(1 + I) / 2 * {{Exp[2 Pi * I / 3], Exp[2 Pi * I / 3] * I, 0, 0},
      {Exp[2 Pi * I / 3], -Exp[2 Pi * I / 3] * I, 0, 0}, {0, 0, Exp[2 Pi * I / 3]^2,
        Exp[2 Pi * I / 3]^2 * I}, {0, 0, Exp[2 Pi * I / 3]^2, -Exp[2 Pi * I / 3]^2 * I}},
      rho4primefieldth}}, {pquatmats[[pquatsalphaautoinvperm[[48]]]],
    ToNumberField[{{0, -I, 0, 0}, {-I, 0, 0, 0}, {0, 0, 0, -I}, {0, 0, -I, 0}},
      rho4primefieldth}}, {pquatmats[[pquatsalphaautoinvperm[[58]]]],
    -ToNumberField[RootReduce[1 / 4 {{Exp[2 Pi * I / 3]^2 - Exp[2 Pi * I / 3] - I, 1 - I,
      -I * Exp[2 Pi * I / 3] * (tau + Exp[2 Pi * I / 3]), (I * Exp[2 Pi * I / 3]^2 - I - 1)
        (Exp[2 Pi * I / 3]^2 * tau + 1)}, {-I - 1, Exp[2 Pi * I / 3]^2 - Exp[2 Pi * I / 3] + I,
        (I * Exp[2 Pi * I / 3]^2 - I + 1) (Exp[2 Pi * I / 3]^2 * tau + 1), I * Exp[2 Pi * I / 3] *
        (tau + Exp[2 Pi * I / 3])}, {-I * Exp[2 Pi * I / 3] * (Exp[2 Pi * I / 3] * tau + 1),
        (I * Exp[2 Pi * I / 3] - I - 1) (Exp[2 Pi * I / 3] * tau + 1),
        -Exp[2 Pi * I / 3]^2 + Exp[2 Pi * I / 3] - I, 1 - I}, {(I * Exp[2 Pi * I / 3] - I + 1)
        (Exp[2 Pi * I / 3] * tau + 1), I * Exp[2 Pi * I / 3] * (Exp[2 Pi * I / 3] * tau + 1),
        -I - 1, -Exp[2 Pi * I / 3]^2 + Exp[2 Pi * I / 3] + I}}], rho4primefieldth}}], 10]];

```

rho5fieldtheta

```

In[ ]:= rho5fieldtheta = ToNumberField[{kappa, Exp[2 Pi * I / 3]]}[[1, 1]]

```

```

Out[ ]:= 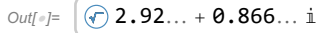 2.92... + 0.866... i

```

rho5rep

```

In[ ]:= rho5rep = Map[Apply[Rule, #] &, sgpairsgen[
  {{pquatmats[[14]], ToNumberField[{{0, 0, 1, 0, 0}, {1, 0, 0, 0, 0}, {0, 1, 0, 0, 0},
    {0, 0, 0, Exp[2 Pi * I / 3], 0}, {0, 0, 0, 0, Exp[2 Pi * I / 3]^2}}, rho5fieldtheta}},
  {pquatmats[[48]], {{1, 0, 0, 0, 0}, {0, -1, 0, 0, 0}, {0, 0, -1, 0, 0}, {0, 0, 0, 1, 0},
    {0, 0, 0, 0, 1}}}, {pquatmats[[58]], ToNumberField[1 / 2 {{0, 1, 1, -1, -1},
    {1, 1, 0, -Exp[2 Pi * I / 3], -Exp[2 Pi * I / 3]^2}, {1, 0, 1, -Exp[2 Pi * I / 3]^2,
      -Exp[2 Pi * I / 3]}, {-1, -Exp[2 Pi * I / 3]^2, -Exp[2 Pi * I / 3], 0, 1},
    {-1, -Exp[2 Pi * I / 3], -Exp[2 Pi * I / 3]^2, 1, 0}}, rho5fieldtheta}}], 10]];

```



rho5alpharep

```

In[ ]:= rho5alpharep = Map[Apply[Rule, #] &,
  sgpairsgen[{{pquatmats[pquatsalphaautoperm[14]]}, ToNumberField[
    {{0, 0, 1, 0, 0}, {1, 0, 0, 0, 0}, {0, 1, 0, 0, 0}, {0, 0, 0, Exp[2 Pi * I / 3], 0},
    {0, 0, 0, 0, Exp[2 Pi * I / 3]^2}}, rho5fieldtheta]],
  {pquatmats[pquatsalphaautoperm[48]]}, {{1, 0, 0, 0, 0}, {0, -1, 0, 0, 0},
    {0, 0, -1, 0, 0}, {0, 0, 0, 1, 0}, {0, 0, 0, 0, 1}}},
  {pquatmats[pquatsalphaautoperm[58]]}, ToNumberField[1 / 2 {{0, 1, 1, -1, -1},
    {1, 1, 0, -Exp[2 Pi * I / 3], -Exp[2 Pi * I / 3]^2}, {1, 0, 1, -Exp[2 Pi * I / 3]^2,
    -Exp[2 Pi * I / 3]}, {-1, -Exp[2 Pi * I / 3]^2, -Exp[2 Pi * I / 3], 0, 1},
    {-1, -Exp[2 Pi * I / 3], -Exp[2 Pi * I / 3]^2, 1, 0}}, rho5fieldtheta]]], 10]];

```

rho5alphainvrep

```

In[ ]:= rho5alphainvrep =
  Map[Apply[Rule, #] &, sgpairsgen[{{pquatmats[pquatsalphaautoinvperm[14]]},
    ToNumberField[{{0, 0, 1, 0, 0}, {1, 0, 0, 0, 0}, {0, 1, 0, 0, 0},
    {0, 0, 0, Exp[2 Pi * I / 3], 0}, {0, 0, 0, 0, Exp[2 Pi * I / 3]^2}}, rho5fieldtheta]],
  {pquatmats[pquatsalphaautoinvperm[48]]}, {{1, 0, 0, 0, 0},
    {0, -1, 0, 0, 0}, {0, 0, -1, 0, 0}, {0, 0, 0, 1, 0}, {0, 0, 0, 0, 1}}},
  {pquatmats[pquatsalphaautoinvperm[58]]}, ToNumberField[1 / 2 {{0, 1, 1, -1, -1},
    {1, 1, 0, -Exp[2 Pi * I / 3], -Exp[2 Pi * I / 3]^2}, {1, 0, 1, -Exp[2 Pi * I / 3]^2,
    -Exp[2 Pi * I / 3]}, {-1, -Exp[2 Pi * I / 3]^2, -Exp[2 Pi * I / 3], 0, 1},
    {-1, -Exp[2 Pi * I / 3], -Exp[2 Pi * I / 3]^2, 1, 0}}, rho5fieldtheta]]], 10]];

```

rho6rep

```

In[ ]:= rho6rep =
  Map[Apply[Rule, #] &, sgpairsgen[{{pquatmats[14]}, -ToNumberField[KroneckerProduct[
    {{0, 0, 1}, {1, 0, 0}, {0, 1, 0}}, (1 + I) / 2 * {{1, I}, {1, -I}}], rho2fieldtheta]],
  {pquatmats[48]}, ToNumberField[KroneckerProduct[{{1, 0, 0}, {0, -1, 0}, {0, 0, -1}},
    {{0, -I}, {-I, 0}}], rho2fieldtheta]], {pquatmats[58]}, -ToNumberField[
    KroneckerProduct[-1 / 2 * {{1, tau, 1 - tau}, {tau, 1 - tau, 1}, {1 - tau, 1, tau}},
    1 / 2 * {{-I * tau, 1 + I - tau}, {-1 + I + tau, I * tau}}], rho2fieldtheta]]], 10]];

```

rho6alpharep

```

In[ ]:= rho6alpharep = Map[Apply[Rule, #] &,
  sgpairsgen[{{pquatmats[pquatsalphaautoperm[14]]}, -ToNumberField[KroneckerProduct[
    {{0, 0, 1}, {1, 0, 0}, {0, 1, 0}}, (1 + I) / 2 * {{1, I}, {1, -I}}], rho2fieldtheta]],
  {pquatmats[pquatsalphaautoperm[48]]}, ToNumberField[KroneckerProduct[
    {{1, 0, 0}, {0, -1, 0}, {0, 0, -1}}, {{0, -I}, {-I, 0}}], rho2fieldtheta]],
  {pquatmats[pquatsalphaautoperm[58]]}, -ToNumberField[
    KroneckerProduct[-1 / 2 * {{1, tau, 1 - tau}, {tau, 1 - tau, 1}, {1 - tau, 1, tau}},
    1 / 2 * {{-I * tau, 1 + I - tau}, {-1 + I + tau, I * tau}}], rho2fieldtheta]]], 10]];

```

rho6alphainvrep

```

In[ ]:= rho6alphainvrep = Map[Apply[Rule, #] &, sgpairsgen[
  {{pquatmats[pquatsalphaautoinvperm[14]]}, -ToNumberField[KroneckerProduct[
    {{0, 0, 1}, {1, 0, 0}, {0, 1, 0}}, (1 + I) / 2 * {{1, I}, {1, -I}}], rho2fieldtheta]],
  {pquatmats[pquatsalphaautoinvperm[48]]}, ToNumberField[KroneckerProduct[
    {{1, 0, 0}, {0, -1, 0}, {0, 0, -1}}, {{0, -I}, {-I, 0}}], rho2fieldtheta]],
  {pquatmats[pquatsalphaautoinvperm[58]]}, -ToNumberField[
    KroneckerProduct[-1 / 2 * {{1, tau, 1 - tau}, {tau, 1 - tau, 1}, {1 - tau, 1, tau}},
    1 / 2 * {{-I * tau, 1 + I - tau}, {-1 + I + tau, I * tau}}], rho2fieldtheta]]], 10]];

```

*pgrpnames*

```
In[ ]:= pgrpnames = {"1", "2", "2'", "3", "3'", "4", "4'", "5", "6"}
```

```
Out[ ]:= {1, 2, 2', 3, 3', 4, 4', 5, 6}
```

*pgrp*

```
In[ ]:= pgrp = {rho1rep, rho2rep, rho2primerep,
  rho3rep, rho3primerep, rho4rep, rho4primerep, rho5rep, rho6rep};
```

*pgrpcharacterTable*

```
In[ ]:= TableForm[formatkappa[pgrpcharacterTable = toQkappa[
  Map[Flatten[Map[Union, Map[Tr, pquatmatsconjclasses /. #, {2}]]] &, pgrp]],
  TableHeadings -> {pgrpnames, MapThread[
    Column[{Length[#1], Length[sggen[#1][[1]]]}, #2] &,
    {pquatmatsconjclasses, pquatmatsconjclassnames}]]]
```

*Out[ ]//TableForm=*

|    |   |    |    |    |             |             |    |            |            |
|----|---|----|----|----|-------------|-------------|----|------------|------------|
|    | 1 | 1  | 20 | 30 | 12          | 12          | 20 | 12         | 12         |
|    | 1 | 2  | 3  | 4  | 5           | 5           | 6  | 10         | 10         |
|    | 1 | 2  | 3  | 4  | 5A          | 5B          | 6  | 10A        | 10B        |
| 1  | 1 | 1  | 1  | 1  | 1           | 1           | 1  | 1          | 1          |
| 2  | 2 | -2 | -1 | 0  | -1 + $\tau$ | - $\tau$    | 1  | $\tau$     | 1 - $\tau$ |
| 2' | 2 | -2 | -1 | 0  | - $\tau$    | -1 + $\tau$ | 1  | 1 - $\tau$ | $\tau$     |
| 3  | 3 | 3  | 0  | -1 | 1 - $\tau$  | $\tau$      | 0  | $\tau$     | 1 - $\tau$ |
| 3' | 3 | 3  | 0  | -1 | $\tau$      | 1 - $\tau$  | 0  | 1 - $\tau$ | $\tau$     |
| 4  | 4 | 4  | 1  | 0  | -1          | -1          | 1  | -1         | -1         |
| 4' | 4 | -4 | 1  | 0  | -1          | -1          | -1 | 1          | 1          |
| 5  | 5 | 5  | -1 | 1  | 0           | 0           | -1 | 0          | 0          |
| 6  | 6 | -6 | 0  | 0  | 1           | 1           | 0  | -1         | -1         |

```

In[ ]:= TableForm[
  formatkappa[toQkappa[Map[Flatten[Map[Union, Map[Tr, pquatmatsconjclasses /. #, {2}]]] &,
    {rho1rep, rho2rep, rho2primerep, rho2primeinvrep, rho3rep, rho3primerep,
      rho3primeinvrep, rho4rep, rho4alpharep, rho4alphainvrep, rho4primerep,
      rho4primealpharep, rho4primealphainvrep, rho5rep, rho5alpharep,
      rho5alphainvrep, rho6rep, rho6alpharep, rho6alphainvrep}]]],
  TableHeadings -> {pgrprepnames[{{1, 2, 3, 3, 4, 5, 5, 6, 6, 6, 7, 7, 7, 8, 8, 8, 9, 9, 9}}],
    MapThread[Column[{Length[#1], Length[sggen[#1][{1}]]], #2] &,
      {pquatmatsconjclasses, pquatmatsconjclassnames}]]]

```

Out[ ]:=TableForm=

|    |   |    |    |    |             |             |    |            |            |
|----|---|----|----|----|-------------|-------------|----|------------|------------|
|    | 1 | 1  | 20 | 30 | 12          | 12          | 20 | 12         | 12         |
|    | 1 | 2  | 3  | 4  | 5           | 5           | 6  | 10         | 10         |
|    | 1 | 2  | 3  | 4  | 5A          | 5B          | 6  | 10A        | 10B        |
| 1  | 1 | 1  | 1  | 1  | 1           | 1           | 1  | 1          | 1          |
| 2  | 2 | -2 | -1 | 0  | $-1 + \tau$ | $-\tau$     | 1  | $\tau$     | $1 - \tau$ |
| 2' | 2 | -2 | -1 | 0  | $-\tau$     | $-1 + \tau$ | 1  | $1 - \tau$ | $\tau$     |
| 2' | 2 | -2 | -1 | 0  | $-\tau$     | $-1 + \tau$ | 1  | $1 - \tau$ | $\tau$     |
| 3  | 3 | 3  | 0  | -1 | $1 - \tau$  | $\tau$      | 0  | $\tau$     | $1 - \tau$ |
| 3' | 3 | 3  | 0  | -1 | $\tau$      | $1 - \tau$  | 0  | $1 - \tau$ | $\tau$     |
| 3' | 3 | 3  | 0  | -1 | $\tau$      | $1 - \tau$  | 0  | $1 - \tau$ | $\tau$     |
| 4  | 4 | 4  | 1  | 0  | -1          | -1          | 1  | -1         | -1         |
| 4  | 4 | 4  | 1  | 0  | -1          | -1          | 1  | -1         | -1         |
| 4  | 4 | 4  | 1  | 0  | -1          | -1          | 1  | -1         | -1         |
| 4' | 4 | -4 | 1  | 0  | -1          | -1          | -1 | 1          | 1          |
| 4' | 4 | -4 | 1  | 0  | -1          | -1          | -1 | 1          | 1          |
| 4' | 4 | -4 | 1  | 0  | -1          | -1          | -1 | 1          | 1          |
| 5  | 5 | 5  | -1 | 1  | 0           | 0           | -1 | 0          | 0          |
| 5  | 5 | 5  | -1 | 1  | 0           | 0           | -1 | 0          | 0          |
| 5  | 5 | 5  | -1 | 1  | 0           | 0           | -1 | 0          | 0          |
| 6  | 6 | -6 | 0  | 0  | 1           | 1           | 0  | -1         | -1         |
| 6  | 6 | -6 | 0  | 0  | 1           | 1           | 0  | -1         | -1         |
| 6  | 6 | -6 | 0  | 0  | 1           | 1           | 0  | -1         | -1         |

characterableinnerproducts

```

In[ ]:= characterableinnerproducts[chartab_, sizes_] :=
  Outer[Total[#1 * #2 * sizes] / Total[sizes] &, chartab, chartab, 1];

In[ ]:= characterableinnerproducts[pgrpcharacterable, Map[Length, pquatmatsconjclasses]] ==
  IdentityMatrix[Length[pquatmatsconjclasses]] // FullSimplify

Out[ ]:= True

```

```

In[ ]:= Pick[pgrprepnames, Map[FullSimplify[(quaternionmatrix[quaternion[-1, 0, 0, 0]] /. #) ==
  - (quaternionmatrix[quaternion[1, 0, 0, 0]] /. #)] &, pgrpreps]]

```

Out[ ]:= {2, 2', 4', 6}

```

In[ ]:= Map[Sort, Map[pquatsalphaautoperm[[]] &, pquatmatsconjclasses /. pquatmatsrules]] ==
  Map[Sort, pquatmatsconjclasses /. pquatmatsrules][[{{1, 2, 3, 4, 6, 5, 7, 9, 8}}]]

```

Out[ ]:= True

```
In[4]:= Map[Sort, Map[pquatsalphaautoinvperm[ $\{ \# \}$ ] &, pquatmatsconjclasses /. pquatmatsrules]] ==  
Map[Sort, pquatmatsconjclasses /. pquatmatsrules][ $\{ \{ 1, 2, 3, 4, 6, 5, 7, 9, 8 \} \}$ ]
```

`Out[•]= True`

```
In[*]:= pgrpcharacterTable[[{1, 3, 2, 5, 4, 6, 7, 8, 9}]] ==  
pgrpcharacterTable[[All, {1, 2, 3, 4, 6, 5, 7, 9, 8}]]
```

*Out[•]*= True

*copsymliftgrp*

```
ln[•]:= Dimensions[copsymliftgrp = Select[davisopsymliftgrp, #[[3]] == 0 &]]
```

$$Out[\bullet]= \{14\,400\}$$

*copsymliftconjclasses*

```
In[ ]:= AbsoluteTiming[
  Map[Length, copsymliftconjclasses = SortBy[FixedPoint[Function[xp, If[xp[[2]] == {},
    xp, Function[cx, {Append[xp[[1]], cx], Complement[xp[[2]], cx}]]],
    Union[Map[davisopsymliftmultiply[davisopsymliftmultiply[#, xp[[2, 1]]],
      davisopsymliftinverse[#]] &, copsymliftgrp]]]],
    {{}, copsymliftgrp}][[1]], {davisopsymliftorder[#[[1]], Length[#]] &}]
```

$Out(*) = \{13.1941, \{1, 1, 1, 1, 20, 20, 400, 30, 30, 30, 30, 900, 12, 12, 12, 12, 144, 144, 144, 144, 20, 20, 20, 20, 20, 400, 400, 400, 12, 12, 12, 12, 12, 12, 12, 12, 12, 12, 12, 144, 144, 144, 144, 144, 144, 144, 144, 144, 144, 144, 144, 144, 600, 600, 600, 600, 240, 240, 240, 240, 360, 360, 360, 360, 360, 360, 360, 360, 240, 240, 240, 240, 240, 240, 240, 240, 240, 240, 240, 240\}\}$

```
In[•]:= Length[%[[2]]]
```

*Out[•]*= 81

```
in[8]:= Apply[Union, Outer[Apply[Union, Outer[davisopsymlift[#1, #2, 0] &, #1, #2, 1]] &,
    pquatmatconjclasses /. pquatmatrules,
    pquatmatconjclasses /. pquatmatrules, 1]] = Union[copsymliftconjclasses]
```

`Out[•]= True`

*copsymliftconjclasses*

```
In[*]:= Dimensions[copsymliftconjclasses =
  Flatten[Outer[Apply[Union, Outer[davisopsymlift[#1, #2, 0] &, #1, #2, 1]] &,
    pquatmatsconjclasses /. pquatmatsrules, pquatmatsconjclasses /. pquatmatsrules, 1], 1]]
```

$$Out[\bullet]= \{81\}$$

```
Inf := Union[pquatmatsconjclasses] == Union[pquats]
```

*Out[●]*= False

copsymliftconjclassnames

```
In[ ]:= copsymliftconjclassnames =
  Flatten[Outer[#1 <> "x" <> #2 &, {"1", "2", "3", "4", "5A", "5B", "6", "10A", "10B"},
    {"1", "2", "3", "4", "5A", "5B", "6", "10A", "10B"}, 1], 1]
```

```
Out[ ]:= {1×1, 1×2, 1×3, 1×4, 1×5A, 1×5B, 1×6, 1×10A, 1×10B, 2×1, 2×2, 2×3, 2×4, 2×5A, 2×5B, 2×6,
  2×10A, 2×10B, 3×1, 3×2, 3×3, 3×4, 3×5A, 3×5B, 3×6, 3×10A, 3×10B, 4×1, 4×2, 4×3, 4×4,
  4×5A, 4×5B, 4×6, 4×10A, 4×10B, 5A×1, 5A×2, 5A×3, 5A×4, 5A×5A, 5A×5B, 5A×6, 5A×10A,
  5A×10B, 5B×1, 5B×2, 5B×3, 5B×4, 5B×5A, 5B×5B, 5B×6, 5B×10A, 5B×10B, 6×1, 6×2, 6×3,
  6×4, 6×5A, 6×5B, 6×6, 6×10A, 6×10B, 10A×1, 10A×2, 10A×3, 10A×4, 10A×5A, 10A×5B, 10A×6,
  10A×10A, 10A×10B, 10B×1, 10B×2, 10B×3, 10B×4, 10B×5A, 10B×5B, 10B×6, 10B×10A, 10B×10B}
```

```
In[ ]:= TableForm[
  Map[{davisopsymliftorder[#[[1]]], Length[#], {Map[formatkappa, pquats[#[[1, 1]]]]},
    Map[formatkappa, pquats[#[[1, 2]]]]}], copsymliftconjclasses],
  TableHeadings → {copsymliftconjclassnames, {"order", "size", "rep"}}, TableDepth → 2]
```

Out[ ]:=TableForm=

|       | order | size | rep                                                                                                                                                                                           |
|-------|-------|------|-----------------------------------------------------------------------------------------------------------------------------------------------------------------------------------------------|
| 1×1   | 1     | 1    | {1, 1}                                                                                                                                                                                        |
| 1×2   | 2     | 1    | {1, -1}                                                                                                                                                                                       |
| 1×3   | 3     | 20   | $\left\{1, -\frac{1}{2} + \mathbb{K} \left(\frac{1}{2} - \frac{\tau}{2}\right) - \frac{i\tau}{2}\right\}$                                                                                     |
| 1×4   | 4     | 30   | {1, -i}                                                                                                                                                                                       |
| 1×5A  | 5     | 12   | $\left\{1, -\frac{1}{2} - \frac{j}{2} + \frac{\tau}{2} - \frac{i\tau}{2}\right\}$                                                                                                             |
| 1×5B  | 5     | 12   | $\left\{1, -\frac{i}{2} + j \left(\frac{1}{2} - \frac{\tau}{2}\right) - \frac{\tau}{2}\right\}$                                                                                               |
| 1×6   | 6     | 20   | $\left\{1, \frac{1}{2} + \mathbb{K} \left(\frac{1}{2} - \frac{\tau}{2}\right) - \frac{i\tau}{2}\right\}$                                                                                      |
| 1×10A | 10    | 12   | $\left\{1, -\frac{i}{2} + j \left(\frac{1}{2} - \frac{\tau}{2}\right) + \frac{\tau}{2}\right\}$                                                                                               |
| 1×10B | 10    | 12   | $\left\{1, \frac{1}{2} - \frac{j}{2} - \frac{\tau}{2} - \frac{i\tau}{2}\right\}$                                                                                                              |
| 2×1   | 2     | 1    | {-1, 1}                                                                                                                                                                                       |
| 2×2   | 2     | 1    | {-1, -1}                                                                                                                                                                                      |
| 2×3   | 6     | 20   | $\left\{-1, -\frac{1}{2} + \mathbb{K} \left(\frac{1}{2} - \frac{\tau}{2}\right) - \frac{i\tau}{2}\right\}$                                                                                    |
| 2×4   | 4     | 30   | {-1, -i}                                                                                                                                                                                      |
| 2×5A  | 10    | 12   | $\left\{-1, -\frac{1}{2} - \frac{j}{2} + \frac{\tau}{2} - \frac{i\tau}{2}\right\}$                                                                                                            |
| 2×5B  | 10    | 12   | $\left\{-1, -\frac{i}{2} + j \left(\frac{1}{2} - \frac{\tau}{2}\right) - \frac{\tau}{2}\right\}$                                                                                              |
| 2×6   | 6     | 20   | $\left\{-1, \frac{1}{2} + \mathbb{K} \left(\frac{1}{2} - \frac{\tau}{2}\right) - \frac{i\tau}{2}\right\}$                                                                                     |
| 2×10A | 10    | 12   | $\left\{-1, -\frac{i}{2} + j \left(\frac{1}{2} - \frac{\tau}{2}\right) + \frac{\tau}{2}\right\}$                                                                                              |
| 2×10B | 10    | 12   | $\left\{-1, \frac{1}{2} - \frac{j}{2} - \frac{\tau}{2} - \frac{i\tau}{2}\right\}$                                                                                                             |
| 3×1   | 3     | 20   | $\left\{-\frac{1}{2} + \mathbb{K} \left(\frac{1}{2} - \frac{\tau}{2}\right) - \frac{i\tau}{2}, 1\right\}$                                                                                     |
| 3×2   | 6     | 20   | $\left\{-\frac{1}{2} + \mathbb{K} \left(\frac{1}{2} - \frac{\tau}{2}\right) - \frac{i\tau}{2}, -1\right\}$                                                                                    |
| 3×3   | 3     | 400  | $\left\{-\frac{1}{2} + \mathbb{K} \left(\frac{1}{2} - \frac{\tau}{2}\right) - \frac{i\tau}{2}, -\frac{1}{2} + \mathbb{K} \left(\frac{1}{2} - \frac{\tau}{2}\right) - \frac{i\tau}{2}\right\}$ |
| 3×4   | 12    | 600  | $\left\{-\frac{1}{2} + \mathbb{K} \left(\frac{1}{2} - \frac{\tau}{2}\right) - \frac{i\tau}{2}, -i\right\}$                                                                                    |
| 3×5A  | 15    | 240  | $\left\{-\frac{1}{2} + \mathbb{K} \left(\frac{1}{2} - \frac{\tau}{2}\right) - \frac{i\tau}{2}, -\frac{1}{2} - \frac{j}{2} + \frac{\tau}{2} - \frac{i\tau}{2}\right\}$                         |
| 3×5B  | 15    | 240  | $\left\{-\frac{1}{2} + \mathbb{K} \left(\frac{1}{2} - \frac{\tau}{2}\right) - \frac{i\tau}{2}, -\frac{i}{2} + j \left(\frac{1}{2} - \frac{\tau}{2}\right) - \frac{\tau}{2}\right\}$           |

|        |    |     |                                                                                                                                                                                                    |
|--------|----|-----|----------------------------------------------------------------------------------------------------------------------------------------------------------------------------------------------------|
| 3×6    | 6  | 400 | $\left\{ -\frac{1}{2} + \mathbb{k} \left( \frac{1}{2} - \frac{\tau}{2} \right) - \frac{i\tau}{2}, \frac{1}{2} + \mathbb{k} \left( \frac{1}{2} - \frac{\tau}{2} \right) - \frac{i\tau}{2} \right\}$ |
| 3×10A  | 30 | 240 | $\left\{ -\frac{1}{2} + \mathbb{k} \left( \frac{1}{2} - \frac{\tau}{2} \right) - \frac{i\tau}{2}, -\frac{i}{2} + \mathbb{j} \left( \frac{1}{2} - \frac{\tau}{2} \right) + \frac{\tau}{2} \right\}$ |
| 3×10B  | 30 | 240 | $\left\{ -\frac{1}{2} + \mathbb{k} \left( \frac{1}{2} - \frac{\tau}{2} \right) - \frac{i\tau}{2}, \frac{1}{2} - \frac{j}{2} - \frac{\tau}{2} - \frac{i\tau}{2} \right\}$                           |
| 4×1    | 4  | 30  | $\{-i, 1\}$                                                                                                                                                                                        |
| 4×2    | 4  | 30  | $\{-i, -1\}$                                                                                                                                                                                       |
| 4×3    | 12 | 600 | $\left\{ -i, -\frac{1}{2} + \mathbb{k} \left( \frac{1}{2} - \frac{\tau}{2} \right) - \frac{i\tau}{2} \right\}$                                                                                     |
| 4×4    | 4  | 900 | $\{-i, -i\}$                                                                                                                                                                                       |
| 4×5A   | 20 | 360 | $\left\{ -i, -\frac{1}{2} - \frac{j}{2} + \frac{\tau}{2} - \frac{i\tau}{2} \right\}$                                                                                                               |
| 4×5B   | 20 | 360 | $\left\{ -i, -\frac{i}{2} + \mathbb{j} \left( \frac{1}{2} - \frac{\tau}{2} \right) - \frac{\tau}{2} \right\}$                                                                                      |
| 4×6    | 12 | 600 | $\left\{ -i, \frac{1}{2} + \mathbb{k} \left( \frac{1}{2} - \frac{\tau}{2} \right) - \frac{i\tau}{2} \right\}$                                                                                      |
| 4×10A  | 20 | 360 | $\left\{ -i, -\frac{i}{2} + \mathbb{j} \left( \frac{1}{2} - \frac{\tau}{2} \right) + \frac{\tau}{2} \right\}$                                                                                      |
| 4×10B  | 20 | 360 | $\left\{ -i, \frac{1}{2} - \frac{j}{2} - \frac{\tau}{2} - \frac{i\tau}{2} \right\}$                                                                                                                |
| 5A×1   | 5  | 12  | $\left\{ -\frac{1}{2} - \frac{j}{2} + \frac{\tau}{2} - \frac{i\tau}{2}, 1 \right\}$                                                                                                                |
| 5A×2   | 10 | 12  | $\left\{ -\frac{1}{2} - \frac{j}{2} + \frac{\tau}{2} - \frac{i\tau}{2}, -1 \right\}$                                                                                                               |
| 5A×3   | 15 | 240 | $\left\{ -\frac{1}{2} - \frac{j}{2} + \frac{\tau}{2} - \frac{i\tau}{2}, -\frac{1}{2} + \mathbb{k} \left( \frac{1}{2} - \frac{\tau}{2} \right) - \frac{i\tau}{2} \right\}$                          |
| 5A×4   | 20 | 360 | $\left\{ -\frac{1}{2} - \frac{j}{2} + \frac{\tau}{2} - \frac{i\tau}{2}, -i \right\}$                                                                                                               |
| 5A×5A  | 5  | 144 | $\left\{ -\frac{1}{2} - \frac{j}{2} + \frac{\tau}{2} - \frac{i\tau}{2}, -\frac{1}{2} - \frac{j}{2} + \frac{\tau}{2} - \frac{i\tau}{2} \right\}$                                                    |
| 5A×5B  | 5  | 144 | $\left\{ -\frac{1}{2} - \frac{j}{2} + \frac{\tau}{2} - \frac{i\tau}{2}, -\frac{i}{2} + \mathbb{j} \left( \frac{1}{2} - \frac{\tau}{2} \right) - \frac{\tau}{2} \right\}$                           |
| 5A×6   | 30 | 240 | $\left\{ -\frac{1}{2} - \frac{j}{2} + \frac{\tau}{2} - \frac{i\tau}{2}, \frac{1}{2} + \mathbb{k} \left( \frac{1}{2} - \frac{\tau}{2} \right) - \frac{i\tau}{2} \right\}$                           |
| 5A×10A | 10 | 144 | $\left\{ -\frac{1}{2} - \frac{j}{2} + \frac{\tau}{2} - \frac{i\tau}{2}, -\frac{i}{2} + \mathbb{j} \left( \frac{1}{2} - \frac{\tau}{2} \right) + \frac{\tau}{2} \right\}$                           |
| 5A×10B | 10 | 144 | $\left\{ -\frac{1}{2} - \frac{j}{2} + \frac{\tau}{2} - \frac{i\tau}{2}, \frac{1}{2} - \frac{j}{2} - \frac{\tau}{2} - \frac{i\tau}{2} \right\}$                                                     |
| 5B×1   | 5  | 12  | $\left\{ -\frac{i}{2} + \mathbb{j} \left( \frac{1}{2} - \frac{\tau}{2} \right) - \frac{\tau}{2}, 1 \right\}$                                                                                       |
| 5B×2   | 10 | 12  | $\left\{ -\frac{i}{2} + \mathbb{j} \left( \frac{1}{2} - \frac{\tau}{2} \right) - \frac{\tau}{2}, -1 \right\}$                                                                                      |
| 5B×3   | 15 | 240 | $\left\{ -\frac{i}{2} + \mathbb{j} \left( \frac{1}{2} - \frac{\tau}{2} \right) - \frac{\tau}{2}, -\frac{1}{2} + \mathbb{k} \left( \frac{1}{2} - \frac{\tau}{2} \right) - \frac{i\tau}{2} \right\}$ |
| 5B×4   | 20 | 360 | $\left\{ -\frac{i}{2} + \mathbb{j} \left( \frac{1}{2} - \frac{\tau}{2} \right) - \frac{\tau}{2}, -i \right\}$                                                                                      |
| 5B×5A  | 5  | 144 | $\left\{ -\frac{i}{2} + \mathbb{j} \left( \frac{1}{2} - \frac{\tau}{2} \right) - \frac{\tau}{2}, -\frac{1}{2} - \frac{j}{2} + \frac{\tau}{2} - \frac{i\tau}{2} \right\}$                           |
| 5B×5B  | 5  | 144 | $\left\{ -\frac{i}{2} + \mathbb{j} \left( \frac{1}{2} - \frac{\tau}{2} \right) - \frac{\tau}{2}, -\frac{i}{2} + \mathbb{j} \left( \frac{1}{2} - \frac{\tau}{2} \right) - \frac{\tau}{2} \right\}$  |
| 5B×6   | 30 | 240 | $\left\{ -\frac{i}{2} + \mathbb{j} \left( \frac{1}{2} - \frac{\tau}{2} \right) - \frac{\tau}{2}, \frac{1}{2} + \mathbb{k} \left( \frac{1}{2} - \frac{\tau}{2} \right) - \frac{i\tau}{2} \right\}$  |
| 5B×10A | 10 | 144 | $\left\{ -\frac{i}{2} + \mathbb{j} \left( \frac{1}{2} - \frac{\tau}{2} \right) - \frac{\tau}{2}, -\frac{i}{2} + \mathbb{j} \left( \frac{1}{2} - \frac{\tau}{2} \right) + \frac{\tau}{2} \right\}$  |
| 5B×10B | 10 | 144 | $\left\{ -\frac{i}{2} + \mathbb{j} \left( \frac{1}{2} - \frac{\tau}{2} \right) - \frac{\tau}{2}, \frac{1}{2} - \frac{j}{2} - \frac{\tau}{2} - \frac{i\tau}{2} \right\}$                            |
| 6×1    | 6  | 20  | $\left\{ \frac{1}{2} + \mathbb{k} \left( \frac{1}{2} - \frac{\tau}{2} \right) - \frac{i\tau}{2}, 1 \right\}$                                                                                       |
| 6×2    | 6  | 20  | $\left\{ \frac{1}{2} + \mathbb{k} \left( \frac{1}{2} - \frac{\tau}{2} \right) - \frac{i\tau}{2}, -1 \right\}$                                                                                      |
| 6×3    | 6  | 400 | $\left\{ \frac{1}{2} + \mathbb{k} \left( \frac{1}{2} - \frac{\tau}{2} \right) - \frac{i\tau}{2}, -\frac{1}{2} + \mathbb{k} \left( \frac{1}{2} - \frac{\tau}{2} \right) - \frac{i\tau}{2} \right\}$ |

|         |    |     |                                                                                                                                                                                                   |
|---------|----|-----|---------------------------------------------------------------------------------------------------------------------------------------------------------------------------------------------------|
| 6×4     | 12 | 600 | $\left\{ \frac{1}{2} + \mathbb{K} \left( \frac{1}{2} - \frac{\tau}{2} \right) - \frac{i\tau}{2}, -i \right\}$                                                                                     |
| 6×5A    | 30 | 240 | $\left\{ \frac{1}{2} + \mathbb{K} \left( \frac{1}{2} - \frac{\tau}{2} \right) - \frac{i\tau}{2}, -\frac{1}{2} - \frac{j}{2} + \frac{\tau}{2} - \frac{i\tau}{2} \right\}$                          |
| 6×5B    | 30 | 240 | $\left\{ \frac{1}{2} + \mathbb{K} \left( \frac{1}{2} - \frac{\tau}{2} \right) - \frac{i\tau}{2}, -\frac{i}{2} + j \left( \frac{1}{2} - \frac{\tau}{2} \right) - \frac{\tau}{2} \right\}$          |
| 6×6     | 6  | 400 | $\left\{ \frac{1}{2} + \mathbb{K} \left( \frac{1}{2} - \frac{\tau}{2} \right) - \frac{i\tau}{2}, \frac{1}{2} + \mathbb{K} \left( \frac{1}{2} - \frac{\tau}{2} \right) - \frac{i\tau}{2} \right\}$ |
| 6×10A   | 30 | 240 | $\left\{ \frac{1}{2} + \mathbb{K} \left( \frac{1}{2} - \frac{\tau}{2} \right) - \frac{i\tau}{2}, -\frac{i}{2} + j \left( \frac{1}{2} - \frac{\tau}{2} \right) + \frac{\tau}{2} \right\}$          |
| 6×10B   | 30 | 240 | $\left\{ \frac{1}{2} + \mathbb{K} \left( \frac{1}{2} - \frac{\tau}{2} \right) - \frac{i\tau}{2}, \frac{1}{2} - \frac{j}{2} - \frac{\tau}{2} - \frac{i\tau}{2} \right\}$                           |
| 10A×1   | 10 | 12  | $\left\{ -\frac{i}{2} + j \left( \frac{1}{2} - \frac{\tau}{2} \right) + \frac{\tau}{2}, 1 \right\}$                                                                                               |
| 10A×2   | 10 | 12  | $\left\{ -\frac{i}{2} + j \left( \frac{1}{2} - \frac{\tau}{2} \right) + \frac{\tau}{2}, -1 \right\}$                                                                                              |
| 10A×3   | 30 | 240 | $\left\{ -\frac{i}{2} + j \left( \frac{1}{2} - \frac{\tau}{2} \right) + \frac{\tau}{2}, -\frac{1}{2} + \mathbb{K} \left( \frac{1}{2} - \frac{\tau}{2} \right) - \frac{i\tau}{2} \right\}$         |
| 10A×4   | 20 | 360 | $\left\{ -\frac{i}{2} + j \left( \frac{1}{2} - \frac{\tau}{2} \right) + \frac{\tau}{2}, -i \right\}$                                                                                              |
| 10A×5A  | 10 | 144 | $\left\{ -\frac{i}{2} + j \left( \frac{1}{2} - \frac{\tau}{2} \right) + \frac{\tau}{2}, -\frac{1}{2} - \frac{j}{2} + \frac{\tau}{2} - \frac{i\tau}{2} \right\}$                                   |
| 10A×5B  | 10 | 144 | $\left\{ -\frac{i}{2} + j \left( \frac{1}{2} - \frac{\tau}{2} \right) + \frac{\tau}{2}, -\frac{i}{2} + j \left( \frac{1}{2} - \frac{\tau}{2} \right) - \frac{\tau}{2} \right\}$                   |
| 10A×6   | 30 | 240 | $\left\{ -\frac{i}{2} + j \left( \frac{1}{2} - \frac{\tau}{2} \right) + \frac{\tau}{2}, \frac{1}{2} + \mathbb{K} \left( \frac{1}{2} - \frac{\tau}{2} \right) - \frac{i\tau}{2} \right\}$          |
| 10A×10A | 10 | 144 | $\left\{ -\frac{i}{2} + j \left( \frac{1}{2} - \frac{\tau}{2} \right) + \frac{\tau}{2}, -\frac{i}{2} + j \left( \frac{1}{2} - \frac{\tau}{2} \right) + \frac{\tau}{2} \right\}$                   |
| 10A×10B | 10 | 144 | $\left\{ -\frac{i}{2} + j \left( \frac{1}{2} - \frac{\tau}{2} \right) + \frac{\tau}{2}, \frac{1}{2} - \frac{j}{2} - \frac{\tau}{2} - \frac{i\tau}{2} \right\}$                                    |
| 10B×1   | 10 | 12  | $\left\{ \frac{1}{2} - \frac{j}{2} - \frac{\tau}{2} - \frac{i\tau}{2}, 1 \right\}$                                                                                                                |
| 10B×2   | 10 | 12  | $\left\{ \frac{1}{2} - \frac{j}{2} - \frac{\tau}{2} - \frac{i\tau}{2}, -1 \right\}$                                                                                                               |
| 10B×3   | 30 | 240 | $\left\{ \frac{1}{2} - \frac{j}{2} - \frac{\tau}{2} - \frac{i\tau}{2}, -\frac{1}{2} + \mathbb{K} \left( \frac{1}{2} - \frac{\tau}{2} \right) - \frac{i\tau}{2} \right\}$                          |
| 10B×4   | 20 | 360 | $\left\{ \frac{1}{2} - \frac{j}{2} - \frac{\tau}{2} - \frac{i\tau}{2}, -i \right\}$                                                                                                               |
| 10B×5A  | 10 | 144 | $\left\{ \frac{1}{2} - \frac{j}{2} - \frac{\tau}{2} - \frac{i\tau}{2}, -\frac{1}{2} - \frac{j}{2} + \frac{\tau}{2} - \frac{i\tau}{2} \right\}$                                                    |
| 10B×5B  | 10 | 144 | $\left\{ \frac{1}{2} - \frac{j}{2} - \frac{\tau}{2} - \frac{i\tau}{2}, -\frac{i}{2} + j \left( \frac{1}{2} - \frac{\tau}{2} \right) - \frac{\tau}{2} \right\}$                                    |
| 10B×6   | 30 | 240 | $\left\{ \frac{1}{2} - \frac{j}{2} - \frac{\tau}{2} - \frac{i\tau}{2}, \frac{1}{2} + \mathbb{K} \left( \frac{1}{2} - \frac{\tau}{2} \right) - \frac{i\tau}{2} \right\}$                           |
| 10B×10A | 10 | 144 | $\left\{ \frac{1}{2} - \frac{j}{2} - \frac{\tau}{2} - \frac{i\tau}{2}, -\frac{i}{2} + j \left( \frac{1}{2} - \frac{\tau}{2} \right) + \frac{\tau}{2} \right\}$                                    |
| 10B×10B | 10 | 144 | $\left\{ \frac{1}{2} - \frac{j}{2} - \frac{\tau}{2} - \frac{i\tau}{2}, \frac{1}{2} - \frac{j}{2} - \frac{\tau}{2} - \frac{i\tau}{2} \right\}$                                                     |

copsymliftreps, r, s

```

In[ ]:= Dimensions[copsymliftreps =
  Flatten[Outer[With[{r = #1, s = #2}, davisopsymlift[i_, j_, 0] ⇨ KroneckerProduct[
    pquatmats[[i]] /. r, pquatmats[[j]] /. s]] &,
    {rho1rep, rho2rep, rho2primerep, rho3rep, rho3primerep, rho4rep, rho4primerep,
      rho5rep, rho6rep}, {rho1rep, rho2rep, rho2primerep, rho3rep,
      rho3primerep, rho4rep, rho4primerep, rho5rep, rho6rep}, 1], 1]]

```

Out[ ]:= {81}

copsymliftreprenames

```
In[ ]:= copsymliftreprenames =
  Flatten[Outer[#1 <> "x" <> #2 &, {"1", "2", "2'", "3", "3'", "4", "4'", "5", "6"},
    {"1", "2", "2'", "3", "3'", "4", "4'", "5", "6"}, 1], 1]
```

```
Out[ ]:= {1×1, 1×2, 1×2', 1×3, 1×3', 1×4, 1×4', 1×5, 1×6, 2×1, 2×2, 2×2', 2×3,
  2×3', 2×4, 2×4', 2×5, 2×6, 2'×1, 2'×2, 2'×2', 2'×3, 2'×3', 2'×4, 2'×4', 2'×5,
  2'×6, 3×1, 3×2, 3×2', 3×3, 3×3', 3×4, 3×4', 3×5, 3×6, 3'×1, 3'×2, 3'×2', 3'×3,
  3'×3', 3'×4, 3'×4', 3'×5, 3'×6, 4×1, 4×2, 4×2', 4×3, 4×3', 4×4, 4×4', 4×5,
  4×6, 4'×1, 4'×2, 4'×2', 4'×3, 4'×3', 4'×4, 4'×4', 4'×5, 4'×6, 5×1, 5×2, 5×2',
  5×3, 5×3', 5×4, 5×4', 5×5, 5×6, 6×1, 6×2, 6×2', 6×3, 6×3', 6×4, 6×4', 6×5, 6×6}
```

copsymliftcharacterstable

```
In[ ]:= TableForm[formatkappa[copsymliftcharacterstable = toQkappa[
  RootReduce[Map[Map[Tr, copsymliftconjclasses[All, 1]] /. #] &, copsymliftreps]]],
  TableHeadings -> {copsymliftreprenames, MapThread[
    Column[Length[#1], davisopsymliftorder[#1[[1]]], #2], ItemSize -> {5, Automatic}] &,
  {Flatten[Outer[Flatten[Outer[davisopsymlift[#1, #2, 0] &, #1, #2, 1], 1] &,
    pquatmatsconjclasses /. pquatmatsrules,
    pquatmatsconjclasses /. pquatmatsrules, 1], 1], copsymliftconjclassnames}}]
```

Out[ ]//TableForm=

|       | 1   | 1   | 20  | 30  | 12            | 12            | 20  |
|-------|-----|-----|-----|-----|---------------|---------------|-----|
|       | 1   | 2   | 3   | 4   | 5             | 5             | 6   |
|       | 1×1 | 1×2 | 1×3 | 1×4 | 1×5A          | 1×5B          | 1×6 |
| 1×1   | 1   | 1   | 1   | 1   | 1             | 1             | 1   |
| 1×2   | 2   | -2  | -1  | 0   | -1 + $\tau$   | - $\tau$      | 1   |
| 1×2'  | 2   | -2  | -1  | 0   | - $\tau$      | -1 + $\tau$   | 1   |
| 1×3   | 3   | 3   | 0   | -1  | 1 - $\tau$    | $\tau$        | 0   |
| 1×3'  | 3   | 3   | 0   | -1  | $\tau$        | 1 - $\tau$    | 0   |
| 1×4   | 4   | 4   | 1   | 0   | -1            | -1            | 1   |
| 1×4'  | 4   | -4  | 1   | 0   | -1            | -1            | -1  |
| 1×5   | 5   | 5   | -1  | 1   | 0             | 0             | -1  |
| 1×6   | 6   | -6  | 0   | 0   | 1             | 1             | 0   |
| 2×1   | 2   | 2   | 2   | 2   | 2             | 2             | 2   |
| 2×2   | 4   | -4  | -2  | 0   | -2 + 2 $\tau$ | -2 $\tau$     | 2   |
| 2×2'  | 4   | -4  | -2  | 0   | -2 $\tau$     | -2 + 2 $\tau$ | 2   |
| 2×3   | 6   | 6   | 0   | -2  | 2 - 2 $\tau$  | 2 $\tau$      | 0   |
| 2×3'  | 6   | 6   | 0   | -2  | 2 $\tau$      | 2 - 2 $\tau$  | 0   |
| 2×4   | 8   | 8   | 2   | 0   | -2            | -2            | 2   |
| 2×4'  | 8   | -8  | 2   | 0   | -2            | -2            | -2  |
| 2×5   | 10  | 10  | -2  | 2   | 0             | 0             | -2  |
| 2×6   | 12  | -12 | 0   | 0   | 2             | 2             | 0   |
| 2'×1  | 2   | 2   | 2   | 2   | 2             | 2             | 2   |
| 2'×2  | 4   | -4  | -2  | 0   | -2 + 2 $\tau$ | -2 $\tau$     | 2   |
| 2'×2' | 4   | -4  | -2  | 0   | -2 $\tau$     | -2 + 2 $\tau$ | 2   |
| 2'×3  | 6   | 6   | 0   | -2  | 2 - 2 $\tau$  | 2 $\tau$      | 0   |
| 2'×3' | 6   | 6   | 0   | -2  | 2 $\tau$      | 2 - 2 $\tau$  | 0   |
| 2'×4  | 8   | 8   | 2   | 0   | -2            | -2            | 2   |
| 2'×4' | 8   | -8  | 2   | 0   | -2            | -2            | -2  |
| 2'×5  | 10  | 10  | -2  | 2   | 0             | 0             | -2  |
| 2'×6  | 12  | -12 | 0   | 0   | 2             | 2             | 0   |
| 3×1   | 3   | 3   | 3   | 3   | 3             | 3             | 3   |



|                |    |     |    |    |               |               |    |
|----------------|----|-----|----|----|---------------|---------------|----|
| $3 \times 2$   | 6  | -6  | -3 | 0  | $-3 + 3 \tau$ | $-3 \tau$     | 3  |
| $3 \times 2'$  | 6  | -6  | -3 | 0  | $-3 \tau$     | $-3 + 3 \tau$ | 3  |
| $3 \times 3$   | 9  | 9   | 0  | -3 | $3 - 3 \tau$  | $3 \tau$      | 0  |
| $3 \times 3'$  | 9  | 9   | 0  | -3 | $3 \tau$      | $3 - 3 \tau$  | 0  |
| $3 \times 4$   | 12 | 12  | 3  | 0  | -3            | -3            | 3  |
| $3 \times 4'$  | 12 | -12 | 3  | 0  | -3            | -3            | -3 |
| $3 \times 5$   | 15 | 15  | -3 | 3  | 0             | 0             | -3 |
| $3 \times 6$   | 18 | -18 | 0  | 0  | 3             | 3             | 0  |
| $3' \times 1$  | 3  | 3   | 3  | 3  | 3             | 3             | 3  |
| $3' \times 2$  | 6  | -6  | -3 | 0  | $-3 + 3 \tau$ | $-3 \tau$     | 3  |
| $3' \times 2'$ | 6  | -6  | -3 | 0  | $-3 \tau$     | $-3 + 3 \tau$ | 3  |
| $3' \times 3$  | 9  | 9   | 0  | -3 | $3 - 3 \tau$  | $3 \tau$      | 0  |
| $3' \times 3'$ | 9  | 9   | 0  | -3 | $3 \tau$      | $3 - 3 \tau$  | 0  |
| $3' \times 4$  | 12 | 12  | 3  | 0  | -3            | -3            | 3  |
| $3' \times 4'$ | 12 | -12 | 3  | 0  | -3            | -3            | -3 |
| $3' \times 5$  | 15 | 15  | -3 | 3  | 0             | 0             | -3 |
| $3' \times 6$  | 18 | -18 | 0  | 0  | 3             | 3             | 0  |
| $4 \times 1$   | 4  | 4   | 4  | 4  | 4             | 4             | 4  |
| $4 \times 2$   | 8  | -8  | -4 | 0  | $-4 + 4 \tau$ | $-4 \tau$     | 4  |
| $4 \times 2'$  | 8  | -8  | -4 | 0  | $-4 \tau$     | $-4 + 4 \tau$ | 4  |
| $4 \times 3$   | 12 | 12  | 0  | -4 | $4 - 4 \tau$  | $4 \tau$      | 0  |
| $4 \times 3'$  | 12 | 12  | 0  | -4 | $4 \tau$      | $4 - 4 \tau$  | 0  |
| $4 \times 4$   | 16 | 16  | 4  | 0  | -4            | -4            | 4  |
| $4 \times 4'$  | 16 | -16 | 4  | 0  | -4            | -4            | -4 |
| $4 \times 5$   | 20 | 20  | -4 | 4  | 0             | 0             | -4 |
| $4 \times 6$   | 24 | -24 | 0  | 0  | 4             | 4             | 0  |
| $4' \times 1$  | 4  | 4   | 4  | 4  | 4             | 4             | 4  |
| $4' \times 2$  | 8  | -8  | -4 | 0  | $-4 + 4 \tau$ | $-4 \tau$     | 4  |
| $4' \times 2'$ | 8  | -8  | -4 | 0  | $-4 \tau$     | $-4 + 4 \tau$ | 4  |
| $4' \times 3$  | 12 | 12  | 0  | -4 | $4 - 4 \tau$  | $4 \tau$      | 0  |
| $4' \times 3'$ | 12 | 12  | 0  | -4 | $4 \tau$      | $4 - 4 \tau$  | 0  |
| $4' \times 4$  | 16 | 16  | 4  | 0  | -4            | -4            | 4  |
| $4' \times 4'$ | 16 | -16 | 4  | 0  | -4            | -4            | -4 |
| $4' \times 5$  | 20 | 20  | -4 | 4  | 0             | 0             | -4 |
| $4' \times 6$  | 24 | -24 | 0  | 0  | 4             | 4             | 0  |
| $5 \times 1$   | 5  | 5   | 5  | 5  | 5             | 5             | 5  |
| $5 \times 2$   | 10 | -10 | -5 | 0  | $-5 + 5 \tau$ | $-5 \tau$     | 5  |
| $5 \times 2'$  | 10 | -10 | -5 | 0  | $-5 \tau$     | $-5 + 5 \tau$ | 5  |
| $5 \times 3$   | 15 | 15  | 0  | -5 | $5 - 5 \tau$  | $5 \tau$      | 0  |
| $5 \times 3'$  | 15 | 15  | 0  | -5 | $5 \tau$      | $5 - 5 \tau$  | 0  |
| $5 \times 4$   | 20 | 20  | 5  | 0  | -5            | -5            | 5  |
| $5 \times 4'$  | 20 | -20 | 5  | 0  | -5            | -5            | -5 |
| $5 \times 5$   | 25 | 25  | -5 | 5  | 0             | 0             | -5 |
| $5 \times 6$   | 30 | -30 | 0  | 0  | 5             | 5             | 0  |
| $6 \times 1$   | 6  | 6   | 6  | 6  | 6             | 6             | 6  |
| $6 \times 2$   | 12 | -12 | -6 | 0  | $-6 + 6 \tau$ | $-6 \tau$     | 6  |
| $6 \times 2'$  | 12 | -12 | -6 | 0  | $-6 \tau$     | $-6 + 6 \tau$ | 6  |
| $6 \times 3$   | 18 | 18  | 0  | -6 | $6 - 6 \tau$  | $6 \tau$      | 0  |
| $6 \times 3'$  | 18 | 18  | 0  | -6 | $6 \tau$      | $6 - 6 \tau$  | 0  |
| $6 \times 4$   | 24 | 24  | 6  | 0  | -6            | -6            | 6  |

|               |    |     |    |   |    |    |    |
|---------------|----|-----|----|---|----|----|----|
| $6 \times 4'$ | 24 | -24 | 6  | 0 | -6 | -6 | -6 |
| $6 \times 5$  | 30 | 30  | -6 | 6 | 0  | 0  | -6 |
| $6 \times 6$  | 36 | -36 | 0  | 0 | 6  | 6  | 0  |

```
In[ ]:= CharacterTableInnerProducts[
  CopsymLiftCharacterTable, Map[Length, CopsymLiftConjClasses]] ==
  IdentityMatrix[Length[CopsymLiftConjClasses]] // FullSimplify
```

```
Out[ ]:= True
```

```
In[ ]:= KroneckerProduct[pgrpCharacterTable, pgrpCharacterTable] ==
  CopsymLiftCharacterTable // FullSimplify
```

```
Out[ ]:= True
```

```
In[ ]:= Pick[CopsymLiftRepNames, Map[
  (DavisOpsymLift[1, 1, 0] /. #) == -(DavisOpsymLift[120, 120, 0] /. #) &, CopsymLiftReps]]
```

```
Out[ ]:= {1x2, 1x2', 1x4', 1x6, 2x1, 2x3, 2x3', 2x4, 2x5, 2'x1, 2'x3, 2'x3', 2'x4,
  2'x5, 3x2, 3x2', 3x4', 3x6, 3'x2, 3'x2', 3'x4', 3'x6, 4x2, 4x2', 4x4', 4x6,
  4'x1, 4'x3, 4'x3', 4'x4, 4'x5, 5x2, 5x2', 5x4', 5x6, 6x1, 6x3, 6x3', 6x4, 6x5}
```

```
In[ ]:= Length[%]
```

```
Out[ ]:= 40
```

*selement*

```
In[ ]:= selement = DavisOpsymLift[1, 120, 1];
```

```
In[ ]:= TrueQ[Apply[And,
  Map[davisopsymLiftMultiply[davisopsymLiftMultiply[davisopsymLiftInverse[selement], #],
    selement] == davisopsymLift[pquatsAlphaAutoInvPerm[#[[2]]]],
  pquatsAlphaAutoPerm[#[[1]]], 0] &, CopsymLiftGrp]]]
```

```
Out[ ]:= True
```

```
In[ ]:= selement
```

```
Out[ ]:= DavisOpsymLift[1, 120, 1]
```

```
In[ ]:= TrueQ[
  Apply[And, Flatten[Table[davisopsymLift[i1, i2, j] == If[j == 0, davisopsymLift[i1, i2, 0],
    davisopsymLiftMultiply[davisopsymLift[pquatsMinusPerm[[i1]], i2, 0], selement]],
    {i1, 1, 120}, {i2, 1, 120}, {j, 0, 1}]]]]]
```

```
Out[ ]:= True
```

*davisopsymLiftTreptype1*

```
In[ ]:= davisopsymLiftTreptype1[r_, s_, pm_] := DavisOpsymLift[i1_, i2_, j_] =>
  If[j == 0, KroneckerProduct[pquatMats[[i1]] /. r, pquatMats[[i2]] /. s],
  pm * KroneckerProduct[pquatMats[[pquatsMinusPerm[[i1]]]] /. r, pquatMats[[i2]] /. s].
  Map[Flatten, Flatten[Transpose[
    Outer[KroneckerProduct, pquatMats[[120]] /. r, pquatMats[[120]] /. r, 1], 1]]];
```

davisopsymliftreptype2

```

In[ ]:= davisopsymliftreptype2[r_, s_, sp_, rp_] := davisopsymlift[i1_, i2_, j_] => If[j == 0,
  ArrayFlatten[{{KroneckerProduct[pquatmats[[i1]] /. r, pquatmats[[i2]] /. s], 0},
    {0, KroneckerProduct[pquatmats[[i1]] /. sp, pquatmats[[i2]] /. rp}}]],
  ArrayFlatten[{{KroneckerProduct[pquatmats[[pquatsminusperm[[i1]]]] /. r,
    pquatmats[[i2]] /. s], 0}, {0, KroneckerProduct[
    pquatmats[[pquatsminusperm[[i1]]]] /. sp, pquatmats[[i2]] /. rp}}]].
  ArrayFlatten[{{0, Map[Flatten, Flatten[Transpose[Outer[KroneckerProduct,
    pquatmats[[120]] /. s, pquatmats[[120]] /. r, 1]], 1]]},
    {Map[Flatten, Flatten[Transpose[Outer[KroneckerProduct,
    pquatmats[[120]] /. r, pquatmats[[120]] /. s, 1]], 1]], 0}}]]];

```

davisopsymliftrepnames, davisopsymliftreps

```

In[ ]:= {davisopsymliftreps, davisopsymliftrepnames} = Transpose[{
  {davisopsymliftreptype2[rho1rep, rho2rep, rho2primeinvrep, rho1rep], "1x2+2'x1"},
  {davisopsymliftreptype2[rho1rep, rho2primerep, rho2rep, rho1rep], "1x2'+2x1"},
  {davisopsymliftreptype2[rho1rep,
    rho4primerep, rho4primealphainvrep, rho1rep], "1x4'+4'x1"},
  {davisopsymliftreptype2[rho1rep, rho6rep, rho6alphainvrep, rho1rep], "1x6+6x1"},
  {davisopsymliftreptype2[rho2rep,
    rho3rep, rho3primeinvrep, rho2primerep], "2x3+3'x2"},
  {davisopsymliftreptype2[rho2rep, rho3primerep, rho3rep, rho2primerep], "2x3'+3x2"},
  {davisopsymliftreptype2[
    rho2primeinvrep, rho3rep, rho3primeinvrep, rho2rep], "2'x3+3'x2"},
  {davisopsymliftreptype2[rho2primeinvrep, rho3primerep, rho3rep, rho2rep],
    "2'x3'+3x2"},
  {davisopsymliftreptype2[rho2rep, rho4rep, rho4alphainvrep, rho2primerep],
    "2x4+4x2"},
  {davisopsymliftreptype2[rho2primeinvrep, rho4rep, rho4alphainvrep, rho2rep],
    "2'x4+4x2"},
  {davisopsymliftreptype2[rho2rep, rho5rep, rho5alphainvrep, rho2primerep],
    "2x5+5x2"},
  {davisopsymliftreptype2[rho2primeinvrep, rho5rep, rho5alphainvrep, rho2rep],
    "2'x5+5x2"},
  {davisopsymliftreptype2[rho3rep, rho4primerep, rho4primealphainvrep, rho3primerep],
    "3x4'+4'x3"},
  {davisopsymliftreptype2[rho3primeinvrep, rho4primerep,
    rho4primealphainvrep, rho3rep], "3'x4'+4'x3"},
  {davisopsymliftreptype2[rho4rep, rho4primerep, rho4primealphainvrep, rho4alpharep],
    "4x4'+4'x4"},
  {davisopsymliftreptype2[rho3rep, rho6rep, rho6alphainvrep, rho3primerep],
    "3x6+6x3"},
  {davisopsymliftreptype2[rho3primeinvrep, rho6rep, rho6alphainvrep, rho3rep],
    "3'x6+6x3"},
  {davisopsymliftreptype2[rho4primerep, rho5rep, rho5alphainvrep,
    rho4primealpharep], "4'x5+5x4"},
  {davisopsymliftreptype2[rho4rep, rho6rep, rho6alphainvrep, rho4alpharep], "4x6+6x4"},
  {davisopsymliftreptype2[rho5rep, rho6rep, rho6alphainvrep, rho5alpharep], "5x6+6x5"},
  {davisopsymliftreptype1[rho1rep, rho1rep, 1], "1x1"},
  {davisopsymliftreptype1[rho1rep, rho1rep, -1], "-1x1"},
  {davisopsymliftreptype1[rho2rep, rho2primerep, 1], "2x2"},
  {davisopsymliftreptype1[rho2rep, rho2primerep, -1], "-2x2"}];

```

```

{davisopsymliftreptype1[rho2primeinvrep, rho2rep, 1], "2'x2"},
{davisopsymliftreptype1[rho2primeinvrep, rho2rep, -1], "-2'x2"},
{davisopsymliftreptype2[rho1rep, rho3rep, rho3primeinvrep, rho1rep], "1x3+3'x1"},
{davisopsymliftreptype2[rho1rep, rho3primerep, rho3rep, rho1rep], "1x3'+3x1"},
{davisopsymliftreptype2[rho1rep, rho4rep, rho4alphainvrep, rho1rep], "1x4+4x1"},
{davisopsymliftreptype2[rho2rep,
  rho2rep, rho2primeinvrep, rho2primerep], "2x2+2'x2"},
{davisopsymliftreptype1[rho3rep, rho3primerep, 1], "3x3"},
{davisopsymliftreptype1[rho3rep, rho3primerep, -1], "-3x3"},
{davisopsymliftreptype1[rho3primeinvrep, rho3rep, 1], "3'x3"},
{davisopsymliftreptype1[rho3primeinvrep, rho3rep, -1], "-3'x3"},
{davisopsymliftreptype2[rho1rep, rho5rep, rho5alphainvrep, rho1rep], "1x5+5x1"},
{davisopsymliftreptype2[rho2rep,
  rho4primerep, rho4primealphainvrep, rho2primerep], "2x4'+4'x2"},
{davisopsymliftreptype2[rho2primeinvrep, rho4primerep,
  rho4primealphainvrep, rho2rep], "2'x4'+4'x2"},
{davisopsymliftreptype1[rho4rep, rho4alpharep, 1], "4x4"},
{davisopsymliftreptype1[rho4rep, rho4alpharep, -1], "-4x4"},
{davisopsymliftreptype1[rho4primerep, rho4primealpharep, 1], "4'x4'"},
{davisopsymliftreptype1[rho4primerep, rho4primealpharep, -1], "-4'x4'"},
{davisopsymliftreptype2[rho3rep,
  rho3rep, rho3primeinvrep, rho3primerep], "3x3+3'x3'"},
{davisopsymliftreptype2[rho2rep, rho6rep, rho6alphainvrep, rho2primerep],
  "2x6+6x2'"},
{davisopsymliftreptype2[rho2primeinvrep, rho6rep, rho6alphainvrep, rho2rep],
  "2'x6+6x2"},
{davisopsymliftreptype2[rho3rep, rho4rep, rho4alphainvrep, rho3primerep],
  "3x4+4x3'"},
{davisopsymliftreptype2[rho3primeinvrep, rho4rep, rho4alphainvrep, rho3rep],
  "3'x4+4x3"},
{davisopsymliftreptype1[rho5rep, rho5alpharep, 1], "5x5"},
{davisopsymliftreptype1[rho5rep, rho5alpharep, -1], "-5x5"},
{davisopsymliftreptype2[
  rho3rep, rho5rep, rho5alphainvrep, rho3primerep], "3x5+5x3'"},
{davisopsymliftreptype2[rho3primeinvrep, rho5rep, rho5alphainvrep, rho3rep],
  "3'x5+5x3"},
{davisopsymliftreptype1[rho6rep, rho6alpharep, 1], "6x6"},
{davisopsymliftreptype1[rho6rep, rho6alpharep, -1], "-6x6"},
{davisopsymliftreptype2[
  rho4rep, rho5rep, rho5alphainvrep, rho4alpharep], "4x5+5x4"},
{davisopsymliftreptype2[rho4primerep, rho6rep, rho6alphainvrep,
  rho4primealpharep], "4'x6+6x4'"}];

```

*In[ ]:=* **davisopsymliftreprenames**

```

Out[ ]:= {1x2+2'x1, 1x2'+2x1, 1x4'+4'x1, 1x6+6x1, 2x3+3'x2', 2x3'+3x2', 2'x3+3'x2, 2'x3'+3x2,
  2x4+4x2', 2'x4+4x2, 2x5+5x2', 2'x5+5x2, 3x4'+4'x3', 3'x4'+4'x3, 4x4'+4'x4,
  3x6+6x3', 3'x6+6x3, 4'x5+5x4', 4x6+6x4, 5x6+6x5, 1x1, -1x1, 2x2', -2x2', 2'x2,
  -2'x2, 1x3+3'x1, 1x3'+3x1, 1x4+4x1, 2x2+2'x2', 3x3', -3x3', 3'x3, -3'x3, 1x5+5x1,
  2x4'+4'x2', 2'x4'+4'x2, 4x4, -4x4, 4'x4', -4'x4', 3x3+3'x3', 2x6+6x2', 2'x6+6x2,
  3x4+4x3', 3'x4+4x3, 5x5, -5x5, 3x5+5x3', 3'x5+5x3, 6x6, -6x6, 4x5+5x4, 4'x6+6x4'}

```

```

In[ ]:= Tally[
  Table[Tally[Table[Apply[Union, Chop[N[(davisopsymliftmultiply[#2, #3] /. #1), 40] - N[
    (#2 /. #1) . (#3 /. #1), 40], 10^-10]] &[
    davisopsymliftreps[[i]], davisopsymliftgrp[[RandomInteger[{1, 28800}]]]],
    davisopsymliftgrp[[RandomInteger[{1, 28800}]]]], {4}]], {i, 1, 54}]]

... N: Internal precision limit $MaxExtraPrecision = 50.` reached while evaluating {<<1>>}.
... N: Internal precision limit $MaxExtraPrecision = 50.` reached while evaluating {<<1>>}.
... N: Internal precision limit $MaxExtraPrecision = 50.` reached while evaluating
{ {AlgebraicNumber[Root[1 + 174 Power[<<2>>] + 11 Power[<<2>>] - 6 Power[<<2>>] + Slot[<<1>>]^8 &, 8, 0], { - $\frac{1}{4}$ , - $\frac{539}{101}$ , 0, - $\frac{745}{2424}$ , 0,  $\frac{145}{808}$ , 0, - $\frac{73}{2424}$  }], <<10>>, 0}, {AlgebraicNumber[Root[Plus[<<3>>] &, 2, 0], {  $\frac{1}{6}$ , 0, - $\frac{1}{6}$ , 0 }]} AlgebraicNumber
[Root[Plus[<<5>>] &, 8, 0], {  $\frac{1}{4}$ ,  $\frac{1647}{808}$ , 0,  $\frac{265}{2424}$ , 0, - $\frac{57}{808}$ , 0,  $\frac{7}{606}$  }]} + AlgebraicNumber[Root[Plus[<<3>>] &, 2, 0], {  $\frac{1}{6}$ , 0,
- $\frac{1}{6}$ , 0 }]} <<15>>[<<1>>, <<1>>], <<10>>, 0}, <<9>>, {0, <<11>>}]}.

... General: Further output of N::meprec will be suppressed during this calculation.

Out[ ]:= { { { { {0}, 4} }, 54} } }

```

*davisopsymliftconjclassnameslong*

```

In[ ]:= davisopsymliftconjclassnameslong = MapIndexed[Function[{c, i},
  If[# == {}, Function[cp, "[" <> Apply[StringJoin, Riffle[#[[All, 1]], "+" ]]] <> "]" &[
    Select[Transpose[{copsymliftconjclassnames, copsymliftconjclasses}],
      Length[Intersection[cp, #[[2]]]] > 0 &]] [Map[ReplacePart[#, {3 -> 0}] &, c]],
    Apply[StringJoin, Riffle[#[[All, 1]], "+" ]]] &[
      Select[Transpose[{copsymliftconjclassnames, copsymliftconjclasses}],
        Length[Intersection[c, #[[2]]]] > 0 &]], davisopsymliftconjclasses]

Out[ ]:= {1×1, 2×2, 1×3+3×1, 2×6+6×2, 3×3, 6×6, 2×4+4×2, 1×4+4×1, 1×5A+5B×1, 2×10B+10A×2,
  1×5B+5A×1, 2×10A+10B×2, 5B×5A, 10A×10B, 5A×5B, 10B×10A, 5A×5A+5B×5B, 10A×10A+10B×10B,
  2×3+3×2, 1×6+6×1, 2×5B+5A×2, 1×10A+10B×1, 2×5A+5B×2, 1×10B+10A×1, 5B×10A+10B×5A,
  5A×10B+10A×5B, 3×4+4×3, 4×6+6×4, 3×5A+5B×3, 6×10B+10A×6, 3×5B+5A×3, 6×10A+10B×6,
  4×5A+5B×4, 4×10B+10A×4, 4×10A+10B×4, 4×5B+5A×4, 5B×6+6×5A, 3×10B+10A×3, 3×10A+10B×3,
  5A×6+6×5B, 1×2+2×1, [1×2+2×1+3×6+4×4+5A×10A+5B×10B+6×3+10A×5A+10B×5B],
  [1×1+2×2+3×3+4×4+5A×5B+5B×5A+6×6+10A×10B+10B×10A], 4×4, 3×6+6×3,
  [1×6+2×3+3×2+3×3+3×4+3×5A+3×5B+3×6+4×3+4×4+4×5A+4×5B+4×6+4×10A+4×10B+5A×3+5A×4+5A×5B+
    5A×10B+5B×3+5B×4+5B×5A+5B×10A+6×1+6×3+6×4+6×6+6×10A+6×10B+10A×4+10A×5B+10A×6+10A×
    10B+10B×4+10B×5A+10B×6+10B×10A],
  [1×4+2×4+3×3+3×4+3×5A+3×5B+3×6+3×10A+3×10B+4×1+4×2+4×3+4×4+4×5A+4×5B+4×6+4×10A+4×10B+
    5A×3+5A×4+5A×5A+5A×6+5A×10B+5B×3+5B×4+5B×5B+5B×6+5B×10A+6×3+6×4+6×5A+6×5B+6×6+6×10
    A+6×10B+10A×3+10A×4+10A×5B+10A×6+10A×10A+10B×3+10B×4+10B×5A+10B×6+10B×10B],
  5B×10B+10A×5A, 5A×10A+10B×5B,
  [1×10A+2×5B+3×3+3×4+3×5B+3×10B+4×3+4×4+4×5A+4×6+4×10B+5A×2+5A×3+5A×5B+5A×10B+5B×4+5B×
    6+5B×10A+5B×10B+6×4+6×5A+6×6+6×10A+10A×3+10A×4+10A×5A+10A×5B+10B×1+10B×5A+10B×6+10B
    ×10A],
  [1×10B+2×5A+3×3+3×4+3×5A+3×10A+4×3+4×4+4×5B+4×6+4×10A+5A×4+5A×6+5A×10A+5A×10B+5B×2+5B
    ×3+5B×5A+5B×10A+6×4+6×5B+6×6+6×10B+10A×1+10A×5B+10A×6+10A×10B+10B×3+10B×4+10B×5A+
    10B×5B],
  [1×3+2×6+3×1+3×3+3×4+3×6+3×10A+3×10B+4×3+4×4+4×5A+4×5B+4×6+4×10A+4×10B+5A×4+5A×5A+5A×
    6+5A×10A+5B×4+5B×5B+5B×6+5B×10B+6×2+6×3+6×4+6×5A+6×5B+6×6+10A×3+10A×4+10A×5A+10A×
    10A+10B×3+10B×4+10B×5B+10B×10B],
  [1×5A+2×10B+3×4+3×5B+3×6+3×10B+4×3+4×4+4×5B+4×6+4×10A+5A×3+5A×4+5A×5A+5A×5B+5B×1+5B×5
    B+5B×6+5B×10B+6×3+6×4+6×5A+6×10A+10A×2+10A×3+10A×5A+10A×10A+10B×4+10B×6+10B×10A+10B
    ×10B],
  [1×5B+2×10A+3×4+3×5A+3×6+3×10A+4×3+4×4+4×5A+4×6+4×10B+5A×1+5A×5A+5A×6+5A×10A+5B×3+5B×
    4+5B×5A+5B×5B+6×3+6×4+6×5B+6×10B+10A×4+10A×6+10A×10A+10A×10B+10B×2+10B×3+10B×5B+10B
    ×10B] }

```

davisopsymliftconjclassnames

```
In[ ]:= davisopsymliftconjclassnames = MapIndexed[
  Function[{c, i}, If[# == {}, Function[cp, "[" <> #[[1, 1]] <> "]" & [Select[Transpose[
    {copsymliftconjclassnames[[Range[9]]], copsymliftconjclasses[[Range[9]]]]],
    Length[Intersection[cp, #[[2]]]] > 0 &]] [Map[ReplacePart[#, {3 -> 0}] &, c]],
    Apply[StringJoin, Riffle[#[[All, 1]], "+"]]] & [
    Select[Transpose[{copsymliftconjclassnames, copsymliftconjclasses}],
      Length[Intersection[c, #[[2]]]] > 0 &]], davisopsymliftconjclasses]
```

```
Out[ ]:= {1×1, 2×2, 1×3+3×1, 2×6+6×2, 3×3, 6×6, 2×4+4×2, 1×4+4×1, 1×5A+5B×1, 2×10B+10A×2,
  1×5B+5A×1, 2×10A+10B×2, 5B×5A, 10A×10B, 5A×5B, 10B×10A, 5A×5A+5B×5B, 10A×10A+10B×10B,
  2×3+3×2, 1×6+6×1, 2×5B+5A×2, 1×10A+10B×1, 2×5A+5B×2, 1×10B+10A×1, 5B×10A+10B×5A,
  5A×10B+10A×5B, 3×4+4×3, 4×6+6×4, 3×5A+5B×3, 6×10B+10A×6, 3×5B+5A×3, 6×10A+10B×6,
  4×5A+5B×4, 4×10B+10A×4, 4×10A+10B×4, 4×5B+5A×4, 5B×6+6×5A, 3×10B+10A×3,
  3×10A+10B×3, 5A×6+6×5B, 1×2+2×1, [1×2], [1×1], 4×4, 3×6+6×3, [1×6], [1×4],
  5B×10B+10A×5A, 5A×10A+10B×5B, [1×10A], [1×10B], [1×3], [1×5A], [1×5B]}
```

```
In[ ]:= TableForm[Outer[Length[Intersection[#1, #2]] &,
  copsymliftconjclasses, Map[ReplacePart[#, {3 -> 0}] &,
    davisopsymliftconjclasses[{{-13, -12, -9, -8, -5, -4, -3, -2, -1}}], {2}], 1],
  TableHeadings -> {copsymliftconjclassnames,
    davisopsymliftconjclassnames[{{-13, -12, -9, -8, -5, -4, -3, -2, -1}}]}
```

Out[ ]//TableForm=

|       | [1×2] | [1×1] | [1×6] | [1×4] | [1×10A] | [1×10B] | [1×3] | [1×5A] |   |
|-------|-------|-------|-------|-------|---------|---------|-------|--------|---|
| 1×1   | 0     | 1     | 0     | 0     | 0       | 0       | 0     | 0      | 0 |
| 1×2   | 1     | 0     | 0     | 0     | 0       | 0       | 0     | 0      | 0 |
| 1×3   | 0     | 0     | 0     | 0     | 0       | 0       | 20    | 0      | 0 |
| 1×4   | 0     | 0     | 0     | 30    | 0       | 0       | 0     | 0      | 0 |
| 1×5A  | 0     | 0     | 0     | 0     | 0       | 0       | 0     | 12     | 0 |
| 1×5B  | 0     | 0     | 0     | 0     | 0       | 0       | 0     | 0      | 1 |
| 1×6   | 0     | 0     | 20    | 0     | 0       | 0       | 0     | 0      | 0 |
| 1×10A | 0     | 0     | 0     | 0     | 12      | 0       | 0     | 0      | 0 |
| 1×10B | 0     | 0     | 0     | 0     | 0       | 12      | 0     | 0      | 0 |
| 2×1   | 1     | 0     | 0     | 0     | 0       | 0       | 0     | 0      | 0 |
| 2×2   | 0     | 1     | 0     | 0     | 0       | 0       | 0     | 0      | 0 |
| 2×3   | 0     | 0     | 20    | 0     | 0       | 0       | 0     | 0      | 0 |
| 2×4   | 0     | 0     | 0     | 30    | 0       | 0       | 0     | 0      | 0 |
| 2×5A  | 0     | 0     | 0     | 0     | 0       | 12      | 0     | 0      | 0 |
| 2×5B  | 0     | 0     | 0     | 0     | 12      | 0       | 0     | 0      | 0 |
| 2×6   | 0     | 0     | 0     | 0     | 0       | 0       | 20    | 0      | 0 |
| 2×10A | 0     | 0     | 0     | 0     | 0       | 0       | 0     | 0      | 1 |
| 2×10B | 0     | 0     | 0     | 0     | 0       | 0       | 0     | 12     | 0 |
| 3×1   | 0     | 0     | 0     | 0     | 0       | 0       | 20    | 0      | 0 |
| 3×2   | 0     | 0     | 20    | 0     | 0       | 0       | 0     | 0      | 0 |
| 3×3   | 0     | 20    | 120   | 120   | 60      | 60      | 20    | 0      | 0 |
| 3×4   | 0     | 0     | 120   | 120   | 60      | 60      | 120   | 60     | 0 |
| 3×5A  | 0     | 0     | 60    | 60    | 0       | 60      | 0     | 0      | 0 |
| 3×5B  | 0     | 0     | 60    | 60    | 60      | 0       | 0     | 60     | 0 |
| 3×6   | 20    | 0     | 20    | 120   | 0       | 0       | 120   | 60     | 0 |
| 3×10A | 0     | 0     | 0     | 60    | 0       | 60      | 60    | 0      | 0 |
| 3×10B | 0     | 0     | 0     | 60    | 60      | 0       | 60    | 60     | 0 |
| 4×1   | 0     | 0     | 0     | 30    | 0       | 0       | 0     | 0      | 0 |

|         |    |    |     |     |     |     |     |     |   |
|---------|----|----|-----|-----|-----|-----|-----|-----|---|
| 4×2     | 0  | 0  | 0   | 30  | 0   | 0   | 0   | 0   | 0 |
| 4×3     | 0  | 0  | 120 | 120 | 60  | 60  | 120 | 60  | 0 |
| 4×4     | 30 | 30 | 120 | 120 | 120 | 120 | 120 | 120 | 1 |
| 4×5A    | 0  | 0  | 60  | 120 | 60  | 0   | 60  | 0   | 0 |
| 4×5B    | 0  | 0  | 60  | 120 | 0   | 60  | 60  | 60  | 0 |
| 4×6     | 0  | 0  | 120 | 120 | 60  | 60  | 120 | 60  | 0 |
| 4×10A   | 0  | 0  | 60  | 120 | 0   | 60  | 60  | 60  | 0 |
| 4×10B   | 0  | 0  | 60  | 120 | 60  | 0   | 60  | 0   | 0 |
| 5A×1    | 0  | 0  | 0   | 0   | 0   | 0   | 0   | 0   | 1 |
| 5A×2    | 0  | 0  | 0   | 0   | 12  | 0   | 0   | 0   | 0 |
| 5A×3    | 0  | 0  | 60  | 60  | 60  | 0   | 0   | 60  | 0 |
| 5A×4    | 0  | 0  | 60  | 120 | 0   | 60  | 60  | 60  | 0 |
| 5A×5A   | 0  | 0  | 0   | 60  | 0   | 0   | 60  | 12  | 1 |
| 5A×5B   | 0  | 12 | 60  | 0   | 60  | 0   | 0   | 12  | 0 |
| 5A×6    | 0  | 0  | 0   | 60  | 0   | 60  | 60  | 0   | 0 |
| 5A×10A  | 12 | 0  | 0   | 0   | 0   | 12  | 60  | 0   | 0 |
| 5A×10B  | 0  | 0  | 60  | 60  | 12  | 12  | 0   | 0   | 0 |
| 5B×1    | 0  | 0  | 0   | 0   | 0   | 0   | 0   | 12  | 0 |
| 5B×2    | 0  | 0  | 0   | 0   | 0   | 12  | 0   | 0   | 0 |
| 5B×3    | 0  | 0  | 60  | 60  | 0   | 60  | 0   | 0   | 0 |
| 5B×4    | 0  | 0  | 60  | 120 | 60  | 0   | 60  | 0   | 0 |
| 5B×5A   | 0  | 12 | 60  | 0   | 0   | 60  | 0   | 0   | 1 |
| 5B×5B   | 0  | 0  | 0   | 60  | 0   | 0   | 60  | 12  | 1 |
| 5B×6    | 0  | 0  | 0   | 60  | 60  | 0   | 60  | 60  | 0 |
| 5B×10A  | 0  | 0  | 60  | 60  | 12  | 12  | 0   | 0   | 0 |
| 5B×10B  | 12 | 0  | 0   | 0   | 12  | 0   | 60  | 60  | 0 |
| 6×1     | 0  | 0  | 20  | 0   | 0   | 0   | 0   | 0   | 0 |
| 6×2     | 0  | 0  | 0   | 0   | 0   | 0   | 20  | 0   | 0 |
| 6×3     | 20 | 0  | 20  | 120 | 0   | 0   | 120 | 60  | 0 |
| 6×4     | 0  | 0  | 120 | 120 | 60  | 60  | 120 | 60  | 0 |
| 6×5A    | 0  | 0  | 0   | 60  | 60  | 0   | 60  | 60  | 0 |
| 6×5B    | 0  | 0  | 0   | 60  | 0   | 60  | 60  | 0   | 0 |
| 6×6     | 0  | 20 | 120 | 120 | 60  | 60  | 20  | 0   | 0 |
| 6×10A   | 0  | 0  | 60  | 60  | 60  | 0   | 0   | 60  | 0 |
| 6×10B   | 0  | 0  | 60  | 60  | 0   | 60  | 0   | 0   | 0 |
| 10A×1   | 0  | 0  | 0   | 0   | 0   | 12  | 0   | 0   | 0 |
| 10A×2   | 0  | 0  | 0   | 0   | 0   | 0   | 0   | 12  | 0 |
| 10A×3   | 0  | 0  | 0   | 60  | 60  | 0   | 60  | 60  | 0 |
| 10A×4   | 0  | 0  | 60  | 120 | 60  | 0   | 60  | 0   | 0 |
| 10A×5A  | 12 | 0  | 0   | 0   | 12  | 0   | 60  | 60  | 0 |
| 10A×5B  | 0  | 0  | 60  | 60  | 12  | 12  | 0   | 0   | 0 |
| 10A×6   | 0  | 0  | 60  | 60  | 0   | 60  | 0   | 0   | 0 |
| 10A×10A | 0  | 0  | 0   | 60  | 0   | 0   | 60  | 12  | 1 |
| 10A×10B | 0  | 12 | 60  | 0   | 0   | 60  | 0   | 0   | 1 |
| 10B×1   | 0  | 0  | 0   | 0   | 12  | 0   | 0   | 0   | 0 |
| 10B×2   | 0  | 0  | 0   | 0   | 0   | 0   | 0   | 0   | 1 |
| 10B×3   | 0  | 0  | 0   | 60  | 0   | 60  | 60  | 0   | 0 |
| 10B×4   | 0  | 0  | 60  | 120 | 0   | 60  | 60  | 60  | 0 |
| 10B×5A  | 0  | 0  | 60  | 60  | 12  | 12  | 0   | 0   | 0 |
| 10B×5B  | 12 | 0  | 0   | 0   | 0   | 12  | 60  | 0   | 0 |



|         |   |    |    |    |    |   |    |    |   |
|---------|---|----|----|----|----|---|----|----|---|
| 10B×6   | 0 | 0  | 60 | 60 | 60 | 0 | 0  | 60 | 0 |
| 10B×10A | 0 | 12 | 60 | 0  | 60 | 0 | 0  | 12 | 0 |
| 10B×10B | 0 | 0  | 0  | 60 | 0  | 0 | 60 | 12 | 1 |

```

In[ ]:= TableForm[
  Map[{davisopsymliftorder[#[[1]]], Length[#], {Map[formatkappa, pquats[#[[1, 1]]]],
    Map[formatkappa, pquats[#[[1, 2]]]], #[[1, 3]]}, Union[Map[davisopsymlift[
      pquatsminusperm[#[[1]]], pquatsminusperm[#[[2]]], #[[3]]] &, #]} /.
    Thread[davisopsymliftconjclasses → davisopsymliftconjclassnames]} &,
  davisopsymliftconjclasses], TableHeadings → {davisopsymliftconjclassnames,
    {"order", "size", "rep", "minus sym"}}, TableDepth → 2]

```

Out[ ]:=TableForm=

|                 | order | size | rep                                                                                                                                                                                            | minus sym  |
|-----------------|-------|------|------------------------------------------------------------------------------------------------------------------------------------------------------------------------------------------------|------------|
| 1×1             | 1     | 1    | {1, 1, 0}                                                                                                                                                                                      | 2×2        |
| 2×2             | 2     | 1    | {-1, -1, 0}                                                                                                                                                                                    | 1×1        |
| 1×3+3×1         | 3     | 40   | $\left\{-\frac{1}{2} + \mathbb{K}\left(\frac{1}{2} - \frac{\tau}{2}\right) - \frac{i\tau}{2}, 1, 0\right\}$                                                                                    | 2×6+6×2    |
| 2×6+6×2         | 6     | 40   | $\left\{-1, \frac{1}{2} + \mathbb{K}\left(\frac{1}{2} - \frac{\tau}{2}\right) - \frac{i\tau}{2}, 0\right\}$                                                                                    | 1×3+3×1    |
| 3×3             | 3     | 400  | $\left\{-\frac{1}{2} + \mathbb{K}\left(\frac{1}{2} - \frac{\tau}{2}\right) - \frac{i\tau}{2}, -\frac{1}{2} + \mathbb{K}\left(\frac{1}{2} - \frac{\tau}{2}\right) - \frac{i\tau}{2}, 0\right\}$ | 6×6        |
| 6×6             | 6     | 400  | $\left\{\frac{1}{2} + \mathbb{K}\left(\frac{1}{2} - \frac{\tau}{2}\right) - \frac{i\tau}{2}, \frac{1}{2} + \mathbb{K}\left(\frac{1}{2} - \frac{\tau}{2}\right) - \frac{i\tau}{2}, 0\right\}$   | 3×3        |
| 2×4+4×2         | 4     | 60   | {-1, -i, 0}                                                                                                                                                                                    | 1×4+4×1    |
| 1×4+4×1         | 4     | 60   | {-i, 1, 0}                                                                                                                                                                                     | 2×4+4×2    |
| 1×5A+5B×1       | 5     | 24   | $\left\{-\frac{i}{2} + \mathbb{J}\left(\frac{1}{2} - \frac{\tau}{2}\right) - \frac{\tau}{2}, 1, 0\right\}$                                                                                     | 2×10B+10A× |
| 2×10B+10A×2     | 10    | 24   | $\left\{-1, \frac{1}{2} - \frac{j}{2} - \frac{\tau}{2} - \frac{i\tau}{2}, 0\right\}$                                                                                                           | 1×5A+5B×1  |
| 1×5B+5A×1       | 5     | 24   | $\left\{-\frac{1}{2} - \frac{j}{2} + \frac{\tau}{2} - \frac{i\tau}{2}, 1, 0\right\}$                                                                                                           | 2×10A+10B× |
| 2×10A+10B×2     | 10    | 24   | $\left\{-1, -\frac{i}{2} + \mathbb{J}\left(\frac{1}{2} - \frac{\tau}{2}\right) + \frac{\tau}{2}, 0\right\}$                                                                                    | 1×5B+5A×1  |
| 5B×5A           | 5     | 144  | $\left\{-\frac{i}{2} + \mathbb{J}\left(\frac{1}{2} - \frac{\tau}{2}\right) - \frac{\tau}{2}, -\frac{1}{2} - \frac{j}{2} + \frac{\tau}{2} - \frac{i\tau}{2}, 0\right\}$                         | 10A×10B    |
| 10A×10B         | 10    | 144  | $\left\{-\frac{i}{2} + \mathbb{J}\left(\frac{1}{2} - \frac{\tau}{2}\right) + \frac{\tau}{2}, \frac{1}{2} - \frac{j}{2} - \frac{\tau}{2} - \frac{i\tau}{2}, 0\right\}$                          | 5B×5A      |
| 5A×5B           | 5     | 144  | $\left\{-\frac{1}{2} - \frac{j}{2} + \frac{\tau}{2} - \frac{i\tau}{2}, -\frac{i}{2} + \mathbb{J}\left(\frac{1}{2} - \frac{\tau}{2}\right) - \frac{\tau}{2}, 0\right\}$                         | 10B×10A    |
| 10B×10A         | 10    | 144  | $\left\{\frac{1}{2} - \frac{j}{2} - \frac{\tau}{2} - \frac{i\tau}{2}, -\frac{i}{2} + \mathbb{J}\left(\frac{1}{2} - \frac{\tau}{2}\right) + \frac{\tau}{2}, 0\right\}$                          | 5A×5B      |
| 5A×5A+5B×5B     | 5     | 288  | $\left\{-\frac{i}{2} + \mathbb{J}\left(\frac{1}{2} - \frac{\tau}{2}\right) - \frac{\tau}{2}, -\frac{i}{2} + \mathbb{J}\left(\frac{1}{2} - \frac{\tau}{2}\right) - \frac{\tau}{2}, 0\right\}$   | 10A×10A+10 |
| 10A×10A+10B×10B | 10    | 288  | $\left\{\frac{1}{2} - \frac{j}{2} - \frac{\tau}{2} - \frac{i\tau}{2}, \frac{1}{2} - \frac{j}{2} - \frac{\tau}{2} - \frac{i\tau}{2}, 0\right\}$                                                 | 5A×5A+5B×5 |
| 2×3+3×2         | 6     | 40   | $\left\{-1, -\frac{1}{2} + \mathbb{K}\left(\frac{1}{2} - \frac{\tau}{2}\right) - \frac{i\tau}{2}, 0\right\}$                                                                                   | 1×6+6×1    |
| 1×6+6×1         | 6     | 40   | $\left\{\frac{1}{2} + \mathbb{K}\left(\frac{1}{2} - \frac{\tau}{2}\right) - \frac{i\tau}{2}, 1, 0\right\}$                                                                                     | 2×3+3×2    |
| 2×5B+5A×2       | 10    | 24   | $\left\{-1, -\frac{i}{2} + \mathbb{J}\left(\frac{1}{2} - \frac{\tau}{2}\right) - \frac{\tau}{2}, 0\right\}$                                                                                    | 1×10A+10B× |
| 1×10A+10B×1     | 10    | 24   | $\left\{\frac{1}{2} - \frac{j}{2} - \frac{\tau}{2} - \frac{i\tau}{2}, 1, 0\right\}$                                                                                                            | 2×5B+5A×2  |
| 2×5A+5B×2       | 10    | 24   | $\left\{-1, -\frac{1}{2} - \frac{j}{2} + \frac{\tau}{2} - \frac{i\tau}{2}, 0\right\}$                                                                                                          | 1×10B+10A× |
| 1×10B+10A×1     | 10    | 24   | $\left\{-\frac{i}{2} + \mathbb{J}\left(\frac{1}{2} - \frac{\tau}{2}\right) + \frac{\tau}{2}, 1, 0\right\}$                                                                                     | 2×5A+5B×2  |
| 5B×10A+10B×5A   | 10    | 288  | $\left\{-\frac{i}{2} + \mathbb{J}\left(\frac{1}{2} - \frac{\tau}{2}\right) - \frac{\tau}{2}, -\frac{i}{2} + \mathbb{J}\left(\frac{1}{2} - \frac{\tau}{2}\right) + \frac{\tau}{2}, 0\right\}$   | 5A×10B+10A |
| 5A×10B+10A×5B   | 10    | 288  | $\left\{-\frac{1}{2} - \frac{j}{2} + \frac{\tau}{2} - \frac{i\tau}{2}, \frac{1}{2} - \frac{j}{2} - \frac{\tau}{2} - \frac{i\tau}{2}, 0\right\}$                                                | 5B×10A+10B |

|                                 |    |      |                                                                                                                                                                                                       |                             |
|---------------------------------|----|------|-------------------------------------------------------------------------------------------------------------------------------------------------------------------------------------------------------|-----------------------------|
| $3 \times 4 + 4 \times 3$       | 12 | 1200 | $\left\{ -\frac{1}{2} + \mathbb{K} \left( \frac{1}{2} - \frac{\tau}{2} \right) - \frac{i\tau}{2}, -i, 0 \right\}$                                                                                     | $4 \times 6 + 6 \times 4$   |
| $4 \times 6 + 6 \times 4$       | 12 | 1200 | $\left\{ -i, \frac{1}{2} + \mathbb{K} \left( \frac{1}{2} - \frac{\tau}{2} \right) - \frac{i\tau}{2}, 0 \right\}$                                                                                      | $3 \times 4 + 4 \times 3$   |
| $3 \times 5A + 5B \times 3$     | 15 | 480  | $\left\{ -\frac{i}{2} + \mathbb{J} \left( \frac{1}{2} - \frac{\tau}{2} \right) - \frac{\tau}{2}, -\frac{1}{2} + \mathbb{K} \left( \frac{1}{2} - \frac{\tau}{2} \right) - \frac{i\tau}{2}, 0 \right\}$ | $6 \times 10B + 10A \times$ |
| $6 \times 10B + 10A \times 6$   | 30 | 480  | $\left\{ \frac{1}{2} + \mathbb{K} \left( \frac{1}{2} - \frac{\tau}{2} \right) - \frac{i\tau}{2}, \frac{1}{2} - \frac{j}{2} - \frac{\tau}{2} - \frac{i\tau}{2}, 0 \right\}$                            | $3 \times 5A + 5B \times 3$ |
| $3 \times 5B + 5A \times 3$     | 15 | 480  | $\left\{ -\frac{1}{2} + \mathbb{K} \left( \frac{1}{2} - \frac{\tau}{2} \right) - \frac{i\tau}{2}, -\frac{i}{2} + \mathbb{J} \left( \frac{1}{2} - \frac{\tau}{2} \right) - \frac{\tau}{2}, 0 \right\}$ | $6 \times 10A + 10B \times$ |
| $6 \times 10A + 10B \times 6$   | 30 | 480  | $\left\{ \frac{1}{2} - \frac{j}{2} - \frac{\tau}{2} - \frac{i\tau}{2}, \frac{1}{2} + \mathbb{K} \left( \frac{1}{2} - \frac{\tau}{2} \right) - \frac{i\tau}{2}, 0 \right\}$                            | $3 \times 5B + 5A \times 3$ |
| $4 \times 5A + 5B \times 4$     | 20 | 720  | $\left\{ -\frac{i}{2} + \mathbb{J} \left( \frac{1}{2} - \frac{\tau}{2} \right) - \frac{\tau}{2}, -i, 0 \right\}$                                                                                      | $4 \times 10B + 10A \times$ |
| $4 \times 10B + 10A \times 4$   | 20 | 720  | $\left\{ -i, \frac{1}{2} - \frac{j}{2} - \frac{\tau}{2} - \frac{i\tau}{2}, 0 \right\}$                                                                                                                | $4 \times 5A + 5B \times 4$ |
| $4 \times 10A + 10B \times 4$   | 20 | 720  | $\left\{ \frac{1}{2} - \frac{j}{2} - \frac{\tau}{2} - \frac{i\tau}{2}, -i, 0 \right\}$                                                                                                                | $4 \times 5B + 5A \times 4$ |
| $4 \times 5B + 5A \times 4$     | 20 | 720  | $\left\{ -i, -\frac{i}{2} + \mathbb{J} \left( \frac{1}{2} - \frac{\tau}{2} \right) - \frac{\tau}{2}, 0 \right\}$                                                                                      | $4 \times 10A + 10B \times$ |
| $5B \times 6 + 6 \times 5A$     | 30 | 480  | $\left\{ -\frac{i}{2} + \mathbb{J} \left( \frac{1}{2} - \frac{\tau}{2} \right) - \frac{\tau}{2}, \frac{1}{2} + \mathbb{K} \left( \frac{1}{2} - \frac{\tau}{2} \right) - \frac{i\tau}{2}, 0 \right\}$  | $3 \times 10B + 10A \times$ |
| $3 \times 10B + 10A \times 3$   | 30 | 480  | $\left\{ -\frac{1}{2} + \mathbb{K} \left( \frac{1}{2} - \frac{\tau}{2} \right) - \frac{i\tau}{2}, \frac{1}{2} - \frac{j}{2} - \frac{\tau}{2} - \frac{i\tau}{2}, 0 \right\}$                           | $5B \times 6 + 6 \times 5A$ |
| $3 \times 10A + 10B \times 3$   | 30 | 480  | $\left\{ -\frac{1}{2} + \mathbb{K} \left( \frac{1}{2} - \frac{\tau}{2} \right) - \frac{i\tau}{2}, -\frac{i}{2} + \mathbb{J} \left( \frac{1}{2} - \frac{\tau}{2} \right) + \frac{\tau}{2}, 0 \right\}$ | $5A \times 6 + 6 \times 5B$ |
| $5A \times 6 + 6 \times 5B$     | 30 | 480  | $\left\{ -\frac{1}{2} - \frac{j}{2} + \frac{\tau}{2} - \frac{i\tau}{2}, \frac{1}{2} + \mathbb{K} \left( \frac{1}{2} - \frac{\tau}{2} \right) - \frac{i\tau}{2}, 0 \right\}$                           | $3 \times 10A + 10B \times$ |
| $1 \times 2 + 2 \times 1$       | 2  | 2    | $\{-1, 1, 0\}$                                                                                                                                                                                        | $1 \times 2 + 2 \times 1$   |
| $[1 \times 2]$                  | 2  | 120  | $\{-1, 1, 1\}$                                                                                                                                                                                        | $[1 \times 2]$              |
| $[1 \times 1]$                  | 4  | 120  | $\{-1, -1, 1\}$                                                                                                                                                                                       | $[1 \times 1]$              |
| $4 \times 4$                    | 4  | 900  | $\{-i, -i, 0\}$                                                                                                                                                                                       | $4 \times 4$                |
| $3 \times 6 + 6 \times 3$       | 6  | 800  | $\left\{ -\frac{1}{2} + \mathbb{K} \left( \frac{1}{2} - \frac{\tau}{2} \right) - \frac{i\tau}{2}, \frac{1}{2} + \mathbb{K} \left( \frac{1}{2} - \frac{\tau}{2} \right) - \frac{i\tau}{2}, 0 \right\}$ | $3 \times 6 + 6 \times 3$   |
| $[1 \times 6]$                  | 6  | 2400 | $\left\{ -1, -\frac{1}{2} + \mathbb{K} \left( \frac{1}{2} - \frac{\tau}{2} \right) - \frac{i\tau}{2}, 1 \right\}$                                                                                     | $[1 \times 6]$              |
| $[1 \times 4]$                  | 8  | 3600 | $\{-1, -i, 1\}$                                                                                                                                                                                       | $[1 \times 4]$              |
| $5B \times 10B + 10A \times 5A$ | 10 | 288  | $\left\{ -\frac{i}{2} + \mathbb{J} \left( \frac{1}{2} - \frac{\tau}{2} \right) - \frac{\tau}{2}, \frac{1}{2} - \frac{j}{2} - \frac{\tau}{2} - \frac{i\tau}{2}, 0 \right\}$                            | $5B \times 10B + 10A$       |
| $5A \times 10A + 10B \times 5B$ | 10 | 288  | $\left\{ \frac{1}{2} - \frac{j}{2} - \frac{\tau}{2} - \frac{i\tau}{2}, -\frac{i}{2} + \mathbb{J} \left( \frac{1}{2} - \frac{\tau}{2} \right) - \frac{\tau}{2}, 0 \right\}$                            | $5A \times 10A + 10B$       |
| $[1 \times 10A]$                | 10 | 1440 | $\left\{ -1, -\frac{i}{2} + \mathbb{J} \left( \frac{1}{2} - \frac{\tau}{2} \right) - \frac{\tau}{2}, 1 \right\}$                                                                                      | $[1 \times 10A]$            |
| $[1 \times 10B]$                | 10 | 1440 | $\left\{ -1, -\frac{1}{2} - \frac{j}{2} + \frac{\tau}{2} - \frac{i\tau}{2}, 1 \right\}$                                                                                                               | $[1 \times 10B]$            |
| $[1 \times 3]$                  | 12 | 2400 | $\left\{ -1, \frac{1}{2} + \mathbb{K} \left( \frac{1}{2} - \frac{\tau}{2} \right) - \frac{i\tau}{2}, 1 \right\}$                                                                                      | $[1 \times 3]$              |
| $[1 \times 5A]$                 | 20 | 1440 | $\left\{ -1, \frac{1}{2} - \frac{j}{2} - \frac{\tau}{2} - \frac{i\tau}{2}, 1 \right\}$                                                                                                                | $[1 \times 5A]$             |
| $[1 \times 5B]$                 | 20 | 1440 | $\left\{ -1, -\frac{i}{2} + \mathbb{J} \left( \frac{1}{2} - \frac{\tau}{2} \right) + \frac{\tau}{2}, 1 \right\}$                                                                                      | $[1 \times 5B]$             |

davisopsymliftcharacterTable

```

In[ ]:= TableForm[formatkappa[davisopsymliftcharacterTable = toQkappa[RootReduce[
  Map[Map[Tr, davisopsymliftconjclasses[[All, 1]] /. #] &, davisopsymlifttreps]]],
  TableHeadings -> {davisopsymlifttrepsnames, MapThread[
    Column[{Length[#1], davisopsymliftorder[#1[[1]]], #2], ItemSize -> {9, 1}] &,
    {davisopsymliftconjclasses, davisopsymliftconjclassnames}]]]

```

Out[ ]:=TableForm=

|     |     |         |         |
|-----|-----|---------|---------|
| 1   | 1   | 40      | 40      |
| 1   | 2   | 3       | 6       |
| 1×1 | 2×2 | 1×3+3×1 | 2×6+6×2 |

|                              |    |     |    |    |
|------------------------------|----|-----|----|----|
| $1 \times 2 + 2' \times 1$   | 4  | -4  | 1  | -1 |
| $1 \times 2' + 2 \times 1$   | 4  | -4  | 1  | -1 |
| $1 \times 4' + 4' \times 1$  | 8  | -8  | 5  | -5 |
| $1 \times 6 + 6 \times 1$    | 12 | -12 | 6  | -6 |
| $2 \times 3 + 3' \times 2'$  | 12 | -12 | -3 | 3  |
| $2 \times 3' + 3 \times 2'$  | 12 | -12 | -3 | 3  |
| $2' \times 3 + 3' \times 2$  | 12 | -12 | -3 | 3  |
| $2' \times 3' + 3 \times 2$  | 12 | -12 | -3 | 3  |
| $2 \times 4 + 4 \times 2'$   | 16 | -16 | -2 | 2  |
| $2' \times 4 + 4 \times 2$   | 16 | -16 | -2 | 2  |
| $2 \times 5 + 5 \times 2'$   | 20 | -20 | -7 | 7  |
| $2' \times 5 + 5 \times 2$   | 20 | -20 | -7 | 7  |
| $3 \times 4' + 4' \times 3'$ | 24 | -24 | 3  | -3 |
| $3' \times 4' + 4' \times 3$ | 24 | -24 | 3  | -3 |
| $4 \times 4' + 4' \times 4$  | 32 | -32 | 8  | -8 |
| $3 \times 6 + 6 \times 3'$   | 36 | -36 | 0  | 0  |
| $3' \times 6 + 6 \times 3$   | 36 | -36 | 0  | 0  |
| $4' \times 5 + 5 \times 4'$  | 40 | -40 | 1  | -1 |
| $4 \times 6 + 6 \times 4$    | 48 | -48 | 6  | -6 |
| $5 \times 6 + 6 \times 5$    | 60 | -60 | -6 | 6  |
| $1 \times 1$                 | 1  | 1   | 1  | 1  |
| $-1 \times 1$                | 1  | 1   | 1  | 1  |
| $2 \times 2'$                | 4  | 4   | -2 | -2 |
| $-2 \times 2'$               | 4  | 4   | -2 | -2 |
| $2' \times 2$                | 4  | 4   | -2 | -2 |
| $-2' \times 2$               | 4  | 4   | -2 | -2 |
| $1 \times 3 + 3' \times 1$   | 6  | 6   | 3  | 3  |
| $1 \times 3' + 3 \times 1$   | 6  | 6   | 3  | 3  |
| $1 \times 4 + 4 \times 1$    | 8  | 8   | 5  | 5  |
| $2 \times 2 + 2' \times 2'$  | 8  | 8   | -4 | -4 |
| $3 \times 3'$                | 9  | 9   | 0  | 0  |
| $-3 \times 3'$               | 9  | 9   | 0  | 0  |
| $3' \times 3$                | 9  | 9   | 0  | 0  |
| $-3' \times 3$               | 9  | 9   | 0  | 0  |
| $1 \times 5 + 5 \times 1$    | 10 | 10  | 4  | 4  |
| $2 \times 4' + 4' \times 2'$ | 16 | 16  | -2 | -2 |
| $2' \times 4' + 4' \times 2$ | 16 | 16  | -2 | -2 |
| $4 \times 4$                 | 16 | 16  | 4  | 4  |
| $-4 \times 4$                | 16 | 16  | 4  | 4  |
| $4' \times 4'$               | 16 | 16  | 4  | 4  |
| $-4' \times 4'$              | 16 | 16  | 4  | 4  |
| $3 \times 3 + 3' \times 3'$  | 18 | 18  | 0  | 0  |
| $2 \times 6 + 6 \times 2'$   | 24 | 24  | -6 | -6 |
| $2' \times 6 + 6 \times 2$   | 24 | 24  | -6 | -6 |
| $3 \times 4 + 4 \times 3'$   | 24 | 24  | 3  | 3  |
| $3' \times 4 + 4 \times 3$   | 24 | 24  | 3  | 3  |
| $5 \times 5$                 | 25 | 25  | -5 | -5 |
| $-5 \times 5$                | 25 | 25  | -5 | -5 |
| $3 \times 5 + 5 \times 3'$   | 30 | 30  | -3 | -3 |
| $3' \times 5 + 5 \times 3$   | 30 | 30  | -3 | -3 |

|                             |    |    |   |   |
|-----------------------------|----|----|---|---|
| $6 \times 6$                | 36 | 36 | 0 | 0 |
| $-6 \times 6$               | 36 | 36 | 0 | 0 |
| $4 \times 5 + 5 \times 4$   | 40 | 40 | 1 | 1 |
| $4' \times 6 + 6 \times 4'$ | 48 | 48 | 6 | 6 |

```
In[ ]:= CharacterTableInnerProducts[
  davisopsymLiftCharacterTable, Map[Length, davisopsymLiftConjClasses]] ==
  IdentityMatrix[Length[davisopsymLiftConjClasses]] // FullSimplify
```

```
Out[ ]:= True
```

davisopsymrepnames

```
In[ ]:= davisopsymrepnames = Drop[davisopsymLiftRepnames, 20];
```

davisopsymreps

```
In[ ]:= davisopsymreps =
  Map[Function[rep, {davisopsymLift[i1p_, i2p_, jp_], davisopsymLift[_, _, _]} >=
    (davisopsymLift[i1p, i2p, jp] /. rep)], Drop[davisopsymLiftReps, 20]];
```

davisopsymconjclassnames

```
In[ ]:= davisopsymconjclassnames =
  MapIndexed[Function[{c, i}, Apply[StringJoin, Riffle[#[[All, 1]], "+"]] &[
    Select[Transpose[{davisopsymLiftConjClassNames, davisopsymLiftConjClasses}],
      Length[Intersection[c, #[[2]]]] > 0 &]],
    Map[Apply[Union, #] &, davisopsymConjClasses]]
```

```
Out[ ]:= {1x1+2x2, 1x3+3x1+2x6+6x2, 3x3+6x6, 2x4+4x2+1x4+4x1, 1x5A+5Bx1+2x10B+10Ax2,
  1x5B+5Ax1+2x10A+10Bx2, 5Bx5A+10Ax10B, 5Ax5B+10Bx10A, 5Ax5A+5Bx5B+10Ax10A+10Bx10B,
  2x3+3x2+1x6+6x1, 2x5B+5Ax2+1x10A+10Bx1, 2x5A+5Bx2+1x10B+10Ax1,
  5Bx10A+10Bx5A+5Ax10B+10Ax5B, 3x4+4x3+4x6+6x4, 3x5A+5Bx3+6x10B+10Ax6,
  3x5B+5Ax3+6x10A+10Bx6, 4x5A+5Bx4+4x10B+10Ax4, 4x10A+10Bx4+4x5B+5Ax4,
  5Bx6+6x5A+3x10B+10Ax3, 3x10A+10Bx3+5Ax6+6x5B, 1x2+2x1, [1x2], [1x1], 4x4, 3x6+6x3,
  [1x6], [1x4], 5Bx10B+10Ax5A, 5Ax10A+10Bx5B, [1x10A], [1x10B], [1x3], [1x5A], [1x5B]}
```

```
In[ ]:= TableForm[
  Map[{davisopsymOrder[#[[1]]], Length[#], {Map[formatKappa, pquats[#[[1, 1, 1]]]],
    Map[formatKappa, pquats[#[[1, 1, 2]]]], #[[1, 1, 3]]}} &, davisopsymConjClasses],
  TableHeadings -> {davisopsymConjClassNames, {"order", "size", "rep"}}, TableDepth -> 2]
```

Out[ ]:=TableForm=

|                                                                 | order | size | rep                                                                                                                                                                                            |
|-----------------------------------------------------------------|-------|------|------------------------------------------------------------------------------------------------------------------------------------------------------------------------------------------------|
| $1 \times 1 + 2 \times 2$                                       | 1     | 1    | $\{1, 1, 0\}$                                                                                                                                                                                  |
| $1 \times 3 + 3 \times 1 + 2 \times 6 + 6 \times 2$             | 3     | 40   | $\left\{-\frac{1}{2} + \mathbb{K}\left(\frac{1}{2} - \frac{\tau}{2}\right) - \frac{i\tau}{2}, 1, 0\right\}$                                                                                    |
| $3 \times 3 + 6 \times 6$                                       | 3     | 400  | $\left\{-\frac{1}{2} + \mathbb{K}\left(\frac{1}{2} - \frac{\tau}{2}\right) - \frac{i\tau}{2}, -\frac{1}{2} + \mathbb{K}\left(\frac{1}{2} - \frac{\tau}{2}\right) - \frac{i\tau}{2}, 0\right\}$ |
| $2 \times 4 + 4 \times 2 + 1 \times 4 + 4 \times 1$             | 4     | 60   | $\{-1, -i, 0\}$                                                                                                                                                                                |
| $1 \times 5A + 5B \times 1 + 2 \times 10B + 10A \times 2$       | 5     | 24   | $\left\{-\frac{i}{2} + \mathbb{J}\left(\frac{1}{2} - \frac{\tau}{2}\right) - \frac{\tau}{2}, 1, 0\right\}$                                                                                     |
| $1 \times 5B + 5A \times 1 + 2 \times 10A + 10B \times 2$       | 5     | 24   | $\left\{-\frac{1}{2} - \frac{j}{2} + \frac{\tau}{2} - \frac{i\tau}{2}, 1, 0\right\}$                                                                                                           |
| $5B \times 5A + 10A \times 10B$                                 | 5     | 144  | $\left\{-\frac{i}{2} + \mathbb{J}\left(\frac{1}{2} - \frac{\tau}{2}\right) - \frac{\tau}{2}, -\frac{1}{2} - \frac{j}{2} + \frac{\tau}{2} - \frac{i\tau}{2}, 0\right\}$                         |
| $5A \times 5B + 10B \times 10A$                                 | 5     | 144  | $\left\{-\frac{1}{2} - \frac{j}{2} + \frac{\tau}{2} - \frac{i\tau}{2}, -\frac{i}{2} + \mathbb{J}\left(\frac{1}{2} - \frac{\tau}{2}\right) - \frac{\tau}{2}, 0\right\}$                         |
| $5A \times 5A + 5B \times 5B + 10A \times 10A + 10B \times 10B$ | 5     | 288  | $\left\{-\frac{i}{2} + \mathbb{J}\left(\frac{1}{2} - \frac{\tau}{2}\right) - \frac{\tau}{2}, -\frac{i}{2} + \mathbb{J}\left(\frac{1}{2} - \frac{\tau}{2}\right) - \frac{\tau}{2}, 0\right\}$   |
| $2 \times 3 + 3 \times 2 + 1 \times 6 + 6 \times 1$             | 6     | 40   | $\left\{-1, -\frac{1}{2} + \mathbb{K}\left(\frac{1}{2} - \frac{\tau}{2}\right) - \frac{i\tau}{2}, 0\right\}$                                                                                   |

|                                                                 |    |      |                                                                                                                                                                             |
|-----------------------------------------------------------------|----|------|-----------------------------------------------------------------------------------------------------------------------------------------------------------------------------|
| $2 \times 5B + 5A \times 2 + 1 \times 10A + 10B \times 1$       | 10 | 24   | $\left\{-1, -\frac{i}{2} + j\left(\frac{1}{2} - \frac{\tau}{2}\right) - \frac{\tau}{2}, 0\right\}$                                                                          |
| $2 \times 5A + 5B \times 2 + 1 \times 10B + 10A \times 1$       | 10 | 24   | $\left\{-1, -\frac{1}{2} - \frac{j}{2} + \frac{\tau}{2} - \frac{i\tau}{2}, 0\right\}$                                                                                       |
| $5B \times 10A + 10B \times 5A + 5A \times 10B + 10A \times 5B$ | 10 | 288  | $\left\{-\frac{i}{2} + j\left(\frac{1}{2} - \frac{\tau}{2}\right) - \frac{\tau}{2}, -\frac{i}{2} + j\left(\frac{1}{2} - \frac{\tau}{2}\right) + \frac{\tau}{2}, 0\right\}$  |
| $3 \times 4 + 4 \times 3 + 4 \times 6 + 6 \times 4$             | 12 | 1200 | $\left\{-\frac{1}{2} + k\left(\frac{1}{2} - \frac{\tau}{2}\right) - \frac{i\tau}{2}, -i, 0\right\}$                                                                         |
| $3 \times 5A + 5B \times 3 + 6 \times 10B + 10A \times 6$       | 15 | 480  | $\left\{-\frac{i}{2} + j\left(\frac{1}{2} - \frac{\tau}{2}\right) - \frac{\tau}{2}, -\frac{1}{2} + k\left(\frac{1}{2} - \frac{\tau}{2}\right) - \frac{i\tau}{2}, 0\right\}$ |
| $3 \times 5B + 5A \times 3 + 6 \times 10A + 10B \times 6$       | 15 | 480  | $\left\{-\frac{1}{2} + k\left(\frac{1}{2} - \frac{\tau}{2}\right) - \frac{i\tau}{2}, -\frac{i}{2} + j\left(\frac{1}{2} - \frac{\tau}{2}\right) - \frac{\tau}{2}, 0\right\}$ |
| $4 \times 5A + 5B \times 4 + 4 \times 10B + 10A \times 4$       | 20 | 720  | $\left\{-\frac{i}{2} + j\left(\frac{1}{2} - \frac{\tau}{2}\right) - \frac{\tau}{2}, -i, 0\right\}$                                                                          |
| $4 \times 10A + 10B \times 4 + 4 \times 5B + 5A \times 4$       | 20 | 720  | $\left\{\frac{1}{2} - \frac{j}{2} - \frac{\tau}{2} - \frac{i\tau}{2}, -i, 0\right\}$                                                                                        |
| $5B \times 6 + 6 \times 5A + 3 \times 10B + 10A \times 3$       | 30 | 480  | $\left\{-\frac{i}{2} + j\left(\frac{1}{2} - \frac{\tau}{2}\right) - \frac{\tau}{2}, \frac{1}{2} + k\left(\frac{1}{2} - \frac{\tau}{2}\right) - \frac{i\tau}{2}, 0\right\}$  |
| $3 \times 10A + 10B \times 3 + 5A \times 6 + 6 \times 5B$       | 30 | 480  | $\left\{-\frac{1}{2} + k\left(\frac{1}{2} - \frac{\tau}{2}\right) - \frac{i\tau}{2}, -\frac{i}{2} + j\left(\frac{1}{2} - \frac{\tau}{2}\right) + \frac{\tau}{2}, 0\right\}$ |
| $1 \times 2 + 2 \times 1$                                       | 2  | 1    | $\{-1, 1, 0\}$                                                                                                                                                              |
| $[1 \times 2]$                                                  | 2  | 60   | $\{-1, 1, 1\}$                                                                                                                                                              |
| $[1 \times 1]$                                                  | 2  | 60   | $\{-1, -1, 1\}$                                                                                                                                                             |
| $4 \times 4$                                                    | 2  | 450  | $\{-i, -i, 0\}$                                                                                                                                                             |
| $3 \times 6 + 6 \times 3$                                       | 6  | 400  | $\left\{-\frac{1}{2} + k\left(\frac{1}{2} - \frac{\tau}{2}\right) - \frac{i\tau}{2}, \frac{1}{2} + k\left(\frac{1}{2} - \frac{\tau}{2}\right) - \frac{i\tau}{2}, 0\right\}$ |
| $[1 \times 6]$                                                  | 6  | 1200 | $\left\{-1, -\frac{1}{2} + k\left(\frac{1}{2} - \frac{\tau}{2}\right) - \frac{i\tau}{2}, 1\right\}$                                                                         |
| $[1 \times 4]$                                                  | 4  | 1800 | $\{-1, -i, 1\}$                                                                                                                                                             |
| $5B \times 10B + 10A \times 5A$                                 | 10 | 144  | $\left\{-\frac{i}{2} + j\left(\frac{1}{2} - \frac{\tau}{2}\right) - \frac{\tau}{2}, \frac{1}{2} - \frac{j}{2} - \frac{\tau}{2} - \frac{i\tau}{2}, 0\right\}$                |
| $5A \times 10A + 10B \times 5B$                                 | 10 | 144  | $\left\{\frac{1}{2} - \frac{j}{2} - \frac{\tau}{2} - \frac{i\tau}{2}, -\frac{i}{2} + j\left(\frac{1}{2} - \frac{\tau}{2}\right) - \frac{\tau}{2}, 0\right\}$                |
| $[1 \times 10A]$                                                | 10 | 720  | $\left\{-1, -\frac{i}{2} + j\left(\frac{1}{2} - \frac{\tau}{2}\right) - \frac{\tau}{2}, 1\right\}$                                                                          |
| $[1 \times 10B]$                                                | 10 | 720  | $\left\{-1, -\frac{1}{2} - \frac{j}{2} + \frac{\tau}{2} - \frac{i\tau}{2}, 1\right\}$                                                                                       |
| $[1 \times 3]$                                                  | 6  | 1200 | $\left\{-1, \frac{1}{2} + k\left(\frac{1}{2} - \frac{\tau}{2}\right) - \frac{i\tau}{2}, 1\right\}$                                                                          |
| $[1 \times 5A]$                                                 | 10 | 720  | $\left\{-1, \frac{1}{2} - \frac{j}{2} - \frac{\tau}{2} - \frac{i\tau}{2}, 1\right\}$                                                                                        |
| $[1 \times 5B]$                                                 | 10 | 720  | $\left\{-1, -\frac{i}{2} + j\left(\frac{1}{2} - \frac{\tau}{2}\right) + \frac{\tau}{2}, 1\right\}$                                                                          |

davisopsymcharacterstable

```

In[ ]:= TableForm[formatkappa[davisopsymcharacterstable = toQkappa[
  RootReduce[Map[Map[Tr, davisopsymconjclasses[All, 1]] /. #] &, davisopsymreps]]],
  TableHeadings -> {davisopsymrepnames, MapThread[Column[{Length[#1],
    davisopsymorder[#1[[1]], #2], ItemSize -> {Floor[StringLength[#2] * 0.5 + 3], 1}] &,
    {davisopsymconjclasses, davisopsymconjclassnames}]]]

```

Out[ ]:=TableForm=

|                              | 1                         | 40                                                  | 400                       | 60                                                  | 24           |
|------------------------------|---------------------------|-----------------------------------------------------|---------------------------|-----------------------------------------------------|--------------|
|                              | 1                         | 3                                                   | 3                         | 4                                                   | 5            |
|                              | $1 \times 1 + 2 \times 2$ | $1 \times 3 + 3 \times 1 + 2 \times 6 + 6 \times 2$ | $3 \times 3 + 6 \times 6$ | $2 \times 4 + 4 \times 2 + 1 \times 4 + 4 \times 1$ | $1 \times 5$ |
| $1 \times 1$                 | 1                         | 1                                                   | 1                         | 1                                                   | 1            |
| $-1 \times 1$                | 1                         | 1                                                   | 1                         | 1                                                   | 1            |
| $2 \times 2'$                | 4                         | -2                                                  | 1                         | 0                                                   | -2           |
| $-2 \times 2'$               | 4                         | -2                                                  | 1                         | 0                                                   | -2           |
| $2' \times 2$                | 4                         | -2                                                  | 1                         | 0                                                   | -2           |
| $-2' \times 2$               | 4                         | -2                                                  | 1                         | 0                                                   | -2           |
| $1 \times 3 + 3' \times 1$   | 6                         | 3                                                   | 0                         | 2                                                   | 4            |
| $1 \times 3' + 3 \times 1$   | 6                         | 3                                                   | 0                         | 2                                                   | 3            |
| $1 \times 4 + 4 \times 1$    | 8                         | 5                                                   | 2                         | 4                                                   | 3            |
| $2 \times 2 + 2' \times 2'$  | 8                         | -4                                                  | 2                         | 0                                                   | -2           |
| $3 \times 3'$                | 9                         | 0                                                   | 0                         | -3                                                  | 3            |
| $-3 \times 3'$               | 9                         | 0                                                   | 0                         | -3                                                  | 3            |
| $3' \times 3$                | 9                         | 0                                                   | 0                         | -3                                                  | 3            |
| $-3' \times 3$               | 9                         | 0                                                   | 0                         | -3                                                  | 3            |
| $1 \times 5 + 5 \times 1$    | 10                        | 4                                                   | -2                        | 6                                                   | 5            |
| $2 \times 4' + 4' \times 2'$ | 16                        | -2                                                  | -2                        | 0                                                   | -2           |
| $2' \times 4' + 4' \times 2$ | 16                        | -2                                                  | -2                        | 0                                                   | -6           |
| $4 \times 4$                 | 16                        | 4                                                   | 1                         | 0                                                   | -4           |
| $-4 \times 4$                | 16                        | 4                                                   | 1                         | 0                                                   | -4           |
| $4' \times 4'$               | 16                        | 4                                                   | 1                         | 0                                                   | -4           |
| $-4' \times 4'$              | 16                        | 4                                                   | 1                         | 0                                                   | -4           |
| $3 \times 3 + 3' \times 3'$  | 18                        | 0                                                   | 0                         | -6                                                  | 3            |
| $2 \times 6 + 6 \times 2'$   | 24                        | -6                                                  | 0                         | 0                                                   | 2            |
| $2' \times 6 + 6 \times 2$   | 24                        | -6                                                  | 0                         | 0                                                   | -4           |
| $3 \times 4 + 4 \times 3'$   | 24                        | 3                                                   | 0                         | -4                                                  | -3           |
| $3' \times 4 + 4 \times 3$   | 24                        | 3                                                   | 0                         | -4                                                  | 1            |
| $5 \times 5$                 | 25                        | -5                                                  | 1                         | 5                                                   | 0            |
| $-5 \times 5$                | 25                        | -5                                                  | 1                         | 5                                                   | 0            |
| $3 \times 5 + 5 \times 3'$   | 30                        | -3                                                  | 0                         | -2                                                  | 5            |
| $3' \times 5 + 5 \times 3$   | 30                        | -3                                                  | 0                         | -2                                                  | 5            |
| $6 \times 6$                 | 36                        | 0                                                   | 0                         | 0                                                   | 6            |
| $-6 \times 6$                | 36                        | 0                                                   | 0                         | 0                                                   | 6            |
| $4 \times 5 + 5 \times 4$    | 40                        | 1                                                   | -2                        | 4                                                   | -5           |
| $4' \times 6 + 6 \times 4'$  | 48                        | 6                                                   | 0                         | 0                                                   | -2           |

```
In[ ]:= characterTableInnerProducts[
  davisopsymcharacterTable, Map[Length, davisopsymconjclasses]] ==
  IdentityMatrix[Length[davisopsymconjclasses]] // FullSimplify
```

Out[ ]:= True

Choose representatives of conjugacy classes so subgroups generated overlap as much as possible.

davisopsymconjclassrules

```
In[ ]:= davisopsymconjclassrules =
  Apply[Union, MapIndexed[Thread[#1 → #2[[1]]] &, davisopsymconjclasses]];
```

davisnormsgccind

```
In[ ]:= TableForm[davisnormsgccind = Map[davisopsymcyclicsg[#] /. davisopsymconjclassrules &,
      davisopsymconjclasses[[All, 1]]], TableDepth → 1, TableHeadings → {Range[34]}]
```

Out[ ]:=TableForm=

```
1 {1}
2 {2, 2, 1}
3 {3, 3, 1}
4 {4, 21, 4, 1}
5 {5, 6, 6, 5, 1}
6 {6, 5, 5, 6, 1}
7 {7, 8, 8, 7, 1}
8 {8, 7, 7, 8, 1}
9 {9, 9, 9, 9, 1}
10 {10, 2, 21, 2, 10, 1}
11 {11, 5, 12, 6, 21, 6, 12, 5, 11, 1}
12 {12, 6, 11, 5, 21, 5, 11, 6, 12, 1}
13 {13, 9, 13, 9, 21, 9, 13, 9, 13, 1}
14 {14, 10, 4, 2, 14, 21, 14, 2, 4, 10, 14, 1}
15 {15, 16, 6, 15, 2, 5, 16, 16, 5, 2, 15, 6, 16, 15, 1}
16 {16, 15, 5, 16, 2, 6, 15, 15, 6, 2, 16, 5, 15, 16, 1}
17 {17, 11, 18, 5, 4, 12, 18, 6, 17, 21, 17, 6, 18, 12, 4, 5, 18, 11, 17, 1}
18 {18, 12, 17, 6, 4, 11, 17, 5, 18, 21, 18, 5, 17, 11, 4, 6, 17, 12, 18, 1}
19 {19, 16, 11, 15, 10, 5, 20, 16, 12, 2, 19, 6, 20, 15, 21, 15, 20, 6, 19, 2, 12, 16, 20, 5, 10, 15,
20 {20, 15, 12, 16, 10, 6, 19, 15, 11, 2, 20, 5, 19, 16, 21, 16, 19, 5, 20, 2, 11, 15, 19, 6, 10, 16,
21 {21, 1}
22 {22, 1}
23 {23, 1}
24 {24, 1}
25 {25, 3, 21, 3, 25, 1}
26 {26, 3, 22, 3, 26, 1}
27 {27, 24, 27, 1}
28 {28, 8, 29, 7, 21, 7, 29, 8, 28, 1}
29 {29, 7, 28, 8, 21, 8, 28, 7, 29, 1}
30 {30, 8, 31, 7, 22, 7, 31, 8, 30, 1}
31 {31, 7, 30, 8, 22, 8, 30, 7, 31, 1}
32 {32, 3, 23, 3, 32, 1}
33 {33, 7, 34, 8, 23, 8, 34, 7, 33, 1}
34 {34, 8, 33, 7, 23, 7, 33, 8, 34, 1}
```

ccrep20

```
In[ ]:= ccrep20 = davisopsymconjclasses[[20, 1]];
```

```
In[ ]:= davisopsymcyclicsg[ccrep20] /. davisopsymconjclassrules
```

```
Out[ ]:= {20, 15, 12, 16, 10, 6, 19, 15, 11, 2, 20, 5, 19,
      16, 21, 16, 19, 5, 20, 2, 11, 15, 19, 6, 10, 16, 12, 15, 20, 1}
```

ccrep1, ccrep10, ccrep11, ccrep12, ccrep15, ccrep16, ccrep19, ccrep2, ccrep21, ccrep5, ccrep6

```
In[ ]:= {ccrep15, ccrep12, ccrep16, ccrep10, ccrep6, ccrep19, ccrep11, ccrep2, ccrep5, ccrep21,
      ccrep1} = davisopsymcyclicsg[ccrep20][[2, 3, 4, 5, 6, 7, 9, 10, 12, 15, 30]]];
```

covered1

```
In[ ]:= covered1 = Apply[Union, Map[davisopsymcyclicsg, {ccrep20, ccrep15, ccrep12, ccrep16,
      ccrep10, ccrep6, ccrep19, ccrep11, ccrep2, ccrep5, ccrep21, ccrep1}]]];
```

```

ccrep18
In[ ]:= ccrep18 = SortBy[davisopsymconjclasses[[18]],
    -Length[Intersection[davisopsymcyclicsg[18], covered1]] &][[1]];

In[ ]:= davisopsymcyclicsg[ccrep18] /. davisopsymconjclassrules
Out[ ]:= {18, 12, 17, 6, 4, 11, 17, 5, 18, 21, 18, 5, 17, 11, 4, 6, 17, 12, 18, 1}

ccrep17, ccrep4
In[ ]:= {ccrep17, ccrep4} = davisopsymcyclicsg[ccrep18][[3, 5]];

covered2
In[ ]:= covered2 =
    Union[covered1, Apply[Union, Map[davisopsymcyclicsg, {ccrep18, ccrep17, ccrep4}]]];

ccrep14
In[ ]:= ccrep14 = SortBy[davisopsymconjclasses[[14]],
    -Length[Intersection[davisopsymcyclicsg[14], covered2]] &][[1]];

In[ ]:= davisopsymcyclicsg[ccrep14] /. davisopsymconjclassrules
Out[ ]:= {14, 10, 4, 2, 14, 21, 14, 2, 4, 10, 14, 1}

covered3
In[ ]:= covered3 = Union[covered2, Apply[Union, Map[davisopsymcyclicsg, {ccrep14}]]];

ccrep13
In[ ]:= ccrep13 = SortBy[davisopsymconjclasses[[13]],
    -Length[Intersection[davisopsymcyclicsg[13], covered3]] &][[1]];

In[ ]:= davisopsymcyclicsg[ccrep13] /. davisopsymconjclassrules
Out[ ]:= {13, 9, 13, 9, 21, 9, 13, 9, 13, 1}

ccrep9
In[ ]:= {ccrep9} = davisopsymcyclicsg[ccrep13][[2]];

covered4
In[ ]:= covered4 = Union[covered3, Apply[Union, Map[davisopsymcyclicsg, {ccrep13, ccrep9}]]];

ccrep34
In[ ]:= ccrep34 = SortBy[davisopsymconjclasses[[34]],
    -Length[Intersection[davisopsymcyclicsg[34], covered4]] &][[1]];

In[ ]:= davisopsymcyclicsg[ccrep34] /. davisopsymconjclassrules
Out[ ]:= {34, 8, 33, 7, 23, 7, 33, 8, 34, 1}

ccrep23, ccrep33, ccrep7, ccrep8
In[ ]:= {ccrep8, ccrep33, ccrep7, ccrep23} = davisopsymcyclicsg[ccrep34][[2, 3, 4, 5]];

covered5
In[ ]:= covered5 = Union[covered4,
    Apply[Union, Map[davisopsymcyclicsg, {ccrep34, ccrep8, ccrep33, ccrep7, ccrep23}]]];

ccrep32
In[ ]:= ccrep32 = SortBy[davisopsymconjclasses[[32]],
    -Length[Intersection[davisopsymcyclicsg[32], covered5]] &][[1]];

In[ ]:= davisopsymcyclicsg[ccrep32] /. davisopsymconjclassrules
Out[ ]:= {32, 3, 23, 3, 32, 1}

```



```

ccrep3
In[ ]:= {ccrep3} = davisopsymcyclicsg[ccrep32][[{2}]];

covered6
In[ ]:= covered6 = Union[covered5, Apply[Union, Map[davisopsymcyclicsg, {ccrep32, ccrep3}]]];

ccrep31
In[ ]:= ccrep31 = SortBy[davisopsymconjclasses[[31]],
  -Length[Intersection[davisopsymcyclicsg[#], covered6]] &][[1]];

In[ ]:= davisopsymcyclicsg[ccrep31] /. davisopsymconjclassrules
Out[ ]:= {31, 7, 30, 8, 22, 8, 30, 7, 31, 1}

ccrep22, ccrep30
In[ ]:= {ccrep30, ccrep22} = davisopsymcyclicsg[ccrep31][[{3, 5}]];

covered7
In[ ]:= covered7 =
  Union[covered6, Apply[Union, Map[davisopsymcyclicsg, {ccrep31, ccrep30, ccrep22}]]];

ccrep29
In[ ]:= ccrep29 = SortBy[davisopsymconjclasses[[29]],
  -Length[Intersection[davisopsymcyclicsg[#], covered7]] &][[1]];

In[ ]:= davisopsymcyclicsg[ccrep29] /. davisopsymconjclassrules
Out[ ]:= {29, 7, 28, 8, 21, 8, 28, 7, 29, 1}

ccrep28
In[ ]:= {ccrep28} = davisopsymcyclicsg[ccrep29][[{3}]];

covered8
In[ ]:= covered8 = Union[covered7, Apply[Union, Map[davisopsymcyclicsg, {ccrep29, ccrep28}]]];

ccrep27
In[ ]:= ccrep27 = SortBy[davisopsymconjclasses[[27]],
  -Length[Intersection[davisopsymcyclicsg[#], covered8]] &][[1]];

In[ ]:= davisopsymcyclicsg[ccrep27] /. davisopsymconjclassrules
Out[ ]:= {27, 24, 27, 1}

ccrep24
In[ ]:= {ccrep24} = davisopsymcyclicsg[ccrep27][[{2}]];

covered9
In[ ]:= covered9 = Union[covered8, Apply[Union, Map[davisopsymcyclicsg, {ccrep27, ccrep24}]]];

ccrep26
In[ ]:= ccrep26 = SortBy[davisopsymconjclasses[[26]],
  -Length[Intersection[davisopsymcyclicsg[#], covered9]] &][[1]];

In[ ]:= davisopsymcyclicsg[ccrep26] /. davisopsymconjclassrules
Out[ ]:= {26, 3, 22, 3, 26, 1}

covered10
In[ ]:= covered10 = Union[covered9, Apply[Union, Map[davisopsymcyclicsg, {ccrep26}]]];

ccrep25
In[ ]:= ccrep25 = SortBy[davisopsymconjclasses[[25]],
  -Length[Intersection[davisopsymcyclicsg[#], covered10]] &][[1]];

```

```
In[ ]:= davisopsymcyclicsg[ccrep25] /. davisopsymconjclassrules
```

```
Out[ ]:= {25, 3, 21, 3, 25, 1}
```

*covered11*

```
In[ ]:= covered11 = Union[covered10, Apply[Union, Map[davisopsymcyclicsg, {ccrep25}]]];
```

```
In[ ]:= Length[covered11]
```

```
Out[ ]:= 84
```

*davisnormopconjreps*

```
In[ ]:= davisnormopconjreps = {ccrep1, ccrep2, ccrep3, ccrep4, ccrep5, ccrep6, ccrep7,
    ccrep8, ccrep9, ccrep10, ccrep11, ccrep12, ccrep13, ccrep14, ccrep15, ccrep16,
    ccrep17, ccrep18, ccrep19, ccrep20, ccrep21, ccrep22, ccrep23, ccrep24, ccrep25,
    ccrep26, ccrep27, ccrep28, ccrep29, ccrep30, ccrep31, ccrep32, ccrep33, ccrep34};
```

## Fixed points

Isolated fixed points of symmetries without inside-out factor will be in the orbit of vertices of the basic 5335 simplex. Non-isolated fixed points will be in orbits of >1-cells of the basic 5335 simplex. There are 600 vertices of the 120-cell in one orbit, 1200 midpoints of edges in orbits of 20 giving 60 different points of the manifold, 720 centers of ridges in orbits of 5 giving 144 points, 120 centers of sides in orbits of 2 giving 60 points, and the center of the 120-cell giving one point of the manifold. Find the stabilizers in the group of symmetries of all 266 points by finding stabilizers of the orbits of vertices of the basic 5335 simplex and conjugating. Find the matrices for the lifts of stabilizers that fix each fixed point by finding the matrices fixing the vertices of the 5335 simplex and conjugating to other points.

*davisspmatliftio*

```
In[ ]:= AbsoluteTiming[Dimensions[davisspmatliftio = davisspmatlift /. Dispatch[Map[
    # → ToNumberField[RootReduce[#], iofieldth] &, Union[Flatten[davisspmatlift]]]]]]
```

```
Out[ ]:= {0.1381, {120, 8, 8}}
```

*davisopsymgrpfixc, davisopsymgrprio*

```
In[ ]:= davisopsymgrpfixc = Select[davisopsymgrp, #[[1, 3]] == 0 &];
    davisopsymgrprio = Select[davisopsymgrp, #[[1, 3]] == 1 &];
```

*davisopsymgrpfixcrules*

```
In[ ]:= davisopsymgrpfixcrules =
    Dispatch[Thread[davisopsymgrpfixc → Range[Length[davisopsymgrpfixc]]]];
```

*davisopsymliftfixcprojrules*

```
In[ ]:= davisopsymliftfixcprojrules =
    Dispatch[Apply[Union, Map[{#[[1]] → (# /. davisopsymgrpfixcrules),
    #[[2]] → (# /. davisopsymgrpfixcrules)} &, davisopsymgrpfixc]]];
```

```
In[ ]:= v1orbit // Dimensions
```

```
Out[ ]:= {600, 5}
```

```
In[ ]:= v1orbit[[-1]] == verts5335[[1]]
```

```
Out[ ]:= True
```

```

v1reps
In[ ]:= v1reps = Table[Length[v1orbit], {Length[v1orbit]}];

v1traces
In[ ]:= v1traces = vertextraces;

t1reps
In[ ]:= t1reps = Union[v1reps];

t1classes
In[ ]:= t1classes =
  GatherBy[Transpose[{Range[Length[v1orbit]], v1reps}], #[[2]] &][[All, All, 1]];

In[ ]:= t1classes[[All, -1]] == t1reps

Out[ ]:= True

In[ ]:= Tally[
  Map[Apply[Dot, davisssmat[[v1traces[[#]]]]].v1orbit[[#]] == v1orbit[[v1reps[[#]]]] &,
    Range[Length[v1orbit]]]]

Out[ ]:= {{True, 600}}

t1fromconj
In[ ]:= t1fromconj = Map[Function[i1, Select[davisopsymgrpfixc,
  davisopsymmat[#].v1orbit[[i1]] == v1orbit[[-1]] &, 1][[-1, 1]]], t1reps];

v1liftstabilizer
In[ ]:= AbsoluteTiming[Dimensions[v1liftstabilizer = Apply[Union, Select[davisopsymgrpfixc,
  v1reps[[davisopsymmat[#].v1orbit[[-1]] /. v1indrules]] == v1reps[[-1]] &]]]]

Out[ ]:= {4.83727, {14400}}

v1liftstabmats
In[ ]:= AbsoluteTiming[
  Dimensions[v1liftstabmats = Map[Function[v1stab, Apply[Dot, davisssmatliftio[[v1traces[[
    (davisopsymmat[davisopsymgrpfixc[[v1stab /. davisopsymliftfixcprojrules]]].
    v1orbit[[-1]] /. v1indrules]]]]].
    davisopsymliftmat[v1stab]], v1liftstabilizer]]]

Out[ ]:= {2926.42, {14400, 8, 8}}

t1liftstabilizersandmats
In[ ]:= AbsoluteTiming[
  Dimensions[t1liftstabilizersandmats = Map[Function[t1c, MapThread[Function[{s, m},
    {davisopsymliftmultiply[davisopsymliftmultiply[davisopsymliftinverse[t1c], s],
      t1c], Inverse[#].m.# &[davisopsymliftmat[t1c]]}],
    {v1liftstabilizer, v1liftstabmats}]], t1fromconj]]]

Out[ ]:= {370.954, {1, 14400, 2}}

In[ ]:= v2orbit // Dimensions

Out[ ]:= {1200, 5}

In[ ]:= v2orbit[[-1]] == verts5335[[2]]

Out[ ]:= True

```

v2edges

```
In[ ]:= v2edges = Map[Function[i,
    (i → Map[{#, davisspmat[{#}].v2orbit[{i]}] &, ind2to4[{i]}] /. v2indrules)],
    Range[Length[v2orbit]]];
```

v2reps

```
In[ ]:= v2reps =
    Sort[Flatten[Map[Thread[{#1, #1[[-1]]}] &, FixedPoint[Function[cp, If[cp[[2]] == {}, cp,
        {Append[cp[[1]], #], Complement[cp[[2]], #]} & FixedPoint[Function[c,
            Union[c, Apply[Union, (c /. v2edges)[{All, All, 2}]]], {cp[[2, 1]]}]]],
        { {}, Range[Length[v2orbit]]}[[1]], 1]][[All, 2]]];
```

t2reps

```
In[ ]:= t2reps = Union[v2reps];
```

v2traces

```
In[ ]:= v2traces =
    SortBy[FixedPoint[Function[vs, GatherBy[Union[vs, Apply[Union, Map[Function[vp, Map[
        {#[[2]], Append[vp[[2]], 121 - #[[1]]}] &, vp[[1]] /. v2edges]], vs]]],
        #[[1]] &][[All, 1]]], Map[{#, {}] &, t2reps]], #[[1]] &][[All, 2]]];
```

t2classes

```
In[ ]:= t2classes = Sort[GatherBy[Transpose[{v2reps, Range[1200]}], #[[1]] &][[All, All, 2]]];
```

```
In[ ]:= t2classes[[All, -1]] == t2reps
```

```
Out[ ]:= True
```

```
In[ ]:= Tally[
    Map[Apply[Dot, davisspmat[v2traces[{#}]]].v2orbit[{#}] == v2orbit[v2reps[{#}]]] &,
    Range[Length[v2orbit]]]
```

```
Out[ ]:= {{True, 1200}}
```

t2fromconj

```
In[ ]:= t2fromconj = Map[Function[i1, Select[davisopsymgrpfxc,
    davisopsymmat[{#}].v2orbit[{i1}] == v2orbit[[-1]] &, 1][[-1, 1]], t2reps];
```

v2liftstabilizer

```
In[ ]:= AbsoluteTiming[Dimensions[v2liftstabilizer = Apply[Union, Select[davisopsymgrpfxc,
    v2reps[[davisopsymmat[{#}].v2orbit[[-1]] /. v2indrules]] == v2reps[[-1]] &]]]
```

```
Out[ ]:= {1.63347, {240}}
```

v2liftstabmats

```
In[ ]:= AbsoluteTiming[
    Dimensions[v2liftstabmats = Map[Function[v2stab, Apply[Dot, davisspmatliftio[v2traces[[
        (davisopsymmat[davisopsymgrpfxc[v2stab /. davisopsymliftfixcprojrules]]].
        v2orbit[[-1]] /. v2indrules]]]]].
        davisopsymliftmat[v2stab]], v2liftstabilizer]]]
```

```
Out[ ]:= {5.58489, {240, 8, 8}}
```

t2liftstabilizersandmats

```
In[ ]:= AbsoluteTiming[
  Dimensions[t2liftstabilizersandmats = Map[Function[t2c, MapThread[Function[{s, m},
    {davisopsymliftmultiply[davisopsymliftmultiply[davisopsymliftinverse[t2c], s],
      t2c], Inverse[#].m.# &[davisopsymliftmat[t2c]]}],
    {v2liftstabilizer, v2liftstabmats}]], t2fromconj]]]
```

```
Out[ ]:= {272.592, {60, 240, 2}}
```

```
In[ ]:= v3orbit // Dimensions
```

```
Out[ ]:= {720, 5}
```

```
In[ ]:= v3orbit[[-1]] == verts5335[[3]]
```

```
Out[ ]:= True
```

v3edges

```
In[ ]:= v3edges = Map[Function[i,
  (i → Map[{#, davisspmat[{#}].v3orbit[{i]}] &, ind3to4[{i}]] /. v3indrules)],
  Range[Length[v3orbit]]];
```

v3reps

```
In[ ]:= v3reps =
  Sort[Flatten[Map[Thread[{#1, #1[[-1]]}] &, FixedPoint[Function[cp, If[cp[[2]] == {}, cp,
    {Append[cp[[1]], #], Complement[cp[[2]], #]} & FixedPoint[Function[c,
      Union[c, Apply[Union, (c /. v3edges)[{All, All, 2}]]], {cp[[2, 1]]}]]],
    { {}, Range[Length[v3orbit]]}[[1]]], 1]][[All, 2]];
```

t3reps

```
In[ ]:= t3reps = Union[v3reps];
```

v3traces

```
In[ ]:= v3traces =
  SortBy[FixedPoint[Function[vs, GatherBy[Union[vs, Apply[Union, Map[Function[vp, Map[
    {#[[2]], Append[vp[[2]], 121 - #[[1]]}] &, vp[[1]] /. v3edges]], vs]]],
    #[[1]] &][[All, 1]]], Map[{#, {}] &, t3reps}], #[[1]] &][[All, 2]];
```

t3classes

```
In[ ]:= t3classes =
  Sort[GatherBy[Transpose[{v3reps, Range[Length[v3orbit]]}], #[[1]] &][[All, All, 2]];
```

```
In[ ]:= t3classes[[All, -1]] == t3reps
```

```
Out[ ]:= True
```

```
In[ ]:= Tally[
  Map[Apply[Dot, davisspmat[v3traces[{#}]]].v3orbit[{#}] == v3orbit[v3reps[{#}]] &,
  Range[Length[v3orbit]]]
```

```
Out[ ]:= {{True, 720}}
```

t3fromconj

```
In[ ]:= t3fromconj = Map[Function[i1, Select[davisopsymgrpfxc,
  davisopsymmat[#].v3orbit[{i1}] == v3orbit[[-1]] &, 1][[-1, 1]]], t3reps];
```

v3liftstabilizer

```
In[ ]:= AbsoluteTiming[Dimensions[v3liftstabilizer = Apply[Union, Select[davisopsymgrpfixc,
v3reps[[davisopsymmat[#].v3orbit[[-1]] /. v3indrulcs]] == v3reps[[-1]] &]]]]

Out[ ]:= {1.97458, {100}}
```

v3liftstabmats

```
In[ ]:= AbsoluteTiming[
Dimensions[v3liftstabmats = Map[Function[v3stab, Apply[Dot, davisspmatliftio[[v3traces[[
(davisopsymmat[davisopsymgrpfixc[[v3stab /. davisopsymliftfixcprojrules]]].
v3orbit[[-1]] /. v3indrulcs]]]]].
davisopsymliftmat[v3stab]], v3liftstabilizer]]]

Out[ ]:= {0.837405, {100, 8, 8}}
```

t3liftstabilizersandmats

```
In[ ]:= AbsoluteTiming[
Dimensions[t3liftstabilizersandmats = Map[Function[t3c, MapThread[Function[{s, m},
{davisopsymliftmultiply[davisopsymliftmultiply[davisopsymliftinverse[t3c], s],
t3c], Inverse[#].m.# &[davisopsymliftmat[t3c]]}],
{v3liftstabilizer, v3liftstabmats}]], t3fromconj]]]

Out[ ]:= {235.375, {144, 100, 2}}
```

```
In[ ]:= v4orbit // Dimensions
```

```
Out[ ]:= {120, 5}
```

```
In[ ]:= v4orbit[[120]] == verts5335[[4]]
```

```
Out[ ]:= True
```

v4edges

```
In[ ]:= v4edges =
Map[Function[i, (i → Map[{#, davisspmat[[#]].v4orbit[[i]]} &, {i}] /. v4indrulcs)],
Range[Length[v4orbit]]];
```

v4reps

```
In[ ]:= v4reps =
Sort[Flatten[Map[Thread[{#1, #1[[-1]]}] &, FixedPoint[Function[cp, If[cp[[2]] == {}, cp,
{Append[cp[[1]], #], Complement[cp[[2]], #]} & FixedPoint[Function[c,
Union[c, Apply[Union, (c /. v4edges)[[All, All, 2]]]], {cp[[2, 1]]}]]]],
{ {}, Range[Length[v4orbit]]}][[1]], 1]][[All, 2]];
```

t4reps

```
In[ ]:= t4reps = Union[v4reps];
```

v4traces

```
In[ ]:= v4traces =
SortBy[FixedPoint[Function[vs, GatherBy[Union[vs, Apply[Union, Map[Function[vp, Map[
#{[[2]], Append[vp[[2]], 121 - #[[1]]}] &, vp[[1]] /. v4edges]], vs]]],
#[[1]] &][[All, 1]]], Map[{#, {} } &, t4reps]], #[[1]] &][[All, 2]];
```

t4classes

```
In[ ]:= t4classes = Sort[GatherBy[Transpose[{v4reps, Range[120]}], #[[1]] &][[All, All, 2]];
```

```
In[ ]:= t4classes[[All, -1]] == t4reps
```

```
Out[ ]:= True
```

```
In[ ]:= Tally[
  Map[Apply[Dot, davissspmat[[v4traces[[#]]]]].v4orbit[[#]] == v4orbit[[v4reps[[#]]]] &,
    Range[Length[v4orbit]]]]
```

```
Out[ ]:= {{True, 120}}
```

t4fromconj

```
In[ ]:= t4fromconj = Map[Function[i1, Select[davisopsymgrpfixc,
  davisopsymmat[[#].v4orbit[[i1]] == v4orbit[[-1]] &, 1][[-1, 1]]], t4reps];
```

v4liftstabilizer

```
In[ ]:= AbsoluteTiming[Dimensions[v4liftstabilizer = Apply[Union, Select[davisopsymgrpfixc,
  v4reps[[davisopsymmat[[#].v4orbit[[-1]] /. v4indrules]] == v4reps[[-1]] &]]]]
```

```
Out[ ]:= {0.517516, {240}}
```

v4liftstabmats

```
In[ ]:= AbsoluteTiming[
  Dimensions[v4liftstabmats = Map[Function[v4stab, Apply[Dot, davissspmatliftio[[v4traces[[
    (davisopsymmat[davisopsymgrpfixc[[v4stab /. davisopsymliftfixcprojrules]]].
    v4orbit[[-1]] /. v4indrules]]]]].
    davisopsymliftmat[v4stab]], v4liftstabilizer]]]
```

```
Out[ ]:= {0.504082, {240, 8, 8}}
```

t4liftstabilizersandmats

```
In[ ]:= AbsoluteTiming[
  Dimensions[t4liftstabilizersandmats = Map[Function[t4c, MapThread[Function[{s, m},
    {davisopsymliftmultiply[davisopsymliftmultiply[davisopsymliftinverse[t4c], s],
    t4c], Inverse[#].m.# &[davisopsymliftmat[t4c]]}],
    {v4liftstabilizer, v4liftstabmats}]], t4fromconj]]]
```

```
Out[ ]:= {134.553, {60, 240, 2}}
```

v5orbit

```
In[ ]:= v5orbit = {verts5335[[5]]};
```

v5indrules

```
In[ ]:= v5indrules = Thread[v5orbit → Range[Length[v5orbit]]];
```

v5reps

```
In[ ]:= v5reps = {1};
```

t5reps

```
In[ ]:= t5reps = Union[v5reps];
```

v5traces

```
In[ ]:= v5traces = {{}};
```

t5classes

```
In[ ]:= t5classes = Sort[GatherBy[Transpose[{v5reps, Range[1]}], #[[1]] &]][[All, All, 2]];
```

```
In[ ]:= t5classes[[All, -1]] == t5reps
```

```
Out[ ]:= True
```

```
In[ ]:= Tally[
  Map[Apply[Dot, davissspmat[[v5traces[[#]]]]].v5orbit[[#]] == v5orbit[[v5reps[[#]]]] &,
    Range[Length[v5orbit]]]]
```

```
Out[ ]:= {{True, 1}}
```

*t5fromconj*

```
In[ ]:= t5fromconj = Map[Function[i1, Select[davisopsymgrpfixc,
      davisopsymmat[#].v5orbit[[i1]] == v5orbit[[-1]] &, 1][[-1, 1]]], t5reps];
```

*v5liftstabilizer*

```
In[ ]:= AbsoluteTiming[Dimensions[v5liftstabilizer = Apply[Union, Select[davisopsymgrpfixc,
      v5reps[[davisopsymmat[#].v5orbit[[-1]] /. v5indrules]] == v5reps[[-1]] &]]]]
```

```
Out[ ]:= {0.149637, {14400}}
```

*v5liftstabmats*

```
In[ ]:= AbsoluteTiming[
  Dimensions[v5liftstabmats = Map[Function[v5stab, Apply[Dot, davispsmatliftio[[v5traces[
    (davisopsymmat[davisopsymgrpfixc[[v5stab /. davisopsymliftfixcprojrules]]].
    v5orbit[[-1]] /. v5indrules]]]]],
    davisopsymliftmat[v5stab]], v5liftstabilizer]]]
```

```
Out[ ]:= {15.5763, {14400, 8, 8}}
```

*t5liftstabilizersandmats*

```
In[ ]:= AbsoluteTiming[
  Dimensions[t5liftstabilizersandmats = Map[Function[t5c, MapThread[Function[{s, m},
    {davisopsymliftmultiply[davisopsymliftmultiply[davisopsymliftinverse[t5c], s],
      t5c], Inverse[#].m.# &[davisopsymliftmat[t5c]]}],
    {v5liftstabilizer, v5liftstabmats}]], t5fromconj]]]
```

```
Out[ ]:= {86.7159, {1, 14400, 2}}
```

---

## Spin table

*tablesequence*

```
In[ ]:= tablesequence = {1, 3, 5, 8, 9, 11, 15, 13, 17, 20, 22, 24, 26, 27, 29, 31, 33, 36, 39, 38};
```

```
In[ ]:= davisopsymliftconjclassnames[[tablesequence]]
```

```
Out[ ]:= {1×1, 1×3+3×1, 3×3, 1×4+4×1, 1×5A+5B×1, 1×5B+5A×1, 5A×5B, 5B×5A,
  5A×5A+5B×5B, 1×6+6×1, 1×10A+10B×1, 1×10B+10A×1, 5A×10B+10A×5B, 3×4+4×3,
  3×5A+5B×3, 3×5B+5A×3, 4×5A+5B×4, 4×5B+5A×4, 3×10A+10B×3, 3×10B+10A×3}
```

```
In[ ]:= Map[Length, {v1liftstabilizer, v2liftstabilizer,
  v3liftstabilizer, v4liftstabilizer, v5liftstabilizer}]
```

```
Out[ ]:= {14400, 240, 100, 240, 14400}
```

```
In[ ]:= Sort[t2liftstabilizersandmats[[-1, All, 1]]] == Sort[v2liftstabilizer]
```

```
Out[ ]:= True
```

*conjclassrepositions*

```
In[ ]:= AbsoluteTiming[
  conjclassrepositions = Map[Position[{t1liftstabilizersandmats, t2liftstabilizersandmats,
    t3liftstabilizersandmats, t4liftstabilizersandmats, t5liftstabilizersandmats}, #] &,
    davisopsymliftconjclasses[[tablesequence, -1]]]]]
```

```
Out[ ]:= {80.8033, {{1, 1, 14400, 1}, {2, 1, 240, 1}, {2, 2, 240, 1}, {2, 3, 240, 1},
  {2, 4, 240, 1}, {2, 5, 240, 1}, {2, 6, 240, 1}, {2, 7, 240, 1}, {2, 8, 240, 1},
  {2, 9, 240, 1}, {2, 10, 240, 1}, {2, 11, 240, 1}, {2, 12, 240, 1}, {2, 13, 240, 1},
  {2, 14, 240, 1}, {2, 15, 240, 1}, {2, 16, 240, 1}, {2, 17, 240, 1}, {2, 18, 240, 1},
```



{2, 19, 240, 1}, {2, 20, 240, 1}, {2, 21, 240, 1}, {2, 22, 240, 1}, {2, 23, 240, 1},  
 {2, 24, 240, 1}, {2, 25, 240, 1}, {2, 26, 240, 1}, {2, 27, 240, 1}, {2, 28, 240, 1},  
 {2, 29, 240, 1}, {2, 30, 240, 1}, {2, 31, 240, 1}, {2, 32, 240, 1}, {2, 33, 240, 1},  
 {2, 34, 240, 1}, {2, 35, 240, 1}, {2, 36, 240, 1}, {2, 37, 240, 1}, {2, 38, 240, 1},  
 {2, 39, 240, 1}, {2, 40, 240, 1}, {2, 41, 240, 1}, {2, 42, 240, 1}, {2, 43, 240, 1},  
 {2, 44, 240, 1}, {2, 45, 240, 1}, {2, 46, 240, 1}, {2, 47, 240, 1}, {2, 48, 240, 1},  
 {2, 49, 240, 1}, {2, 50, 240, 1}, {2, 51, 240, 1}, {2, 52, 240, 1}, {2, 53, 240, 1},  
 {2, 54, 240, 1}, {2, 55, 240, 1}, {2, 56, 240, 1}, {2, 57, 240, 1}, {2, 58, 240, 1},  
 {2, 59, 240, 1}, {2, 60, 240, 1}, {3, 1, 100, 1}, {3, 2, 100, 1}, {3, 3, 100, 1},  
 {3, 4, 100, 1}, {3, 5, 100, 1}, {3, 6, 100, 1}, {3, 7, 100, 1}, {3, 8, 100, 1},  
 {3, 9, 100, 1}, {3, 10, 100, 1}, {3, 11, 100, 1}, {3, 12, 100, 1}, {3, 13, 100, 1},  
 {3, 14, 100, 1}, {3, 15, 100, 1}, {3, 16, 100, 1}, {3, 17, 100, 1}, {3, 18, 100, 1},  
 {3, 19, 100, 1}, {3, 20, 100, 1}, {3, 21, 100, 1}, {3, 22, 100, 1}, {3, 23, 100, 1},  
 {3, 24, 100, 1}, {3, 25, 100, 1}, {3, 26, 100, 1}, {3, 27, 100, 1}, {3, 28, 100, 1},  
 {3, 29, 100, 1}, {3, 30, 100, 1}, {3, 31, 100, 1}, {3, 32, 100, 1}, {3, 33, 100, 1},  
 {3, 34, 100, 1}, {3, 35, 100, 1}, {3, 36, 100, 1}, {3, 37, 100, 1}, {3, 38, 100, 1},  
 {3, 39, 100, 1}, {3, 40, 100, 1}, {3, 41, 100, 1}, {3, 42, 100, 1}, {3, 43, 100, 1},  
 {3, 44, 100, 1}, {3, 45, 100, 1}, {3, 46, 100, 1}, {3, 47, 100, 1}, {3, 48, 100, 1},  
 {3, 49, 100, 1}, {3, 50, 100, 1}, {3, 51, 100, 1}, {3, 52, 100, 1}, {3, 53, 100, 1},  
 {3, 54, 100, 1}, {3, 55, 100, 1}, {3, 56, 100, 1}, {3, 57, 100, 1}, {3, 58, 100, 1},  
 {3, 59, 100, 1}, {3, 60, 100, 1}, {3, 61, 100, 1}, {3, 62, 100, 1}, {3, 63, 100, 1},  
 {3, 64, 100, 1}, {3, 65, 100, 1}, {3, 66, 100, 1}, {3, 67, 100, 1}, {3, 68, 100, 1},  
 {3, 69, 100, 1}, {3, 70, 100, 1}, {3, 71, 100, 1}, {3, 72, 100, 1}, {3, 73, 100, 1},  
 {3, 74, 100, 1}, {3, 75, 100, 1}, {3, 76, 100, 1}, {3, 77, 100, 1}, {3, 78, 100, 1},  
 {3, 79, 100, 1}, {3, 80, 100, 1}, {3, 81, 100, 1}, {3, 82, 100, 1}, {3, 83, 100, 1},  
 {3, 84, 100, 1}, {3, 85, 100, 1}, {3, 86, 100, 1}, {3, 87, 100, 1}, {3, 88, 100, 1},  
 {3, 89, 100, 1}, {3, 90, 100, 1}, {3, 91, 100, 1}, {3, 92, 100, 1}, {3, 93, 100, 1},  
 {3, 94, 100, 1}, {3, 95, 100, 1}, {3, 96, 100, 1}, {3, 97, 100, 1}, {3, 98, 100, 1},  
 {3, 99, 100, 1}, {3, 100, 100, 1}, {3, 101, 100, 1}, {3, 102, 100, 1}, {3, 103, 100, 1},  
 {3, 104, 100, 1}, {3, 105, 100, 1}, {3, 106, 100, 1}, {3, 107, 100, 1}, {3, 108, 100, 1},  
 {3, 109, 100, 1}, {3, 110, 100, 1}, {3, 111, 100, 1}, {3, 112, 100, 1}, {3, 113, 100, 1},  
 {3, 114, 100, 1}, {3, 115, 100, 1}, {3, 116, 100, 1}, {3, 117, 100, 1}, {3, 118, 100, 1},  
 {3, 119, 100, 1}, {3, 120, 100, 1}, {3, 121, 100, 1}, {3, 122, 100, 1}, {3, 123, 100, 1},  
 {3, 124, 100, 1}, {3, 125, 100, 1}, {3, 126, 100, 1}, {3, 127, 100, 1}, {3, 128, 100, 1},  
 {3, 129, 100, 1}, {3, 130, 100, 1}, {3, 131, 100, 1}, {3, 132, 100, 1}, {3, 133, 100, 1},  
 {3, 134, 100, 1}, {3, 135, 100, 1}, {3, 136, 100, 1}, {3, 137, 100, 1}, {3, 138, 100, 1},  
 {3, 139, 100, 1}, {3, 140, 100, 1}, {3, 141, 100, 1}, {3, 142, 100, 1}, {3, 143, 100, 1},  
 {3, 144, 100, 1}, {4, 1, 240, 1}, {4, 2, 240, 1}, {4, 3, 240, 1}, {4, 4, 240, 1},  
 {4, 5, 240, 1}, {4, 6, 240, 1}, {4, 7, 240, 1}, {4, 8, 240, 1}, {4, 9, 240, 1},  
 {4, 10, 240, 1}, {4, 11, 240, 1}, {4, 12, 240, 1}, {4, 13, 240, 1}, {4, 14, 240, 1},  
 {4, 15, 240, 1}, {4, 16, 240, 1}, {4, 17, 240, 1}, {4, 18, 240, 1}, {4, 19, 240, 1},  
 {4, 20, 240, 1}, {4, 21, 240, 1}, {4, 22, 240, 1}, {4, 23, 240, 1}, {4, 24, 240, 1},  
 {4, 25, 240, 1}, {4, 26, 240, 1}, {4, 27, 240, 1}, {4, 28, 240, 1}, {4, 29, 240, 1},  
 {4, 30, 240, 1}, {4, 31, 240, 1}, {4, 32, 240, 1}, {4, 33, 240, 1}, {4, 34, 240, 1},  
 {4, 35, 240, 1}, {4, 36, 240, 1}, {4, 37, 240, 1}, {4, 38, 240, 1}, {4, 39, 240, 1},  
 {4, 40, 240, 1}, {4, 41, 240, 1}, {4, 42, 240, 1}, {4, 43, 240, 1}, {4, 44, 240, 1},  
 {4, 45, 240, 1}, {4, 46, 240, 1}, {4, 47, 240, 1}, {4, 48, 240, 1}, {4, 49, 240, 1},  
 {4, 50, 240, 1}, {4, 51, 240, 1}, {4, 52, 240, 1}, {4, 53, 240, 1}, {4, 54, 240, 1},  
 {4, 55, 240, 1}, {4, 56, 240, 1}, {4, 57, 240, 1}, {4, 58, 240, 1}, {4, 59, 240, 1},  
 {4, 60, 240, 1}, {5, 1, 14400, 1}, {{1, 1, 14313, 1}, {5, 1, 14312, 1}},  
 {{1, 1, 3873, 1}, {2, 1, 45, 1}, {2, 26, 45, 1}, {2, 45, 45, 1}, {4, 28, 65, 1},

```

{4, 47, 65, 1}, {4, 60, 63, 1}, {5, 1, 3872, 1}}, {{1, 1, 14354, 1}, {5, 1, 14353, 1}},
{{1, 1, 14365, 1}, {3, 1, 98, 1}, {3, 3, 98, 1}, {3, 20, 98, 1}, {3, 23, 98, 1},
{3, 26, 98, 1}, {3, 29, 98, 1}, {3, 34, 98, 1}, {3, 51, 98, 1}, {3, 54, 98, 1}, {3, 58, 98, 1},
{3, 60, 98, 1}, {3, 65, 98, 1}, {3, 83, 99, 1}, {3, 86, 99, 1}, {3, 91, 99, 1},
{3, 97, 99, 1}, {3, 100, 99, 1}, {3, 110, 99, 1}, {3, 115, 99, 1}, {3, 117, 99, 1},
{3, 121, 99, 1}, {3, 124, 99, 1}, {3, 133, 99, 1}, {3, 144, 99, 1}, {5, 1, 14367, 1}},
{{1, 1, 14291, 1}, {3, 1, 96, 1}, {3, 3, 96, 1}, {3, 20, 96, 1}, {3, 23, 96, 1},
{3, 26, 96, 1}, {3, 29, 96, 1}, {3, 34, 96, 1}, {3, 51, 96, 1}, {3, 54, 96, 1}, {3, 58, 96, 1},
{3, 60, 96, 1}, {3, 65, 96, 1}, {3, 83, 97, 1}, {3, 86, 97, 1}, {3, 91, 97, 1},
{3, 97, 97, 1}, {3, 100, 97, 1}, {3, 110, 97, 1}, {3, 115, 97, 1}, {3, 117, 97, 1},
{3, 121, 97, 1}, {3, 124, 97, 1}, {3, 133, 97, 1}, {3, 144, 97, 1}, {5, 1, 14293, 1}},
{{1, 1, 10091, 1}, {3, 1, 81, 1}, {3, 3, 81, 1}, {3, 133, 82, 1},
{3, 144, 82, 1}, {5, 1, 10333, 1}}, {{1, 1, 1285, 1}, {3, 1, 13, 1},
{3, 3, 13, 1}, {3, 133, 14, 1}, {3, 144, 14, 1}, {5, 1, 1527, 1}},
{{1, 1, 10165, 1}, {2, 1, 170, 1}, {2, 2, 168, 1}, {2, 12, 170, 1}, {2, 14, 170, 1},
{2, 18, 170, 1}, {3, 1, 83, 1}, {3, 3, 83, 1}, {3, 133, 84, 1}, {3, 144, 84, 1},
{4, 16, 174, 1}, {4, 27, 174, 1}, {4, 48, 174, 1}, {4, 59, 174, 1},
{4, 60, 174, 1}, {5, 1, 10407, 1}}, {{1, 1, 14387, 1}, {5, 1, 14386, 1}},
{{1, 1, 14397, 1}, {5, 1, 14399, 1}}, {{1, 1, 14323, 1}, {5, 1, 14325, 1}},
{{1, 1, 13931, 1}, {2, 54, 229, 1}, {2, 55, 229, 1}, {2, 58, 237, 1}, {2, 59, 237, 1},
{2, 60, 223, 1}, {4, 1, 237, 1}, {4, 3, 237, 1}, {4, 4, 237, 1}, {4, 7, 237, 1},
{4, 8, 237, 1}, {5, 1, 14173, 1}}, {{1, 1, 8793, 1}, {5, 1, 8912, 1}},
{{1, 1, 3925, 1}, {5, 1, 3927, 1}}, {{1, 1, 10113, 1}, {5, 1, 10352, 1}},
{{1, 1, 8845, 1}, {5, 1, 8967, 1}}, {{1, 1, 10154, 1}, {5, 1, 10393, 1}},
{{1, 1, 5073, 1}, {5, 1, 5312, 1}}, {{1, 1, 13953, 1}, {5, 1, 14192, 1}}}

```

```
In[ ]:= Map[Length, conjclassrepositions]
```

```
Out[ ]:= {266, 2, 8, 2, 26, 26, 6, 6, 16, 2, 2, 2, 12, 2, 2, 2, 2, 2, 2}
```

*noninfpositions*

```
In[ ]:= noninfpositions = {2, 4, 5, 6, 7, 8, 10, 11, 12, 13, 14, 15, 16, 17, 18, 19, 20};
```

*spinnuofptandmat*

```
In[ ]:= spinnuofptandmat[pr_, mliftatfp_] :=
Function[p, RootReduce[(Sqrt[-ldot[p, p]] / p[[-1]]) * Simplify[
2 * (#[1, 1, 1] - #[2, 2, 1]) &[rmattoqmat[mliftatfp]] / Det[
spinprojection[mliftatfp] - IdentityMatrix[5] - KroneckerProduct[p, p].jmat[4] /
(-ldot[p, p])]]]]][ToNumberField[pr, iofieldth]];
```

*spinnuofptandmatchcheck*

```
In[ ]:= spinnuofptandmatchcheck[pr_, mliftatfp_] :=
Function[p, spinprojection[mliftatfp].p == p][ToNumberField[pr, iofieldth]];
```

## Results

```
In[ ]:= Column[formatkappa[verts5335]]
{κ (2 + 3 τ), κ (1 + τ), 0, κ, 5 + 8 τ}
{κ (1 + τ), κ, 0, 0, 2 + 3 τ}
Out[ ]:= {κ τ, κ (-1/5 + 2τ/5), κ (3/5 - τ/5), 0, 1 + 2 τ}
{κ, 0, 0, 0, 1 + τ}
{0, 0, 0, 0, 1}
```

```
In[ ]:= TableForm[Map[Function[n,
  Function[{name, sym, ccpos}, Join[{name, {Map[formatkappa, pquats[[sym[[1]]]]},
    Map[formatkappa, pquats[[sym[[2]]]]}, 0}, Length[ccpos]],
  Prepend[Flatten[#, 1], Row[{"spin# = ", FullSimplify[Total[#[[All, -1]]]]}] &[
    Map[Function[i, {formatkappa[#1], MatrixForm[rmattoqmat[formatkappa[RootReduce[
      #2]]]], MatrixForm[formatkappa[RootReduce[spinprojection[#2]]]],
      spinuofptandmat[#1, #2]] &[{v1orbit, v2orbit, v3orbit, v4orbit, v5orbit}][[
        i[[1]], {t1reps, t2reps, t3reps, t4reps, t5reps}][[i[[1]], i[[2]]]]]],
      {t1liftstabilizersandmats, t2liftstabilizersandmats, t3liftstabilizersandmats,
        t4liftstabilizersandmats, t5liftstabilizersandmats}][[
        i[[1]], i[[2]], i[[3]], 2]]]], ccpos]]][[
    davisopsymliftconjclassnames[tablesequence[[n]]],
    davisopsymliftconjclasses[[
      tablesequence[[n]], -1]],
    conjclassrepositions[[n]]],
    noninfpositions], TableDepth →
  2,
  TableDirections →
  {Column,
    Column}, TableSpacing → {8,
    1}]
```

Out[ ]//TableForm=

1×3+3×1

$$\left\{1, -\frac{1}{2} + \mathbb{k} \left(-\frac{1}{2} + \frac{\tau}{2}\right) + \frac{i\tau}{2}, 0\right\}$$

2

spin# = 0

$$\{\kappa (2 + 3 \tau), \kappa (1 + \tau), 0, \kappa, 5 + 8 \tau\}$$

$$\left( \begin{array}{cc} -\frac{7}{2} - 6 \tau + \mathbb{k} \left(\frac{1}{2} + \frac{3\tau}{2}\right) + i \left(2 + \frac{7\tau}{2}\right) & \kappa \left(-\frac{3}{2} - 3 \tau\right) + \mathbb{k} \kappa \left(-\frac{1}{2} + \frac{\tau}{2}\right) + \frac{i\kappa\tau}{2} \\ i \kappa \left(-\frac{3}{2} - 2 \tau\right) + \mathbb{k} \kappa \left(-1 - \frac{\tau}{2}\right) + \kappa \left(\frac{3}{2} + \frac{3\tau}{2}\right) & 4 + i (-2 - 3 \tau) + \mathbb{k} (-1 - \tau) + 6 \tau \end{array} \right)$$

$$\left( \begin{array}{ccccc} -\frac{229}{2} - \frac{369\tau}{2} & -\frac{95}{2} - 77\tau & 0 & -18 - \frac{59\tau}{2} & \kappa (51 + 84 \tau) \\ -\frac{79}{2} - 64\tau & -17 - 27\tau & \frac{1}{2} - \frac{\tau}{2} & -6 - \frac{21\tau}{2} & \kappa (18 + 29 \tau) \\ 0 & -\frac{1}{2} + \frac{\tau}{2} & -\frac{1}{2} & -\frac{\tau}{2} & 0 \\ -15 - \frac{49\tau}{2} & -6 - \frac{21\tau}{2} & \frac{\tau}{2} & -2 - \frac{9\tau}{2} & \kappa (7 + 11 \tau) \\ \kappa (-51 - 81 \tau) & \kappa (-21 - 34 \tau) & 0 & \kappa (-8 - 13 \tau) & 133 + 216 \tau \end{array} \right)$$

-1/3

$$\{0, 0, 0, 0, 1\}$$

$$\left( \begin{array}{c} 1 \\ 0 \end{array} \quad \begin{array}{c} 0 \\ -\frac{1}{2} + \mathbb{k} \left(-\frac{1}{2} + \frac{\tau}{2}\right) + \frac{i\tau}{2} \end{array} \right)$$

$$\left( \begin{array}{ccccc} -\frac{1}{2} & \frac{\tau}{2} & 0 & -\frac{1}{2} + \frac{\tau}{2} & 0 \\ -\frac{\tau}{2} & -\frac{1}{2} & \frac{1}{2} - \frac{\tau}{2} & 0 & 0 \\ 0 & 1 & \tau & 1 & \tau & 0 \end{array} \right)$$

$$1 \times 4 + 4 \times 1$$

$$\{1, \mathbf{i}, 0\}$$

$$2$$

$$\text{spin}\sharp = 0$$

$$\{\kappa(2+3\tau), \kappa(1+\tau), 0, \kappa, 5+8\tau\}$$

$$\begin{pmatrix} -2 + \mathbf{i} \left(-\frac{3}{2} - 2\tau\right) - 4\tau + \mathbb{k} \left(\frac{1}{2} + \frac{3\tau}{2}\right) + \mathbf{j} \left(2 + \frac{7\tau}{2}\right) & -\frac{\mathbb{k}\kappa}{2} + \kappa \left(-\frac{1}{2} - \frac{3\tau}{2}\right) + \mathbf{i} \kappa(-1-\tau) + \mathbf{j} \kappa \left(1 + \frac{3\tau}{2}\right) \\ -\frac{\mathbb{k}\kappa}{2} + \mathbf{j} \kappa \left(-1 - \frac{3\tau}{2}\right) + \kappa \left(\frac{3}{2} + \frac{3\tau}{2}\right) & 3 + \mathbf{j} \left(-2 - \frac{7\tau}{2}\right) + 4\tau + \mathbf{i} \left(\frac{1}{2} + \tau\right) + \mathbb{k} \left(\frac{1}{2} + \frac{3\tau}{2}\right) \end{pmatrix}$$

$$\begin{pmatrix} -76 - 123\tau & -27 - 44\tau & -4 - 7\tau & -11 - 18\tau & \kappa(33 + 55\tau) \\ -31 - 50\tau & -11 - 18\tau & -1 - 3\tau & -4 - 7\tau & \kappa(14 + 22\tau) \\ 4 + 7\tau & 1 + 3\tau & 0 & 1 + \tau & \kappa(-2 - 3\tau) \\ -11 - 18\tau & -4 - 7\tau & -1 - \tau & -1 - 3\tau & \kappa(5 + 8\tau) \\ \kappa(-35 - 55\tau) & \kappa(-12 - 20\tau) & \kappa(-2 - 3\tau) & \kappa(-5 - 8\tau) & 89 + 144\tau \end{pmatrix}$$

$$-\frac{1}{2}$$

$$\{0, 0, 0, 0, 1\}$$

$$\begin{pmatrix} 1 & 0 \\ 0 & \mathbf{i} \end{pmatrix}$$

$$\begin{pmatrix} 0 & 1 & 0 & 0 & 0 \\ -1 & 0 & 0 & 0 & 0 \\ 0 & 0 & 0 & -1 & 0 \\ 0 & 0 & 1 & 0 & 0 \\ 0 & 0 & 0 & 0 & 1 \end{pmatrix}$$

$$\frac{1}{2}$$

$$1 \times 5A + 5B \times 1$$

$$\left\{ 1, -\frac{1}{2} + \frac{j}{2} + \frac{\tau}{2} + \frac{i\tau}{2}, 0 \right\}$$

$$26$$

$$\text{spin}\# = 5 \sqrt{5}$$

$$\{ \kappa (2 + 3\tau), \kappa (1 + \tau), 0, \kappa, 5 + 8\tau \}$$

$$\begin{pmatrix} -4 + \mathbb{k} \left( -\frac{3}{2} - 2\tau \right) - \frac{15\tau}{2} + i \left( \frac{1}{2} + \frac{3\tau}{2} \right) & \kappa \left( -\frac{3}{2} - 3\tau \right) + \mathbb{k} \kappa (-1 - \tau) + i \kappa \left( -\frac{1}{2} - \frac{\tau}{2} \right) - \frac{j\kappa\tau}{2} \\ i \kappa \left( -1 - \frac{3\tau}{2} \right) + \frac{j\kappa\tau}{2} + \frac{\mathbb{k}\kappa\tau}{2} + \kappa \left( 2 + \frac{5\tau}{2} \right) & 5 + i \left( -\frac{1}{2} - \tau \right) + 7\tau + \mathbb{k} \left( \frac{1}{2} + \frac{3\tau}{2} \right) + j \left( 1 + \frac{3\tau}{2} \right) \end{pmatrix}$$

$$\begin{pmatrix} -\frac{275}{2} - 223\tau & -\frac{107}{2} - \frac{175\tau}{2} & 1 + \frac{3\tau}{2} & -18 - 29\tau & \kappa (61 + 100\tau) \\ -\frac{103}{2} - \frac{165\tau}{2} & -20 - 33\tau & 1 + \frac{\tau}{2} & -\frac{13}{2} - 11\tau & \kappa (23 + 37\tau) \\ -1 - \frac{3\tau}{2} & -1 - \frac{\tau}{2} & -\frac{\tau}{2} & -\frac{\tau}{2} & \kappa\tau \\ -22 - 36\tau & -\frac{17}{2} - 14\tau & \frac{\tau}{2} & -\frac{5}{2} - \frac{11\tau}{2} & \kappa (10 + 16\tau) \\ \kappa (-62 - 99\tau) & \kappa (-24 - 39\tau) & \kappa\tau & \kappa (-8 - 13\tau) & 161 + 260\tau \end{pmatrix}$$

$$\frac{1}{10} (-5 + \sqrt{5})$$

$$\left\{ 0, \kappa \left( \frac{2}{5} + \frac{\tau}{5} \right), \kappa \left( -\frac{1}{5} - \frac{3\tau}{5} \right), \kappa, 1 + 2\tau \right\}$$

$$\begin{pmatrix} \frac{1}{2} + j \left( 1 + \frac{\tau}{2} \right) + \tau + i \left( \frac{1}{2} + \frac{3\tau}{2} \right) & -\frac{\mathbb{k}\kappa}{2} + j \kappa \left( -\frac{1}{2} - \frac{\tau}{2} \right) + \frac{i\kappa\tau}{2} \\ \mathbb{k}\kappa\tau & -1 - \tau + j\tau + i(1 + \tau) \end{pmatrix}$$

$$\begin{pmatrix} -\frac{1}{2} + \frac{\tau}{2} & \frac{\tau}{2} & \frac{1}{2} & 0 & 0 \\ -\frac{\tau}{2} & -\frac{3}{2} - \frac{5\tau}{2} & 3 + 4\tau & -\frac{5}{2} - 4\tau & \kappa (1 + 3\tau) \\ -\frac{1}{2} & 3 + 4\tau & -\frac{9}{2} - \frac{13\tau}{2} & 4 + \frac{13\tau}{2} & \kappa (-3 - 4\tau) \\ 0 & -\frac{3}{2} - 3\tau & 3 + \frac{9\tau}{2} & -\frac{5}{2} - \frac{11\tau}{2} & \kappa (2 + 3\tau) \\ 0 & \kappa (-2 - 2\tau) & \kappa (2 + 4\tau) & \kappa (-2 - 4\tau) & 9 + 14\tau \end{pmatrix}$$

$$\frac{1}{\sqrt{5}}$$

$$\left\{ 0, \kappa \left( -\frac{2}{5} + \frac{4\tau}{5} \right), \kappa \left( -\frac{4}{5} - \frac{2\tau}{5} \right), 0, 1 + 2\tau \right\}$$

$$\begin{pmatrix} \frac{1}{2} + j \left( 1 + \frac{\tau}{2} \right) + \tau + i \left( \frac{1}{2} + \frac{3\tau}{2} \right) & \frac{i\kappa}{2} + \mathbb{k} \kappa \left( -\frac{1}{2} - \frac{\tau}{2} \right) - \frac{j\kappa\tau}{2} \\ \frac{i\kappa}{2} + \mathbb{k} \kappa \left( \frac{1}{2} + \frac{\tau}{2} \right) - \frac{j\kappa\tau}{2} & -1 - \tau + j\tau + i(1 + \tau) \end{pmatrix}$$

$$\begin{pmatrix} -\frac{1}{2} + \frac{\tau}{2} & \frac{\tau}{2} & \frac{1}{2} & 0 & 0 \\ -\frac{\tau}{2} & -2 - 4\tau & \frac{9}{2} + 6\tau & -\frac{1}{2} - \frac{\tau}{2} & \kappa (2 + 3\tau) \\ -\frac{1}{2} & \frac{9}{2} + 6\tau & -\frac{13}{2} - 10\tau & \frac{1}{2} + \tau & \kappa (-3 - 5\tau) \\ 0 & \frac{1}{2} + \frac{\tau}{2} & -\frac{1}{2} - \tau & -\frac{\tau}{2} & -\kappa \\ 0 & \kappa (-2 - 3\tau) & \kappa (3 + 5\tau) & -\kappa & 9 + 14\tau \end{pmatrix}$$

$$\frac{1}{\sqrt{5}}$$

$$\left\{ \kappa \left( \frac{2}{5} + \frac{\tau}{5} \right), \kappa \left( -\frac{3}{5} + \frac{\tau}{5} \right), \kappa \left( \frac{4}{5} + \frac{2\tau}{5} \right), \kappa \left( \frac{1}{5} - \frac{2\tau}{5} \right), 1 + 2\tau \right\}$$

$$\begin{pmatrix} \frac{1}{2} + i \left( 1 + \frac{\tau}{2} \right) + \tau + \mathbb{k} \left( \frac{1}{2} + \frac{3\tau}{2} \right) & \frac{\kappa\tau}{2} - \frac{i\kappa\tau}{2} + \frac{j\kappa\tau}{2} + \frac{\mathbb{k}\kappa\tau}{2} \\ \frac{i\kappa}{2} + \mathbb{k} \kappa \left( -\frac{1}{2} - \frac{\tau}{2} \right) + \frac{j\kappa\tau}{2} & -1 - \tau + j\tau + i(1 + \tau) \end{pmatrix}$$

$$\begin{pmatrix} -\frac{3}{2} - \frac{5\tau}{2} & 1 + \tau & -3 - \frac{11\tau}{2} & \frac{3}{2} + 2\tau & \kappa (1 + 3\tau) \\ \frac{1}{2} + \tau & -\frac{\tau}{2} & 1 + 3\tau & -\frac{1}{2} - \frac{\tau}{2} & \kappa (-1 - \tau) \\ -3 - 5\tau & \frac{1}{2} + \frac{3\tau}{2} & -\frac{13}{2} - 10\tau & 3 + \frac{7\tau}{2} & \kappa (3 + 5\tau) \\ 1 + \frac{\tau}{2} & -\frac{1}{2} & \frac{3}{2} + \frac{5\tau}{2} & -1 - \tau & \kappa (-1 - \tau) \\ \kappa (-2 - 2\tau) & \kappa\tau & \kappa (-3 - 5\tau) & \kappa (1 + 2\tau) & 9 + 14\tau \end{pmatrix}$$

$$\frac{1}{\sqrt{5}}$$

$$1 \times 5B + 5A \times 1$$

$$\left\{ 1, \frac{i}{2} + j \left( -\frac{1}{2} + \frac{\tau}{2} \right) - \frac{\tau}{2}, 0 \right\}$$

$$26$$

$$\text{spin}\# = -5 \sqrt{5}$$

$$\{ \kappa (2 + 3 \tau), \kappa (1 + \tau), 0, \kappa, 5 + 8 \tau \}$$

$$\left( \begin{array}{ccccc} -\frac{3}{2} + i \left( -\frac{3}{2} - 2 \tau \right) - \frac{5 \tau}{2} + k \left( 2 + \frac{7 \tau}{2} \right) & i \kappa (-1 - \tau) + \kappa \left( -\frac{1}{2} - \tau \right) + j \kappa \left( \frac{1}{2} + \frac{\tau}{2} \right) + \frac{3 k \kappa \tau}{2} & & & \\ k \kappa \left( -\frac{3}{2} - \tau \right) + j \kappa \left( -\frac{1}{2} - \frac{\tau}{2} \right) + \frac{i \kappa \tau}{2} + \kappa (1 + \tau) & 2 + j \left( -\frac{3}{2} - \frac{5 \tau}{2} \right) + k \left( -\frac{3}{2} - 2 \tau \right) + 3 \tau + i \left( 1 + \frac{3 \tau}{2} \right) & & & \\ -53 - \frac{169 \tau}{2} & -\frac{35}{2} - 29 \tau & -\frac{3}{2} - \frac{5 \tau}{2} & -11 - 18 \tau & \kappa (23 + 38 \tau) \\ -\frac{45}{2} - 36 \tau & -8 - 12 \tau & -\frac{1}{2} - \frac{3 \tau}{2} & -4 - \frac{15 \tau}{2} & \kappa (10 + 16 \tau) \\ \frac{3}{2} + \frac{5 \tau}{2} & \frac{1}{2} + \frac{3 \tau}{2} & -\frac{1}{2} + \frac{\tau}{2} & \frac{1}{2} + \frac{\tau}{2} & \kappa (-1 - \tau) \\ -4 - 7 \tau & -1 - \frac{5 \tau}{2} & -\frac{1}{2} - \frac{\tau}{2} & -\frac{1}{2} - 2 \tau & \kappa (2 + 3 \tau) \\ \kappa (-24 - 38 \tau) & \kappa (-8 - 13 \tau) & \kappa (-1 - \tau) & \kappa (-5 - 8 \tau) & 61 + 100 \tau \end{array} \right)$$

$$\frac{1}{10} (-5 - \sqrt{5})$$

$$\left\{ 0, \kappa \left( \frac{2}{5} + \frac{\tau}{5} \right), \kappa \left( -\frac{1}{5} - \frac{3 \tau}{5} \right), \kappa, 1 + 2 \tau \right\}$$

$$\left( \begin{array}{ccccc} -1 - \tau & -\frac{i \kappa}{2} + k \kappa \left( \frac{1}{2} - \frac{\tau}{2} \right) + \frac{j \kappa \tau}{2} & & & \\ \frac{j \kappa}{2} + i \kappa \left( \frac{1}{2} - \frac{\tau}{2} \right) - \frac{k \kappa \tau}{2} & \frac{1}{2} + i \left( -\frac{1}{2} - \frac{\tau}{2} \right) + \tau - \frac{j \tau}{2} & & & \\ -\frac{\tau}{2} & \frac{1}{2} & -\frac{1}{2} + \frac{\tau}{2} & 0 & 0 \\ -\frac{1}{2} & -1 - \tau & \frac{1}{2} + \frac{3 \tau}{2} & -\frac{\tau}{2} & \kappa \tau \\ \frac{1}{2} - \frac{\tau}{2} & \frac{1}{2} + \frac{3 \tau}{2} & -\frac{3}{2} - \frac{5 \tau}{2} & \frac{1}{2} + \frac{\tau}{2} & \kappa (-1 - \tau) \\ 0 & -1 - \frac{5 \tau}{2} & \frac{5}{2} + \frac{7 \tau}{2} & -\frac{1}{2} - 2 \tau & \kappa (1 + 2 \tau) \\ 0 & \kappa (-1 - \tau) & \kappa (1 + 2 \tau) & -\kappa \tau & 3 + 6 \tau \end{array} \right)$$

$$-\frac{1}{\sqrt{5}}$$

$$\left\{ 0, \kappa \left( -\frac{2}{5} + \frac{4 \tau}{5} \right), \kappa \left( -\frac{4}{5} - \frac{2 \tau}{5} \right), 0, 1 + 2 \tau \right\}$$

$$\left( \begin{array}{ccccc} -1 - \tau & -\frac{i \kappa}{2} + k \kappa \left( -\frac{1}{2} + \frac{\tau}{2} \right) + \frac{j \kappa \tau}{2} & & & \\ -\frac{i \kappa}{2} + k \kappa \left( \frac{1}{2} - \frac{\tau}{2} \right) + \frac{j \kappa \tau}{2} & \frac{1}{2} + i \left( -\frac{1}{2} - \frac{\tau}{2} \right) + \tau - \frac{j \tau}{2} & & & \\ -\frac{\tau}{2} & \frac{1}{2} & -\frac{1}{2} + \frac{\tau}{2} & 0 & 0 \\ -\frac{1}{2} & -\frac{1}{2} - 2 \tau & \frac{3}{2} + 2 \tau & \frac{1}{2} + \tau & \kappa (1 + \tau) \\ \frac{1}{2} - \frac{\tau}{2} & \frac{3}{2} + 2 \tau & -2 - 4 \tau & -1 - \frac{3 \tau}{2} & \kappa (-1 - 2 \tau) \\ 0 & -\frac{1}{2} - \tau & 1 + \frac{3 \tau}{2} & -\frac{1}{2} + \frac{\tau}{2} & \kappa \tau \\ 0 & \kappa (-1 - \tau) & \kappa (1 + 2 \tau) & \kappa \tau & 3 + 6 \tau \end{array} \right)$$

$$-\frac{1}{\sqrt{5}}$$

$$\left\{ \kappa \left( \frac{2}{5} + \frac{\tau}{5} \right), \kappa \left( -\frac{3}{5} + \frac{\tau}{5} \right), \kappa \left( \frac{4}{5} + \frac{2 \tau}{5} \right), \kappa \left( \frac{1}{5} - \frac{2 \tau}{5} \right), 1 + 2 \tau \right\}$$

$$\left( \begin{array}{ccccc} -1 - \tau & -\frac{\kappa}{2} + i \kappa \left( -\frac{1}{2} + \frac{\tau}{2} \right) - \frac{j \kappa \tau}{2} & & & \\ \frac{k \kappa}{2} + \kappa \left( -\frac{1}{2} + \frac{\tau}{2} \right) - \frac{j \kappa \tau}{2} & \frac{1}{2} + i \left( -\frac{1}{2} - \frac{\tau}{2} \right) + \tau - \frac{j \tau}{2} & & & \\ -1 - \tau & \tau & -1 - \tau & 0 & \kappa \tau \\ -\frac{1}{2} & -\frac{\tau}{2} & 0 & -\frac{1}{2} + \frac{\tau}{2} & 0 \\ -1 - \frac{5 \tau}{2} & \frac{1}{2} + \frac{3 \tau}{2} & -2 - 4 \tau & -\frac{1}{2} & \kappa (1 + 2 \tau) \\ \frac{1}{2} + \frac{3 \tau}{2} & -\frac{1}{2} - \tau & 2 + 2 \tau & -\frac{\tau}{2} & \kappa (-1 - \tau) \\ \kappa (-1 - \tau) & \kappa \tau & \kappa (-1 - 2 \tau) & 0 & 3 + 6 \tau \end{array} \right)$$

$$-\frac{1}{\sqrt{5}}$$

5A×5B

$$\left\{ -\frac{1}{2} + \frac{j}{2} + \frac{\tau}{2} + \frac{j\tau}{2}, \frac{j}{2} + j \left( -\frac{1}{2} + \frac{\tau}{2} \right) - \frac{\tau}{2}, 0 \right\}$$

6

spin $\sharp = 0$ 

$$\{ \kappa (2 + 3 \tau), \kappa (1 + \tau), 0, \kappa, 5 + 8 \tau \}$$

$$\left( \begin{array}{cc} \frac{5}{2} + j \left( -\frac{3}{2} - \frac{3\tau}{2} \right) + j \left( -\frac{1}{2} - \frac{\tau}{2} \right) + \frac{9\tau}{2} + k \left( \frac{1}{2} + \frac{3\tau}{2} \right) & k \kappa \tau + \kappa (1 + 2 \tau) \\ -\frac{k \kappa}{2} + \kappa \left( -1 - \frac{3\tau}{2} \right) + j \kappa \left( \frac{1}{2} + \frac{3\tau}{2} \right) & -3 + k \left( -1 - \frac{\tau}{2} \right) - \frac{9\tau}{2} - \frac{j\tau}{2} + j \left( 1 + \frac{3\tau}{2} \right) \end{array} \right)$$

$$\left( \begin{array}{ccccc} -\frac{115}{2} - 93 \tau & -\frac{47}{2} - \frac{75\tau}{2} & 1 + \frac{3\tau}{2} & -4 - 7 \tau & \kappa (25 + 42 \tau) \\ -\frac{39}{2} - \frac{63\tau}{2} & -\frac{17}{2} - 13 \tau & \tau & -1 - \frac{5\tau}{2} & \kappa (9 + 14 \tau) \\ -2 - \frac{9\tau}{2} & -1 - 2 \tau & -\frac{1}{2} & -\frac{1}{2} - \frac{\tau}{2} & \kappa (1 + 2 \tau) \\ -11 - 18 \tau & -4 - \frac{15\tau}{2} & \frac{1}{2} + \frac{\tau}{2} & -\frac{1}{2} - 2 \tau & \kappa (5 + 8 \tau) \\ \kappa (-26 - 41 \tau) & \kappa (-10 - 17 \tau) & \kappa \tau & \kappa (-2 - 3 \tau) & 67 + 108 \tau \end{array} \right)$$

$$\frac{1}{\sqrt{5}}$$

$$\left\{ 0, \kappa \left( \frac{2}{5} + \frac{\tau}{5} \right), \kappa \left( -\frac{1}{5} - \frac{3\tau}{5} \right), \kappa, 1 + 2 \tau \right\}$$

$$\left( \begin{array}{cc} j \left( -\frac{1}{2} - \tau \right) + j \left( -\frac{1}{2} - \frac{\tau}{2} \right) - \frac{\tau}{2} - \frac{j \kappa}{2} + k \kappa \left( -\frac{1}{2} + \frac{\tau}{2} \right) + \frac{j \kappa \tau}{2} & \\ -k \kappa & \frac{1}{2} + j \left( -\frac{1}{2} - \frac{\tau}{2} \right) + \tau - \frac{j \tau}{2} \end{array} \right)$$

$$\left( \begin{array}{ccccc} -\frac{1}{2} + \frac{\tau}{2} & \frac{\tau}{2} & \frac{1}{2} & 0 & 0 \\ -\frac{\tau}{2} & -1 - \frac{\tau}{2} & 1 + \frac{3\tau}{2} & -1 - \frac{5\tau}{2} & \kappa (1 + \tau) \\ -\frac{1}{2} & 1 + \frac{3\tau}{2} & -2 - 2 \tau & \frac{5}{2} + \frac{7\tau}{2} & \kappa (-1 - 2 \tau) \\ 0 & -\frac{\tau}{2} & \frac{1}{2} + \frac{\tau}{2} & -\frac{1}{2} - 2 \tau & \kappa \tau \\ 0 & -\kappa \tau & \kappa (1 + \tau) & \kappa (-1 - 2 \tau) & 3 + 6 \tau \end{array} \right)$$

$$\frac{1}{10} (-5 - \sqrt{5})$$

$$\left\{ 0, \kappa \left( -\frac{2}{5} + \frac{4\tau}{5} \right), \kappa \left( -\frac{4}{5} - \frac{2\tau}{5} \right), 0, 1 + 2 \tau \right\}$$

$$\left( \begin{array}{cc} j \left( -\frac{1}{2} - \tau \right) + j \left( -\frac{1}{2} - \frac{\tau}{2} \right) - \frac{\tau}{2} - \frac{j \kappa}{2} + j \kappa \left( \frac{1}{2} - \frac{\tau}{2} \right) + \frac{k \kappa \tau}{2} & \\ \frac{j \kappa}{2} + j \kappa \left( \frac{1}{2} - \frac{\tau}{2} \right) - \frac{k \kappa \tau}{2} & \frac{1}{2} + j \left( -\frac{1}{2} - \frac{\tau}{2} \right) + \tau - \frac{j \tau}{2} \end{array} \right)$$

$$\left( \begin{array}{ccccc} -\frac{1}{2} + \frac{\tau}{2} & \frac{\tau}{2} & \frac{1}{2} & 0 & 0 \\ -\frac{\tau}{2} & -\frac{1}{2} - \frac{3\tau}{2} & 2 + 2 \tau & -\frac{1}{2} - \tau & \kappa (1 + \tau) \\ -\frac{1}{2} & 2 + 2 \tau & -\frac{5}{2} - \frac{7\tau}{2} & 1 + \frac{3\tau}{2} & \kappa (-1 - 2 \tau) \\ 0 & \frac{1}{2} + \tau & -1 - \frac{3\tau}{2} & -\frac{1}{2} + \frac{\tau}{2} & -\kappa \tau \\ 0 & \kappa (-1 - \tau) & \kappa (1 + 2 \tau) & -\kappa \tau & 3 + 6 \tau \end{array} \right)$$

$$\frac{1}{10} (-5 - \sqrt{5})$$

$$\left\{ \kappa \tau, \kappa \left( \frac{1}{5} - \frac{2\tau}{5} \right), \kappa \left( -\frac{3}{5} + \frac{\tau}{5} \right), 0, 1 + 2 \tau \right\}$$

$$\left( \begin{array}{cc} \frac{3}{2} + \frac{j}{2} + \frac{3\tau}{2} + \frac{j\tau}{2} & \kappa \tau \\ -\frac{j \kappa}{2} + \kappa \left( -\frac{1}{2} - \frac{\tau}{2} \right) - \frac{j \kappa \tau}{2} & -\frac{1}{2} + j \left( -\frac{1}{2} - \frac{\tau}{2} \right) - 2 \tau - \frac{j \tau}{2} \end{array} \right)$$

$$\left( \begin{array}{ccccc} -\frac{15}{2} - 13 \tau & \frac{3}{2} + \frac{5\tau}{2} & 1 + \frac{3\tau}{2} & 0 & \kappa (4 + 5 \tau) \\ \frac{5}{2} + \frac{9\tau}{2} & -\frac{1}{2} - \frac{3\tau}{2} & -\frac{1}{2} - \frac{\tau}{2} & \frac{1}{2} - \frac{\tau}{2} & \kappa (-1 - 2 \tau) \\ 2 + \frac{5\tau}{2} & -\frac{1}{2} - \frac{\tau}{2} & -\tau & \frac{1}{2} & \kappa (-1 - \tau) \\ 0 & -\frac{1}{2} + \frac{\tau}{2} & -\frac{1}{2} & -\frac{\tau}{2} & 0 \\ \kappa (-3 - 6 \tau) & \kappa (1 + \tau) & \kappa \tau & 0 & 9 + 14 \tau \end{array} \right)$$

$$\frac{1}{10} (5 - \sqrt{5})$$

5B×5A

$$\left\{ \frac{\mathbf{i}}{2} + \mathbf{j} \left( -\frac{1}{2} + \frac{\tau}{2} \right) - \frac{\tau}{2}, -\frac{1}{2} + \frac{\mathbf{j}}{2} + \frac{\tau}{2} + \frac{\mathbf{i}\tau}{2}, \mathbf{0} \right\}$$

6

spin $\sharp = \mathbf{0}$ 

$$\{ \kappa (2 + 3\tau), \kappa (1 + \tau), \mathbf{0}, \kappa, 5 + 8\tau \}$$

$$\begin{pmatrix} -3 - \frac{9\tau}{2} + \mathbf{i}\tau + \mathbf{j} \left( \frac{1}{2} + \tau \right) + \mathbf{k} \left( \frac{1}{2} + \frac{3\tau}{2} \right) & \frac{\mathbf{k}\kappa}{2} + \kappa (-1 - 2\tau) + \mathbf{j}\kappa \left( \frac{1}{2} + \frac{\tau}{2} \right) - \frac{\mathbf{i}\kappa\tau}{2} \\ \mathbf{i}\kappa \left( -\frac{1}{2} - \tau \right) + \mathbf{j}\kappa \left( -\frac{1}{2} - \frac{\tau}{2} \right) - \mathbf{k}\kappa\tau + \kappa \left( 1 + \frac{3\tau}{2} \right) & \frac{5}{2} + \mathbf{j} (-1 - 2\tau) + \mathbf{i} \left( -\frac{1}{2} - \tau \right) + \mathbf{k} \left( -1 - \frac{\tau}{2} \right) + \frac{9\tau}{2} \\ -\frac{115}{2} - 93\tau & -\frac{45}{2} - \frac{71\tau}{2} & 2 + \frac{5\tau}{2} & -4 - 7\tau & \kappa (26 + 41\tau) \\ -\frac{41}{2} - \frac{67\tau}{2} & -\frac{17}{2} - 13\tau & \tau & -1 - \frac{5\tau}{2} & \kappa (9 + 15\tau) \\ -3 - \frac{11\tau}{2} & -1 - 2\tau & -\frac{1}{2} & -\frac{1}{2} - \frac{\tau}{2} & \kappa (2 + 2\tau) \\ -11 - 18\tau & -4 - \frac{15\tau}{2} & \frac{1}{2} + \frac{\tau}{2} & -\frac{1}{2} - 2\tau & \kappa (5 + 8\tau) \\ \kappa (-25 - 42\tau) & \kappa (-10 - 16\tau) & \kappa (1 + \tau) & \kappa (-2 - 3\tau) & 67 + 108\tau \end{pmatrix}$$

$$-\frac{1}{\sqrt{5}}$$

$$\left\{ \mathbf{0}, \kappa \left( \frac{2}{5} + \frac{\tau}{5} \right), \kappa \left( -\frac{1}{5} - \frac{3\tau}{5} \right), \kappa, 1 + 2\tau \right\}$$

$$\begin{pmatrix} \frac{1}{2} + \mathbf{i} \left( -\frac{1}{2} - \frac{\tau}{2} \right) + \tau - \frac{\mathbf{j}\tau}{2} & \mathbf{k}\kappa \\ \frac{\mathbf{i}\kappa}{2} + \mathbf{k}\kappa \left( \frac{1}{2} - \frac{\tau}{2} \right) - \frac{\mathbf{j}\kappa\tau}{2} & \mathbf{i} \left( -\frac{1}{2} - \tau \right) + \mathbf{j} \left( -\frac{1}{2} - \frac{\tau}{2} \right) - \frac{\tau}{2} \\ -\frac{1}{2} + \frac{\tau}{2} & -\frac{\tau}{2} & -\frac{1}{2} & \mathbf{0} & \mathbf{0} \\ \frac{\tau}{2} & -1 - \frac{\tau}{2} & 1 + \frac{3\tau}{2} & -1 - \frac{5\tau}{2} & \kappa (1 + \tau) \\ \frac{1}{2} & 1 + \frac{3\tau}{2} & -2 - 2\tau & \frac{5}{2} + \frac{7\tau}{2} & \kappa (-1 - 2\tau) \\ \mathbf{0} & -\frac{\tau}{2} & \frac{1}{2} + \frac{\tau}{2} & -\frac{1}{2} - 2\tau & \kappa\tau \\ \mathbf{0} & -\kappa\tau & \kappa (1 + \tau) & \kappa (-1 - 2\tau) & 3 + 6\tau \end{pmatrix}$$

$$\frac{1}{10} (5 + \sqrt{5})$$

$$\left\{ \mathbf{0}, \kappa \left( -\frac{2}{5} + \frac{4\tau}{5} \right), \kappa \left( -\frac{4}{5} - \frac{2\tau}{5} \right), \mathbf{0}, 1 + 2\tau \right\}$$

$$\begin{pmatrix} \frac{1}{2} + \mathbf{i} \left( -\frac{1}{2} - \frac{\tau}{2} \right) + \tau - \frac{\mathbf{j}\tau}{2} & -\frac{\mathbf{j}\kappa}{2} + \mathbf{i}\kappa \left( -\frac{1}{2} + \frac{\tau}{2} \right) + \frac{\mathbf{k}\kappa\tau}{2} \\ -\frac{\mathbf{j}\kappa}{2} + \mathbf{i}\kappa \left( -\frac{1}{2} + \frac{\tau}{2} \right) - \frac{\mathbf{k}\kappa\tau}{2} & \mathbf{i} \left( -\frac{1}{2} - \tau \right) + \mathbf{j} \left( -\frac{1}{2} - \frac{\tau}{2} \right) - \frac{\tau}{2} \\ -\frac{1}{2} + \frac{\tau}{2} & -\frac{\tau}{2} & -\frac{1}{2} & \mathbf{0} & \mathbf{0} \\ \frac{\tau}{2} & -\frac{1}{2} - \frac{3\tau}{2} & 2 + 2\tau & -\frac{1}{2} - \tau & \kappa (1 + \tau) \\ \frac{1}{2} & 2 + 2\tau & -\frac{5}{2} - \frac{7\tau}{2} & 1 + \frac{3\tau}{2} & \kappa (-1 - 2\tau) \\ \mathbf{0} & \frac{1}{2} + \tau & -1 - \frac{3\tau}{2} & -\frac{1}{2} + \frac{\tau}{2} & -\kappa\tau \\ \mathbf{0} & \kappa (-1 - \tau) & \kappa (1 + 2\tau) & -\kappa\tau & 3 + 6\tau \end{pmatrix}$$

$$\frac{1}{10} (5 + \sqrt{5})$$

$$\left\{ \kappa\tau, \kappa \left( \frac{1}{5} - \frac{2\tau}{5} \right), \kappa \left( -\frac{3}{5} + \frac{\tau}{5} \right), \mathbf{0}, 1 + 2\tau \right\}$$

$$\begin{pmatrix} -\frac{1}{2} + \mathbf{i} \left( -\frac{1}{2} - \frac{\tau}{2} \right) - 2\tau - \frac{\mathbf{j}\tau}{2} & -\kappa\tau \\ \frac{\mathbf{j}\kappa}{2} + \kappa \left( \frac{1}{2} + \frac{\tau}{2} \right) + \frac{\mathbf{i}\kappa\tau}{2} & \frac{3}{2} + \frac{\mathbf{j}}{2} + \frac{3\tau}{2} + \frac{\mathbf{i}\tau}{2} \\ -\frac{15}{2} - 13\tau & \frac{5}{2} + \frac{9\tau}{2} & 2 + \frac{5\tau}{2} & \mathbf{0} & \kappa (3 + 6\tau) \\ \frac{3}{2} + \frac{5\tau}{2} & -\frac{1}{2} - \frac{3\tau}{2} & -\frac{1}{2} - \frac{\tau}{2} & \frac{1}{2} - \frac{\tau}{2} & \kappa (-1 - \tau) \\ 1 + \frac{3\tau}{2} & -\frac{1}{2} - \frac{\tau}{2} & -\tau & \frac{1}{2} & -\kappa\tau \\ \mathbf{0} & -\frac{1}{2} + \frac{\tau}{2} & -\frac{1}{2} & -\frac{\tau}{2} & \mathbf{0} \\ \kappa (-4 - 5\tau) & \kappa (1 + 2\tau) & \kappa (1 + \tau) & \mathbf{0} & 9 + 14\tau \end{pmatrix}$$

$$\frac{1}{10} (5 + \sqrt{5})$$



$$1 \times 6 + 6 \times 1$$

$$\left\{ 1, \frac{1}{2} + \mathbb{K} \left( -\frac{1}{2} + \frac{\tau}{2} \right) + \frac{i\tau}{2}, 0 \right\}$$

$$2$$

$$\text{spin}^\sharp = 0$$

$$\{ \kappa(2 + 3\tau), \kappa(1 + \tau), 0, \kappa, 5 + 8\tau \}$$

$$\begin{pmatrix} -\frac{1}{2} - 2\tau + \mathbb{K} \left( \frac{1}{2} + \frac{3\tau}{2} \right) + i \left( 2 + \frac{7\tau}{2} \right) & \kappa \left( -\frac{1}{2} - \frac{3\tau}{2} \right) + \frac{\mathbb{K}\kappa\tau}{2} + i \kappa \left( \frac{1}{2} + \tau \right) \\ \frac{\kappa}{2} + i \kappa \left( -1 - \frac{3\tau}{2} \right) + \mathbb{K} \kappa \left( -\frac{1}{2} - \frac{\tau}{2} \right) & 2 + i(-2 - 3\tau) + \mathbb{K}(-1 - \tau) + 2\tau \end{pmatrix}$$

$$\begin{pmatrix} -\frac{75}{2} - \frac{123\tau}{2} & -\frac{37}{2} - 30\tau & 0 & -7 - \frac{23\tau}{2} & \kappa(17 + 29\tau) \\ -\frac{21}{2} - 17\tau & -5 - 9\tau & \frac{1}{2} - \frac{\tau}{2} & -2 - \frac{7\tau}{2} & \kappa(5 + 8\tau) \\ 0 & -\frac{1}{2} + \frac{\tau}{2} & \frac{1}{2} & -\frac{\tau}{2} & 0 \\ -4 - \frac{13\tau}{2} & -2 - \frac{7\tau}{2} & \frac{\tau}{2} & -\frac{3\tau}{2} & \kappa(2 + 3\tau) \\ \kappa(-17 - 26\tau) & \kappa(-8 - 13\tau) & 0 & \kappa(-3 - 5\tau) & 45 + 72\tau \end{pmatrix}$$

$$-1$$

$$\{0, 0, 0, 0, 1\}$$

$$\begin{pmatrix} 1 & 0 \\ 0 & \frac{1}{2} + \mathbb{K} \left( -\frac{1}{2} + \frac{\tau}{2} \right) + \frac{i\tau}{2} \end{pmatrix}$$

$$\begin{pmatrix} \frac{1}{2} & \frac{\tau}{2} & 0 & -\frac{1}{2} + \frac{\tau}{2} & 0 \\ -\frac{\tau}{2} & \frac{1}{2} & \frac{1}{2} - \frac{\tau}{2} & 0 & 0 \\ 0 & -\frac{1}{2} + \frac{\tau}{2} & \frac{1}{2} & -\frac{\tau}{2} & 0 \\ \frac{1}{2} - \frac{\tau}{2} & 0 & \frac{\tau}{2} & \frac{1}{2} & 0 \\ 0 & 0 & 0 & 0 & 1 \end{pmatrix}$$

$$1$$

1×10A+10B×1

$$\left\{1, \frac{i}{2} + j \left(-\frac{1}{2} + \frac{\tau}{2}\right) + \frac{\tau}{2}, 0\right\}$$

2

$$\text{spin}\sharp = \sqrt{5}$$

$$\{\kappa(2+3\tau), \kappa(1+\tau), 0, \kappa, 5+8\tau\}$$

$$\left( \begin{array}{ccccc} -\frac{5}{2} + i \left(-\frac{3}{2} - 2\tau\right) - \frac{11\tau}{2} + \mathbb{k} \left(2 + \frac{7\tau}{2}\right) & \kappa(-1-2\tau) + i \kappa \left(-1 - \frac{3\tau}{2}\right) + j \kappa \left(\frac{1}{2} + \frac{\tau}{2}\right) + \mathbb{k} \kappa \left(\frac{1}{2} + \tau\right) \\ \mathbb{k} \kappa \left(-1 - \frac{3\tau}{2}\right) + j \kappa \left(-\frac{1}{2} - \frac{\tau}{2}\right) + \kappa \left(\frac{3}{2} + 2\tau\right) & 4 + j \left(-\frac{3}{2} - \frac{5\tau}{2}\right) + \mathbb{k} \left(-\frac{3}{2} - 2\tau\right) + 5\tau + i \left(1 + \frac{3\tau}{2}\right) \end{array} \right)$$

$$\left( \begin{array}{ccccc} -99 - \frac{323\tau}{2} & -\frac{71}{2} - 58\tau & -\frac{3}{2} - \frac{5\tau}{2} & -18 - 29\tau & \kappa(44 + 72\tau) \\ -\frac{81}{2} - 65\tau & -14 - 24\tau & -\frac{1}{2} - \frac{3\tau}{2} & -7 - \frac{23\tau}{2} & \kappa(18 + 29\tau) \\ \frac{3}{2} + \frac{5\tau}{2} & \frac{1}{2} + \frac{3\tau}{2} & \frac{1}{2} - \frac{\tau}{2} & \frac{1}{2} + \frac{\tau}{2} & \kappa(-1 - \tau) \\ -11 - 18\tau & -4 - \frac{13\tau}{2} & -\frac{1}{2} - \frac{\tau}{2} & -\frac{3}{2} - 4\tau & \kappa(5 + 8\tau) \\ \kappa(-45 - 72\tau) & \kappa(-16 - 26\tau) & \kappa(-1 - \tau) & \kappa(-8 - 13\tau) & 117 + 188\tau \end{array} \right)$$

$$\frac{1}{2}(-3 + \sqrt{5})$$

$$\{0, 0, 0, 0, 1\}$$

$$\left( \begin{array}{c} 1 \\ 0 \\ 0 \\ 0 \\ 0 \end{array} \begin{array}{c} 0 \\ \frac{i}{2} + j \left(-\frac{1}{2} + \frac{\tau}{2}\right) + \frac{\tau}{2} \\ \frac{\tau}{2} + \frac{1}{2} \\ \frac{1}{2} - \frac{\tau}{2} \\ \frac{1}{2} - \frac{\tau}{2} \end{array} \right)$$

$$\left( \begin{array}{ccccc} \frac{\tau}{2} & \frac{1}{2} & -\frac{1}{2} + \frac{\tau}{2} & 0 & 0 \\ -\frac{1}{2} & \frac{\tau}{2} & 0 & -\frac{1}{2} + \frac{\tau}{2} & 0 \\ \frac{1}{2} - \frac{\tau}{2} & 0 & \frac{\tau}{2} & -\frac{1}{2} & 0 \\ 0 & \frac{1}{2} - \frac{\tau}{2} & \frac{1}{2} & \frac{\tau}{2} & 0 \\ 0 & 0 & 0 & 0 & 1 \end{array} \right)$$

$$\frac{1}{2}(3 + \sqrt{5})$$

**1×10B+10A×1**

$$\left\{ \mathbf{1}, \frac{1}{2} + \frac{j}{2} - \frac{\tau}{2} + \frac{i\tau}{2}, \mathbf{0} \right\}$$

**2**

$$\text{spin}\sharp = -\sqrt{5}$$

$$\{\kappa(2+3\tau), \kappa(1+\tau), \mathbf{0}, \kappa, 5+8\tau\}$$

$$\begin{pmatrix} \mathbb{K}\left(-\frac{3}{2}-2\tau\right) - \frac{\tau}{2} + i\left(\frac{1}{2} + \frac{3\tau}{2}\right) & \mathbb{K}\kappa\left(-1 - \frac{\tau}{2}\right) - \frac{\kappa\tau}{2} + \frac{i\kappa\tau}{2} - \frac{j\kappa\tau}{2} \\ \frac{\kappa}{2} + i\kappa\left(-\frac{1}{2} - \frac{\tau}{2}\right) + \frac{j\kappa\tau}{2} + \mathbb{K}\kappa\tau & \mathbf{1} + i\left(-\frac{1}{2} - \tau\right) + \tau + \mathbb{K}\left(\frac{1}{2} + \frac{3\tau}{2}\right) + j\left(\mathbf{1} + \frac{3\tau}{2}\right) \end{pmatrix}$$

$$\begin{pmatrix} -\frac{29}{2} - 23\tau & -\frac{13}{2} - \frac{23\tau}{2} & \mathbf{1} + \frac{3\tau}{2} & \mathbf{0} & \kappa(6+11\tau) \\ -\frac{9}{2} - \frac{13\tau}{2} & -2-3\tau & \mathbf{1} + \frac{\tau}{2} & \frac{1}{2} & \kappa(2+3\tau) \\ -1 - \frac{3\tau}{2} & -1 - \frac{\tau}{2} & \frac{\tau}{2} & -\frac{\tau}{2} & \kappa\tau \\ -4-7\tau & -\frac{3}{2}-3\tau & \frac{\tau}{2} & \frac{1}{2} - \frac{\tau}{2} & \kappa(2+3\tau) \\ \kappa(-7-10\tau) & \kappa(-3-5\tau) & \kappa\tau & \mathbf{0} & 17+28\tau \end{pmatrix}$$

$$\frac{1}{2}(-3-\sqrt{5})$$

$$\{\mathbf{0}, \mathbf{0}, \mathbf{0}, \mathbf{0}, \mathbf{1}\}$$

$$\begin{pmatrix} \mathbf{1} & \mathbf{0} \\ \mathbf{0} & \frac{1}{2} + \frac{j}{2} - \frac{\tau}{2} + \frac{i\tau}{2} \end{pmatrix}$$

$$\begin{pmatrix} \frac{1}{2} - \frac{\tau}{2} & \frac{\tau}{2} & \frac{1}{2} & \mathbf{0} & \mathbf{0} \\ -\frac{\tau}{2} & \frac{1}{2} - \frac{\tau}{2} & \mathbf{0} & \frac{1}{2} & \mathbf{0} \\ -\frac{1}{2} & \mathbf{0} & \frac{1}{2} - \frac{\tau}{2} & -\frac{\tau}{2} & \mathbf{0} \\ \mathbf{0} & -\frac{1}{2} & \frac{\tau}{2} & \frac{1}{2} - \frac{\tau}{2} & \mathbf{0} \\ \mathbf{0} & \mathbf{0} & \mathbf{0} & \mathbf{0} & \mathbf{1} \end{pmatrix}$$

$$\frac{1}{2}(3-\sqrt{5})$$

5A×10B+10A×5B

$$\left\{ \frac{\mathfrak{j}}{2} + \mathfrak{j} \left( -\frac{1}{2} + \frac{\tau}{2} \right) + \frac{\tau}{2}, \frac{\mathfrak{j}}{2} + \mathfrak{j} \left( -\frac{1}{2} + \frac{\tau}{2} \right) - \frac{\tau}{2}, \mathbf{0} \right\}$$

12

$$\text{spin}\sharp = -2\sqrt{5}$$

$$\{ \kappa (2+3\tau), \kappa (1+\tau), \mathbf{0}, \kappa, 5+8\tau \}$$

$$\left( \begin{array}{ccccc} \frac{3}{2} + \mathfrak{j} \left( -2 - \frac{5\tau}{2} \right) + \frac{5\tau}{2} + \mathfrak{j} \left( \frac{1}{2} + \tau \right) + \mathbb{k} (4+7\tau) & \mathfrak{j} \kappa \left( -\frac{1}{2} - \frac{\tau}{2} \right) + \kappa \left( \frac{1}{2} + \tau \right) + \mathfrak{j} \kappa \left( 1 + \frac{3\tau}{2} \right) + \mathbb{k} \kappa & & & \\ \mathbb{k} \kappa (-2-2\tau) + \mathfrak{j} \kappa \left( -1 - \frac{3\tau}{2} \right) + \kappa \left( -\frac{1}{2} - \tau \right) + \mathfrak{j} \kappa \left( \frac{1}{2} + \frac{3\tau}{2} \right) & -\frac{3}{2} + \mathfrak{j} \left( -\frac{7}{2} - 6\tau \right) + \mathbb{k} (-3-4\tau) - \frac{5\tau}{2} + \mathfrak{j} (1 & & & \\ -\frac{289}{2} - 233\tau & -\frac{113}{2} - \frac{183\tau}{2} & 1 + \frac{3\tau}{2} & -22 - 36\tau & \kappa (64 + 105\tau) \\ -\frac{111}{2} - \frac{179\tau}{2} & -22 - \frac{69\tau}{2} & \frac{1}{2} + \tau & -8 - 14\tau & \kappa (25 + 40\tau) \\ 2 + \frac{5\tau}{2} & \frac{1}{2} + \tau & -\frac{1}{2} + \frac{\tau}{2} & \mathbf{0} & \kappa (-1 - \tau) \\ -22 - 36\tau & -8 - 14\tau & \mathbf{0} & -3 - 6\tau & \kappa (10 + 16\tau) \\ \kappa (-65 - 104\tau) & \kappa (-25 - 41\tau) & \kappa \tau & \kappa (-10 - 16\tau) & 169 + 274\tau \end{array} \right)$$

$$\frac{1}{4} (1 + \sqrt{5})$$

$$\left\{ \kappa (1+\tau), \frac{\kappa}{2}, \frac{\kappa\tau}{2}, \kappa \left( \frac{1}{2} - \frac{\tau}{2} \right), 2+3\tau \right\}$$

$$\left( \begin{array}{ccccc} -\frac{1}{2} + \frac{\mathfrak{j}}{2} - \tau + \mathfrak{j} \left( \frac{1}{2} + \tau \right) + \mathbb{k} \left( \frac{3}{2} + 2\tau \right) & \mathbb{k} \kappa \left( 1 + \frac{\tau}{2} \right) - \frac{\kappa\tau}{2} - \frac{\mathfrak{j}\kappa\tau}{2} + \frac{\mathfrak{j}\kappa\tau}{2} & & & \\ \frac{\mathfrak{j}\kappa}{2} + \mathfrak{j} \kappa \left( -\frac{1}{2} - \frac{\tau}{2} \right) + \frac{\kappa\tau}{2} - \mathbb{k} \kappa \tau & \frac{1}{2} + \mathbb{k} \left( -\frac{1}{2} - \frac{3\tau}{2} \right) + \mathfrak{j} (-1 - \tau) + \tau + \mathfrak{j} \left( 1 + \frac{3\tau}{2} \right) & & & \\ -\frac{29}{2} - 23\tau & -\frac{5}{2} - \frac{9\tau}{2} & -6 - \frac{19\tau}{2} & 3 + 4\tau & \kappa (6 + 11\tau) \\ -\frac{3}{2} - \frac{5\tau}{2} & -\frac{1}{2} & -1 - \tau & 1 + \frac{\tau}{2} & \kappa (1 + \tau) \\ -5 - \frac{17\tau}{2} & -1 - \tau & -\frac{5}{2} - 3\tau & \frac{1}{2} + \frac{3\tau}{2} & \kappa (2 + 4\tau) \\ 3 + 4\tau & 1 + \frac{\tau}{2} & \frac{1}{2} + \frac{3\tau}{2} & -\frac{1}{2} - \tau & \kappa (-1 - 2\tau) \\ \kappa (-7 - 10\tau) & \kappa (-1 - 2\tau) & \kappa (-3 - 4\tau) & \kappa (1 + 2\tau) & 17 + 28\tau \end{array} \right)$$

$$\frac{1}{4} (-1 - \sqrt{5})$$

$$\left\{ \kappa (1+\tau), \frac{\kappa}{2}, \frac{\kappa\tau}{2}, \kappa \left( -\frac{1}{2} + \frac{\tau}{2} \right), 2+3\tau \right\}$$

$$\left( \begin{array}{ccccc} -\frac{1}{2} + \mathfrak{j} (-1 - \tau) - \tau + \mathbb{k} \left( \frac{1}{2} + \frac{3\tau}{2} \right) + \mathfrak{j} \left( 1 + \frac{3\tau}{2} \right) & \frac{\mathfrak{j}\kappa}{2} + \mathfrak{j} \kappa \left( -\frac{1}{2} - \frac{\tau}{2} \right) - \frac{\kappa\tau}{2} + \mathbb{k} \kappa \tau & & & \\ \mathbb{k} \kappa (-1 - \frac{\tau}{2}) + \frac{\kappa\tau}{2} - \frac{\mathfrak{j}\kappa\tau}{2} + \frac{\mathfrak{j}\kappa\tau}{2} & \frac{1}{2} + \frac{\mathfrak{j}}{2} + \mathbb{k} \left( -\frac{3}{2} - 2\tau \right) + \tau + \mathfrak{j} \left( \frac{1}{2} + \tau \right) & & & \\ -\frac{29}{2} - 23\tau & -\frac{5}{2} - \frac{9\tau}{2} & -6 - \frac{19\tau}{2} & -3 - 4\tau & \kappa (6 + 11\tau) \\ -\frac{3}{2} - \frac{5\tau}{2} & -\frac{1}{2} & -1 - \tau & -1 - \frac{\tau}{2} & \kappa (1 + \tau) \\ -5 - \frac{17\tau}{2} & -1 - \tau & -\frac{5}{2} - 3\tau & -\frac{1}{2} - \frac{3\tau}{2} & \kappa (2 + 4\tau) \\ -3 - 4\tau & -1 - \frac{\tau}{2} & -\frac{1}{2} - \frac{3\tau}{2} & -\frac{1}{2} - \tau & \kappa (1 + 2\tau) \\ \kappa (-7 - 10\tau) & \kappa (-1 - 2\tau) & \kappa (-3 - 4\tau) & \kappa (-1 - 2\tau) & 17 + 28\tau \end{array} \right)$$

$$\frac{1}{4} (-1 - \sqrt{5})$$

$$\left\{ \kappa (1+\tau), \frac{\kappa\tau}{2}, \kappa \left( -\frac{1}{2} + \frac{\tau}{2} \right), -\frac{\kappa}{2}, 2+3\tau \right\}$$

$$\left( \begin{array}{ccccc} -\frac{1}{2} + \mathfrak{j} \left( -\frac{1}{2} - \frac{\tau}{2} \right) - \tau + \mathfrak{j} \left( 1 + \frac{5\tau}{2} \right) & -\frac{\mathbb{k}\kappa}{2} + \mathfrak{j} \kappa \left( -\frac{1}{2} - \frac{\tau}{2} \right) - \frac{\kappa\tau}{2} + \mathfrak{j} \kappa \tau & & & \\ \mathfrak{j} \kappa \left( -1 - \frac{\tau}{2} \right) + \frac{\kappa\tau}{2} + \frac{\mathfrak{j}\kappa\tau}{2} + \frac{\mathbb{k}\kappa\tau}{2} & \frac{1}{2} + \mathfrak{j} (-1 - \tau) + \tau + \mathbb{k} \left( \frac{1}{2} + \frac{3\tau}{2} \right) + \mathfrak{j} \left( 1 + \frac{3\tau}{2} \right) & & & \\ -\frac{29}{2} - 23\tau & -\frac{11}{2} - \frac{17\tau}{2} & -2 - \frac{5\tau}{2} & 4 + 7\tau & \kappa (6 + 11\tau) \\ -\frac{9}{2} - \frac{13\tau}{2} & -2 - 2\tau & -\frac{\tau}{2} & \frac{3}{2} + 2\tau & \kappa (2 + 3\tau) \\ -1 - \frac{3\tau}{2} & -\frac{\tau}{2} & -\frac{\tau}{2} & 1 + \frac{\tau}{2} & \kappa \tau \\ 4 + 7\tau & \frac{3}{2} + 2\tau & 1 + \frac{\tau}{2} & -\frac{3}{2} - \frac{3\tau}{2} & \kappa (-2 - 3\tau) \\ \kappa (-7 - 10\tau) & \kappa (-2 - 4\tau) & \kappa (-1 - \tau) & \kappa (2 + 3\tau) & 17 + 28\tau \end{array} \right)$$

$$\frac{1}{4} (-1 - \sqrt{5})$$

3×4+4×3

$$\left\{ \mathbf{i}, -\frac{1}{2} + \mathbb{K} \left( -\frac{1}{2} + \frac{\tau}{2} \right) + \frac{\mathbf{i}\tau}{2}, \mathbf{0} \right\}$$

2

spin $\sharp = \mathbf{0}$

$$\{ \mathcal{K} (2 + 3 \tau), \mathcal{K} (1 + \tau), \mathbf{0}, \mathcal{K}, 5 + 8 \tau \}$$

$$\begin{pmatrix} -\frac{3}{2} - 2 \tau + \mathbb{K} (1 + 3 \tau) + \mathbf{j} \left( 2 + \frac{7\tau}{2} \right) + \mathbf{i} \left( \frac{5}{2} + \frac{9\tau}{2} \right) & \mathcal{K} \left( -1 - \frac{3\tau}{2} \right) + \frac{\mathbb{K} \mathcal{K} \tau}{2} + \mathbf{i} \mathcal{K} \left( 1 + \frac{3\tau}{2} \right) + \mathbf{j} \mathcal{K} \left( 1 + \frac{3\tau}{2} \right) \\ \mathbf{i} \mathcal{K} \left( -\frac{3}{2} - 2 \tau \right) + \mathbf{j} \mathcal{K} \left( -1 - \frac{3\tau}{2} \right) + \mathbb{K} \mathcal{K} \left( -\frac{1}{2} - \frac{\tau}{2} \right) & 1 + \mathbf{i} \left( -\frac{7}{2} - 5 \tau \right) + \mathbf{j} \left( -2 - \frac{7\tau}{2} \right) + \mathbb{K} \left( -\frac{1}{2} + \frac{\tau}{2} \right) + 2 \tau \end{pmatrix}$$

$$\begin{pmatrix} -99 - \frac{323\tau}{2} & -\frac{77}{2} - 62\tau & \frac{5}{2} + \frac{9\tau}{2} & -11 - 18\tau & \mathcal{K} (44 + 72 \tau) \\ -\frac{81}{2} - 65\tau & -16 - 25\tau & \frac{1}{2} + \frac{3\tau}{2} & -4 - \frac{15\tau}{2} & \mathcal{K} (18 + 29 \tau) \\ -\frac{3}{2} - \frac{5\tau}{2} & -\frac{1}{2} - \frac{3\tau}{2} & -\frac{1}{2} + \frac{\tau}{2} & -\frac{1}{2} - \frac{\tau}{2} & \mathcal{K} (1 + \tau) \\ -11 - 18\tau & -4 - \frac{15\tau}{2} & \frac{1}{2} + \frac{\tau}{2} & -\frac{1}{2} - 2\tau & \mathcal{K} (5 + 8 \tau) \\ \mathcal{K} (-45 - 72 \tau) & \mathcal{K} (-17 - 28 \tau) & \mathcal{K} (1 + 2 \tau) & \mathcal{K} (-5 - 8 \tau) & 117 + 188 \tau \end{pmatrix}$$

-1

$$\{\mathbf{0}, \mathbf{0}, \mathbf{0}, \mathbf{0}, 1\}$$

$$\begin{pmatrix} \mathbf{i} & \mathbf{0} \\ \mathbf{0} & -\frac{1}{2} + \mathbb{K} \left( -\frac{1}{2} + \frac{\tau}{2} \right) + \frac{\mathbf{i}\tau}{2} \end{pmatrix}$$

$$\begin{pmatrix} \frac{\tau}{2} & \frac{1}{2} & -\frac{1}{2} + \frac{\tau}{2} & \mathbf{0} & \mathbf{0} \\ -\frac{1}{2} & \frac{\tau}{2} & \mathbf{0} & -\frac{1}{2} + \frac{\tau}{2} & \mathbf{0} \\ -\frac{1}{2} + \frac{\tau}{2} & \mathbf{0} & -\frac{\tau}{2} & \frac{1}{2} & \mathbf{0} \\ \mathbf{0} & -\frac{1}{2} + \frac{\tau}{2} & -\frac{1}{2} & -\frac{\tau}{2} & \mathbf{0} \\ \mathbf{0} & \mathbf{0} & \mathbf{0} & \mathbf{0} & 1 \end{pmatrix}$$

1

$$3 \times 5A + 5B \times 3$$

$$\left\{ -\frac{1}{2} + \mathbb{K} \left( -\frac{1}{2} + \frac{\tau}{2} \right) + \frac{i\tau}{2}, -\frac{1}{2} + \frac{j}{2} + \frac{\tau}{2} + \frac{i\tau}{2}, \emptyset \right\}$$

$$2$$

$$\text{spin}\sharp = -\sqrt{5}$$

$$\{\kappa(2+3\tau), \kappa(1+\tau), \emptyset, \kappa, 5+8\tau\}$$

$$\left( \begin{array}{ccccc} -1 + \mathbb{K} \left( -\frac{5}{2} - 3\tau \right) + i \left( -\frac{3}{2} - \frac{3\tau}{2} \right) - \frac{3\tau}{2} & \mathbb{K} \kappa \left( -\frac{1}{2} - \frac{3\tau}{2} \right) + i \kappa \left( -\frac{1}{2} - \tau \right) - \frac{j\kappa\tau}{2} & & & \\ i \kappa \left( \frac{1}{2} + \frac{\tau}{2} \right) + \frac{j\kappa\tau}{2} + \kappa \left( \frac{1}{2} + \tau \right) + \mathbb{K} \kappa (1+\tau) & \frac{1}{2} + \tau + j \left( 1 + \frac{3\tau}{2} \right) + i \left( \frac{3}{2} + \frac{5\tau}{2} \right) + \mathbb{K} (1+3\tau) & & & \\ -\frac{75}{2} - \frac{123\tau}{2} & -17 - 27\tau & 2 + \frac{5\tau}{2} & -\frac{17}{2} - 14\tau & \kappa(18+28\tau) \\ -\frac{23}{2} - 19\tau & -\frac{11}{2} - 8\tau & \frac{1}{2} + \tau & -\frac{5}{2} - 5\tau & \kappa(5+9\tau) \\ 3+4\tau & 1 + \frac{3\tau}{2} & -\frac{1}{2} + \frac{\tau}{2} & \frac{1}{2} + \tau & \kappa(-1-2\tau) \\ -4 - \frac{13\tau}{2} & -\frac{3}{2} - \frac{7\tau}{2} & \emptyset & -\frac{1}{2} - 2\tau & \kappa(2+3\tau) \\ \kappa(-16-27\tau) & \kappa(-7-12\tau) & \kappa(1+\tau) & \kappa(-4-6\tau) & 45+72\tau \end{array} \right)$$

$$\frac{1}{2}(-1-\sqrt{5})$$

$$\{\emptyset, \emptyset, \emptyset, \emptyset, 1\}$$

$$\left( \begin{array}{cccc} -\frac{1}{2} + \mathbb{K} \left( -\frac{1}{2} + \frac{\tau}{2} \right) + \frac{i\tau}{2} & & & \emptyset \\ & \emptyset & & -\frac{1}{2} + \frac{j}{2} + \frac{\tau}{2} + \frac{i\tau}{2} \\ \frac{1}{2} & -\frac{1}{2} & -\frac{1}{2} & -\frac{1}{2} & \emptyset \\ \frac{\tau}{2} & \frac{1}{2} & -\frac{1}{2} + \frac{\tau}{2} & \emptyset & \emptyset \\ \emptyset & \frac{1}{2} & -\frac{\tau}{2} & -\frac{1}{2} + \frac{\tau}{2} & \emptyset \\ \frac{1}{2} - \frac{\tau}{2} & \frac{1}{2} & \emptyset & -\frac{\tau}{2} & \emptyset \\ \emptyset & \emptyset & \emptyset & \emptyset & 1 \end{array} \right)$$

$$\frac{1}{2}(1-\sqrt{5})$$

$$3 \times 5B + 5A \times 3$$

$$\left\{ -\frac{1}{2} + \frac{j}{2} + \frac{\tau}{2} + \frac{i\tau}{2}, -\frac{1}{2} + \mathbb{k} \left( -\frac{1}{2} + \frac{\tau}{2} \right) + \frac{i\tau}{2}, \mathbf{0} \right\}$$

2

$$\text{spin}\sharp = \sqrt{5}$$

$$\{\kappa(2+3\tau), \kappa(1+\tau), \mathbf{0}, \kappa, 5+8\tau\}$$

$$\left( \begin{array}{ccccc} \frac{1}{2} + \mathbb{k} \left( -1 - \frac{\tau}{2} \right) + j \left( -\frac{1}{2} - \frac{\tau}{2} \right) + \tau + i(2+4\tau) & -\frac{\mathbb{k}\kappa}{2} + j\kappa \left( -\frac{1}{2} - \frac{\tau}{2} \right) + i\kappa \left( 1 + \frac{3\tau}{2} \right) & & & \\ i\kappa(-1-\tau) + \kappa \left( -\frac{1}{2} - \tau \right) + j\kappa \left( \frac{1}{2} + \frac{\tau}{2} \right) + \frac{\mathbb{k}\kappa\tau}{2} & -1 + i(-2-3\tau) + \mathbb{k} \left( -\frac{1}{2} + \frac{\tau}{2} \right) - \frac{3\tau}{2} + j \left( \frac{3}{2} + 2\tau \right) & & & \end{array} \right)$$

$$\left( \begin{array}{ccccc} -\frac{75}{2} - \frac{123\tau}{2} & -11 - 17\tau & 1 + \frac{3\tau}{2} & -\frac{13}{2} - 11\tau & \kappa(16+27\tau) \\ -\frac{35}{2} - 28\tau & -\frac{11}{2} - 8\tau & \frac{1}{2} + \tau & -\frac{5}{2} - 5\tau & \kappa(8+12\tau) \\ 3+4\tau & 1 + \frac{3\tau}{2} & -\frac{1}{2} + \frac{\tau}{2} & \frac{1}{2} + \tau & \kappa(-1-2\tau) \\ -7 - \frac{23\tau}{2} & -\frac{3}{2} - \frac{7\tau}{2} & \mathbf{0} & -\frac{1}{2} - 2\tau & \kappa(3+5\tau) \\ \kappa(-18-28\tau) & \kappa(-5-8\tau) & \kappa\tau & \kappa(-3-5\tau) & 45+72\tau \end{array} \right)$$

$$\frac{1}{2} (1 + \sqrt{5})$$

$$\{\mathbf{0}, \mathbf{0}, \mathbf{0}, \mathbf{0}, 1\}$$

$$\left( \begin{array}{ccccc} -\frac{1}{2} + \frac{j}{2} + \frac{\tau}{2} + \frac{i\tau}{2} & & & & \mathbf{0} \\ & \mathbf{0} & & & -\frac{1}{2} + \mathbb{k} \left( -\frac{1}{2} + \frac{\tau}{2} \right) + \frac{i\tau}{2} \end{array} \right)$$

$$\left( \begin{array}{ccccc} \frac{1}{2} & \frac{1}{2} & \frac{1}{2} & \frac{1}{2} & \mathbf{0} \\ -\frac{\tau}{2} & \frac{1}{2} & -\frac{1}{2} + \frac{\tau}{2} & \mathbf{0} & \mathbf{0} \\ \mathbf{0} & \frac{1}{2} & -\frac{\tau}{2} & -\frac{1}{2} + \frac{\tau}{2} & \mathbf{0} \\ -\frac{1}{2} + \frac{\tau}{2} & \frac{1}{2} & \mathbf{0} & -\frac{\tau}{2} & \mathbf{0} \\ \mathbf{0} & \mathbf{0} & \mathbf{0} & \mathbf{0} & 1 \end{array} \right)$$

$$\frac{1}{2} (-1 + \sqrt{5})$$

4×5A+5B×4

$$\left\{ \mathbf{i}, -\frac{1}{2} + \frac{\mathbf{j}}{2} + \frac{\tau}{2} + \frac{\mathbf{i}\tau}{2}, \mathbf{0} \right\}$$

2

$$\text{spin}\sharp = -\sqrt{5}$$

$$\{\kappa(2+3\tau), \kappa(1+\tau), \mathbf{0}, \kappa, 5+8\tau\}$$

$$\left( \begin{array}{ccccc} -2 + \mathbb{k} \left( -1 - \frac{\tau}{2} \right) - \frac{7\tau}{2} + \mathbf{i} \left( 1 + \frac{5\tau}{2} \right) + \mathbf{j} \left( 2 + \frac{7\tau}{2} \right) & \kappa \left( -1 - \frac{3\tau}{2} \right) + \mathbb{k} \kappa \left( -\frac{1}{2} - \tau \right) + \mathbf{i} \kappa \left( \frac{1}{2} + \frac{\tau}{2} \right) + \mathbf{j} \kappa (1 + \\ \mathbf{i} \kappa \left( -1 - \frac{3\tau}{2} \right) + \mathbf{j} \kappa (-1 - \tau) + \mathbb{k} \kappa \left( \frac{1}{2} + \frac{\tau}{2} \right) + \kappa \left( \frac{1}{2} + \tau \right) & 2 + \mathbf{i} (-2 - 3\tau) + \mathbf{j} (-1 - 2\tau) + 3\tau + \mathbb{k} (1 + 3\tau) \\ -7\mathbf{0} - \frac{229\tau}{2} & -\frac{47}{2} - \frac{75\tau}{2} & 3 + 4\tau & -\frac{17}{2} - 14\tau & \kappa(31 + 50\tau) \\ -\frac{53}{2} - \frac{85\tau}{2} & -9 - 14\tau & 1 + \frac{3\tau}{2} & -\frac{5}{2} - 5\tau & \kappa(11 + 19\tau) \\ -4 - 7\tau & -2 - \frac{5\tau}{2} & -\frac{1}{2} + \frac{\tau}{2} & -\frac{1}{2} - \tau & \kappa(2 + 3\tau) \\ -\frac{17}{2} - 14\tau & -\frac{5}{2} - 5\tau & \frac{1}{2} + \tau & -\frac{1}{2} - 2\tau & \kappa(4 + 6\tau) \\ \kappa(-31 - 51\tau) & \kappa(-10 - 17\tau) & \kappa(1 + 2\tau) & \kappa(-4 - 6\tau) & 81 + 130\tau \end{array} \right)$$

$$\frac{1}{2} (1 - \sqrt{5})$$

$$\{\mathbf{0}, \mathbf{0}, \mathbf{0}, \mathbf{0}, 1\}$$

$$\left( \begin{array}{c} \mathbf{i} \quad \mathbf{0} \\ \mathbf{0} \quad -\frac{1}{2} + \frac{\mathbf{j}}{2} + \frac{\tau}{2} + \frac{\mathbf{i}\tau}{2} \end{array} \right)$$

$$\left( \begin{array}{ccccc} \frac{\tau}{2} & \frac{1}{2} - \frac{\tau}{2} & \mathbf{0} & -\frac{1}{2} & \mathbf{0} \\ -\frac{1}{2} + \frac{\tau}{2} & \frac{\tau}{2} & \frac{1}{2} & \mathbf{0} & \mathbf{0} \\ \mathbf{0} & \frac{1}{2} & -\frac{\tau}{2} & \frac{1}{2} - \frac{\tau}{2} & \mathbf{0} \\ -\frac{1}{2} & \mathbf{0} & -\frac{1}{2} + \frac{\tau}{2} & -\frac{\tau}{2} & \mathbf{0} \\ \mathbf{0} & \mathbf{0} & \mathbf{0} & \mathbf{0} & 1 \end{array} \right)$$

$$\frac{1}{2} (-1 - \sqrt{5})$$



4×5B+5A×4

$$\left\{-\frac{1}{2}+\frac{j}{2}+\frac{\tau}{2}+\frac{j\tau}{2}, j, 0\right\}$$

2

$$\text{spin}\sharp = \sqrt{5}$$

$$\{\kappa(2+3\tau), \kappa(1+\tau), 0, \kappa, 5+8\tau\}$$

$$\begin{pmatrix} 2+j\left(-\frac{3}{2}-\frac{3\tau}{2}\right)+\mathbb{k}\left(-1-\frac{\tau}{2}\right)+3\tau+j\left(\frac{3}{2}+3\tau\right) & \mathbb{k}\kappa\left(-\frac{1}{2}-\frac{\tau}{2}\right)+j\kappa\left(\frac{1}{2}+\tau\right)+\kappa\left(1+\frac{3\tau}{2}\right) \\ \kappa\left(-\frac{1}{2}-\tau\right)+j\kappa\left(-\frac{1}{2}-\tau\right)+j\kappa\left(\frac{1}{2}+\tau\right)+\mathbb{k}\kappa\left(\frac{1}{2}+\tau\right) & -2+j\left(-\frac{1}{2}-\frac{3\tau}{2}\right)-\frac{7\tau}{2}+j\left(\frac{1}{2}+\tau\right)+\mathbb{k}\left(1+3\tau\right) \end{pmatrix}$$

$$\begin{pmatrix} -48-\frac{157\tau}{2} & -\frac{45}{2}-\frac{71\tau}{2} & 3+4\tau & -\frac{13}{2}-11\tau & \kappa(22+36\tau) \\ -\frac{39}{2}-\frac{61\tau}{2} & -9-14\tau & 1+\frac{3\tau}{2} & -\frac{5}{2}-5\tau & \kappa(9+14\tau) \\ -4-7\tau & -2-\frac{5\tau}{2} & -\frac{1}{2}+\frac{\tau}{2} & -\frac{1}{2}-\tau & \kappa(2+3\tau) \\ -\frac{13}{2}-11\tau & -\frac{5}{2}-5\tau & \frac{1}{2}+\tau & -\frac{1}{2}-2\tau & \kappa(3+5\tau) \\ \kappa(-22-35\tau) & \kappa(-10-16\tau) & \kappa(1+2\tau) & \kappa(-3-5\tau) & 59+94\tau \end{pmatrix}$$

$$\frac{1}{2}(-1+\sqrt{5})$$

$$\{0, 0, 0, 0, 1\}$$

$$\begin{pmatrix} -\frac{1}{2}+\frac{j}{2}+\frac{\tau}{2}+\frac{j\tau}{2} & 0 \\ 0 & j \end{pmatrix}$$

$$\begin{pmatrix} \frac{\tau}{2} & -\frac{1}{2}+\frac{\tau}{2} & 0 & \frac{1}{2} & 0 \\ \frac{1}{2}-\frac{\tau}{2} & \frac{\tau}{2} & \frac{1}{2} & 0 & 0 \\ 0 & \frac{1}{2} & -\frac{\tau}{2} & \frac{1}{2}-\frac{\tau}{2} & 0 \\ \frac{1}{2} & 0 & -\frac{1}{2}+\frac{\tau}{2} & -\frac{\tau}{2} & 0 \\ 0 & 0 & 0 & 0 & 1 \end{pmatrix}$$

$$\frac{1}{2}(1+\sqrt{5})$$

3×10A+10B×3

$$\left\{ \frac{1}{2} + \frac{j}{2} - \frac{\tau}{2} + \frac{i\tau}{2}, -\frac{1}{2} + \mathbb{k} \left( -\frac{1}{2} + \frac{\tau}{2} \right) + \frac{i\tau}{2}, \mathbf{0} \right\}$$

2

$$\text{spin}\sharp = \sqrt{5}$$

$$\left( \kappa (2 + 3 \tau), \kappa (1 + \tau), \mathbf{0}, \kappa, 5 + 8 \tau \right)$$

$$\left( -\frac{7}{2} + \mathbb{k} \left( -1 - \frac{\tau}{2} \right) + j \left( -\frac{1}{2} - \frac{\tau}{2} \right) - 5 \tau + i (2 + 4 \tau) \quad \kappa \left( -\frac{3}{2} - \frac{5\tau}{2} \right) + j \kappa \left( -\frac{1}{2} - \frac{\tau}{2} \right) + \mathbb{k} \kappa \left( -\frac{1}{2} - \frac{\tau}{2} \right) + i \kappa \left( \frac{1}{2} + \frac{\tau}{2} \right) \right. \\ \left. i \kappa \left( -\frac{3}{2} - 2 \tau \right) + j \kappa \left( \frac{1}{2} + \frac{\tau}{2} \right) + \kappa \left( 1 + \frac{3\tau}{2} \right) \quad 3 + i (-2 - 3 \tau) + \mathbb{k} \left( -\frac{1}{2} + \frac{\tau}{2} \right) + \frac{11\tau}{2} + j \left( \frac{3}{2} + 2 \tau \right) \right)$$

$$\left( \begin{array}{ccccc} -99 - \frac{323\tau}{2} & -41 - \frac{131\tau}{2} & 1 + \frac{3\tau}{2} & -18 - \frac{59\tau}{2} & \kappa (45 + 73 \tau) \\ -\frac{69}{2} - \frac{111\tau}{2} & -\frac{29}{2} - 23 \tau & \tau & -6 - \frac{21\tau}{2} & \kappa (16 + 25 \tau) \\ 3 + 4 \tau & \frac{3}{2} + \frac{3\tau}{2} & -\frac{1}{2} & \frac{\tau}{2} & \kappa (-1 - 2 \tau) \\ -\frac{27}{2} - 22 \tau & -5 - 9 \tau & \frac{1}{2} + \frac{\tau}{2} & -2 - \frac{9\tau}{2} & \kappa (6 + 10 \tau) \\ \kappa (-44 - 71 \tau) & \kappa (-18 - 29 \tau) & \kappa \tau & \kappa (-8 - 13 \tau) & 117 + 188 \tau \end{array} \right)$$

$$\frac{1}{2} (-3 + \sqrt{5})$$

$$\{\mathbf{0}, \mathbf{0}, \mathbf{0}, \mathbf{0}, 1\}$$

$$\left( \begin{array}{ccccc} \frac{1}{2} + \frac{j}{2} - \frac{\tau}{2} + \frac{i\tau}{2} & & & & \mathbf{0} \\ & \mathbf{0} & & & -\frac{1}{2} + \mathbb{k} \left( -\frac{1}{2} + \frac{\tau}{2} \right) + \frac{i\tau}{2} \end{array} \right)$$

$$\left( \begin{array}{ccccc} \frac{\tau}{2} & \mathbf{0} & \frac{1}{2} & -\frac{1}{2} + \frac{\tau}{2} & \mathbf{0} \\ \frac{1}{2} - \frac{\tau}{2} & \frac{\tau}{2} & \frac{1}{2} & \mathbf{0} & \mathbf{0} \\ \mathbf{0} & -\frac{1}{2} + \frac{\tau}{2} & -\frac{1}{2} & \frac{\tau}{2} & \mathbf{0} \\ \frac{1}{2} & \frac{1}{2} & -\frac{1}{2} & -\frac{1}{2} & \mathbf{0} \\ \mathbf{0} & \mathbf{0} & \mathbf{0} & \mathbf{0} & 1 \end{array} \right)$$

$$\frac{1}{2} (3 + \sqrt{5})$$

$3 \times 10B + 10A \times 3$

$$\left\{ \frac{i}{2} + j \left( -\frac{1}{2} + \frac{\tau}{2} \right) + \frac{\tau}{2}, -\frac{1}{2} + k \left( -\frac{1}{2} + \frac{\tau}{2} \right) + \frac{i\tau}{2}, 0 \right\}$$

2

$$\text{spin}\# = -\sqrt{5}$$

$$\{ \kappa (2 + 3\tau), \kappa (1 + \tau), 0, \kappa, 5 + 8\tau \}$$

$$\begin{pmatrix} -\frac{1}{2} - \tau + j \left( \frac{1}{2} + \tau \right) + i \left( \frac{3}{2} + 3\tau \right) + k \left( \frac{5}{2} + 5\tau \right) & \kappa \left( -\frac{1}{2} - \tau \right) + i \kappa \left( \frac{1}{2} + \tau \right) + j \kappa \left( \frac{1}{2} + \tau \right) + k \kappa \left( \frac{1}{2} + 2\tau \right) \\ k \kappa \left( -\frac{3}{2} - \frac{3\tau}{2} \right) + i \kappa (-1 - \tau) + j \kappa \left( -\frac{1}{2} - \tau \right) - \frac{\kappa\tau}{2} & \frac{1}{2} + j \left( -2 - \frac{7\tau}{2} \right) + k \left( -\frac{5}{2} - 3\tau \right) + i (-2 - 3\tau) + \frac{\tau}{2} \end{pmatrix}$$

$$\begin{pmatrix} -76 - 123\tau & -29 - \frac{93\tau}{2} & -\frac{3}{2} - \frac{5\tau}{2} & -\frac{13}{2} - 11\tau & \kappa (33 + 55\tau) \\ -31 - 50\tau & -12 - \frac{37\tau}{2} & -\frac{1}{2} - \frac{3\tau}{2} & -\frac{5}{2} - 5\tau & \kappa (14 + 22\tau) \\ -4 - 7\tau & -2 - \frac{5\tau}{2} & -\frac{1}{2} + \frac{\tau}{2} & -\frac{1}{2} - \tau & \kappa (2 + 3\tau) \\ -11 - 18\tau & -4 - \frac{15\tau}{2} & -\frac{1}{2} - \frac{\tau}{2} & -\frac{1}{2} - 2\tau & \kappa (5 + 8\tau) \\ \kappa (-35 - 55\tau) & \kappa (-13 - 21\tau) & \kappa (-1 - \tau) & \kappa (-3 - 5\tau) & 89 + 144\tau \end{pmatrix}$$

$$\frac{1}{2} (-3 - \sqrt{5})$$

$$\{0, 0, 0, 0, 1\}$$

$$\begin{pmatrix} \frac{i}{2} + j \left( -\frac{1}{2} + \frac{\tau}{2} \right) + \frac{\tau}{2} & 0 \\ 0 & -\frac{1}{2} + k \left( -\frac{1}{2} + \frac{\tau}{2} \right) + \frac{i\tau}{2} \end{pmatrix}$$

$$\begin{pmatrix} 0 & \frac{\tau}{2} & -\frac{1}{2} + \frac{\tau}{2} & \frac{1}{2} & 0 \\ -1 & 0 & 0 & 0 & 0 \\ 0 & \frac{1}{2} & -\frac{\tau}{2} & \frac{1}{2} - \frac{\tau}{2} & 0 \\ 0 & -\frac{1}{2} + \frac{\tau}{2} & \frac{1}{2} & -\frac{\tau}{2} & 0 \\ 0 & 0 & 0 & 0 & 1 \end{pmatrix}$$

$$\frac{1}{2} (3 - \sqrt{5})$$

## Index

all1by4cycles  
all2by4cycles  
allcycles  
allcyclesandperms  
alledgecycles  
allridgecycles  
alpha1hat  
alpha2hat  
antipodalindex  
beta1hat  
beta2hat  
ccrep1

cprep10  
cprep11  
cprep12  
cprep13  
cprep14  
cprep15  
cprep16  
cprep17  
cprep18  
cprep19  
cprep2  
cprep20  
cprep21  
cprep22  
cprep23  
cprep24  
cprep25  
cprep26  
cprep27  
cprep28  
cprep29  
cprep3  
cprep30  
cprep31  
cprep32  
cprep33  
cprep34  
cprep4  
cprep5  
cprep6  
cprep7  
cprep8  
cprep9  
charactertableinnerproducts  
cm1  
cm2  
cm3  
cm4  
cm5  
cmatisqmat

cmatrixisquaternion  
cmatrixtoquaternion  
cmattoqmat  
cmattormat  
complex  
complexconjugate  
compleximat  
complexnorm  
complexonemat  
complextomatrix  
conjclasses  
conjclassrepositions  
copsymliftcharactertable  
copsymliftconjclasses  
copsymliftconjclassnames  
copsymliftgrp  
copsymliftrepsnames  
copsymliftreps  
covered1  
covered10  
covered11  
covered2  
covered3  
covered4  
covered5  
covered6  
covered7  
covered8  
covered9  
davisnormopconjreps  
davisnormsgccind  
davisopsymcharactertable  
davisopsymconjclasses  
davisopsymconjclassesstart  
davisopsymconjclassnames  
davisopsymconjclassrules  
davisopsymcyclicsg  
davisopsymgrp  
davisopsymgrpfixc  
davisopsymgrpfixcrules

davisopsymgrp  
davisopsymident  
davisopsyminverse  
davisopsymliftcharactertable  
davisopsymliftconjclasses  
davisopsymliftconjclassesstart  
davisopsymliftconjclassnames  
davisopsymliftconjclassnameslong  
davisopsymliftcyclicsg  
davisopsymliftfixcprojrules  
davisopsymliftgrp  
davisopsymliftident  
davisopsymliftinverse  
davisopsymliftmat  
davisopsymliftminus  
davisopsymliftmultiply  
davisopsymliftorder  
davisopsymliftprojection  
davisopsymliftqmat  
davisopsymliftrepnames  
davisopsymliftreps  
davisopsymliftreptype1  
davisopsymliftreptype2  
davisopsymmat  
davisopsymmat1  
davisopsymmultiply  
davisopsymnorm  
davisopsymorder  
davisopsymrepnames  
davisopsymreps  
davisrelators  
davisspmat  
davisspmatlift  
davisspmatlift1  
davisspmatliftio  
davisspmatliftpre  
diagram  
elementorder  
evenperms  
Format

formatkappa  
fromcomplex  
fromformatkapparule  
gamma  
gen533  
gen5335  
gen5335i  
genop533  
genop5335  
genop5335lift  
genop533lift  
gm5335  
grp533  
grpop533  
grpop533grpop533lifts  
grpop533lift  
grpop533lift1  
h4tow  
ind1by2  
ind1by3  
ind1by4  
ind1by4sp  
ind1by4spperm  
ind1to2  
ind1to3  
ind1to4  
ind2by3  
ind2by4  
ind2by4sp  
ind2by4spperm  
ind2to1  
ind2to3  
ind2to4  
ind3by4  
ind3by4sp  
ind3by4spperm  
ind3to1  
ind3to2  
ind3to4  
ind4to1

ind4to2  
ind4to3  
insideoutmat  
insideoutmatlift  
insideoutmatlift2  
inverseSU11H  
inverseSU11Hq  
ioconjspmat1word  
iofieldth  
isSU11H  
isSU11Hq  
jmat  
kappa  
ldot  
matrixiscomplex  
matrixisquaternion  
matrixtocomplex  
matrixtoquaternion  
moveback  
moveback1  
noninfpositions  
nv5335  
pbarcomplex  
pbargen1  
pbargen1lift  
pbargen1liftconj  
pbargen2  
pbargen2lift  
pbargen2liftconj  
pbargrp  
pbargrplift  
pbargrppbargrplift  
pbarquats  
pbarquatsalphaauto  
pbarquatsalphaautoperm  
pcomplex  
pcomplexconjclasses  
permsignmats  
pgen1  
pgen1lift



pgen1liftconj  
pgen2  
pgen2lift  
pgen2liftconj  
pgrp  
pgrpcharacter table  
pgrplift  
pgrppgrplift  
pgrpnames  
pgrpnames  
pquatmats  
pquatmatsconjclasses  
pquatmatsconjclassnames  
pquatmatsio  
pquatmatsiorules  
pquatmatsrules  
pquats  
pquatsalphaauto  
pquatsalphaautoinvperm  
pquatsalphaautoperm  
pquatsbetamapperm  
pquatsinverseperm  
pquatsio  
pquatsiorules  
pquatsminusperm  
pquatsmultiplyperm  
pquatsrules  
qm1  
qm2  
qm3  
qm4  
qm5  
qmattocmat  
qmattormat  
quaternion  
quaternionconjugate  
quaternionicmat  
quaternionjcmat  
quaternionkcmat  
quaternionnorm

quaterniononecmat  
quaterniontocmatrix  
quaterniontomatrix  
r  
reduce1  
reducesetp  
reflectionfactor  
reflectionfactor1  
reflectionfactor2  
reflectionfactor3  
reflectionfactor4  
reflectionlift  
reflectvectorseq  
relators533  
relators5335  
relators5335i  
relatorsop533  
relatorsop5335  
repcycles  
represent  
representcondition  
representmat  
representmatcondition  
rho1rep  
rho2fieldtheta  
rho2primeinvrep  
rho2primerep  
rho2primereporig  
rho2rep  
rho3primeinvrep  
rho3primerep  
rho3primereporig  
rho3rep  
rho4alphainvrep  
rho4alpharep  
rho4primealphainvrep  
rho4primealpharep  
rho4primefieldth  
rho4primerep  
rho4rep

rho5alphainvrep  
rho5alpharep  
rho5fieldtheta  
rho5rep  
rho6alphainvrep  
rho6alpharep  
rho6rep  
rhtwist  
rm1  
rm2  
rm3  
rm4  
rm5  
rmat  
rmatiscmat  
rmatismat  
rmattocmat  
rmattoqmat  
s  
s5points  
selement  
sggen  
sgpairsgen  
signmats  
spinlift  
spinnuofptandmat  
spinnuofptandmatcheck  
spinprojection  
spinprojectionq  
spinvectorseq  
stab45  
symgrp  
t1classes  
t1fromconj  
t1liftstabilizersandmats  
t1reps  
t2classes  
t2fromconj  
t2liftstabilizersandmats  
t2reps

t3classes  
t3fromconj  
t3liftstabilizersandmats  
t3reps  
t4classes  
t4fromconj  
t4liftstabilizersandmats  
t4reps  
t5classes  
t5fromconj  
t5liftstabilizersandmats  
t5reps  
tablesequence  
tau  
tocomplex  
toQkappa  
toQroot5  
toQtau  
trymat1a  
trymat1b  
trymat1c  
trymat2c  
v1indrules  
v1liftstabilizer  
v1liftstabmats  
v1orbit  
v1reps  
v1traces  
v2edges  
v2indrules  
v2liftstabilizer  
v2liftstabmats  
v2orbit  
v2reps  
v2traces  
v3edges  
v3indrules  
v3liftstabilizer  
v3liftstabmats  
v3orbit

v3reps  
v3traces  
v4edges  
v4entrylist  
v4entrylistt  
v4indrules  
v4liftstabilizer  
v4liftstabmats  
v4orbit  
v4orbitpre  
v4reps  
v4traces  
v5indrules  
v5liftstabilizer  
v5liftstabmats  
v5orbit  
v5reps  
v5traces  
vertextraces  
verts5335  
wtoh4
